# Supplementary material for: Void galaxies in the nearby Universe. I. Sample description
Source: arXiv:1812.02785 ancillary file (2018-12-13)
Supplement: Supplementary file 1 [file Appendix.pdf]

## APPENDIX A: ON-LINE DATA FOR ELECTRONIC VERSION

### A1 Tables of the Nearby Void Galaxy catalog, 'inner' and 'outer' parts

Here we present the compilation of main parameters for the whole Nearby Void Galaxy sample divided into Table A1 and A2 with inner and outer subsamples, respectively. They both have the structure as described in Subsection ?? . Table A1 contains 1088 inner void galaxies with Notes in the bottom of the table for part of individual galaxies, mainly devoted to galaxy clustering with other void galaxies. Table A2 contains 266 outer void galaxies with similar Notes in the bottom.

Table A1: Main parameters of 'inner' subsample galaxies in the nearby voids

| Nu. | Name                    | RA (J2000)       | Dec.     | $V_{\text{hel}} \pm \sigma_V$ | $V_{\text{LG}}$ | $V_{\text{dist}}$ | $B_{\text{tot}}$ | $A_B$  | $M_B$  | $M_K$  | $D_{\text{NN}}$ | Void | Notes |
|-----|-------------------------|------------------|----------|-------------------------------|-----------------|-------------------|------------------|--------|--------|--------|-----------------|------|-------|
| (1) | (2)                     | (3)              | (4)      | (5)                           | (6)             | (7)               | (8)              | (9)    | (10)   | (11)   | (12)            | (13) |       |
| 1   | AGC102728               | J000021.4+310119 |          | 566 5                         | 836             | 685               | 19.40            | 0.20   | -10.66 | -      | 4.17            | 25   |       |
| 2   | PGC000083               | J000106.5+322241 |          | 542 8                         | 815             | 667               | 18.04            | 0.22   | -11.99 | -14.72 | 4.09            | 25   |       |
| 3   | ESO149-013              | J000246.7-524618 | 1498 12  | 1498 12                       | 1418            | 1259              | 15.71            | 0.07   | -15.55 | -17.90 | 4.70            | 04   |       |
| 4   | PGC000285               | J000406.3-572333 | 1889 64  | 1786                          | 1640            | 16.55             | 0.08             | -15.29 | -17.63 | 2.42   | 04              |      |       |
| 5   | PGC000389               | J000535.9-412856 | 1500 57  | 1475                          | 1278            | 18.23             | 0.07             | -13.06 | -      | 3.26   | 03              | ++   |       |
| 6   | ESO293-034              | J000619.9-413000 | 1512 6   | 1487                          | 1279            | 13.62             | 0.07             | -17.67 | -21.80 | 3.28   | 03              | ++   |       |
| 7   | PGC000482               | J000625.4-413024 | 1428 62  | 1402                          | 1279            | 15.10             | 0.07             | -16.18 | -18.57 | 3.28   | 03              | ++   |       |
| 8   | AGC748778               | J000634.3+153039 | 258 5    | 486                           | 463             | 18.91             | 0.28             | -10.38 | -      | 4.38   | 25              |      |       |
| 9   | ESO293-035              | J000651.6-415023 | 1552 7   | 1525                          | 1280            | 16.77             | 0.06             | -14.51 | -16.86 | 3.29   | 03              | ++   |       |
| 10  | PGC000544               | J000652.8-412530 | 1435 81  | 1410                          | 1279            | 17.92             | 0.07             | -13.37 | -15.97 | 3.30   | 03              | ++   |       |
| 11  | ESO149-018              | J000714.4-523712 | 1791 6   | 1710                          | 1554            | 15.86             | 0.05             | -15.83 | -18.19 | 3.02   | 04              |      |       |
| 12  | NGC0007                 | J000820.9-295455 | 1499 3   | 1531                          | 1340            | 14.34             | 0.06             | -17.04 | -18.49 | 2.23   | 03              |      |       |
| 13  | PGC1737465              | J000903.3+252750 | 1393 5   | 1647                          | 1492            | 17.49             | 0.16             | -14.22 | -17.44 | 4.73   | 01              |      |       |
| 14  | PGC736507               | J000936.2-285138 | 898 54   | 935                           | 744             | 19.14             | 0.05             | -10.95 | -13.30 | 2.94   | 03              |      |       |
| 15  | IC1532                  | J000952.7-642218 | 1834 9   | 1698                          | 1573            | 14.77             | 0.09             | -16.99 | -20.59 | 4.65   | 04              |      |       |
| 16  | PGC3193167              | J001002.7-280554 | 839 89   | 879                           | 688             | 19.47             | 0.06             | -10.46 | -12.81 | 2.16   | 03              |      |       |
| 17  | ESO538-024              | J001017.9-181554 | 1546 2   | 1634                          | 1438            | 15.14             | 0.14             | -16.47 | -18.82 | 3.43   | 25              |      |       |
| 18  | ESO293-045              | J001124.8-412354 | 1465 4   | 1438                          | 1283            | 15.12             | 0.05             | -16.15 | -18.80 | 3.46   | 03              |      |       |
| 19  | PGC138138               | J001354.1+124826 | 1700 5   | 1915                          | 1732            | 17.91             | 0.45             | -14.42 | -      | 4.20   | 03              | ++   |       |
| 20  | UGC00132                | J001400.8+125750 | 1678 3   | 1894                          | 1733            | 15.41             | 0.45             | -16.92 | -19.11 | 4.22   | 03              | ++   |       |
| 21  | PISCESA                 | J001446.0+104847 | 235 2    | 443                           | 412             | 17.89             | 0.42             | -11.29 | -13.65 | 3.51   | 25              |      |       |
| 22  | PGC1409128              | J001617.5+122454 | 1664 10  | 1876                          | 1707            | 17.19             | 0.47             | -15.12 | -18.47 | 4.08   | 03              |      |       |
| 23  | PGC127393               | J001636.1-641137 | 1745 39  | 1608                          | 1494            | 15.48             | 0.07             | -16.14 | -19.05 | 4.51   | 04              |      |       |
| 24  | ESO194-002              | J001830.5-473920 | 1494 60  | 1433                          | 1277            | 16.20             | 0.05             | -15.07 | -17.92 | 4.25   | 04              |      |       |
| 25  | PGC001225               | J001909.3-573830 | 1746 3   | 1637                          | 1502            | 15.36             | 0.06             | -16.27 | -19.35 | 4.06   | 04              |      |       |
| 26  | UGC00191                | J002005.1+105245 | 1144 2   | 1349                          | 1182            | 14.00             | 0.50             | -17.55 | -19.99 | 2.02   | 03              |      |       |
| 27  | HIPASSJ0021+08          | J002041.7+083655 | 693 3    | 890                           | 720             | 17.22             | 0.59             | -13.34 | -      | 3.43   | 25              |      |       |
| 28  | ESO078-022              | J002057.0-635125 | 1759 5   | 1622                          | 1495            | 14.52             | 0.08             | -17.12 | -20.37 | 4.72   | 04              |      |       |
| 29  | ESO150-005              | J002226.3-533852 | 1436 3   | 1345                          | 1203            | 14.00             | 0.08             | -17.16 | -19.81 | 5.80   | 04              |      |       |
| 30  | PGC001457               | J002244.4-064107 | 1539 7   | 1674                          | 1494            | 15.66             | 0.17             | -16.07 | -19.57 | 2.03   | 25              |      |       |
| 31  | PGC580292               | J002305.0-405906 | 1703 44  | 1672                          | 1510            | 17.03             | 0.03             | -14.58 | -16.93 | 3.00   | 04              |      |       |
| 32  | NGC0100                 | J002402.9+162913 | 838 3    | 1059                          | 906             | 13.86             | 0.26             | -16.87 | -19.61 | 4.15   | 25              |      |       |
| 33  | PGC001714               | J002751.5+032923 | 1382 3   | 1555                          | 1390            | 16.22             | 0.09             | -15.27 | -17.56 | 4.65   | 03              |      |       |
| 34  | PGC001750               | J002826.6+050016 | 1340 8   | 1519                          | 1356            | 15.44             | 0.06             | -15.96 | -18.09 | 4.30   | 03              |      |       |
| 35  | UGC00290                | J002908.4+155357 | 765 1    | 982                           | 834             | 16.71             | 0.46             | -14.04 | -16.39 | 3.34   | 25              |      |       |
| 36  | PGC901638               | J002951.4-160954 | 724 59   | 811                           | 639             | 17.74             | 0.12             | -12.09 | -15.79 | 2.00   | 03              |      |       |
| 37  | UGC00300                | J003004.2+033046 | 1345 2   | 1518                          | 1355            | 16.52             | 0.09             | -14.91 | -15.78 | 4.72   | 03              |      |       |
| 38  | AGC102655               | J003013.6+241759 | 1651 5   | 1891                          | 1759            | 17.89             | 0.12             | -14.14 | -      | 7.35   | 03              |      |       |
| 39  | ESO294-020              | J003209.4-401602 | 1418 23  | 1387                          | 1258            | 14.38             | 0.13             | -16.94 | -20.05 | 3.20   | 03              |      |       |
| 40  | ESO539-015              | J003248.2-183516 | 1328 64  | 1402                          | 1235            | 15.56             | 0.09             | -15.67 | -18.01 | 3.95   | 03              |      |       |
| 41  | PGC002084               | J003448.9+072701 | 555 10   | 739                           | 588             | 15.46             | 0.17             | -14.07 | -18.09 | 3.33   | 25              |      |       |
| 42  | PGC240489               | J003916.4-762054 | 1743 7   | 1553                          | 1472            | 15.30             | 0.26             | -16.48 | -18.47 | 3.70   | 24              |      |       |
| 43  | ESO079-005              | J004044.2-632627 | 1713 6   | 1572                          | 1464            | 13.75             | 0.09             | -17.85 | -19.82 | 5.37   | 04              |      |       |
| 44  | NGC0216                 | J004126.9-210253 | 1536 7   | 1594                          | 1437            | 13.71             | 0.08             | -17.84 | -20.92 | 2.38   | 03              |      |       |
| 45  | PGC1662401              | J004129.4+220232 | 810 8    | 1037                          | 916             | 16.94             | 0.23             | -13.78 | -15.91 | 3.80   | 03              |      |       |
| 46  | AGC104208               | J004142.5+125934 | 676 8    | 875                           | 740             | 20.43             | 0.43             | -10.03 | -      | 2.39   | 25              |      |       |
| 47  | PGC773446               | J004311.4-255614 | 1409 123 | 1442                          | 1214            | 18.10             | 0.06             | -13.06 | -15.41 | 3.06   | 03              |      |       |
| 48  | NGC0244                 | J004546.4-153549 | 941 4    | 1021                          | 871             | 13.79             | 0.09             | -16.68 | -19.22 | 5.05   | 03              |      |       |
| 49  | PGC002805               | J004747.5-095358 | 1344 1   | 1449                          | 1302            | 14.45             | 0.15             | -16.95 | -19.88 | 3.76   | 03              |      |       |
| 50  | ESO079-007              | J005004.1-663310 | 1670 4   | 1514                          | 1417            | 13.65             | 0.07             | -17.86 | -20.64 | 5.18   | 04              |      |       |
| 51  | PGC838777               | J005039.9-203903 | 1598 39  | 1651                          | 1507            | 16.00             | 0.08             | -15.65 | -17.27 | 2.71   | 03              |      |       |
| 52  | UGC00521                | J005112.1+120128 | 677 5    | 867                           | 744             | 15.63             | 0.28             | -14.69 | -15.82 | 2.06   | 25              |      |       |
| 53  | PGC002997               | J005115.6+104800 | 1137 8   | 1322                          | 1198            | 16.22             | 0.20             | -15.05 | -17.40 | 3.74   | 03              |      |       |
| 54  | PGC003043               | J005159.6-002912 | 1625 1   | 1767                          | 1632            | 15.26             | 0.17             | -16.66 | -19.11 | 2.86   | 03              |      |       |
| 55  | PGC003062               | J005217.2-035801 | 1411 3   | 1538                          | 1401            | 16.05             | 0.25             | -15.62 | -17.49 | 3.43   | 03              |      |       |
| 56  | PGC3200457              | J005225.7-305426 | 1349 123 | 1352                          | 1214            | 19.26             | 0.07             | -11.91 | -14.27 | 3.19   | 03              |      |       |
| 57  | ESO151-002              | J005311.4-542157 | 1387 45  | 1281                          | 1166            | 15.21             | 0.08             | -15.88 | -19.99 | 6.89   | 04              |      |       |
| 58  | UGC00578                | J005621.1+394933 | 1509 8   | 1766                          | 1697            | 14.76             | 0.26             | -17.33 | -20.37 | 9.20   | 01              |      |       |
| 59  | PGC1677631              | J005713.8+225239 | 1705 6   | 1925                          | 1824            | 17.84             | 0.17             | -14.32 | -16.67 | 8.99   | 03              |      |       |
| 60  | AGC104227               | J005823.7+041825 | 1198 8   | 1354                          | 1233            | 19.31             | 0.10             | -11.93 | -      | 5.27   | 03              |      |       |
| 61  | PGC3197947              | J005909.1-273651 | 1439 89  | 1454                          | 1322            | 19.34             | 0.09             | -12.04 | -14.39 | 2.32   | 03              |      |       |
| 62  | NGC0337A                | J010133.9-073517 | 1080 6   | 1185                          | 1059            | 12.90             | 0.44             | -18.35 | -18.50 | 6.68   | 03              |      |       |
| 63  | ESO151-019              | J010220.6-541933 | 1360 6   | 1250                          | 1143            | 14.87             | 0.07             | -16.18 | -18.55 | 6.68   | 04              |      |       |
| 64  | PGC073553               | J010321.8-355250 | 1350 66  | 1323                          | 1201            | 16.10             | 0.06             | -15.04 | -17.83 | 3.75   | 03              |      |       |
| 65  | UGC00655                | J010401.4+415030 | 828 4    | 1084                          | 1027            | 15.08             | 0.28             | -15.94 | -18.18 | 2.77   | 01              |      |       |
| 66  | PGC003853               | J010504.9-061245 | 1095 2   | 1203                          | 1083            | 12.43             | 0.57             | -19.00 | -21.22 | 6.65   | 03              |      |       |
| 67  | PGC493444               | J010718.0-475633 | 837 59   | 753                           | 644             | 19.22             | 0.06             | -10.56 | -12.91 | 3.86   | 02              |      |       |
| 68  | NGC0406                 | J010725.2-695246 | 1506 6   | 1333                          | 1251            | 13.05             | 0.10             | -18.22 | -20.91 | 4.61   | 04              |      |       |
| 69  | UGC00695                | J010746.5+010350 | 636 1    | 772                           | 670             | 15.33             | 0.12             | -14.60 | -17.13 | 2.68   | 03              |      |       |
| 70  | PGC004055               | J010822.0-381233 | 645 60   | 605                           | 489             | 16.09             | 0.05             | -13.09 | -15.44 | 2.29   | 02              |      |       |
| 71  | PGC1185205              | J010908.0+010716 | 1157 1   | 1304                          | 1178            | 17.10             | 0.11             | -14.05 | -16.40 | 6.05   | 03              | ++   |       |
| 72  | PGC1190331              | J010910.1+011728 | 1094 6   | 1231                          | 1122            | 17.54             | 0.10             | -13.49 | -15.84 | 6.23   | 03              | ++   |       |
| 73  | PGC3202636              | J011000.3-304749 | 1049 123 | 1042                          | 925             | 19.24             | 0.10             | -11.37 | -13.72 | 5.89   | 03              |      |       |
| 74  | SDSSJ011003.68-000036.4 | J011003.7-000036 | 1137 2   | 1268                          | 1159            | 19.82             | 0.13             | -11.32 | -13.67 | 6.04   | 03              | ++   |       |
| 75  | ESO243-050              | J011049.0-422231 | 1477 4   | 1416                          | 1306            | 17.04             | 0.03             | -14.26 | -19.15 | 4.27   | 04              |      |       |
| 76  | AGC114584               | J011250.5+015207 | 1089 6   | 1225                          | 1123            | 18.08             | 0.16             | -13.02 | -      | 5.99   | 03              | ++   |       |
| 77  | PGC135629               | J011250.7+010249 | 1100 6   | 1233                          | 1184            | 16.10             | 0.13             | -15.08 | -17.43 | 5.81   | 03              | ++   |       |
| 78  | NGC0428                 | J011255.7+005854 | 1154 3   | 1287                          | 1184            | 11.95             | 0.12             | -19.22 | -21.67 | 5.80   | 03              | ++   |       |
| 79  | UGC00772                | J011339.4+005230 | 1175 3   | 1307                          | 1185            | 16.46             | 0.12             | -14.71 | -17.06 | 5.75   | 03              | ++   |       |
| 80  | IC0088                  | J011420.4+005501 | 1108 2   | 1239                          | 1186            | 17.15             | 0.14             | -14.04 | -16.39 | 5.71   | 03              | ++   |       |
| 81  | PGC3309554              | J011542.4-610053 | 1139 123 | 997                           | 908             | 19.24             | 0.09             | -11.32 | -13.68 | 5.66   | 02              |      |       |

| (1) | (2)            | (3)              | (4)      | (5)  | (6)  | (7)   | (8)  | (9)    | (10)   | (11) | (12) | (13) |
|-----|----------------|------------------|----------|------|------|-------|------|--------|--------|------|------|------|
| 82  | PGC597056      | J011603.8-393218 | 1903 54  | 1852 | 1746 | 18.89 | 0.06 | -13.06 | -15.41 | 5.11 | 04   |      |
| 83  | PGC289052      | J011901.7-680242 | 2052 6   | 1882 | 1804 | 14.77 | 0.10 | -17.29 | -20.15 | 7.90 | 04   |      |
| 84  | NGC0525        | J012452.9+094212 | 1624 8   | 1781 | 1704 | 14.54 | 0.38 | -17.68 | -21.26 | 3.22 | 03   | +    |
| 85  | PGC238395      | J012453.3-765405 | 1696 6   | 1496 | 1431 | 16.55 | 0.21 | -15.12 | -17.71 | 3.11 | 24   |      |
| 86  | PGC3310386     | J012651.8-201453 | 1229 123 | 1259 | 1165 | 19.25 | 0.14 | -11.90 | -14.26 | 4.09 | 03   |      |
| 87  | UGC01038       | J012747.3+431507 | 1228 7   | 1473 | 1445 | 17.45 | 0.27 | -14.31 | -17.24 | 5.88 | 01   |      |
| 88  | PGC127483      | J012822.4-651615 | 1644 6   | 1481 | 1406 | 14.86 | 0.13 | -16.70 | -19.87 | 5.71 | 04   |      |
| 89  | PGC3177089     | J012828.0-342659 | 1589 89  | 1554 | 1461 | 16.57 | 0.07 | -15.01 | -17.36 | 2.07 | 04   |      |
| 90  | PGC1024261     | J012949.8-070640 | 1453 45  | 1539 | 1455 | 16.92 | 0.15 | -14.73 | -18.42 | 2.63 | 03   |      |
| 91  | PGC087289      | J013032.0+112925 | 975 5    | 1134 | 1067 | 18.39 | 0.47 | -12.90 | -      | 4.68 | 03   |      |
| 92  | ESO052-008     | J013647.7-675726 | 1428 4   | 1253 | 1185 | 14.71 | 0.10 | -16.44 | -18.25 | 3.74 | 04   |      |
| 93  | ESO297-015     | J013752.4-403220 | 1414 45  | 1346 | 1265 | 14.53 | 0.08 | -16.74 | -19.76 | 3.86 | 04   |      |
| 94  | PGC1041571     | J014014.0-054127 | 1288 6   | 1372 | 1305 | 17.42 | 0.15 | -13.99 | -16.34 | 2.77 | 03   |      |
| 95  | ESO297-020     | J014047.8-411247 | 1441 7   | 1368 | 1290 | 15.54 | 0.08 | -15.78 | -18.63 | 3.98 | 04   |      |
| 96  | 6dFJ0142...    | J014253.2-432355 | 1529 64  | 1445 | 1370 | 18.90 | 0.06 | -12.53 | -16.63 | 4.62 | 04   |      |
| 97  | PGC627745      | J014320.3-370842 | 1449 45  | 1392 | 1317 | 16.60 | 0.06 | -14.74 | -18.78 | 2.71 | 04   |      |
| 98  | ESO013-020     | J014355.5-775736 | 1123 60  | 917  | 860  | 16.31 | 0.26 | -14.31 | -17.71 | 5.17 | 02   |      |
| 99  | PGC3175680     | J014616.6-331334 | 1649 123 | 1607 | 1537 | 19.50 | 0.09 | -12.21 | -14.56 | 2.66 | 04   |      |
| 100 | ESO080-006     | J014717.6-625812 | 1554 8   | 1392 | 1327 | 14.33 | 0.11 | -17.08 | -19.43 | 4.85 | 04   |      |
| 101 | UGC01207       | J014726.3+820934 | 1256 4   | 1501 | 1539 | 16.50 | 1.20 | -16.32 | -17.61 | 5.21 | 22   |      |
| 102 | PGC3209216     | J014742.4-300706 | 1049 123 | 1020 | 952  | 19.43 | 0.07 | -11.22 | -13.57 | 4.73 | 03   |      |
| 103 | NGC0685        | J014742.8-524543 | 1360 3   | 1236 | 1168 | 11.90 | 0.10 | -19.22 | -21.84 | 5.98 | 04   |      |
| 104 | UGC01198       | J014917.6+851537 | 1143 9   | 1383 | 1425 | 14.94 | 0.51 | -17.03 | -20.57 | 4.52 | 22   |      |
| 105 | PGC166411      | J014928.9+553354 | 656 1    | 905  | 915  | 15.73 | 1.54 | -16.30 | -16.77 | 2.66 | 01   |      |
| 106 | UGC01281       | J014931.6+323520 | 143 4    | 353  | 383  | 13.10 | 0.20 | -15.70 | -15.61 | 2.74 | 08   |      |
| 107 | ESO245-008     | J015159.6-425750 | 1379 39  | 1292 | 1228 | 16.00 | 0.07 | -15.20 | -18.63 | 4.83 | 04   |      |
| 108 | PGC131044      | J015212.8-373238 | 1385 38  | 1321 | 1257 | 15.75 | 0.08 | -15.51 | -19.61 | 3.29 | 04   |      |
| 109 | NGC0723        | J015345.7-234528 | 1486 3   | 1480 | 1413 | 13.47 | 0.05 | -18.01 | -21.10 | 2.36 | 03   | ++   |
| 110 | ESO477-012     | J015346.2-230646 | 1463 60  | 1460 | 1413 | 16.52 | 0.05 | -14.96 | -17.32 | 2.34 | 03   | ++   |
| 111 | PGC131056      | J015429.6-395941 | 1272 39  | 1196 | 1134 | 15.85 | 0.07 | -15.18 | -18.53 | 4.30 | 03   |      |
| 112 | PGC166064      | J015520.2+275714 | 207 2    | 400  | 418  | 16.30 | 0.30 | -12.79 | -15.14 | 3.36 | 08   |      |
| 113 | PGC007237      | J015612.0+053519 | 900 64   | 1017 | 983  | 15.11 | 0.22 | -15.76 | -19.42 | 3.83 | 03   |      |
| 114 | ESO052-010     | J015649.7-685946 | 1386 5   | 1202 | 1146 | 15.90 | 0.12 | -15.20 | -18.48 | 3.11 | 24   |      |
| 115 | 2MASXJ0157...  | J015722.4-491520 | 1322 67  | 1206 | 1147 | 18.06 | 0.07 | -12.99 | -17.61 | 5.51 | 04   |      |
| 116 | UGC01443       | J015733.9+034253 | 845 8    | 953  | 920  | 16.13 | 0.14 | -14.52 | -18.18 | 3.32 | 03   |      |
| 117 | NGC0746        | J015751.0+445507 | 705 10   | 935  | 942  | 13.70 | 0.43 | -17.28 | -19.67 | 2.78 | 01   |      |
| 118 | NGC0802        | J015906.1-675213 | 1479 5   | 1298 | 1242 | 14.15 | 0.11 | -17.11 | -19.78 | 3.44 | 04   |      |
| 119 | PGC166065      | J020010.1+284952 | 164 2    | 357  | 387  | 17.20 | 0.24 | -11.66 | -14.40 | 2.96 | 08   | ++   |
| 120 | NGC0784        | J020116.9+285014 | 188 4    | 380  | 387  | 12.22 | 0.25 | -16.65 | -17.88 | 2.66 | 08   | ++   |
| 121 | PGC3207684     | J020140.1-291749 | 660 123  | 624  | 575  | 19.45 | 0.07 | -10.10 | -12.45 | 3.36 | 03   |      |
| 122 | UGC01561       | J020405.0+241230 | 608 2    | 784  | 778  | 15.37 | 0.36 | -15.13 | -17.48 | 2.02 | 03   |      |
| 123 | ESO114-028     | J020637.3-605806 | 1448 6   | 1286 | 1234 | 15.99 | 0.13 | -15.28 | -17.63 | 4.07 | 04   |      |
| 124 | ESO030-008     | J020901.8-755606 | 1658 30  | 1452 | 1403 | 14.88 | 0.21 | -16.75 | -18.96 | 3.14 | 24   |      |
| 125 | PGC3211474     | J020953.2-285926 | 1319 123 | 1279 | 1241 | 19.25 | 0.05 | -11.95 | -14.30 | 2.19 | 03   |      |
| 126 | ESO298-015     | J021038.9-405504 | 1416 4   | 1326 | 1283 | 14.22 | 0.08 | -17.08 | -19.21 | 3.92 | 04   |      |
| 127 | ESO114-032     | J021353.0-594216 | 1471 17  | 1310 | 1264 | 16.19 | 0.14 | -15.14 | -18.09 | 4.30 | 04   |      |
| 128 | ESO298-023     | J021427.5-391107 | 1373 7   | 1287 | 1250 | 14.73 | 0.06 | -16.50 | -19.59 | 3.28 | 04   |      |
| 129 | PGC3211230     | J021440.1-301009 | 1739 89  | 1690 | 1658 | 19.21 | 0.09 | -12.66 | -15.01 | 4.87 | 04   |      |
| 130 | PGC768347      | J021444.9-262328 | 1312 59  | 1279 | 1250 | 18.14 | 0.06 | -13.09 | -17.38 | 2.06 | 03   |      |
| 131 | ESO197-033     | J021457.7-512603 | 1288 7   | 1155 | 1112 | 16.36 | 0.11 | -14.66 | -17.48 | 4.91 | 04   |      |
| 132 | PGC721555      | J021525.7-300518 | 1499 89  | 1450 | 1419 | 18.30 | 0.08 | -13.23 | -15.58 | 3.04 | 04   |      |
| 133 | PGC3210819     | J022308.8-295233 | 779 89   | 725  | 704  | 18.85 | 0.07 | -11.07 | -13.50 | 3.59 | 03   |      |
| 134 | PGC009119      | J022414.9-194930 | 1052 29  | 1039 | 1028 | 15.52 | 0.14 | -15.37 | -17.66 | 3.97 | 03   |      |
| 135 | PGC168300      | J022434.4+560041 | 294 16   | 526  | 567  | 17.16 | 2.10 | -14.39 | -17.89 | 2.72 | 09   |      |
| 136 | PGC3240297     | J022435.7-264832 | 1109 123 | 1067 | 1050 | 19.32 | 0.05 | -11.52 | -13.87 | 2.87 | 03   |      |
| 137 | PGC009140      | J022443.5-733048 | 316 7    | 112  | 151  | 16.00 | 0.22 | -10.80 | -15.77 | 2.07 | 10   |      |
| 138 | PGC690109      | J022705.1-323242 | 1469 89  | 1401 | 1383 | 16.54 | 0.05 | -14.90 | -17.25 | 2.46 | 04   | ++   |
| 139 | PGC686530      | J022756.7-324543 | 1469 89  | 1399 | 1384 | 17.60 | 0.07 | -13.86 | -16.20 | 2.46 | 04   | ++   |
| 140 | UGC01958       | J022858.8+280839 | 1016 2   | 1184 | 1216 | 16.01 | 0.58 | -15.68 | -18.81 | 3.24 | 03   |      |
| 141 | PGC3180410     | J023107.9-343430 | 1679 123 | 1600 | 1586 | 19.31 | 0.09 | -12.46 | -14.82 | 4.18 | 04   |      |
| 142 | AGC122400      | J023122.1+254245 | 938 4    | 1097 | 1131 | 18.48 | 0.50 | -12.97 | -      | 3.61 | 03   |      |
| 143 | AGC124137      | J023137.0+093144 | 897 6    | 999  | 1022 | -     | 0.44 | -      | -      | 2.93 | 03   |      |
| 144 | PGC1800124     | J023139.3+271046 | 980 3    | 1144 | 1179 | 16.79 | 0.47 | -14.72 | -18.12 | 3.31 | 03   |      |
| 145 | UGC01999       | J023152.2+190911 | 972 3    | 1109 | 1139 | 14.87 | 0.45 | -16.55 | -18.04 | 5.12 | 03   |      |
| 146 | PGC128602      | J023155.5-543305 | 1396 8   | 1243 | 1215 | 16.11 | 0.13 | -15.13 | -17.48 | 4.11 | 04   |      |
| 147 | NGC0986A       | J023241.5-391746 | 1431 9   | 1332 | 1316 | 14.64 | 0.08 | -16.72 | -19.06 | 3.07 | 04   |      |
| 148 | PGC009723      | J023316.0+281041 | 1012 3   | 1177 | 1215 | 17.30 | 0.40 | -14.21 | -16.56 | 3.20 | 03   |      |
| 149 | PGC1681473     | J023422.1+230606 | 1490 6   | 1638 | 1674 | 17.67 | 0.73 | -14.86 | -17.21 | 2.01 | 05   |      |
| 150 | UGC02082       | J023616.1+252526 | 707 2    | 861  | 902  | 13.69 | 0.74 | -17.51 | -20.07 | 3.27 | 05   |      |
| 151 | HIPASSJ0237+12 | J023718.6+123108 | 960 4    | 1068 | 1102 | -     | 0.62 | -      | -      | 3.29 | 03   |      |
| 152 | AGC124076      | J023730.2+212246 | 950 8    | 1090 | 1130 | 17.96 | 0.65 | -13.64 | -      | 4.76 | 03   |      |
| 153 | PGC1462017     | J023741.9+143537 | 969 4    | 1084 | 1120 | 16.43 | 0.69 | -15.19 | -17.77 | 3.84 | 03   |      |
| 154 | ESO115-021     | J023747.8-612025 | 514 4    | 337  | 369  | 13.18 | 0.11 | -15.45 | -18.56 | 3.30 | 10   |      |
| 155 | AGC122397      | J023805.9+304016 | 850 4    | 1019 | 1064 | -     | 0.66 | -      | -      | 2.43 | 05   |      |
| 156 | AGC124630      | J023809.8+163233 | 975 8    | 1097 | 1135 | -     | 0.43 | -      | -      | 4.37 | 03   |      |
| 157 | PGC009994      | J023816.5+295423 | 693 2    | 860  | 905  | 16.50 | 0.64 | -14.61 | -      | 2.62 | 05   |      |
| 158 | ESO115-022     | J023824.0-581422 | 1305 17  | 1137 | 1112 | 15.38 | 0.12 | -15.71 | -16.45 | 3.43 | 04   |      |
| 159 | NGC1012        | J023915.0+300906 | 986 2    | 1152 | 1199 | 13.21 | 0.63 | -18.50 | -21.70 | 2.59 | 05   |      |
| 160 | PGC128614      | J023928.0-555906 | 1230 39  | 1069 | 1033 | 15.56 | 0.14 | -15.33 | -17.68 | 3.77 | 04   | ++   |
| 161 | ESO154-007     | J024009.5-562034 | 1204 45  | 1042 | 1033 | 15.68 | 0.11 | -15.18 | -18.03 | 3.70 | 04   | ++   |
| 162 | PGC504827      | J024024.4-471257 | 812 59   | 679  | 665  | 19.24 | 0.08 | -10.64 | -15.97 | 3.03 | 02   |      |
| 163 | NGC1036        | J024029.0+191749 | 790 2    | 920  | 963  | 13.77 | 0.40 | -17.23 | -20.14 | 4.36 | 05   |      |
| 164 | UGC02168       | J024100.8+172553 | 786 3    | 908  | 951  | 17.12 | 0.40 | -13.85 | -16.20 | 4.17 | 05   |      |
| 165 | 2MASXJ0241...  | J024147.0+080329 | 938 6    | 1025 | 1063 | -     | 0.60 | -      | -17.56 | 2.27 | 05   |      |

| (1) | (2)                     | (3)              | (4)      | (5)  | (6)  | (7)   | (8)  | (9)    | (10)   | (11) | (12) | (13) |
|-----|-------------------------|------------------|----------|------|------|-------|------|--------|--------|------|------|------|
| 166 | PGC2832054              | J024325.6+164359 | 820 4    | 938  | 983  | -     | 0.46 | -      | -      | 4.58 | 05   | ++   |
| 167 | PGC087158               | J024326.8+163946 | 818 10   | 936  | 983  | -     | 0.47 | -      | -19.86 | 4.58 | 05   | ++   |
| 168 | AGC123250               | J024340.1+230524 | 1091 6   | 1231 | 1281 | -     | 1.09 | -      | -      | 4.98 | 05   | ++   |
| 169 | AGC123170               | J024403.2+291719 | 886 4    | 1046 | 1099 | 18.11 | 0.85 | -13.63 | -      | 2.69 | 05   |      |
| 170 | AGC123843               | J024447.3+225001 | 1045 6   | 1184 | 1235 | -     | 1.18 | -      | -      | 4.76 | 05   | ++   |
| 171 | UGC02221                | J024458.0+302240 | 832 2    | 995  | 1050 | 16.65 | 0.80 | -14.94 | -17.63 | 2.62 | 05   |      |
| 172 | PGC779164               | J024535.6-252521 | 929 123  | 875  | 889  | 17.42 | 0.07 | -13.08 | -17.33 | 3.57 | 03   |      |
| 173 | PGC086806               | J024638.9+274335 | 472 4    | 625  | 681  | 17.13 | 0.54 | -13.26 | -16.66 | 2.30 | 08   |      |
| 174 | AGC123223               | J024709.3+100516 | 767 6    | 857  | 904  | -     | 0.96 | -      | -      | 3.92 | 05   |      |
| 175 | PGC351098               | J024816.0-615519 | 1229 123 | 1046 | 1025 | 18.43 | 0.11 | -12.42 | -14.77 | 2.90 | 02   |      |
| 176 | AGC124635               | J024838.5+191942 | 569 8    | 692  | 747  | -     | 0.49 | -      | -      | 2.95 | 05   |      |
| 177 | AGC124609               | J024928.4+344429 | 1588 8   | 1760 | 1822 | 18.07 | 0.32 | -14.24 | -      | 2.87 | 05   |      |
| 178 | PGC777591               | J024955.3-253327 | 1109 123 | 1051 | 1071 | 17.82 | 0.07 | -13.09 | -15.44 | 2.49 | 03   |      |
| 179 | PGC010768               | J025019.7+190643 | 1237 4   | 1358 | 1415 | 15.35 | 0.52 | -16.61 | -19.17 | 4.07 | 05   |      |
| 180 | AGC122900               | J025027.3+241834 | 1391 4   | 1530 | 1590 | -     | 0.68 | -      | -      | 2.88 | 05   |      |
| 181 | UGC02345                | J025152.7-011022 | 1513 2   | 1554 | 1600 | 14.32 | 0.31 | -17.70 | -20.10 | 2.77 | 05   |      |
| 182 | PGC087509               | J025156.8-533009 | 1330 42  | 1170 | 1161 | 16.17 | 0.16 | -15.00 | -18.29 | 3.55 | 04   |      |
| 183 | PGC1162139              | J025216.8+001741 | 1576 1   | 1623 | 1671 | 17.78 | 0.35 | -14.36 | -18.47 | 3.77 | 05   |      |
| 184 | SDSSJ025349.19-012830.2 | J025349.2-012830 | 1595 10  | 1633 | 1682 | 19.15 | 0.25 | -12.91 | -13.42 | 3.51 | 05   |      |
| 185 | ESO247-010              | J025428.6-471043 | 1407 18  | 1265 | 1266 | 15.12 | 0.11 | -16.18 | -18.58 | 2.96 | 04   |      |
| 186 | ESO356-018              | J025512.7-361758 | 1438 4   | 1335 | 1388 | 15.17 | 0.09 | -16.32 | -20.30 | 2.32 | 04   | ++   |
| 187 | PGC2807172              | J025537.8+193804 | 559 6    | 677  | 742  | 18.70 | 6.70 | -18.04 | -20.39 | 3.22 | 05   |      |
| 188 | PGC142353               | J025539.4-362008 | 1515 39  | 1411 | 1388 | 16.60 | 0.09 | -14.88 | -18.23 | 2.29 | 04   | ++   |
| 189 | UGC02392                | J025546.4+334600 | 1547 2   | 1711 | 1781 | 15.16 | 0.44 | -17.22 | -18.80 | 2.52 | 05   |      |
| 190 | AGC124629               | J025605.6+024831 | 794 8    | 847  | 903  | 19.75 | 0.48 | -11.19 | -      | 3.43 | 05   |      |
| 191 | PGC3312971              | J025610.1-510501 | 1049 123 | 894  | 892  | 19.24 | 0.11 | -11.30 | -13.65 | 2.27 | 02   |      |
| 192 | ESO154-023              | J025650.2-543414 | 575 3    | 409  | 426  | 12.74 | 0.07 | -16.16 | -18.53 | 3.71 | 10   |      |
| 193 | UGC02432                | J025726.7+100811 | 759 3    | 841  | 903  | 17.32 | 1.46 | -14.60 | -16.99 | 4.13 | 05   |      |
| 194 | IC1870                  | J025753.3-022047 | 1541 3   | 1571 | 1625 | 13.84 | 0.31 | -18.21 | -21.83 | 2.85 | 05   |      |
| 195 | ESO199-007              | J025804.1-492256 | 630 5    | 480  | 440  | 16.50 | 0.09 | -12.49 | -15.10 | 3.70 | 10   |      |
| 196 | GALFA-DW3               | J025856.2+133748 | 537 5    | 631  | 697  | 17.52 | 0.67 | -13.05 | -15.40 | 3.16 | 05   |      |
| 197 | NGC1156                 | J025942.5+251419 | 373 1    | 508  | 581  | 12.07 | 0.97 | -18.41 | -20.04 | 3.26 | 08   |      |
| 198 | SDSSJ025957.65+001545.4 | J025957.7+001545 | 1642 2   | 1682 | 1741 | 19.72 | 0.38 | -12.54 | -14.89 | 2.96 | 05   |      |
| 199 | AGESJ0300...            | J030038.7+254701 | 308 8    | 443  | 518  | -     | 1.32 | -      | -      | 3.59 | 08   |      |
| 200 | PGC2807110              | J030305.9+334139 | 210 5    | 369  | 349  | 16.70 | 0.86 | -12.56 | -14.91 | 2.28 | 08   |      |
| 201 | PGC1142424              | J030434.8-002831 | 1683 1   | 1715 | 1781 | 17.13 | 0.37 | -14.76 | -17.49 | 2.17 | 05   |      |
| 202 | ESO248-002              | J030506.2-455743 | 1389 4   | 1245 | 1258 | 14.10 | 0.06 | -17.14 | -19.27 | 2.48 | 04   |      |
| 203 | PGC142029               | J030638.9-541123 | 971 48   | 801  | 804  | 16.83 | 0.05 | -13.43 | -15.78 | 2.72 | 02   |      |
| 204 | AGC132121               | J030644.1+052008 | 678 8    | 732  | 805  | 17.27 | 0.74 | -13.68 | -      | 4.18 | 05   |      |
| 205 | PGC1166738              | J030646.9+002811 | 710 4    | 744  | 814  | 18.41 | 0.45 | -12.27 | -14.62 | 4.64 | 03   |      |
| 206 | PGC011692               | J030714.1-060534 | 1672 45  | 1678 | 1743 | 16.06 | 0.29 | -16.12 | -19.11 | 2.65 | 05   |      |
| 207 | IC1896                  | J030752.6-541251 | 1101 10  | 930  | 934  | 15.81 | 0.06 | -14.79 | -18.86 | 3.01 | 02   |      |
| 208 | ESO248-004              | J030821.2-462216 | 1393 45  | 1246 | 1262 | 17.20 | 0.07 | -14.06 | -17.61 | 2.36 | 04   |      |
| 209 | NGC1249                 | J031001.2-532009 | 1071 4   | 902  | 938  | 12.18 | 0.07 | -18.44 | -21.20 | 2.85 | 02   | ++   |
| 210 | PGC431118               | J031016.3-531953 | 1197 39  | 1027 | 938  | 15.87 | 0.07 | -14.74 | -17.10 | 2.85 | 02   | ++   |
| 211 | PGC131167               | J031049.7-414757 | 1386 39  | 1252 | 1278 | 16.03 | 0.06 | -15.25 | -18.30 | 2.14 | 04   |      |
| 212 | ESO116-012              | J031304.7-572126 | 1145 3   | 963  | 967  | 13.04 | 0.10 | -17.67 | -20.55 | 3.13 | 02   |      |
| 213 | PGC012057               | J031419.8+240914 | 1303 6   | 1421 | 1514 | 16.30 | 0.60 | -15.88 | -17.94 | 4.60 | 05   |      |
| 214 | PGC012188               | J031702.3+033858 | 890 60   | 928  | 1020 | 16.19 | 0.54 | -15.08 | -19.66 | 2.92 | 05   | ++   |
| 215 | PGC012210               | J031718.4+033643 | 900 49   | 937  | 1020 | 15.56 | 0.57 | -15.73 | -19.54 | 2.93 | 05   | ++   |
| 216 | NGC1313                 | J031815.7-662952 | 466 7    | 260  | 310  | 9.65  | 0.47 | -18.96 | -20.07 | 3.16 | 10   |      |
| 217 | NGC1311                 | J032006.9-521108 | 571 4    | 399  | 403  | 13.39 | 0.09 | -15.41 | -17.80 | 3.56 | 10   |      |
| 218 | UGC02684                | J032023.5+171746 | 351 2    | 439  | 539  | 16.53 | 0.61 | -13.42 | -15.93 | 4.40 | 08   |      |
| 219 | PGC904955               | J032032.6-155416 | 892 45   | 847  | 922  | 16.27 | 0.17 | -14.41 | -16.76 | 3.43 | 03   |      |
| 220 | PGC3243611              | J032232.5-235649 | 899 123  | 820  | 887  | 19.32 | 0.07 | -11.17 | -13.52 | 2.75 | 03   |      |
| 221 | UGC02716                | J032407.4+174512 | 381 3    | 467  | 572  | 15.28 | 0.60 | -14.79 | -16.54 | 4.35 | 08   |      |
| 222 | PGC2802320              | J032454.6+601015 | 1186 12  | 1396 | 1484 | -     | 4.31 | -      | -      | 5.08 | 06   |      |
| 223 | IC1933                  | J032539.9-524708 | 1062 3   | 885  | 908  | 12.92 | 0.08 | -17.63 | -20.28 | 2.57 | 02   |      |
| 224 | PGC645417               | J032733.9-354303 | 723 79   | 597  | 652  | 16.84 | 0.05 | -12.97 | -16.39 | 2.47 | 10   |      |
| 225 | NGC1337                 | J032805.9-082318 | 1239 3   | 1217 | 1311 | 12.44 | 0.29 | -19.12 | -21.73 | 4.13 | 05   |      |
| 226 | PGC2802321              | J033055.8+604722 | 759 12   | 967  | 1059 | -     | 4.08 | -      | -      | 2.17 | 01   |      |
| 227 | IC1954                  | J033131.4-515417 | 1063 3   | 885  | 915  | 12.13 | 0.07 | -18.43 | -21.75 | 2.47 | 02   |      |
| 228 | IC1959                  | J033312.6-502451 | 640 4    | 466  | 448  | 13.19 | 0.05 | -15.80 | -17.89 | 4.12 | 10   |      |
| 229 | PGC013216               | J033415.5-610541 | 1152 6   | 951  | 965  | 16.38 | 0.14 | -14.37 | -16.71 | 2.43 | 02   |      |
| 230 | ESO200-045              | J033501.5-512721 | 1029 4   | 850  | 919  | 16.25 | 0.06 | -14.31 | -16.66 | 2.43 | 02   |      |
| 231 | PGC013294               | J033556.8-451129 | 737 42   | 575  | 531  | 16.07 | 0.05 | -13.29 | -15.64 | 3.48 | 10   |      |
| 232 | PGC013327               | J033640.9-572114 | 986 88   | 792  | 815  | 15.82 | 0.09 | -14.51 | -18.24 | 2.83 | 02   |      |
| 233 | NGC1390                 | J033752.2-190030 | 1231 6   | 1158 | 1246 | 14.88 | 0.27 | -16.55 | -19.64 | 3.71 | 07   |      |
| 234 | FCOS1-2077              | J033840.6-352910 | 681 3    | 548  | 616  | -     | 0.05 | -      | -      | 2.70 | 10   |      |
| 235 | PGC712531               | J033903.0-304921 | 839 123  | 722  | 799  | 18.29 | 0.05 | -11.96 | -14.31 | 2.35 | 03   |      |
| 236 | NSFJ0339...             | J033923.7+350249 | 899 60   | 1035 | 1158 | -     | 2.16 | -      | -      | 3.61 | 05   |      |
| 237 | UGC02809                | J033933.0+194703 | 1288 3   | 1369 | 1496 | 16.41 | 1.13 | -16.28 | -18.63 | 4.44 | 05   |      |
| 238 | PGC681755               | J033955.0-330309 | 747 26   | 621  | 696  | 16.55 | 0.04 | -13.39 | -17.49 | 2.29 | 10   |      |
| 239 | ESO548-065              | J034002.7-192159 | 1221 34  | 1145 | 1249 | 15.44 | 0.32 | -16.05 | -18.24 | 3.70 | 07   |      |
| 240 | ESO548-073              | J034104.4-190540 | 989 39   | 913  | 1012 | 15.57 | 0.33 | -15.47 | -17.96 | 2.54 | 03   |      |
| 241 | UGC02816                | J034111.9+240045 | 1260 4   | 1355 | 1484 | 15.85 | 1.75 | -17.44 | -19.63 | 4.50 | 05   |      |
| 242 | HIPASSJ0341+18          | J034201.9+180831 | 1297 4   | 1369 | 1499 | -     | 0.91 | -      | -      | 4.32 | 05   |      |
| 243 | ESO549-002              | J034257.4-190113 | 1112 5   | 1035 | 1137 | 14.87 | 0.34 | -16.43 | -17.07 | 3.49 | 07   |      |
| 244 | PGC013684               | J034335.5-160052 | 1214 10  | 1148 | 1275 | 14.44 | 0.25 | -17.02 | -21.08 | 3.17 | 07   |      |
| 245 | PGC013745               | J034457.5-525643 | 1167 88  | 979  | 1018 | 17.04 | 0.09 | -13.77 | -17.95 | 3.02 | 04   |      |
| 246 | SDSSJ034457.81+010901.1 | J034457.8+010901 | 744 6    | 746  | 873  | 19.52 | 0.71 | -11.58 | -13.93 | 3.03 | 05   |      |
| 247 | PGC170437               | J034559.4-123149 | 955 25   | 900  | 1015 | 15.23 | 0.26 | -15.75 | -19.54 | 3.14 | 07   |      |
| 248 | UGC02905                | J035700.3+163123 | 293 3    | 345  | 496  | 15.84 | 1.32 | -14.64 | -15.56 | 5.02 | 08   |      |
| 249 | ESO201-014              | J040029.4-490147 | 1053 5   | 866  | 928  | 13.94 | 0.04 | -16.62 | -19.50 | 2.36 | 02   |      |



| (1) | (2)            | (3)              | (4)     | (5)  | (6)  | (7)   | (8)  | (9)    | (10)   | (11)  | (12) | (13) |
|-----|----------------|------------------|---------|------|------|-------|------|--------|--------|-------|------|------|
| 250 | HIPASSJ0403-01 | J040331.3-015541 | 908 5   | 880  | 990  | 16.80 | 0.99 | -14.85 | -17.20 | 2.84  | 05   | ++   |
| 251 | NGC1507        | J040427.2-021117 | 866 11  | 836  | 991  | 12.83 | 0.72 | -18.56 | -20.72 | 2.81  | 05   | ++   |
| 252 | PGC2802322     | J040808.0+643612 | 1245 12 | 1445 | 1555 | -     | 5.41 | -      | -      | 3.66  | 06   |      |
| 253 | PGC014562      | J040904.0-083737 | 894 3   | 834  | 985  | 15.44 | 0.22 | -15.43 | -15.93 | 2.86  | 07   |      |
| 254 | UGC02984       | J041312.4+132519 | 1543 2  | 1569 | 1746 | 16.49 | 2.43 | -17.83 | -19.96 | 3.55  | 05   | ++   |
| 255 | PGC213274      | J041314.4+132109 | 1553 11 | 1578 | 1746 | 16.00 | 2.46 | -18.35 | -20.87 | 3.57  | 05   | ++   |
| 256 | UGC02997       | J041604.9+081048 | 1595 5  | 1596 | 1771 | 14.98 | 1.83 | -18.78 | -21.73 | 5.47  | 05   |      |
| 257 | PGC089976      | J041639.8+605528 | 1156 4  | 1344 | 1467 | 16.31 | 3.62 | -18.82 | -21.97 | 4.55  | 06   |      |
| 258 | ESO202-028     | J043001.3-484014 | 1917 8  | 1712 | 1802 | 16.44 | 0.05 | -15.57 | -17.93 | 5.81  | 13   |      |
| 259 | ESO202-035     | J043216.4-494033 | 1872 4  | 1664 | 1753 | 13.30 | 0.05 | -18.66 | -21.82 | 5.30  | 13   |      |
| 260 | PGC3094336     | J043353.5-201027 | 1428 45 | 1302 | 1467 | 15.58 | 0.18 | -16.12 | -18.02 | 2.54  | 07   |      |
| 261 | PGC090718      | J043521.9-085619 | 1675 67 | 1590 | 1775 | 16.89 | 0.64 | -15.67 | -19.72 | 5.05  | 07   |      |
| 262 | ESO202-041     | J043657.2-521032 | 1659 5  | 1444 | 1528 | 15.01 | 0.04 | -16.64 | -19.01 | 2.49  | 13   |      |
| 263 | ESO157-047     | J043919.2-541238 | 1657 12 | 1436 | 1516 | 15.46 | 0.04 | -16.17 | -18.48 | 2.11  | 13   |      |
| 264 | ESO157-049     | J043936.9-530046 | 1673 5  | 1455 | 1539 | 14.35 | 0.03 | -17.30 | -21.36 | 2.51  | 13   |      |
| 265 | ESO119-005     | J044817.4-601738 | 989 5   | 756  | 821  | 15.69 | 0.13 | -14.70 | -18.27 | 2.77  | 02   |      |
| 266 | PGC484937      | J044832.2-484043 | 1469 54 | 1253 | 1359 | 17.82 | 0.05 | -13.58 | -15.93 | 2.22  | 13   |      |
| 267 | 2MASXJ0448...  | J044841.7+191928 | 1469 12 | 1488 | 1703 | -     | 2.29 | -      | -21.21 | 2.40  | 07   |      |
| 268 | ESO421-019     | J044910.5-291223 | 1476 5  | 1308 | 1472 | 13.21 | 0.11 | -18.42 | -18.90 | 2.84  | 07   |      |
| 269 | ESO119-016     | J045129.2-613903 | 972 4   | 737  | 802  | 14.89 | 0.11 | -15.42 | -17.77 | 2.92  | 02   | ++   |
| 270 | ESO361-015     | J045157.4-331045 | 1170 4  | 989  | 1147 | 13.56 | 0.09 | -17.51 | -20.19 | 2.64  | 07   |      |
| 271 | ESO422-005     | J045205.5-283532 | 1462 3  | 1294 | 1461 | 14.88 | 0.09 | -16.72 | -17.02 | 3.13  | 07   |      |
| 272 | PGC1021840     | J045215.7-071552 | 1657 45 | 1563 | 1772 | 16.32 | 0.25 | -15.86 | -18.58 | 5.72  | 07   |      |
| 273 | ESO485-021     | J045253.0-251445 | 1372 3  | 1214 | 1390 | 13.72 | 0.14 | -17.82 | -20.37 | 3.89  | 07   |      |
| 274 | PGC573679      | J045320.2-413808 | 1380 39 | 1176 | 1308 | 16.46 | 0.07 | -14.88 | -17.22 | 3.14  | 13   |      |
| 275 | NGC1705        | J045413.5-532140 | 629 5   | 402  | 418  | 12.79 | 0.03 | -16.03 | -18.12 | 4.59  | 10   |      |
| 276 | PGC016318      | J045455.4-613353 | 980 5   | 743  | 804  | 17.30 | 0.09 | -13.00 | -15.36 | 2.87  | 02   | ++   |
| 277 | HIPASSJ0455-28 | J045536.5-281753 | 997 6   | 827  | 999  | -     | 0.10 | -      | -      | 2.27  | 07   |      |
| 278 | PGC016389      | J045658.7-424802 | 662 6   | 453  | 507  | 14.46 | 0.05 | -14.80 | -17.41 | 3.99  | 10   |      |
| 279 | NGC1744        | J045958.0-260128 | 742 2   | 575  | 749  | 11.71 | 0.18 | -18.52 | -21.45 | 3.14  | 10   |      |
| 280 | PGC092107      | J050136.8-221520 | 1385 60 | 1229 | 1422 | 17.77 | 0.13 | -13.81 | -18.09 | 3.53  | 07   |      |
| 281 | NGC1796        | J050242.7-610824 | 1012 7  | 772  | 842  | 12.85 | 0.11 | -17.57 | -20.49 | 2.35  | 02   |      |
| 282 | ESO486-015     | J050300.3-252806 | 834 6   | 667  | 854  | 17.39 | 0.14 | -13.09 | -15.44 | 2.41  | 10   | ++   |
| 283 | ESO486-021     | J050320.0-252525 | 834 4   | 667  | 855  | 14.42 | 0.14 | -16.06 | -18.92 | 2.41  | 10   | ++   |
| 284 | UGC03234       | J050324.6+162416 | 1404 3  | 1398 | 1633 | 15.10 | 1.67 | -18.32 | -20.67 | 3.72  | 07   |      |
| 285 | ESO422-025     | J050345.9-321951 | 1212 8  | 1024 | 1194 | 15.51 | 0.08 | -15.64 | -18.09 | 3.20  | 07   |      |
| 286 | ESO552-066     | J050514.5-182321 | 1708 3  | 1562 | 1768 | 16.26 | 0.22 | -15.88 | -18.23 | 2.84  | 07   |      |
| 287 | NGC1800        | J050625.7-315715 | 804 16  | 615  | 788  | 13.12 | 0.06 | -17.11 | -19.84 | 2.36  | 10   |      |
| 288 | ESO422-033     | J050649.0-273928 | 1270 3  | 1093 | 1279 | 14.43 | 0.07 | -16.86 | -20.73 | 4.58  | 07   |      |
| 289 | ESO423-002     | J051516.3-303135 | 1469 3  | 1277 | 1464 | 13.48 | 0.12 | -18.15 | -20.96 | 4.15  | 07   |      |
| 290 | PGC3316612     | J051519.9-312545 | 1469 64 | 1275 | 1459 | 18.03 | 0.09 | -13.56 | -15.91 | 4.41  | 13   |      |
| 291 | HIPASSJ0517-32 | J051721.6-324535 | 798 6   | 599  | 781  | 15.96 | 0.08 | -14.27 | -16.62 | 2.09  | 10   |      |
| 292 | UGC03273       | J051744.4+533305 | 616 4   | 752  | 935  | 14.95 | 1.79 | -17.38 | -19.33 | 4.20  | 09   |      |
| 293 | NGC1879        | J051948.4-320837 | 1241 3  | 1042 | 1228 | 13.18 | 0.10 | -18.05 | -19.52 | 3.70  | 07   |      |
| 294 | ESO119-059     | J052229.7-600623 | 1652 45 | 1405 | 1491 | 15.90 | 0.13 | -15.78 | -18.27 | 2.18  | 13   |      |
| 295 | UGC03303       | J052459.5+043018 | 521 2   | 446  | 703  | 14.32 | 0.56 | -16.16 | -18.51 | 3.14  | 08   |      |
| 296 | HIPASSJ0525-63 | J052553.4-631547 | 895 6   | 645  | 719  | 14.96 | 0.23 | -15.23 | -      | 3.89  | 02   |      |
| 297 | ESO553-046     | J052705.7-204040 | 542 6   | 371  | 489  | 14.62 | 0.20 | -14.71 | -14.17 | 5.75  | 10   |      |
| 298 | 6dFJ0527...    | J052726.1-353317 | 1336 39 | 1123 | 1305 | 16.75 | 0.14 | -14.65 | -18.75 | 4.58  | 13   |      |
| 299 | HIPASSJ0531+08 | J053102.4+082104 | 961 6   | 898  | 1162 | -     | 1.86 | -      | -      | 5.83  | 07   |      |
| 300 | IC2135         | J053312.9-362356 | 1323 3  | 1104 | 1289 | 13.28 | 0.16 | -18.11 | -21.59 | 4.42  | 13   |      |
| 301 | ESO204-022     | J053625.8-521103 | 1291 6  | 1044 | 1170 | 15.53 | 0.18 | -15.68 | -18.03 | 3.31  | 13   |      |
| 302 | ESO487-030     | J053719.2-262553 | 1486 8  | 1290 | 1508 | 15.93 | 0.12 | -15.76 | -20.64 | 2.46  | 07   |      |
| 303 | PGC017603      | J054142.2+064051 | 451 5   | 372  | 647  | 15.70 | 2.29 | -16.33 | -19.54 | 4.19  | 08   |      |
| 304 | IC2147         | J054328.0-302942 | 1308 1  | 1096 | 1308 | 13.57 | 0.13 | -17.82 | -21.52 | 4.19  | 07   |      |
| 305 | PGC017716      | J054502.1+050409 | 375 8   | 287  | 564  | 15.55 | 3.03 | -16.92 | -19.27 | 4.88  | 08   |      |
| 306 | GALFA-DW4      | J054544.8+104616 | 629 4   | 565  | 844  | 17.36 | 2.71 | -15.67 | -18.02 | 4.23  | 08   |      |
| 307 | ESO488-017     | J054729.0-233434 | 1040 39 | 845  | 1080 | 14.87 | 0.14 | -16.12 | -18.89 | 3.51  | 07   |      |
| 308 | 2MASXJ0548...  | J054849.7-172643 | 908 45  | 731  | 983  | -     | 0.29 | -      | -17.45 | 2.81  | 07   |      |
| 309 | PGC017978      | J055054.5-144648 | 902 0   | 732  | 992  | 12.97 | 0.68 | -18.38 | -20.20 | 2.29  | 07   |      |
| 310 | PGC018096      | J055542.6+032330 | 797 3   | 693  | 980  | 15.48 | 3.56 | -18.72 | -18.59 | 3.17  | 08   |      |
| 311 | PGC138836      | J055735.2+072913 | 428 4   | 340  | 630  | 18.40 | 2.54 | -11.28 | -16.17 | 4.81  | 08   |      |
| 312 | 6dFJ0600...    | J060008.3-311734 | 1373 45 | 1148 | 1371 | -     | 0.16 | -      | -      | 3.16  | 13   | ++   |
| 313 | ESO425-001     | J060010.7-314714 | 1354 5  | 1128 | 1349 | 15.05 | 0.17 | -16.45 | -18.80 | 3.41  | 13   | ++   |
| 314 | ESO425-002     | J060034.8-285932 | 1390 2  | 1171 | 1402 | 14.48 | 0.15 | -17.09 | -17.46 | 2.53  | 07   |      |
| 315 | UGC03390       | J060205.2+360616 | 1518 2  | 1556 | 1818 | 15.56 | 2.01 | -18.43 | -21.50 | 10.95 | 09   |      |
| 316 | PGC086284      | J060226.6+145054 | 766 3   | 707  | 1000 | -     | 3.76 | -      | -19.33 | 5.63  | 09   |      |
| 317 | ESO555-028     | J060428.0-193718 | 882 3   | 686  | 946  | 15.75 | 0.39 | -15.20 | -16.15 | 2.81  | 07   |      |
| 318 | ESO364-029     | J060545.0-330454 | 786 3   | 554  | 678  | 13.67 | 0.19 | -16.36 | -19.59 | 3.16  | 10   |      |
| 319 | PGC018431      | J060719.7-341216 | 774 13  | 538  | 678  | 15.66 | 0.16 | -14.34 | -17.20 | 3.17  | 10   |      |
| 320 | ESO086-060     | J060809.4-633509 | 1626 4  | 1360 | 1451 | 15.96 | 0.22 | -15.75 | -19.68 | 3.47  | 13   |      |
| 321 | 2MASXJ0609...  | J060944.7-325001 | 1418 39 | 1183 | 1408 | 15.61 | 0.23 | -16.05 | -18.56 | 2.45  | 13   |      |
| 322 | NGC2188        | J061009.5-340621 | 743 13  | 505  | 613  | 12.09 | 0.14 | -17.67 | -18.02 | 4.05  | 10   |      |
| 323 | ESO556-002     | J061116.1-213600 | 859 8   | 652  | 913  | 14.10 | 0.33 | -16.72 | -19.07 | 2.97  | 10   |      |
| 324 | PGC075555      | J061214.2-384623 | 1718 42 | 1470 | 1675 | 16.23 | 0.33 | -15.90 | -18.20 | 4.20  | 13   |      |
| 325 | ESO205-035     | J061401.2-513240 | 1251 5  | 987  | 1138 | 16.54 | 0.28 | -14.70 | -17.05 | 3.42  | 13   |      |
| 326 | ESO121-020     | J061554.3-574332 | 582 2   | 314  | 444  | 15.73 | 0.18 | -13.37 | -15.72 | 6.63  | 10   | ++   |
| 327 | PGC385975      | J061608.5-574551 | 554 5   | 286  | 408  | 17.01 | 0.18 | -11.91 | -14.25 | 4.22  | 10   | ++   |
| 328 | 2MASXJ0619...  | J061945.7+033708 | 766 72  | 645  | 953  | -     | 3.53 | -      | -19.81 | 2.87  | 08   |      |
| 329 | PGC2807186     | J062054.3+200828 | 1318 6  | 1270 | 1573 | -     | 3.45 | -      | -      | 9.79  | 12   |      |
| 330 | 2MASXJ0622...  | J062253.7-373840 | 1833 42 | 1581 | 1796 | -     | 0.43 | -      | -18.55 | 4.46  | 13   |      |
| 331 | ESO489-056     | J062617.0-261556 | 492 3   | 263  | 461  | 16.35 | 0.27 | -12.92 | -15.27 | 5.49  | 10   |      |
| 332 | HIPASSJ0626+24 | J062621.0+243920 | 1473 3  | 1443 | 1744 | 17.70 | 1.75 | -15.95 | -18.80 | 10.80 | 12   |      |
| 333 | PGC1689759     | J062958.2+233428 | 1452 3  | 1414 | 1719 | 17.00 | 1.17 | -16.03 | -18.88 | 10.27 | 12   |      |

| (1) | (2)                     | (3)              | (4)     | (5)  | (6)  | (7)   | (8)  | (9)    | (10)   | (11)  | (12) | (13) |
|-----|-------------------------|------------------|---------|------|------|-------|------|--------|--------|-------|------|------|
| 334 | HIZOA J0630+08          | J063009.2+082116 | 364 6   | 256  | 573  | -     | 2.93 | -      | -      | 6.14  | 08   |      |
| 335 | UGC03476                | J063028.8+331805 | 447 10  | 455  | 742  | 15.76 | 1.03 | -15.30 | -17.65 | 5.04  | 09   |      |
| 336 | UGC03475                | J063028.9+393014 | 480 19  | 518  | 789  | 15.43 | 0.80 | -15.54 | -17.69 | 5.25  | 09   |      |
| 337 | ESO206-016              | J063109.6-522506 | 1191 4  | 919  | 1073 | 15.47 | 0.28 | -15.65 | -16.32 | 2.71  | 13   |      |
| 338 | ESO490-017              | J063757.1-260001 | 501 2   | 265  | 463  | 13.66 | 0.33 | -15.68 | -16.48 | 5.32  | 10   |      |
| 339 | PGC019343               | J063800.2-150123 | 747 1   | 543  | 839  | 14.33 | 1.47 | -17.44 | -21.52 | 2.71  | 08   |      |
| 340 | UGC03503                | J063801.4+223906 | 1385 3  | 1338 | 1650 | 15.93 | 0.66 | -16.50 | -19.07 | 9.81  | 12   |      |
| 341 | UGC03501                | J063838.3+491531 | 452 15  | 532  | 775  | 17.60 | 0.50 | -13.03 | -15.38 | 4.94  | 09   |      |
| 342 | ESO308-022              | J063932.9-404317 | 822 4   | 556  | 684  | 16.22 | 0.39 | -14.03 | -16.38 | 3.50  | 10   |      |
| 343 | UGC03516                | J064308.5+225226 | 1295 5  | 1245 | 1560 | 16.98 | 1.13 | -15.80 | -18.40 | 10.09 | 12   |      |
| 344 | IC2171                  | J064427.6-175557 | 786 3   | 569  | 888  | 15.17 | 1.80 | -17.06 | -19.05 | 2.49  | 08   | ++   |
| 345 | NGC2283                 | J064552.9-181243 | 841 4   | 622  | 888  | 12.95 | 1.65 | -19.13 | -21.64 | 2.41  | 08   | ++   |
| 346 | PGC076040               | J064656.6-175627 | 696 3   | 477  | 772  | 16.91 | 1.83 | -15.04 | -18.54 | 2.22  | 10   |      |
| 347 | PGC2807122              | J064755.2+473047 | 451 1   | 518  | 772  | 17.40 | 0.40 | -13.12 | -15.47 | 4.85  | 09   |      |
| 348 | HIPASSJ0653-73          | J065352.7-734228 | 1208 4  | 940  | 988  | 17.9  | 0.58 | -13.34 | -      | 2.92  | 24   |      |
| 349 | UGC03587                | J065354.8+191759 | 1267 1  | 1194 | 1519 | 14.15 | 0.40 | -17.84 | -20.69 | 8.98  | 12   |      |
| 350 | UGC03600                | J065540.0+390543 | 404 6   | 427  | 750  | 16.35 | 0.40 | -14.11 | -16.45 | 4.21  | 09   |      |
| 351 | HIZSS003B               | J070024.6-041314 | 324 5   | 145  | 456  | -     | 4.55 | -      | -      | 5.80  | 08   | ++   |
| 352 | PGC2807061              | J070028.9-041220 | 291 4   | 112  | 456  | 18.00 | 4.39 | -15.37 | -17.72 | 5.80  | 08   | ++   |
| 353 | PGC020086               | J070359.2+562911 | 1413 16 | 1516 | 1725 | 15.44 | 0.25 | -16.68 | -19.03 | 3.32  | 09   |      |
| 354 | UGC03658                | J070440.0+173457 | 1183 4  | 1096 | 1428 | 17.00 | 0.23 | -14.69 | -17.03 | 9.15  | 12   |      |
| 355 | UGC03647                | J070450.6+563113 | 1386 2  | 1489 | 1725 | 14.73 | 0.26 | -17.40 | -19.75 | 3.27  | 09   |      |
| 356 | PGC020125               | J070517.7-583108 | 564 4   | 279  | 381  | 14.95 | 0.52 | -14.16 | -16.51 | 3.70  | 10   |      |
| 357 | SDSS                    | J070623.4+302051 | 952 15  | 916  | 1269 | 19.15 | 0.32 | -12.31 | -      | 8.53  | 12   | ++   |
| 358 | UGC03672                | J070627.5+301920 | 982 2   | 956  | 1269 | 15.89 | 0.31 | -15.62 | -17.23 | 8.53  | 12   | ++   |
| 359 | UGC03698                | J070918.3+442248 | 423 4   | 466  | 822  | 15.55 | 0.41 | -15.11 | -17.47 | 4.47  | 09   | ++   |
| 360 | NGC2337                 | J071013.6+442726 | 436 5   | 479  | 822  | 13.17 | 0.38 | -17.46 | -19.83 | 4.45  | 09   | ++   |
| 361 | NGC2344                 | J071228.6+471001 | 970 5   | 1025 | 1289 | 12.89 | 0.45 | -18.80 | -21.93 | 4.89  | 09   |      |
| 362 | SDSS                    | J071305.1+292643 | 938 2   | 904  | 1175 | 16.79 | 0.31 | -14.55 | -      | 7.76  | 12   | +    |
| 363 | HIPASSJ0712-41          | J071310.6-411935 | 1693 9  | 1411 | 1635 | -     | 0.70 | -      | -      | 4.60  | 13   |      |
| 364 | UGC03755                | J071351.7+103116 | 314 2   | 189  | 554  | 14.60 | 0.38 | -15.18 | -17.77 | 5.01  | 08   |      |
| 365 | ESO310-007              | J071633.3-400547 | 1390 5  | 1108 | 1338 | 16.44 | 1.14 | -16.02 | -18.37 | 3.38  | 13   |      |
| 366 | HIPASSJ0718-79          | J071745.1-792440 | 1571 4  | 1310 | 1327 | -     | 1.50 | -      | -      | 3.28  | 24   |      |
| 367 | PGC2807062              | J071821.0-090316 | 914 5   | 706  | 1035 | -     | 1.90 | -      | -      | 3.48  | 12   |      |
| 368 | UGC03817                | J072244.5+450630 | 437 4   | 479  | 753  | 16.17 | 0.44 | -14.34 | -18.21 | 3.68  | 09   |      |
| 369 | SDSSJ072301.42+362117.1 | J072301.4+362117 | 886 2   | 882  | 1185 | 16.99 | 0.23 | -14.30 | -16.65 | 6.23  | 09   | ++   |
| 370 | SDSSJ072313.46+362213.0 | J072313.5+362213 | 973 2   | 970  | 1185 | 19.34 | 0.23 | -12.10 | -14.45 | 6.24  | 09   | ++   |
| 371 | [MU2012]J07...          | J072320.6+362441 | 938 6   | 935  | 1185 | 21.59 | 0.23 | -9.78  | -12.14 | 6.25  | 09   | ++   |
| 372 | UGC03830                | J072330.5+023657 | 1361 8  | 1196 | 1541 | 15.03 | 0.49 | -17.08 | -21.65 | 4.44  | 12   |      |
| 373 | PGC020914               | J072355.2+571653 | 1257 17 | 1358 | 1582 | 14.99 | 0.24 | -16.93 | -20.20 | 3.17  | 09   |      |
| 374 | PGC020981               | J072539.0+091059 | 1178 14 | 1040 | 1387 | 16.29 | 0.27 | -15.38 | -17.73 | 7.54  | 12   |      |
| 375 | PGC2518162              | J072655.0+555335 | 786 16  | 879  | 1110 | 18.39 | 0.32 | -12.84 | -15.19 | 3.52  | 09   |      |
| 376 | UGC03853                | J072740.0-482646 | 935 2   | 992  | 1254 | 16.45 | 0.47 | -15.19 | -18.27 | 4.27  | 12   |      |
| 377 | UGC03860                | J072817.6+404612 | 344 4   | 361  | 764  | 15.12 | 0.25 | -15.24 | -16.93 | 3.34  | 09   |      |
| 378 | ESO035-009              | J072842.6-750308 | 1124 7  | 852  | 897  | 16.33 | 0.88 | -15.00 | -17.35 | 2.74  | 02   |      |
| 379 | UGC03876                | J072917.5+275401 | 862 4   | 813  | 1140 | 14.08 | 0.20 | -17.09 | -20.04 | 7.37  | 12   |      |
| 380 | HIZOA J0730-17          | J073036.1-171747 | 1651 14 | 1410 | 1726 | -     | 4.89 | -      | -      | 4.20  | 11   |      |
| 381 | PGC2176737              | J073058.9+411000 | 891 1   | 909  | 1200 | 16.71 | 0.27 | -14.64 | -16.99 | 5.31  | 12   |      |
| 382 | ESO059-001              | J073118.4-681115 | 529 3   | 246  | 338  | 13.78 | 0.64 | -15.19 | -17.13 | 2.73  | 10   |      |
| 383 | UGC03895                | J073123.4+000312 | 1456 4  | 1276 | 1622 | 16.45 | 0.61 | -15.90 | -18.24 | 3.15  | 12   |      |
| 384 | PGC085969               | J073242.2-135404 | 1315 40 | 1084 | 1409 | 16.73 | 1.86 | -16.56 | -21.63 | 3.48  | 11   |      |
| 385 | ESO368-004              | J073254.7-352920 | 1396 4  | 1114 | 1369 | 16.39 | 1.94 | -16.92 | -19.27 | 4.08  | 13   |      |
| 386 | UGC03912                | J073412.6+043247 | 1238 2  | 1076 | 1425 | 14.67 | 0.23 | -17.01 | -19.55 | 6.09  | 12   |      |
| 387 | HIPASSJ0736-74          | J073610.0-744115 | 1145 6  | 872  | 920  | -     | 0.93 | -      | -      | 2.50  | 24   |      |
| 388 | AGC174585               | J073610.3+095911 | 356 5   | 217  | 575  | -     | 0.17 | -      | -      | 4.60  | 08   |      |
| 389 | SDSSJ073728.49+472432.8 | J073728.5+472433 | 472 5   | 520  | 789  | 18.07 | 0.46 | -12.56 | -14.91 | 3.76  | 09   |      |
| 390 | UGC03946                | J073759.6+031858 | 1195 3  | 1026 | 1376 | 14.33 | 0.23 | -17.27 | -19.62 | 6.37  | 12   |      |
| 391 | PGC2807123              | J073802.2-013014 | 1349 6  | 1160 | 1507 | 16.49 | 0.49 | -15.57 | -      | 4.09  | 12   |      |
| 392 | HIZOA J0738-15          | J073857.6-153020 | 883 14  | 644  | 967  | -     | 2.52 | -      | -      | 2.41  | 12   |      |
| 393 | PGC021494               | J073909.4-004536 | 1464 4  | 1277 | 1624 | 16.50 | 0.28 | -15.52 | -19.70 | 3.22  | 12   |      |
| 394 | PGC021511               | J073942.6-023717 | 1668 5  | 1474 | 1820 | 15.60 | 0.46 | -16.84 | -19.19 | 2.51  | 12   |      |
| 395 | UGC03964                | J074017.8-013426 | 1462 3  | 1272 | 1618 | 15.15 | 0.41 | -16.99 | -19.00 | 3.13  | 12   |      |
| 396 | UGC03966                | J074125.9+400643 | 362 2   | 371  | 757  | 14.44 | 0.22 | -15.86 | -16.65 | 2.88  | 09   |      |
| 397 | UGC03974                | J074155.4+164809 | 272 1   | 163  | 514  | 13.74 | 0.14 | -15.64 | -17.99 | 3.99  | 08   |      |
| 398 | PGC021614               | J074231.7+163340 | 283 4   | 172  | 515  | 15.39 | 0.14 | -13.99 | -16.72 | 4.00  | 08   |      |
| 399 | PGC021644               | J074308.8+035659 | 934 4   | 765  | 1117 | 15.87 | 0.18 | -15.23 | -17.30 | 6.23  | 12   |      |
| 400 | SDSSJ074443.72+250826.2 | J074443.7+250826 | 756 1   | 687  | 1023 | 18.23 | 0.18 | -12.68 | -16.78 | 5.73  | 12   | ++   |
| 401 | SDSS                    | J074455.5+250602 | 752 6   | 683  | 1023 | 20.47 | 0.18 | -10.30 | -      | 5.70  | 12   | ++   |
| 402 | HIZOA J0746-28          | J074616.3-282808 | 492 14  | 217  | 502  | -     | 4.50 | -      | -      | 4.09  | 10   |      |
| 403 | PGC021768               | J074643.5-054719 | 1329 5  | 1119 | 1463 | 14.92 | 0.62 | -17.21 | -      | 3.15  | 12   |      |
| 404 | PGC021772               | J074656.4+511743 | 447 8   | 511  | 675  | 16.68 | 0.27 | -13.42 | -15.78 | 3.42  | 09   | ++   |
| 405 | PGC021812               | J074731.8+511130 | 434 6   | 498  | 675  | 15.13 | 0.31 | -15.01 | -17.05 | 3.43  | 09   | ++   |
| 406 | ESO560-014              | J074813.9-183833 | 921 4   | 668  | 986  | -     | 1.63 | -      | -      | 2.27  | 12   |      |
| 407 | PGC021882               | J074909.8+553617 | 1198 42 | 1284 | 1520 | 15.27 | 0.32 | -16.65 | -20.32 | 2.36  | 12   |      |
| 408 | AGC174605               | J075021.7+074740 | 351 4   | 196  | 723  | 18.68 | 0.10 | -11.40 | -      | 4.84  | 08   |      |
| 409 | UGC04115                | J075702.2+142328 | 348 6   | 220  | 572  | 14.72 | 0.12 | -14.87 | -17.22 | 3.73  | 08   |      |
| 410 | UGC04117                | J075725.9+355622 | 771 13  | 752  | 1064 | 15.64 | 0.20 | -15.38 | -17.73 | 4.59  | 12   |      |
| 411 | HIZOA J0759-30          | J075959.8-304840 | 1553 14 | 1268 | 1547 | -     | 3.39 | -      | -      | 2.05  | 13   |      |
| 412 | UGC04148                | J080023.8+421138 | 722 1   | 736  | 1028 | 15.37 | 0.18 | -15.56 | -18.35 | 3.13  | 09   |      |
| 413 | PGC2463543              | J080057.9+541355 | 894 1   | 970  | 1214 | 17.70 | 0.19 | -13.59 | -15.94 | 2.54  | 12   |      |
| 414 | NGC2500                 | J080153.2+504414 | 500 12  | 558  | 817  | 12.22 | 0.17 | -18.19 | -20.73 | 3.03  | 09   |      |
| 415 | PGC022748               | J080611.2-031658 | 1347 4  | 1139 | 1489 | 14.80 | 0.13 | -16.87 | -19.31 | 3.50  | 12   |      |
| 416 | UGC04100                | J080656.4+844519 | 1008 4  | 1222 | 1301 | 16.55 | 0.27 | -14.97 | -17.32 | 2.57  | 22   |      |
| 417 | PGC1084489              | J080815.8-024313 | 1177 39 | 970  | 1321 | 17.19 | 0.15 | -14.25 | -18.42 | 4.79  | 12   |      |

| (1) | (2)                      | (3)              | (4)     | (5)  | (6)  | (7)   | (8)   | (9)    | (10)   | (11)  | (12) | (13) |
|-----|--------------------------|------------------|---------|------|------|-------|-------|--------|--------|-------|------|------|
| 418 | PGC022900                | J080935.9+413540 | 682 3   | 690  | 985  | 15.97 | 0.22  | -14.90 | -17.57 | 2.91  | 09   |      |
| 419 | HIZOA J0810-39           | J081006.6-392604 | 1421 14 | 1121 | 1365 | -     | 5.82  | -      | -      | 4.79  | 13   |      |
| 420 | SDSS J081030.65+183704.2 | J081030.7+183704 | 1486 1  | 1374 | 1724 | 18.35 | 0.16  | -13.68 | -16.03 | 7.53  | 12   |      |
| 421 | PGC2321523               | J081239.5+483645 | 526 1   | 570  | 870  | 17.34 | 0.22  | -13.26 | -15.62 | 2.36  | 09   | ++   |
| 422 | NGC2537                  | J081314.7+455924 | 452 4   | 482  | 761  | 12.27 | 0.23  | -18.05 | -20.68 | 2.73  | 09   | ++   |
| 423 | IC2233                   | J081358.9+454431 | 558 2   | 587  | 866  | 12.45 | 0.23  | -18.15 | -21.12 | 2.62  | 09   | ++   |
| 424 | NGC2541                  | J081440.1+490342 | 547 10  | 593  | 870  | 12.25 | 0.21  | -18.34 | -19.97 | 2.29  | 09   | ++   |
| 425 | HIZOA J0815-32           | J081539.8-322209 | 1301 14 | 1008 | 1283 | -     | 2.26  | -      | -      | 3.24  | 13   |      |
| 426 | NGC2552                  | J081920.5+500035 | 506 6   | 556  | 819  | 12.69 | 0.20  | -17.76 | -16.66 | 2.73  | 09   |      |
| 427 | ESO006-001               | J081922.2-850836 | 738 95  | 489  | 473  | 15.20 | 0.83  | -14.69 | -16.16 | 3.78  | 02   |      |
| 428 | ESO495-008               | J082101.1-234645 | 791 6   | 514  | 819  | 16.06 | 0.48  | -14.67 | -17.02 | 2.33  | 12   |      |
| 429 | AGC188955                | J082137.0+041901 | 758 5   | 576  | 932  | 17.50 | 0.09  | -13.12 | -15.47 | 5.50  | 12   |      |
| 430 | AGC189201                | J082325.6+175457 | 1475 6  | 1355 | 1706 | 18.99 | 0.16  | -13.01 | -      | 6.36  | 12   |      |
| 431 | PGC086398                | J082504.9+320105 | 642 1   | 595  | 919  | 16.82 | 0.20  | -13.88 | -16.23 | 3.41  | 12   |      |
| 432 | PGC2790884               | J082555.5+353232 | 747 4   | 718  | 1030 | 17.80 | 0.20  | -13.14 | -15.49 | 4.02  | 12   | ++   |
| 433 | SAO0822+3545             | J082605.6+353525 | 742 2   | 713  | 1030 | 17.76 | 0.19  | -13.18 | -15.53 | 4.00  | 12   | ++   |
| 434 | SDSS                     | J082620.0+214522 | 420 2   | 319  | 630  | 18.23 | 0.18  | -11.63 | -      | 2.18  | 08   | +    |
| 435 | ESO060-007               | J082726.9-710421 | 1524 8  | 1238 | 1309 | 16.78 | 0.80  | -15.29 | -18.64 | 2.03  | 13   |      |
| 436 | HIZOA J0829-38           | J082919.8-385740 | 1675 14 | 1371 | 1617 | -     | 9.34  | -      | -      | 3.60  | 13   |      |
| 437 | PGC023847                | J082954.3-073220 | 1527 4  | 1295 | 1640 | 14.93 | 0.18  | -17.01 | -18.54 | 2.27  | 12   |      |
| 438 | PGC2175402               | J083141.2+410454 | 581 29  | 581  | 878  | 17.74 | 0.16  | -12.82 | -16.92 | 2.94  | 09   |      |
| 439 | ESO431-018               | J083535.5-320845 | 1548 5  | 1250 | 1525 | 12.88 | 1.00  | -19.72 | -21.80 | 2.37  | 13   |      |
| 440 | ESO495-021               | J083615.2-262434 | 860 9   | 573  | 602  | 12.46 | 0.48  | -17.60 | -20.59 | 2.08  | 08   |      |
| 441 | ESO371-004               | J084014.4-325551 | 1397 14 | 1098 | 1369 | 16.32 | 1.25  | -16.29 | -19.84 | 4.34  | 13   |      |
| 442 | PGC081925                | J084203.2-331526 | 1788 47 | 1488 | 1757 | 16.07 | 1.50  | -17.34 | -21.31 | 2.86  | 13   |      |
| 443 | SDSS J084337.97+402546.9 | J084338.0+402547 | 622 1   | 616  | 914  | 17.80 | 0.14  | -12.83 | -15.18 | 2.76  | 12   |      |
| 444 | UGC04527                 | J084423.6+765501 | 720 4   | 901  | 1025 | 17.00 | 0.12  | -13.86 | -16.21 | 3.21  | 22   |      |
| 445 | HIZOA J0844-39           | J084444.2-395010 | 1813 14 | 1505 | 1746 | -     | 7.67  | -      | -      | 4.60  | 13   |      |
| 446 | HIZOA J0845-42           | J084521.7-421846 | 1748 14 | 1438 | 1667 | -     | 13.38 | -      | -      | 4.89  | 13   |      |
| 447 | HIPASS J0846-76          | J084624.1-765934 | 1516 5  | 1242 | 1277 | -     | 0.67  | -      | -      | 2.90  | 24   |      |
| 448 | HIPASS J0848-33          | J084903.4-330255 | 1316 9  | 1015 | 1285 | -     | 1.40  | -      | -      | 3.99  | 13   |      |
| 449 | PGC1013641               | J085201.4-074457 | 1556 45 | 1318 | 1659 | 15.68 | 0.16  | -16.26 | -18.23 | 2.56  | 12   |      |
| 450 | SDSS J085233.75+135028.3 | J085233.8+135028 | 1521 1  | 1374 | 1726 | 17.30 | 0.16  | -14.73 | -17.08 | 3.52  | 12   | ++   |
| 451 | SDSS J085240.94+135157.0 | J085240.9+135157 | 1565 22 | 1418 | 1770 | 19.71 | 0.16  | -12.38 | -14.72 | 3.83  | 12   | ++   |
| 452 | ESO371-027               | J085441.6-324859 | 1313 3  | 1011 | 1280 | 17.43 | 1.35  | -15.14 | -17.50 | 4.12  | 13   |      |
| 453 | ESO432-012               | J085515.8-320248 | 1473 30 | 1172 | 1445 | -     | 1.47  | -      | -      | 21.74 | 3.27 | 13   |
| 454 | ESO060-019               | J085726.7-690336 | 1443 3  | 1151 | 1233 | 12.80 | 0.43  | -18.77 | -20.92 | 2.16  | 13   |      |
| 455 | UGC04704                 | J085900.3+391235 | 602 3   | 587  | 886  | 15.13 | 0.13  | -15.42 | -18.02 | 2.98  | 12   | ++   |
| 456 | PGC2148839               | J085947.0+392304 | 588 34  | 573  | 886  | 17.34 | 0.11  | -13.19 | -15.54 | 2.98  | 12   | ++   |
| 457 | SDSS J0900+3222          | J090018.3+322236 | 730 4   | 678  | 972  | 18.97 | 0.14  | -11.77 | -      | 3.96  | 12   | +    |
| 458 | ESO371-030               | J090018.6-340449 | 1343 3  | 1039 | 1302 | 15.06 | 1.77  | -17.97 | -20.31 | 4.48  | 13   |      |
| 459 | PGC096431                | J090218.7-555657 | 1669 40 | 1358 | 1515 | 17.80 | 1.42  | -15.21 | -19.43 | 4.06  | 13   |      |
| 460 | NGC2788B                 | J090335.8-675811 | 1454 45 | 1159 | 1247 | 14.49 | 0.49  | -17.17 | -18.82 | 2.45  | 13   |      |
| 461 | HIPASS J0906-34          | J090656.9-341910 | 1410 8  | 1104 | 1365 | -     | 1.52  | -      | -      | 3.80  | 13   |      |
| 462 | ESO433-004               | J090719.9-321031 | 1465 5  | 1162 | 1431 | 16.60 | 1.06  | -15.92 | -18.77 | 2.91  | 13   |      |
| 463 | PGC2807128               | J090836.5+051728 | 595 1   | 406  | 756  | 17.03 | 0.19  | -13.23 | -15.59 | 3.06  | 12   |      |
| 464 | PGC1200328               | J090920.2+013651 | 1322 2  | 1118 | 1465 | 17.30 | 0.14  | -14.35 | -16.70 | 2.97  | 12   |      |
| 465 | ESO372-007               | J090929.9-332044 | 1133 5  | 829  | 1093 | 15.78 | 1.32  | -16.42 | -      | 2.13  | 13   |      |
| 466 | ESO372-008               | J091003.7-330915 | 1531 17 | 1226 | 1491 | 14.02 | 1.07  | -18.60 | -19.29 | 2.11  | 13   |      |
| 467 | HIZOA J0910-44           | J091047.2-442431 | 1875 14 | 1561 | 1776 | -     | 4.50  | -      | -      | 3.22  | 13   |      |
| 468 | PGC1954672               | J091159.4+313536 | 757 1   | 699  | 1017 | 18.14 | 0.07  | -12.65 | -15.00 | 4.11  | 12   |      |
| 469 | PGC026144                | J091604.9-090906 | 1671 4  | 1425 | 1757 | 14.58 | 0.16  | -17.49 | -18.94 | 2.25  | 14   |      |
| 470 | AGC198354                | J091630.9+091024 | 1295 5  | 1123 | 1470 | 18.96 | 0.17  | -12.73 | -      | 2.34  | 12   |      |
| 471 | SDSS J091858.62+581407.6 | J091858.6+581408 | 1167 2  | 1254 | 1473 | 17.35 | 0.13  | -14.30 | -16.65 | 2.25  | 12   |      |
| 472 | SDSS J092000.56+395333.2 | J092000.6+395333 | 1440 2  | 1426 | 1739 | 18.33 | 0.08  | -13.64 | -17.73 | 3.73  | 12   | ++   |
| 473 | PGC026453                | J092059.6+110333 | 1331 2  | 1167 | 1512 | 15.82 | 0.16  | -15.92 | -18.84 | 2.37  | 12   |      |
| 474 | NGC2844                  | J092147.9+400904 | 1478 8  | 1466 | 1737 | 13.69 | 0.08  | -18.28 | -21.95 | 3.71  | 12   | ++   |
| 475 | PGC026525                | J092213.4-074750 | 1701 5  | 1459 | 1791 | 15.62 | 0.16  | -16.49 | -19.09 | 2.17  | 14   |      |
| 476 | PGC960363                | J092217.0-115355 | 1558 10 | 1302 | 1626 | 18.00 | 0.16  | -13.90 | -15.34 | 4.11  | 14   |      |
| 477 | PGC970380                | J092806.3-110406 | 1744 41 | 1491 | 1815 | 15.90 | 0.18  | -16.26 | -19.54 | 2.35  | 14   |      |
| 478 | AGC198454                | J092811.3+073237 | 1373 4  | 1193 | 1535 | 18.82 | 0.22  | -13.01 | -      | 2.08  | 12   |      |
| 479 | PGC2369692               | J092837.4+501932 | 1509 8  | 1553 | 1805 | 17.32 | 0.08  | -14.73 | -17.08 | 4.23  | 12   |      |
| 480 | PGC1845056               | J092859.1+284529 | 1228 1  | 1154 | 1473 | 16.72 | 0.09  | -14.89 | -17.24 | 3.09  | 12   |      |
| 481 | SDSS J093136.15+271746.6 | J093136.1+271747 | 1511 3  | 1428 | 1750 | 17.99 | 0.08  | -13.99 | -16.33 | 2.27  | 12   |      |
| 482 | [MU2012] J09...          | J093359.7+551445 | 751 3   | 821  | 1328 | 19.73 | 0.14  | -11.57 | -14.06 | 2.12  | 12   | ++   |
| 483 | UGCA166                  | J093402.1+551426 | 747 2   | 817  | 1328 | 16.19 | 0.14  | -14.96 | -17.46 | 2.12  | 12   | ++   |
| 484 | PGC027228                | J093444.7+062532 | 546 2   | 360  | 699  | 15.27 | 0.18  | -14.82 | -17.17 | 2.60  | 08   |      |
| 485 | PGC082454                | J093550.5-053441 | 1496 6  | 1261 | 1591 | 16.54 | 0.14  | -15.29 | -18.43 | 3.60  | 14   |      |
| 486 | PGC2256640               | J094003.3+445932 | 1370 1  | 1383 | 1652 | 17.99 | 0.06  | -13.85 | -17.95 | 4.99  | 12   |      |
| 487 | PGC027612                | J094026.1-035308 | 1454 4  | 1225 | 1554 | 16.60 | 0.23  | -15.27 | -17.62 | 2.69  | 14   |      |
| 488 | PGC1084555               | J094101.8-024303 | 1633 6  | 1408 | 1739 | 16.93 | 0.15  | -15.10 | -17.70 | 3.44  | 14   |      |
| 489 | UGC05186                 | J094258.7+331556 | 555 4   | 504  | 807  | 16.21 | 0.06  | -14.07 | -16.41 | 2.44  | 12   | ++   |
| 490 | UGC05187                 | J094306.3+410535 | 1466 4  | 1458 | 1739 | 14.34 | 0.08  | -17.63 | -20.48 | 3.25  | 12   |      |
| 491 | AGC198691                | J094332.4+332658 | 514 6   | 464  | 766  | 19.82 | 0.06  | -10.35 | -12.70 | 2.15  | 12   | ++   |
| 492 | PGC2183147               | J094343.0+413409 | 1403 40 | 1398 | 1677 | 17.74 | 0.06  | -14.12 | -16.47 | 3.58  | 12   |      |
| 493 | PGC027864                | J094401.9-003832 | 1449 6  | 1233 | 1591 | 16.06 | 0.27  | -15.90 | -18.26 | 2.24  | 14   | ++   |
| 494 | UGC05205                 | J094407.2-003930 | 1503 4  | 1287 | 1591 | 15.61 | 0.27  | -16.35 | -18.70 | 2.24  | 14   | ++   |
| 495 | IC0559                   | J094443.8+093658 | 540 3   | 369  | 703  | 14.82 | 0.11  | -15.21 | -17.57 | 2.13  | 08   |      |
| 496 | UGC05209                 | J094504.2+321416 | 539 4   | 483  | 761  | 16.77 | 0.08  | -13.40 | -15.76 | 2.02  | 12   |      |
| 497 | PGC027949                | J094515.8+692325 | 571 4   | 714  | 873  | 16.90 | 0.32  | -13.81 | -16.16 | 2.49  | 22   |      |
| 498 | PGC2184302               | J094718.3+413816 | 1396 1  | 1392 | 1669 | 18.01 | 0.07  | -13.85 | -16.20 | 3.60  | 12   |      |
| 499 | PGC028153                | J094747.6+390503 | 1585 2  | 1566 | 1819 | 15.13 | 0.07  | -16.92 | -19.41 | 2.48  | 12   | ++   |
| 500 | PGC2800953               | J094750.3+390832 | 1553 23 | 1535 | 1819 | 16.80 | 0.07  | -15.25 | -17.60 | 2.51  | 12   | ++   |
| 501 | SDSS J094758.45+390510.1 | J094758.4+390510 | 1501 60 | 1483 | 1819 | 18.06 | 0.07  | -13.99 | -16.34 | 2.48  | 12   | ++   |

| (1) | (2)                     | (3)              | (4)      | (5)  | (6)  | (7)   | (8)   | (9)    | (10)   | (11) | (12) | (13) |
|-----|-------------------------|------------------|----------|------|------|-------|-------|--------|--------|------|------|------|
| 502 | PGC2807083              | J094801.0-543924 | 1736 7   | 1422 | 1575 | -     | 10.37 | -      | -      | 4.07 | 13   |      |
| 503 | PGC1314481              | J094805.9+070743 | 526 3    | 343  | 675  | 16.98 | 0.11  | -12.96 | -15.31 | 2.60 | 08   |      |
| 504 | PGC2807084              | J094943.0-563208 | 1760 6   | 1448 | 1591 | -     | 8.97  | -      | -      | 3.72 | 13   |      |
| 505 | PGC028305               | J095011.1+280046 | 1443 2   | 1364 | 1359 | 15.95 | 0.11  | -15.51 | -18.55 | 2.64 | 12   |      |
| 506 | PGC086265               | J095019.5+312722 | 536 1    | 475  | 772  | 17.73 | 0.09  | -12.48 | -14.83 | 2.01 | 12   | ++   |
| 507 | UGC05272                | J095022.4+312916 | 520 7    | 460  | 771  | 14.46 | 0.10  | -15.76 | -17.68 | 2.01 | 12   | ++   |
| 508 | NGC3026                 | J095055.3+283304 | 1480 4   | 1404 | 1359 | 13.85 | 0.09  | -17.59 | -20.65 | 2.70 | 12   |      |
| 509 | UGC05288                | J095117.2+074934 | 561 2    | 382  | 838  | 14.47 | 0.15  | -15.98 | -18.82 | 2.74 | 12   |      |
| 510 | SDSSJ095141.68+384207.1 | J095141.7+384207 | 1439 2   | 1419 | 1703 | 17.41 | 0.07  | -14.50 | -16.85 | 2.32 | 12   |      |
| 511 | NGC3032                 | J095208.2+291411 | 1541 6   | 1469 | 1359 | 13.07 | 0.07  | -18.35 | -21.65 | 2.80 | 12   | ++   |
| 512 | AGC190869               | J095241.9+292141 | 1459 6   | 1388 | 1359 | 17.60 | 0.08  | -13.83 | -      | 2.81 | 12   | ++   |
| 513 | UGC05332                | J095548.2+162449 | 805 1    | 667  | 991  | 16.73 | 0.14  | -14.07 | -16.42 | 3.89 | 12   |      |
| 514 | PGC028673               | J095614.8-293619 | 1839 60  | 1539 | 1798 | 16.16 | 0.40  | -16.19 | -18.65 | 3.93 | 14   |      |
| 515 | AGC749303               | J095633.2+271649 | 1073 4   | 991  | 1300 | 18.07 | 0.09  | -13.27 | -15.62 | 3.02 | 12   |      |
| 516 | DDO068C                 | J095641.1+290051 | 504 5    | 430  | 911  | -     | 0.08  | -      | -      | 3.00 | 12   | ++   |
| 517 | PGC3257044              | J095644.3-050827 | 1559 89  | 1326 | 1645 | 19.24 | 0.15  | -12.67 | -15.02 | 3.63 | 14   |      |
| 518 | UGC05340                | J095645.7+284933 | 510 2    | 436  | 911  | 14.77 | 0.08  | -15.79 | -17.67 | 3.00 | 12   | ++   |
| 519 | UGC05349                | J095806.1+371729 | 1377 5   | 1349 | 1634 | 14.46 | 0.06  | -17.35 | -18.41 | 2.13 | 12   |      |
| 520 | SDSSJ095816.17+210520.4 | J095816.2+210520 | 651 6    | 536  | 854  | 17.16 | 0.10  | -13.28 | -15.63 | 2.05 | 12   |      |
| 521 | UGC05354                | J095853.4+474413 | 1170 2   | 1199 | 1450 | 14.44 | 0.07  | -17.12 | -19.72 | 2.76 | 12   | ++   |
| 522 | PGC3095910              | J095918.7+473658 | 1100 1   | 1128 | 1380 | 17.05 | 0.06  | -14.40 | -16.75 | 2.89 | 12   | ++   |
| 523 | PGC029033               | J100138.2-081455 | 446 3    | 203  | 513  | 15.41 | 0.25  | -14.07 | -18.17 | 2.71 | 08   |      |
| 524 | PGC3098502              | J100223.2+294333 | 822 2    | 753  | 1054 | 17.30 | 0.10  | -13.59 | -15.95 | 3.05 | 12   |      |
| 525 | PGC2125269              | J100302.0+382238 | 1340 3   | 1318 | 1597 | 16.93 | 0.06  | -14.83 | -17.18 | 2.74 | 12   |      |
| 526 | PGC1230703              | J100425.1+023331 | 1126 2   | 924  | 1245 | 18.47 | 0.11  | -12.80 | -15.15 | 2.99 | 12   |      |
| 527 | UGC05453                | J100707.2+155903 | 846 4    | 706  | 1023 | 15.36 | 0.15  | -15.53 | -17.88 | 4.00 | 12   |      |
| 528 | UGC05464                | J100807.7+293233 | 1020 3   | 950  | 1248 | 15.64 | 0.09  | -15.61 | -18.02 | 3.30 | 12   |      |
| 529 | HIPASSJ1008-33          | J100829.3-330835 | 1643 6   | 1338 | 1578 | -     | 0.35  | -      | -      | 3.72 | 13   |      |
| 530 | PGC2278740              | J101015.0+461744 | 1099 1   | 1122 | 1372 | 18.32 | 0.03  | -13.08 | -17.19 | 3.02 | 12   |      |
| 531 | SDSSJ101259.87+394616.9 | J101259.9+394617 | 1340 6   | 1327 | 1597 | 18.33 | 0.06  | -13.43 | -14.33 | 3.03 | 12   |      |
| 532 | ESO263-021              | J101441.8-445116 | 1107 8   | 793  | 953  | 13.52 | 0.91  | -17.97 | -19.81 | 2.18 | 13   |      |
| 533 | PGC1046766              | J101509.3-051713 | 1332 39  | 1101 | 1406 | 16.78 | 0.17  | -14.81 | -17.16 | 3.04 | 14   |      |
| 534 | PGC2108569              | J101547.9+374459 | 1272 1   | 1247 | 1521 | 17.58 | 0.06  | -14.08 | -16.43 | 3.17 | 12   | ++   |
| 535 | UGC05540                | J101622.0+374647 | 1166 6   | 1142 | 1414 | 14.75 | 0.07  | -16.75 | -18.59 | 3.41 | 12   | ++   |
| 536 | PGC029998               | J101624.5+375446 | 1163 1   | 1140 | 1414 | 16.17 | 0.06  | -15.32 | -17.68 | 3.45 | 12   | ++   |
| 537 | ESO263-025              | J101627.3-455108 | 1918 8   | 1604 | 1787 | 15.73 | 0.87  | -17.08 | -19.43 | 2.18 | 13   |      |
| 538 | IC0600                  | J101710.9-032952 | 1308 2   | 1083 | 1350 | 13.75 | 0.15  | -17.74 | -19.60 | 2.95 | 14   |      |
| 539 | PGC030055               | J101733.0+430841 | 1132 2   | 1138 | 1395 | 16.74 | 0.07  | -14.73 | -17.08 | 3.86 | 12   |      |
| 540 | IC2563                  | J101851.9-323548 | 1354 9   | 1051 | 1286 | 15.51 | 0.32  | -16.04 | -18.89 | 3.51 | 13   |      |
| 541 | SDSSJ101928.52+292302.3 | J101928.5+292302 | 876 2    | 807  | 1098 | 17.46 | 0.14  | -13.56 | -15.91 | 3.15 | 12   |      |
| 542 | [CKT2009]D10...         | J101952.9+691119 | 557 38   | 700  | 852  | 18.50 | 0.15  | -11.99 | -14.34 | 2.39 | 22   |      |
| 543 | PGC2172303              | J102026.4+405241 | 1162 1   | 1155 | 1418 | 19.13 | 0.06  | -12.38 | -14.72 | 4.31 | 12   |      |
| 544 | PGC1178576              | J102138.9+005400 | 701 1    | 494  | 801  | 17.27 | 0.22  | -13.15 | -16.52 | 2.12 | 12   |      |
| 545 | ESO168-002              | J102445.2-544755 | 1080 7   | 769  | 907  | 15.70 | 2.79  | -17.56 | -20.96 | 2.32 | 13   |      |
| 546 | NGC3239                 | J102504.9+170949 | 752 4    | 621  | 925  | 11.68 | 0.14  | -18.97 | -19.79 | 2.41 | 12   |      |
| 547 | ESO037-015              | J102541.7-763014 | 1622 5   | 1347 | 1373 | 16.47 | 1.75  | -16.65 | -19.00 | 2.23 | 24   |      |
| 548 | PGC083029               | J102853.1-353252 | 1618 24  | 1313 | 1531 | 19.60 | 0.37  | -12.38 | -16.48 | 4.71 | 13   |      |
| 549 | PGC083049               | J102913.1-352915 | 1355 60  | 1050 | 1268 | 15.55 | 0.39  | -16.03 | -19.30 | 3.69 | 13   |      |
| 550 | ESO375-041              | J102931.0-351535 | 1749 31  | 1444 | 1676 | 14.68 | 0.43  | -17.56 | -21.22 | 2.96 | 13   | ++   |
| 551 | PGC030939               | J102953.0-352231 | 1776 28  | 1471 | 1675 | 15.64 | 0.42  | -16.58 | -20.66 | 2.97 | 13   | ++   |
| 552 | PGC083115               | J103018.3-351149 | 1749 52  | 1445 | 1676 | 16.22 | 0.44  | -16.03 | -19.40 | 2.96 | 13   | ++   |
| 553 | PGC030985               | J103023.8-351513 | 1192 43  | 887  | 1105 | 15.44 | 0.45  | -15.91 | -18.79 | 2.04 | 13   |      |
| 554 | PGC030981               | J103025.8-350629 | 1781 39  | 1476 | 1676 | 14.98 | 0.44  | -17.26 | -20.45 | 2.95 | 13   | ++   |
| 555 | UGC05723                | J103212.8-012936 | 1171 6   | 957  | 1253 | 15.09 | 0.24  | -16.09 | -20.03 | 2.66 | 14   |      |
| 556 | UGC05745                | J103444.8-015808 | 957 27   | 741  | 1036 | 13.76 | 0.25  | -17.25 | -21.33 | 2.57 | 12   |      |
| 557 | AGC208397               | J103858.1+035227 | 763 5    | 573  | 867  | 19.80 | 0.17  | -10.74 | -      | 2.00 | 12   |      |
| 558 | ABELL1084.15...         | J104117.3-063030 | 1727 68  | 1496 | 1779 | 19.32 | 0.22  | -12.83 | -      | 4.51 | 14   |      |
| 559 | ABELL1084.03...         | J104349.8-070210 | 1473 22  | 1240 | 1521 | 19.94 | 0.18  | -11.83 | -      | 4.66 | 14   |      |
| 560 | ESO502-020              | J110922.0-225231 | 1381 4   | 1108 | 1333 | 14.41 | 0.37  | -17.27 | -19.26 | 2.23 | 14   |      |
| 561 | ESO063-011              | J111307.9-691546 | 1329 4   | 1042 | 1091 | 14.20 | 0.96  | -17.63 | -20.33 | 2.22 | 24   | ++   |
| 562 | PGC2815815              | J111941.3-690514 | 1330 5   | 1043 | 1089 | 18.00 | 1.21  | -14.08 | -16.43 | 2.34 | 24   | ++   |
| 563 | ESO039-006              | J120913.4-752831 | 1916 6   | 1648 | 1652 | 15.62 | 1.52  | -17.67 | -20.39 | 2.23 | 15   |      |
| 564 | PGC2619398              | J121952.4+613111 | 516 4    | 643  | 769  | 18.03 | 0.08  | -12.16 | -14.51 | 3.58 | 22   |      |
| 565 | PGC039883               | J122100.2+124333 | 672 4    | 563  | 747  | 17.12 | 0.20  | -13.13 | -15.48 | 2.66 | 18   |      |
| 566 | UGC07490                | J122424.8+702002 | 466 3    | 631  | 733  | 13.42 | 0.11  | -16.70 | -19.08 | 2.71 | 22   |      |
| 567 | UGC07544                | J122638.0+622246 | 709 4    | 842  | 961  | 16.80 | 0.07  | -13.86 | -16.21 | 2.94 | 22   |      |
| 568 | ESO172-004              | J123101.8-550815 | 1715 5   | 1434 | 1490 | 14.46 | 1.90  | -18.99 | -21.02 | 3.03 | 15   |      |
| 569 | PGC041667               | J123307.9-003158 | 740 9    | 581  | 742  | 16.50 | 0.10  | -13.63 | -15.99 | 2.13 | 18   |      |
| 570 | UGC07748                | J123438.4+682025 | 460 1    | 619  | 721  | 15.66 | 0.07  | -14.38 | -16.93 | 2.93 | 22   |      |
| 571 | UGC07745                | J123438.4+734000 | 1187 3   | 1367 | 1436 | 17.00 | 0.09  | -14.56 | -16.91 | 2.46 | 17   | ++   |
| 572 | [RGK2003]J12...         | J123521.0+273347 | 1499 60  | 1470 | 1631 | 17.08 | 0.08  | -14.75 | -      | 3.06 | 16   |      |
| 573 | UGC07767                | J123532.5+734029 | 1148 52  | 1328 | 1436 | 13.76 | 0.09  | -17.80 | -21.24 | 2.47 | 17   | ++   |
| 574 | PGC091215               | J123655.0+013654 | 590 1    | 442  | 442  | 16.35 | 0.09  | -12.65 | -15.35 | 2.17 | 18   |      |
| 575 | ESO218-012              | J123947.5-521346 | 1809 60  | 1532 | 1588 | 16.89 | 0.82  | -15.62 | -17.97 | 3.43 | 15   |      |
| 576 | ESO172-006              | J124312.6-524749 | 1910 60  | 1634 | 1686 | 16.36 | 0.75  | -16.21 | -19.56 | 2.37 | 15   |      |
| 577 | PGC043010               | J124536.4+711907 | 1200 110 | 1373 | 1463 | 15.58 | 0.07  | -16.00 | -19.70 | 2.56 | 17   |      |
| 578 | AGC227970               | J124601.4+042252 | 643 4    | 513  | 672  | 16.00 | 0.11  | -13.93 | -      | 2.57 | 18   |      |
| 579 | ESO172-009              | J124732.9-535647 | 1869 6   | 1594 | 1623 | 14.05 | 1.14  | -18.82 | -19.74 | 3.24 | 15   | ++   |
| 580 | ESO172-010              | J124737.3-533300 | 1834 7   | 1559 | 1623 | 14.80 | 0.84  | -17.78 | -21.35 | 3.15 | 15   | ++   |
| 581 | UGC07979                | J124939.5+123731 | 791 17   | 700  | 845  | 15.27 | 0.17  | -15.22 | -16.10 | 2.70 | 18   |      |
| 582 | SDSSJ124942.06+052922.2 | J124942.1+052922 | 738 6    | 615  | 736  | 18.38 | 0.13  | -11.77 | -14.11 | 3.03 | 18   |      |
| 583 | UGC07983                | J124947.0+035033 | 694 2    | 565  | 735  | 16.11 | 0.18  | -14.08 | -16.43 | 2.77 | 18   |      |
| 584 | NGC4713                 | J124957.8+051841 | 651 2    | 528  | 667  | 12.21 | 0.12  | -17.72 | -20.06 | 2.72 | 18   | ++   |
| 585 | PGC1289726              | J124959.2+054916 | 618 1    | 497  | 667  | 16.76 | 0.13  | -13.17 | -15.53 | 2.80 | 18   | ++   |

| (1) | (2)                     | (3)              | (4)      | (5)  | (6)  | (7)   | (8)  | (9)    | (10)   | (11) | (12) | (13) |
|-----|-------------------------|------------------|----------|------|------|-------|------|--------|--------|------|------|------|
| 586 | PGC135809               | J125004.8-001357 | 754 6    | 608  | 745  | 17.69 | 0.10 | -12.45 | -14.80 | 2.23 | 18   |      |
| 587 | AGC227972               | J125024.0+045422 | 650 4    | 526  | 666  | 19.50 | 0.16 | -10.46 | -      | 2.66 | 18   |      |
| 588 | AGC227973               | J125039.9+052052 | 675 4    | 553  | 666  | 19.50 | 0.12 | -10.42 | -      | 2.73 | 18   |      |
| 589 | PGC086644               | J125146.0+214403 | 582 2    | 535  | 677  | 16.02 | 0.17 | -13.99 | -16.34 | 2.89 | 18   |      |
| 590 | AGC226122               | J125215.4+042727 | 700 4    | 575  | 732  | 18.33 | 0.18 | -11.86 | -      | 2.86 | 18   |      |
| 591 | PGC1264260              | J125343.3+040914 | 761 1    | 635  | 729  | 17.45 | 0.14 | -12.69 | -15.04 | 2.81 | 18   |      |
| 592 | SDSSJ125440.94+635324.9 | J125441.0+635325 | 563 2    | 710  | 808  | 18.61 | 0.07 | -11.68 | -14.02 | 3.97 | 22   |      |
| 593 | UGC08055                | J125604.5+034846 | 616 2    | 491  | 491  | 16.30 | 0.14 | -12.98 | -15.32 | 2.36 | 18   |      |
| 594 | PGC166151               | J125900.9+352848 | 704 32   | 728  | 857  | 17.51 | 0.04 | -12.84 | -15.23 | 2.12 | 20   |      |
| 595 | PGC044681               | J125956.6-192441 | 827 2    | 620  | 531  | 17.00 | 0.42 | -12.73 | -15.09 | 2.29 | 21   | +    |
| 596 | PGC044996               | J130222.8-492841 | 1799 60  | 1533 | 1578 | 15.56 | 0.92 | -17.03 | -19.38 | 3.47 | 15   | ++   |
| 597 | ESO219-022              | J130223.6-492824 | 1802 51  | 1536 | 1578 | 14.13 | 0.92 | -18.46 | -21.48 | 3.47 | 15   | ++   |
| 598 | PGC045058               | J130255.7+554140 | 1358 2   | 1474 | 1579 | 16.89 | 0.07 | -14.85 | -17.47 | 3.79 | 17   |      |
| 599 | SDSSJ130320.36+175909.7 | J130320.4+175910 | 964 17   | 907  | 1033 | 17.65 | 0.10 | -13.20 | -15.56 | 2.06 | 20   |      |
| 600 | SDSSJ130440.05+184438.7 | J130440.1+184439 | 920 1    | 867  | 992  | 17.71 | 0.11 | -13.07 | -15.42 | 2.26 | 20   |      |
| 601 | PGC045370               | J130623.2+102602 | 930 3    | 841  | 962  | 15.59 | 0.11 | -15.12 | -17.47 | 2.20 | 18   |      |
| 602 | PGC166153               | J130642.5+180008 | 1573 6   | 1518 | 1640 | 17.90 | 0.11 | -13.97 | -16.32 | 2.49 | 16   |      |
| 603 | PGC1614069              | J130828.4+200202 | 1484 2   | 1440 | 1560 | 17.72 | 0.12 | -14.05 | -16.39 | 3.20 | 16   |      |
| 604 | PGC2575228              | J131045.8+580925 | 1412 1   | 1541 | 1637 | 16.50 | 0.05 | -15.31 | -17.18 | 3.85 | 17   |      |
| 605 | UGC08276                | J131206.6+052833 | 912 2    | 806  | 916  | 16.35 | 0.16 | -14.30 | -14.25 | 2.03 | 18   |      |
| 606 | UGC08285                | J131233.3+071103 | 904 2    | 805  | 914  | 14.82 | 0.14 | -15.80 | -16.99 | 2.19 | 18   |      |
| 607 | AGC238737               | J131304.4+061707 | 892 5    | 790  | 898  | 18.09 | 0.18 | -12.54 | -      | 2.26 | 18   |      |
| 608 | UGC08333                | J131553.9+252608 | 938 2    | 924  | 1034 | 15.62 | 0.06 | -15.20 | -16.17 | 2.46 | 20   |      |
| 609 | PGC046161               | J131556.3+174538 | 974 1    | 924  | 1033 | 16.19 | 0.07 | -14.63 | -16.27 | 2.70 | 20   |      |
| 610 | AGC749463               | J131610.9+254015 | 1013 4   | 1000 | 1110 | 15.99 | 0.05 | -14.97 | -      | 2.91 | 20   |      |
| 611 | NGC5058                 | J131652.3+123254 | 968 2    | 896  | 1002 | 14.25 | 0.14 | -16.57 | -19.22 | 2.45 | 18   |      |
| 612 | SDSSJ131952.91+134825.5 | J131953.0+134824 | 937 4    | 873  | 975  | 18.58 | 0.11 | -12.16 | -13.80 | 2.81 | 18   |      |
| 613 | PGC722221               | J132014.0-300210 | 1670 39  | 1446 | 1504 | 16.07 | 0.30 | -15.80 | -18.15 | 2.88 | 19   |      |
| 614 | UGC08382                | J132032.1+052429 | 965 2    | 864  | 961  | 15.25 | 0.15 | -15.50 | -17.85 | 2.18 | 18   |      |
| 615 | PGC046578               | J132046.3+222342 | 1055 1   | 1030 | 1133 | 16.88 | 0.06 | -14.14 | -16.49 | 3.22 | 20   |      |
| 616 | PGC1700671              | J132104.8+240836 | 922 2    | 906  | 1009 | 16.87 | 0.04 | -13.87 | -16.22 | 2.36 | 20   |      |
| 617 | PGC2793496              | J132244.3-285712 | 990 5    | 771  | 828  | 15.63 | 0.31 | -14.95 | -17.31 | 4.15 | 21   |      |
| 618 | ESO444-029              | J132513.6-284655 | 1764 7   | 1547 | 1600 | 17.07 | 0.24 | -14.87 | -17.22 | 2.60 | 19   |      |
| 619 | AGC238691               | J132517.6+053236 | 989 5    | 893  | 983  | 17.78 | 0.14 | -13.01 | -      | 2.24 | 18   |      |
| 620 | UGC08441                | J132529.1+574919 | 1519 8   | 1653 | 1737 | 15.20 | 0.05 | -16.74 | -19.08 | 3.44 | 17   |      |
| 621 | PGC135827               | J132812.2+021642 | 1008 2   | 900  | 983  | 17.44 | 0.11 | -13.32 | -15.67 | 2.17 | 18   |      |
| 622 | UGC08509                | J132818.9+673754 | 992 4    | 1163 | 1236 | 16.66 | 0.06 | -14.54 | -16.89 | 5.02 | 17   |      |
| 623 | AGC239114               | J132834.4+330850 | 750 8    | 780  | 872  | 18.02 | 0.04 | -12.41 | -      | 2.37 | 20   |      |
| 624 | PGC135828               | J132955.7+013239 | 1047 1   | 937  | 1018 | 16.55 | 0.12 | -14.29 | -16.63 | 2.09 | 18   |      |
| 625 | AGC239115               | J133009.3+321715 | 746 8    | 773  | 864  | 18.01 | 0.04 | -12.40 | -      | 2.31 | 20   |      |
| 626 | UGC08507                | J133058.7+192611 | 997 2    | 966  | 1066 | 13.99 | 0.10 | -16.94 | -19.29 | 3.14 | 20   |      |
| 627 | UGC08516                | J133152.6+200004 | 1016 2   | 989  | 1065 | 13.95 | 0.13 | -17.00 | -19.85 | 3.27 | 20   |      |
| 628 | PGC047710               | J133305.9+685137 | 1500 110 | 1677 | 1746 | 16.48 | 0.08 | -15.50 | -18.27 | 3.05 | 17   |      |
| 629 | HIPASSJ1334-58          | J133400.6-585032 | 1458 8   | 1200 | 1198 | -     | 3.95 | -      | -      | 2.77 | 15   |      |
| 630 | PGC099542               | J133404.4-322136 | 1625 64  | 1405 | 1442 | 16.92 | 0.24 | -14.80 | -18.15 | 3.09 | 19   |      |
| 631 | PGC3097882              | J133436.5-291350 | 1347 60  | 1135 | 1176 | -     | 0.23 | -      | -      | 2.78 | 19   |      |
| 632 | UGC08578                | J133535.6+291301 | 851 1    | 868  | 952  | 15.28 | 0.05 | -15.34 | -17.27 | 2.53 | 20   |      |
| 633 | PGC1456087              | J133537.2+142140 | 1005 22  | 955  | 1035 | 17.64 | 0.13 | -13.25 | -17.35 | 2.28 | 20   |      |
| 634 | SDSSJ133625.55+181753.5 | J133625.5+181753 | 954 5    | 922  | 1002 | 17.97 | 0.12 | -12.84 | -15.19 | 3.29 | 20   |      |
| 635 | PGC706589               | J133658.9-311905 | 1691 8   | 1475 | 1510 | 16.73 | 0.22 | -15.06 | -18.41 | 3.61 | 19   |      |
| 636 | PGC048176               | J133808.0-305506 | 1684 58  | 1470 | 1504 | 15.47 | 0.24 | -16.34 | -18.67 | 3.52 | 19   |      |
| 637 | ESO444-088              | J133819.6-311827 | 1923 60  | 1709 | 1741 | 16.22 | 0.25 | -15.92 | -18.27 | 3.39 | 19   |      |
| 638 | PGC214132               | J133922.3+311458 | 704 1    | 732  | 811  | 16.97 | 0.08 | -13.34 | -15.69 | 2.64 | 20   | ++   |
| 639 | PGC169748               | J133931.6+392559 | 683 2    | 748  | 826  | 17.38 | 0.03 | -12.92 | -15.26 | 2.76 | 20   | ++   |
| 640 | PGC2807149              | J133945.0+390809 | 674 4    | 737  | 816  | 19.00 | 0.04 | -11.28 | -      | 2.70 | 20   | ++   |
| 641 | UGC08647                | J133947.9+311726 | 741 5    | 769  | 848  | 16.27 | 0.07 | -14.13 | -16.48 | 2.58 | 20   | ++   |
| 642 | ESO445-007              | J134021.4-314204 | 1657 3   | 1443 | 1472 | 16.65 | 0.24 | -15.12 | -17.46 | 3.66 | 19   |      |
| 643 | PGC2040056              | J134123.5+335130 | 1528 6   | 1570 | 1646 | 18.14 | 0.05 | -13.67 | -16.03 | 3.89 | 16   |      |
| 644 | SDSSJ134134.82+383144.9 | J134134.8+383145 | 1352 1   | 1414 | 1501 | 17.39 | 0.03 | -14.21 | -18.31 | 2.40 | 16   | ++   |
| 645 | UGC08667                | J134142.4+382957 | 1374 4   | 1435 | 1501 | 16.17 | 0.03 | -15.43 | -18.05 | 2.41 | 16   | ++   |
| 646 | PGC048501               | J134156.5+303110 | 958 3    | 984  | 1060 | 16.23 | 0.08 | -14.66 | -16.44 | 2.33 | 20   |      |
| 647 | PGC169750               | J134417.4+333929 | 1619 105 | 1661 | 1734 | 18.71 | 0.09 | -13.26 | -      | 4.32 | 16   |      |
| 648 | AGC238847               | J134509.7+272011 | 901 4    | 916  | 986  | 18.72 | 0.06 | -12.05 | -      | 3.11 | 20   |      |
| 649 | PGC048822               | J134628.1+210958 | 919 1    | 908  | 974  | 16.70 | 0.10 | -14.03 | -16.51 | 3.26 | 20   |      |
| 650 | SDSSJ134711.12+625006.2 | J134711.1+625006 | 1496 17  | 1657 | 1722 | 18.09 | 0.08 | -13.85 | -16.20 | 3.30 | 17   |      |
| 651 | PGC2123347              | J134722.1+381810 | 1339 1   | 1404 | 1539 | 16.94 | 0.06 | -14.74 | -18.84 | 2.51 | 16   | ++   |
| 652 | PGC166178               | J134736.7+331221 | 779 6    | 822  | 891  | 16.77 | 0.07 | -13.73 | -16.08 | 3.09 | 20   |      |
| 653 | NGC5303                 | J134745.0+381816 | 1412 7   | 1477 | 1538 | 12.86 | 0.06 | -18.82 | -21.33 | 2.49 | 16   | ++   |
| 654 | PGC048920               | J134745.5+381533 | 1405 1   | 1469 | 1538 | 15.36 | 0.06 | -16.31 | -18.71 | 2.49 | 16   | ++   |
| 655 | SDSSJ134757.44+041850.5 | J134757.4+041851 | 954 74   | 871  | 925  | 18.57 | 0.09 | -12.04 | -16.13 | 3.51 | 18   |      |
| 656 | ESO577-038              | J134825.6-185218 | 1889 3   | 1718 | 1751 | 16.58 | 0.39 | -15.71 | -18.59 | 3.32 | 19   |      |
| 657 | AGC239144               | J134908.2+354434 | 1366 8   | 1421 | 1488 | 19.06 | 0.05 | -12.54 | -      | 2.96 | 16   |      |
| 658 | PGC1672707              | J134913.6+223524 | 946 1    | 943  | 1007 | 16.89 | 0.07 | -13.87 | -16.65 | 3.53 | 20   |      |
| 659 | PGC1638331              | J135047.7+205354 | 869 1    | 860  | 920  | 16.77 | 0.12 | -13.85 | -16.20 | 3.18 | 20   |      |
| 660 | ESO384-002              | J135118.9-334828 | 1390 3   | 1178 | 1191 | 12.59 | 0.28 | -18.76 | -21.35 | 2.16 | 19   |      |
| 661 | ESO384-005              | J135216.1-372725 | 1641 3   | 1421 | 1429 | 15.41 | 0.33 | -16.38 | -19.00 | 2.81 | 19   |      |
| 662 | PGC872895               | J135221.1-180527 | 1586 39  | 1421 | 1449 | 16.84 | 0.35 | -15.00 | -17.35 | 2.08 | 19   |      |
| 663 | ESO325-034              | J135258.3-385038 | 1667 39  | 1445 | 1450 | 15.62 | 0.30 | -16.17 | -18.85 | 2.29 | 19   |      |
| 664 | NGC5338                 | J135326.5+051228 | 809 4    | 733  | 781  | 14.03 | 0.12 | -16.24 | -19.78 | 4.06 | 18   |      |
| 665 | PGC476604               | J135407.2-492750 | 1794 10  | 1555 | 1547 | 17.59 | 0.82 | -14.87 | -17.47 | 2.49 | 15   |      |
| 666 | PGC2807150              | J135433.5+041440 | 286 2    | 207  | 189  | 17.08 | 0.12 | -10.11 | -12.99 | 2.36 | 21   |      |
| 667 | UGC08839                | J135525.1+174742 | 955 2    | 935  | 988  | 15.88 | 0.11 | -14.88 | -17.23 | 3.50 | 20   |      |
| 668 | AGC233571               | J135741.0+152223 | 1257 2   | 1229 | 1277 | 16.79 | 0.10 | -14.52 | -16.88 | 2.83 | 16   |      |
| 669 | SDSSJ135749.50+421329.5 | J135749.5+421330 | 1369 4   | 1456 | 1514 | 16.65 | 0.03 | -14.96 | -15.61 | 2.03 | 16   |      |

| (1) | (2)                     | (3)              | (4)     | (5)  | (6)  | (7)   | (8)  | (9)    | (10)   | (11) | (12) | (13) |
|-----|-------------------------|------------------|---------|------|------|-------|------|--------|--------|------|------|------|
| 670 | VVDS140092139           | J135821.4+041901 | 869 60  | 794  | 833  | 23.30 | 0.13 | -7.12  | -      | 3.93 | 18   |      |
| 671 | PGC1453627              | J135843.4+141541 | 1288 3  | 1256 | 1301 | 17.45 | 0.08 | -13.89 | -16.24 | 2.89 | 16   |      |
| 672 | PGC1700854              | J135845.0+240905 | 971 1   | 982  | 1033 | 17.14 | 0.07 | -13.69 | -16.57 | 3.94 | 20   |      |
| 673 | NGC5398                 | J140121.6-330349 | 1219 3  | 1016 | 1017 | 14.08 | 0.28 | -16.92 | -20.18 | 2.70 | 21   |      |
| 674 | PGC2268822              | J140217.9+454053 | 766 35  | 870  | 924  | 17.53 | 0.04 | -13.02 | -15.37 | 3.10 | 20   |      |
| 675 | PGC050011               | J140236.1+391313 | 1326 1  | 1405 | 1456 | 17.15 | 0.07 | -14.42 | -16.78 | 2.07 | 16   |      |
| 676 | ESO510-052              | J140334.6-271647 | 1327 4  | 1142 | 1145 | 15.18 | 0.28 | -16.08 | -17.65 | 3.35 | 19   |      |
| 677 | PGC2325111              | J140344.7+484559 | 757 1   | 874  | 927  | 17.09 | 0.06 | -13.49 | -15.83 | 3.10 | 20   |      |
| 678 | PGC050212               | J140458.4+353634 | 865 1   | 930  | 977  | 17.13 | 0.05 | -13.55 | -16.52 | 3.22 | 20   |      |
| 679 | SDSSJ140749.40+464824.2 | J140749.4+464824 | 691 2   | 803  | 851  | 17.77 | 0.04 | -12.60 | -14.96 | 3.48 | 20   |      |
| 680 | PGC2167923              | J141329.9+403446 | 642 32  | 733  | 772  | 17.39 | 0.04 | -12.77 | -15.11 | 2.78 | 20   |      |
| 681 | NGC5510                 | J141337.2-175901 | 1438 1  | 1290 | 1288 | 14.49 | 0.38 | -17.12 | -20.00 | 2.66 | 19   |      |
| 682 | NGC5523                 | J141452.3+251903 | 1043 2  | 1072 | 1101 | 13.08 | 0.08 | -17.89 | -20.96 | 3.69 | 20   |      |
| 683 | HIZOA J1416-58B         | J141658.9-580810 | 1480 14 | 1241 | 1206 | -     | 7.92 | -      | -      | 2.69 | 15   |      |
| 684 | PGC051017               | J141702.0+433020 | 613 11  | 718  | 754  | 16.52 | 0.04 | -13.59 | -15.94 | 2.46 | 20   |      |
| 685 | SDSSJ141853.47+091728.7 | J141853.5+091729 | 1202 3  | 1166 | 1177 | 18.27 | 0.13 | -12.90 | -15.24 | 2.03 | 20   | ++   |
| 686 | UGC09169                | J141944.7+092145 | 1274 2  | 1238 | 1247 | 14.39 | 0.14 | -16.92 | -17.86 | 2.16 | 20   | ++   |
| 687 | PGC051225               | J142012.2+430111 | 635 1   | 740  | 773  | 17.69 | 0.05 | -12.48 | -14.83 | 3.22 | 20   |      |
| 688 | NGC5556                 | J142034.1-291430 | 1383 3  | 1205 | 1183 | 12.82 | 0.30 | -18.52 | -21.52 | 4.31 | 19   | ++   |
| 689 | SDSSJ142044.53+083735.8 | J142044.5+083736 | 1300 3  | 1262 | 1270 | 16.66 | 0.12 | -14.67 | -17.01 | 2.23 | 16   |      |
| 690 | PGC731537               | J142110.4-291504 | 1262 39 | 1084 | 1183 | 15.90 | 0.31 | -15.46 | -17.09 | 4.33 | 19   | ++   |
| 691 | UGC09193                | J142113.9+364437 | 710 7   | 791  | 819  | 17.00 | 0.03 | -13.28 | -15.63 | 3.68 | 20   |      |
| 692 | ESO446-053              | J142117.1-291548 | 1392 4  | 1214 | 1182 | 14.57 | 0.31 | -16.79 | -19.14 | 4.34 | 19   |      |
| 693 | PGC1107216              | J142212.2-015329 | 1021 5  | 941  | 938  | 17.93 | 0.20 | -12.81 | -15.16 | 4.42 | 18   |      |
| 694 | UGC09211                | J142232.3+452300 | 686 2   | 801  | 833  | 15.00 | 0.04 | -15.33 | -17.16 | 3.43 | 20   |      |
| 695 | NGC5608                 | J142318.0+414634 | 666 11  | 768  | 823  | 14.03 | 0.04 | -16.27 | -17.07 | 3.45 | 20   |      |
| 696 | SDSSJ142343.66+055236.6 | J142343.7+055237 | 1387 3  | 1340 | 1341 | 17.36 | 0.13 | -14.09 | -16.44 | 2.55 | 16   |      |
| 697 | UGC09225                | J142424.3+081634 | 1253 4  | 1217 | 1219 | 15.63 | 0.10 | -15.58 | -17.94 | 2.22 | 20   |      |
| 698 | PGC890565               | J142431.1-165918 | 1487 4  | 1352 | 1334 | 15.04 | 0.38 | -16.65 | -19.30 | 3.68 | 19   |      |
| 699 | UGC09249                | J142659.8+084101 | 1371 2  | 1339 | 1304 | 14.90 | 0.09 | -16.44 | -19.27 | 2.83 | 16   |      |
| 700 | UGC09274                | J142802.4+211812 | 1147 7  | 1169 | 1170 | 14.42 | 0.18 | -16.79 | -18.39 | 4.83 | 20   |      |
| 701 | UGC09273                | J142810.9+133306 | 1296 3  | 1285 | 1286 | 15.25 | 0.09 | -16.07 | -18.12 | 3.57 | 16   | ++   |
| 702 | IC1014                  | J142818.4+134649 | 1288 2  | 1278 | 1286 | 13.85 | 0.10 | -17.48 | -19.97 | 3.62 | 16   | ++   |
| 703 | PGC051694               | J142821.7+493341 | 670 3   | 804  | 832  | 15.78 | 0.08 | -14.59 | -16.94 | 3.48 | 20   |      |
| 704 | PGC3097720              | J142826.8-085524 | 1541 5  | 1439 | 1421 | -     | 0.25 | -      | -      | 4.15 | 19   |      |
| 705 | UGC09282                | J142841.5+212024 | 1134 4  | 1157 | 1169 | 15.79 | 0.19 | -15.42 | -17.77 | 4.87 | 20   |      |
| 706 | UGC09320                | J142958.4+365223 | 775 1   | 862  | 880  | 15.55 | 0.04 | -14.89 | -16.53 | 4.54 | 20   |      |
| 707 | SDSSJ143007.17+084216.0 | J143007.2+084216 | 1424 36 | 1395 | 1389 | 18.57 | 0.11 | -12.94 | -15.29 | 2.07 | 16   |      |
| 708 | PGC1069207              | J143011.3-033552 | 690 123 | 610  | 594  | 18.34 | 0.40 | -11.62 | -13.97 | 4.36 | 18   |      |
| 709 | NGC5645                 | J143039.4+071630 | 1366 1  | 1331 | 1322 | 12.90 | 0.12 | -18.51 | -21.61 | 2.63 | 16   | ++   |
| 710 | SDSSJ143048.66+070925.9 | J143048.7+070926 | 1365 4  | 1330 | 1322 | 18.10 | 0.11 | -13.30 | -15.65 | 2.63 | 16   | ++   |
| 711 | PGC1114278              | J143141.1-013729 | 1452 20 | 1381 | 1364 | 17.99 | 0.19 | -13.56 | -15.91 | 3.01 | 19   |      |
| 712 | SDSSJ143155.74+361820.8 | J143155.7+361821 | 787 1   | 873  | 888  | 19.52 | 0.05 | -10.95 | -13.30 | 4.70 | 20   |      |
| 713 | PGC051945               | J143220.8+095601 | 1399 6  | 1376 | 1369 | 15.57 | 0.12 | -15.92 | -18.54 | 2.46 | 16   | ++   |
| 714 | PGC051947               | J143226.1+231642 | 1149 8  | 1183 | 1186 | 15.58 | 0.14 | -15.62 | -17.97 | 4.69 | 20   |      |
| 715 | NGC5669                 | J143243.9+095329 | 1374 2  | 1352 | 1368 | 13.01 | 0.12 | -18.48 | -21.02 | 2.45 | 16   | ++   |
| 716 | PGC087128               | J143320.2+265952 | 832 2   | 882  | 886  | 15.50 | 0.07 | -14.99 | -17.34 | 4.85 | 20   |      |
| 717 | HIZOA J1434-55          | J143443.4-550537 | 2005 14 | 1779 | 1729 | -     | 3.17 | -      | -      | 4.80 | 15   |      |
| 718 | PGC3097721              | J143525.4-171001 | 1575 4  | 1448 | 1414 | -     | 0.32 | -      | -      | 4.99 | 19   |      |
| 719 | UGC09389                | J143533.3+125430 | 1833 4  | 1826 | 1812 | 14.55 | 0.11 | -17.54 | -19.68 | 3.66 | 16   | ++   |
| 720 | UGC09394                | J143539.9+131012 | 1776 6  | 1770 | 1813 | 15.01 | 0.10 | -17.06 | -18.57 | 3.77 | 16   | ++   |
| 721 | SDSSJ143619.44+473354.6 | J143619.4+473354 | 734 2   | 865  | 884  | 17.26 | 0.09 | -13.24 | -15.60 | 3.41 | 20   |      |
| 722 | PGC052212               | J143640.9+113437 | 1800 9  | 1788 | 1775 | 15.91 | 0.10 | -16.12 | -19.14 | 3.08 | 16   |      |
| 723 | PGC1344367              | J143701.3+081905 | 1712 2  | 1687 | 1670 | 17.17 | 0.11 | -14.74 | -18.84 | 2.40 | 16   |      |
| 724 | PGC052358               | J143905.5+364822 | 578 10  | 672  | 678  | 16.41 | 0.05 | -13.48 | -15.83 | 2.69 | 20   |      |
| 725 | PGC1360237              | J143912.5+090806 | 1763 2  | 1743 | 1724 | 16.58 | 0.14 | -15.43 | -17.78 | 2.30 | 16   |      |
| 726 | PGC2043836              | J144003.5+340600 | 1498 1  | 1582 | 1584 | 16.42 | 0.06 | -15.32 | -17.67 | 2.57 | 16   | ++   |
| 727 | SDSSJ144021.99+541328.5 | J144022.0+541329 | 624 4   | 780  | 801  | 18.11 | 0.07 | -12.16 | -16.26 | 3.40 | 20   |      |
| 728 | NGC5727                 | J144026.2+335920 | 1498 2  | 1582 | 1583 | 14.71 | 0.07 | -17.05 | -19.30 | 2.62 | 16   | ++   |
| 729 | AGC249590               | J144031.6+341601 | 1489 8  | 1574 | 1583 | 18.68 | 0.05 | -13.05 | -      | 2.54 | 16   | ++   |
| 730 | HIZOA J1441-55          | J144145.8-554138 | 2089 14 | 1865 | 1810 | -     | 3.41 | -      | -      | 5.09 | 15   |      |
| 731 | PGC2056934              | J144205.9+345618 | 1595 1  | 1683 | 1684 | 17.72 | 0.04 | -14.13 | -16.48 | 2.89 | 16   |      |
| 732 | SDSSJ144213.99+333517.4 | J144214.0+333518 | 1503 9  | 1586 | 1585 | 17.49 | 0.04 | -14.23 | -      | 2.82 | 16   |      |
| 733 | ESO386-013              | J144303.7-332930 | 1376 6  | 1202 | 1149 | 16.45 | 0.36 | -14.89 | -18.58 | 3.85 | 19   |      |
| 734 | PGC2053650              | J144330.1+344348 | 1682 1  | 1771 | 1769 | 17.55 | 0.05 | -14.43 | -16.78 | 3.77 | 16   |      |
| 735 | UGC09497                | J144412.8+423744 | 634 3   | 753  | 758  | 15.97 | 0.06 | -14.17 | -16.92 | 3.03 | 20   | ++   |
| 736 | PGC2801019              | J144444.2+553517 | 590 6   | 753  | 770  | 16.90 | 0.08 | -13.30 | -15.64 | 3.20 | 20   |      |
| 737 | SDSS                    | J144449.8+424254 | 634 3   | 753  | 794  | 19.69 | 0.05 | -10.54 | -      | 3.42 | 20   | ++   |
| 738 | AGC749485               | J144520.1+254151 | 1190 5  | 1244 | 1231 | 19.02 | 0.13 | -12.24 | -      | 4.89 | 16   |      |
| 739 | PGC2047492              | J144520.3+341948 | 1665 3  | 1754 | 1727 | 17.56 | 0.07 | -14.38 | -16.72 | 3.54 | 16   |      |
| 740 | UGC09500                | J144521.5+075144 | 1690 2  | 1671 | 1640 | 15.02 | 0.13 | -16.75 | -16.26 | 2.20 | 16   |      |
| 741 | UGC09504                | J144528.1+312559 | 1524 8  | 1601 | 1636 | 15.30 | 0.05 | -16.50 | -      | 3.80 | 16   | ++   |
| 742 | UGC09506                | J144532.5+312456 | 1500 10 | 1577 | 1581 | 16.77 | 0.06 | -14.97 | -16.37 | 3.65 | 16   | ++   |
| 743 | SDSSJ144533.59+315456.1 | J144533.6+315456 | 1208 15 | 1287 | 1280 | 17.92 | 0.05 | -13.35 | -      | 4.19 | 16   |      |
| 744 | SDSSJ144536.28+341043.8 | J144536.3+341044 | 1643 5  | 1731 | 1726 | 17.67 | 0.07 | -14.26 | -16.62 | 3.58 | 16   | ++   |
| 745 | UGC09519                | J144621.1+342214 | 1640 1  | 1730 | 1726 | 14.28 | 0.09 | -17.68 | -21.64 | 3.56 | 16   | ++   |
| 746 | PGC087175               | J144624.3+141245 | 1790 2  | 1798 | 1772 | 16.60 | 0.09 | -15.42 | -17.76 | 4.39 | 16   |      |
| 747 | PGC052819               | J144728.4+124554 | 1802 4  | 1805 | 1766 | 15.96 | 0.10 | -16.05 | -18.14 | 3.86 | 16   | ++   |
| 748 | PGC2081790              | J144744.6+363017 | 1226 2  | 1325 | 1319 | 18.04 | 0.05 | -13.29 | -15.64 | 4.11 | 16   |      |
| 749 | NGC5762                 | J144842.6+122726 | 1782 3  | 1785 | 1763 | 14.29 | 0.14 | -17.76 | -21.04 | 3.80 | 16   | ++   |
| 750 | PGC052893               | J144848.0-034259 | 932 4   | 868  | 823  | 15.06 | 0.46 | -15.66 | -18.00 | 5.34 | 18   |      |
| 751 | PGC200320               | J144852.0+344243 | 801 1   | 894  | 885  | 16.73 | 0.10 | -13.79 | -16.26 | 5.07 | 20   |      |
| 752 | PGC052903               | J144859.0+331135 | 1700 2  | 1787 | 1777 | 16.02 | 0.08 | -15.99 | -18.48 | 4.42 | 16   |      |
| 753 | SDSSJ144950.70+095630.0 | J144950.7+095630 | 1809 5  | 1802 | 1767 | 18.69 | 0.12 | -13.35 | -15.70 | 2.94 | 16   |      |

| (1) | (2)                     | (3)              | (4)     | (5)  | (6)  | (7)   | (8)   | (9)    | (10)   | (11) | (12) | (13) |
|-----|-------------------------|------------------|---------|------|------|-------|-------|--------|--------|------|------|------|
| 754 | PGC1393069              | J145022.6+112414 | 1779 1  | 1778 | 1744 | 16.87 | 0.11  | -15.13 | -17.48 | 3.52 | 16   |      |
| 755 | SDSSJ145053.09+341150.4 | J145053.1+341151 | 1208 2  | 1300 | 1289 | 18.20 | 0.09  | -13.13 | -15.48 | 4.37 | 16   |      |
| 756 | UGC09560                | J145056.6+353419 | 1188 9  | 1286 | 1276 | 14.76 | 0.05  | -16.50 | -18.43 | 4.25 | 16   | ++   |
| 757 | UGC09562                | J145114.4+353232 | 1275 4  | 1373 | 1362 | 14.44 | 0.06  | -16.98 | -19.17 | 3.89 | 16   | ++   |
| 758 | PGC1350028              | J145132.8+083600 | 1761 2  | 1750 | 1711 | 17.62 | 0.12  | -14.35 | -18.45 | 2.81 | 16   |      |
| 759 | SDSSJ145243.51+114019.9 | J145243.5+114020 | 1804 2  | 1807 | 1769 | 17.07 | 0.11  | -14.97 | -17.57 | 3.71 | 16   |      |
| 760 | PGC1427585              | J145254.3+131801 | 1842 1  | 1852 | 1816 | 17.93 | 0.11  | -14.16 | -16.50 | 4.35 | 16   |      |
| 761 | ESO386-029              | J145323.3-360512 | 1565 39 | 1391 | 1325 | 15.87 | 0.33  | -15.75 | -19.17 | 3.99 | 19   |      |
| 762 | UGC09597                | J145500.2+304929 | 1741 3  | 1824 | 1803 | 16.61 | 0.08  | -15.43 | -17.86 | 5.51 | 16   |      |
| 763 | PGC053410               | J145631.1+593541 | 533 2   | 713  | 726  | 15.90 | 0.03  | -14.12 | -15.68 | 3.22 | 20   |      |
| 764 | NGC5781                 | J145641.2-171438 | 1907 3  | 1799 | 1733 | 13.82 | 0.42  | -18.48 | -21.88 | 2.30 | 19   |      |
| 765 | PGC3089451              | J145739.4+263953 | 1276 1  | 1344 | 1315 | 15.98 | 0.18  | -15.48 | -17.65 | 5.73 | 16   |      |
| 766 | NGC5832                 | J145745.7+714057 | 447 3   | 656  | 682  | 13.57 | 0.12  | -16.40 | -19.57 | 4.16 | 22   |      |
| 767 | SDSSJ145801.75+364258.4 | J145801.8+364259 | 800 2   | 907  | 889  | 18.14 | 0.07  | -12.36 | -14.71 | 5.11 | 20   |      |
| 768 | ESO273-014              | J145830.3-474156 | 1052 3  | 853  | 781  | 12.88 | 1.32  | -18.58 | -20.47 | 2.42 | 21   |      |
| 769 | SDSSJ145901.96+441033.4 | J145902.0+441034 | 639 3   | 773  | 764  | 17.67 | 0.08  | -12.51 | -14.86 | 3.32 | 20   |      |
| 770 | PGC2249481              | J145938.3+444023 | 683 15  | 819  | 810  | 17.21 | 0.10  | -13.11 | -15.47 | 3.80 | 20   | ++   |
| 771 | UGC09660                | J150109.3+444153 | 600 10  | 738  | 786  | 14.42 | 0.10  | -15.84 | -18.25 | 3.57 | 20   | ++   |
| 772 | PGC2801020              | J150434.2-023513 | 1625 2  | 1580 | 1512 | 16.46 | 0.42  | -15.54 | -17.89 | 2.42 | 19   |      |
| 773 | HIPASSJ1506-40 **       | J150639.9-401702 | 1864 9  | 1689 | 1606 | 16.59 | 0.42  | -15.54 | -      | 3.00 | 21   | +    |
| 774 | HIPASSJ1506-49          | J150658.8-492450 | 1041 5  | 843  | 763  | -     | 1.45  | -      | -      | 2.85 | 21   |      |
| 775 | PGC1067957              | J150704.8-034202 | 1685 39 | 1639 | 1566 | 16.39 | 0.80  | -16.07 | -18.30 | 2.83 | 19   |      |
| 776 | UGC09739                | J150855.3+254401 | 1366 4  | 1440 | 1395 | 15.55 | 0.19  | -16.04 | -18.64 | 6.56 | 16   |      |
| 777 | PGC091421               | J151218.5+711556 | 1534 5  | 1747 | 1765 | 16.70 | 0.09  | -15.31 | -18.01 | 4.06 | 17   |      |
| 778 | SDSSJ151222.82+304855.5 | J151222.9+304855 | 1618 3  | 1714 | 1671 | 19.59 | 0.09  | -12.30 | -14.65 | 5.48 | 16   |      |
| 779 | ESO328-030              | J151228.0-423756 | 2064 11 | 1886 | 1797 | 14.26 | 0.48  | -18.18 | -20.01 | 3.50 | 21   |      |
| 780 | PGC1743738              | J151240.7+253802 | 1390 1  | 1467 | 1416 | 16.87 | 0.26  | -14.83 | -17.17 | 6.69 | 16   |      |
| 781 | HIPASSJ1516-58          | J151640.2-580847 | 1748 8  | 1537 | 1454 | -     | 11.94 | -      | -      | 4.32 | 15   |      |
| 782 | PGC054545               | J151701.7+394146 | 820 3   | 951  | 915  | 15.35 | 0.08  | -15.22 | -16.73 | 4.40 | 20   |      |
| 783 | SDSSJ151746.79+181053.2 | J151746.8+181053 | 1546 2  | 1598 | 1530 | 18.13 | 0.18  | -13.66 | -17.76 | 4.58 | 16   |      |
| 784 | PGC054607               | J151754.5+161844 | 721 4   | 765  | 695  | 16.10 | 0.13  | -13.92 | -16.28 | 5.73 | 20   |      |
| 785 | SDSSJ151832.11+310940.2 | J151832.1+310941 | 1656 3  | 1759 | 1708 | 17.27 | 0.09  | -14.66 | -17.01 | 5.96 | 16   |      |
| 786 | ESO328-043              | J151917.6-411401 | 1338 4  | 1168 | 1072 | 14.06 | 0.57  | -17.34 | -19.76 | 2.85 | 19   |      |
| 787 | PGC1405127              | J152059.5+121053 | 1167 2  | 1198 | 1119 | 17.32 | 0.21  | -13.81 | -16.16 | 3.15 | 20   |      |
| 788 | SDSSJ152255.55+420158.2 | J152255.5+420158 | 608 1   | 751  | 712  | 17.74 | 0.10  | -12.31 | -14.66 | 3.52 | 20   |      |
| 789 | PGC1744110              | J152753.1+253838 | 1471 1  | 1560 | 1489 | 18.44 | 0.22  | -13.33 | -17.43 | 6.57 | 16   |      |
| 790 | NGC5949                 | J152800.7+644547 | 428 10  | 633  | 632  | 12.87 | 0.10  | -16.92 | -20.22 | 3.49 | 22   |      |
| 791 | ESO274-016              | J152855.4-424701 | 1331 4  | 1164 | 1057 | 15.34 | 0.63  | -16.10 | -18.44 | 2.96 | 19   |      |
| 792 | UGC09893                | J153257.1+462709 | 653 3   | 816  | 775  | 15.35 | 0.06  | -14.84 | -17.49 | 4.10 | 20   |      |
| 793 | UGC09912                | J153510.3+163258 | 1031 1  | 1092 | 998  | 15.34 | 0.20  | -15.54 | -18.14 | 4.99 | 20   |      |
| 794 | NGC5961                 | J153515.8+305151 | 1770 18 | 1885 | 1789 | 14.48 | 0.12  | -17.59 | -21.16 | 6.61 | 16   | ++   |
| 795 | SDSSJ153545.34+310808.5 | J153545.4+310809 | 1692 52 | 1808 | 1789 | 18.38 | 0.12  | -13.69 | -16.03 | 6.73 | 16   | ++   |
| 796 | PGC1915372              | J153618.9+304333 | 1750 1  | 1865 | 1788 | 16.01 | 0.15  | -16.09 | -20.18 | 6.56 | 16   | ++   |
| 797 | PGC055576               | J153619.5+304056 | 1743 6  | 1858 | 1788 | 15.86 | 0.14  | -16.23 | -18.67 | 6.54 | 16   | ++   |
| 798 | PGC086658               | J153700.5+204745 | 1718 3  | 1797 | 1706 | 16.80 | 0.23  | -15.27 | -17.62 | 3.39 | 16   |      |
| 799 | SDSSJ153705.06+244644.2 | J153705.1+244644 | 1737 3  | 1831 | 1746 | 18.26 | 0.23  | -13.86 | -16.21 | 4.39 | 16   |      |
| 800 | SDSSJ153935.42+133959.6 | J153935.4+134000 | 932 20  | 985  | 881  | 17.00 | 0.20  | -13.61 | -17.71 | 5.52 | 20   |      |
| 801 | ABELL2104_03...         | J154010.0-031838 | 1132 24 | 1117 | 996  | 21.81 | 1.05  | -9.91  | -      | 3.79 | 21   |      |
| 802 | UGC09992                | J154147.9+671514 | 428 3   | 643  | 823  | 15.40 | 0.16  | -15.02 | -17.36 | 4.29 | 22   |      |
| 803 | NGC5984                 | J154253.4+141349 | 1092 8  | 1150 | 1042 | 13.28 | 0.19  | -17.68 | -20.57 | 4.55 | 20   |      |
| 804 | AGC258574               | J154507.9+014822 | 1523 6  | 1534 | 1409 | 17.50 | 0.35  | -13.31 | -      | 2.39 | 20   |      |
| 805 | UGC10014                | J154544.0+123038 | 1123 2  | 1177 | 1063 | 15.64 | 0.21  | -15.38 | -17.73 | 4.26 | 20   |      |
| 806 | PGC10023                | J154609.7+065354 | 1407 2  | 1439 | 1318 | 15.56 | 0.14  | -15.86 | -18.22 | 2.02 | 20   |      |
| 807 | UGC10025                | J154624.1+025039 | 1523 3  | 1539 | 1413 | 16.79 | 0.38  | -15.02 | -17.60 | 2.37 | 20   |      |
| 808 | PGC1001786              | J154807.0-083522 | 1866 39 | 1837 | 1701 | 16.29 | 0.65  | -16.20 | -17.76 | 4.22 | 19   |      |
| 809 | HIPASSJ1548-46          | J154848.0-465011 | 786 9   | 620  | 497  | -     | 2.60  | -      | -      | 3.60 | 21   |      |
| 810 | PGC2800435              | J155039.8-582600 | 2085 8  | 1890 | 1781 | 16.40 | 3.08  | -18.62 | -      | 7.94 | 21   |      |
| 811 | NGC6015                 | J155125.3+621836 | 832 3   | 1042 | 1020 | 11.61 | 0.05  | -19.17 | -21.97 | 2.02 | 22   |      |
| 812 | PGC056228               | J155128.1+640733 | 924 3   | 1138 | 1120 | 15.56 | 0.07  | -15.44 | -17.79 | 2.43 | 22   |      |
| 813 | UGC10090                | J155407.8+610606 | 627 4   | 837  | 810  | 17.00 | 0.05  | -13.27 | -15.67 | 3.94 | 22   |      |
| 814 | SDSSJ155701.55+300528.9 | J155701.6+300529 | 1716 1  | 1846 | 1745 | 17.72 | 0.16  | -14.34 | -16.69 | 6.61 | 16   |      |
| 815 | HIPASSJ1558-10          | J155820.0-103207 | 935 4   | 908  | 757  | 15.76 | 1.10  | -15.42 | -18.02 | 7.20 | 21   |      |
| 816 | PGC056622               | J155957.1+695946 | 989 90  | 1214 | 1207 | 15.59 | 0.12  | -15.62 | -17.28 | 3.89 | 22   |      |
| 817 | PGC056796               | J160227.9+642112 | 1594 19 | 1813 | 1789 | 15.63 | 0.09  | -16.41 | -18.70 | 6.01 | 17   |      |
| 818 | SDSSJ160247.91+065230.6 | J160247.9+065231 | 1451 1  | 1499 | 1354 | 18.33 | 0.22  | -13.23 | -17.33 | 3.32 | 20   |      |
| 819 | UGC10194                | J160403.8+634247 | 870 4   | 1088 | 1061 | 16.14 | 0.08  | -14.75 | -17.65 | 2.43 | 22   |      |
| 820 | UGC10175                | J160437.7+304253 | 801 4   | 939  | 830  | 15.85 | 0.14  | -14.57 | -16.91 | 6.42 | 20   |      |
| 821 | SDSSJ160549.93+411948.2 | J160549.9+411948 | 1667 28 | 1838 | 1751 | 18.16 | 0.04  | -13.78 | -16.14 | 8.25 | 16   |      |
| 822 | PGC057120               | J160602.1+083024 | 1370 2  | 1427 | 1279 | 16.11 | 0.24  | -15.35 | -17.82 | 3.67 | 20   |      |
| 823 | PGC160812               | J160705.2-112552 | 1809 39 | 1786 | 1623 | 15.79 | 1.26  | -17.20 | -20.21 | 4.52 | 19   |      |
| 824 | IC1197                  | J160817.3+073219 | 1364 3  | 1419 | 1267 | 14.35 | 0.21  | -17.06 | -20.12 | 3.79 | 20   |      |
| 825 | PGC1510033              | J160818.3+162927 | 1139 3  | 1229 | 1090 | 18.88 | 0.19  | -12.18 | -14.53 | 5.75 | 20   |      |
| 826 | PGC057323               | J160936.8-043716 | 830 6   | 837  | 673  | 15.30 | 1.03  | -15.55 | -18.18 | 6.64 | 18   |      |
| 827 | UGC10281                | J161320.5+171134 | 1085 2  | 1182 | 1037 | 17.00 | 0.26  | -14.02 | -16.37 | 6.32 | 20   |      |
| 828 | UGC10310                | J161617.9+470243 | 717 4   | 910  | 825  | 13.69 | 0.05  | -16.62 | -18.98 | 4.52 | 20   |      |
| 829 | IC1218                  | J161637.1+681209 | 1119 34 | 1348 | 1327 | 14.53 | 0.14  | -16.91 | -20.16 | 2.66 | 17   |      |
| 830 | PGC057723               | J161715.8-114354 | 977 3   | 962  | 785  | 12.72 | 1.30  | -18.74 | -20.35 | 7.63 | 21   |      |
| 831 | NGC6106                 | J161847.0+072434 | 1450 2  | 1514 | 1348 | 12.79 | 0.29  | -18.83 | -21.74 | 3.36 | 20   |      |
| 832 | NGC6140                 | J162057.8+652324 | 907 3   | 1135 | 1103 | 12.25 | 0.11  | -18.75 | -20.79 | 3.13 | 22   |      |
| 833 | UGC10351                | J162128.2+283823 | 892 1   | 1037 | 903  | 14.97 | 0.20  | -15.69 | -17.21 | 7.38 | 20   |      |
| 834 | UGC10369                | J162150.5+671735 | 1001 5  | 1230 | 1204 | 16.15 | 0.20  | -15.14 | -18.21 | 3.98 | 22   |      |
| 835 | PGC3078150              | J162158.1-575948 | 1404 5  | 1226 | 1093 | -     | 1.67  | -      | -      | 2.28 | 21   |      |
| 836 | HIPASSJ1624-47          | J162432.5-472254 | 1388 8  | 1243 | 1087 | -     | 12.85 | -      | -      | 3.49 | 21   |      |
| 837 | ESO137-027              | J162639.9-595714 | 1374 12 | 1193 | 1061 | 14.11 | 0.89  | -17.59 | -20.38 | 2.58 | 24   |      |

| (1) | (2)                     | (3)              | (4)     | (5)  | (6)  | (7)   | (8)   | (9)    | (10)   | (11)  | (12) | (13) |
|-----|-------------------------|------------------|---------|------|------|-------|-------|--------|--------|-------|------|------|
| 838 | UGC10445                | J163347.5+285904 | 960 2   | 1115 | 969  | 13.92 | 0.14  | -16.84 | -17.86 | 7.52  | 20   |      |
| 839 | SDSSJ163424.67+245741.4 | J163424.7+245742 | 1003 2  | 1146 | 990  | 18.30 | 0.18  | -12.54 | -14.89 | 8.45  | 20   |      |
| 840 | PGC3078543              | J163606.9-573246 | 818 8   | 648  | 504  | -     | 1.69  | -      | -      | 3.47  | 21   |      |
| 841 | UGC10477                | J163734.9+371710 | 872 1   | 1055 | 916  | 15.34 | 0.06  | -15.22 | -17.24 | 5.93  | 20   |      |
| 842 | SDSSJ164021.43+284555.9 | J164021.4+284556 | 977 2   | 1137 | 982  | 17.28 | 0.15  | -13.51 | -15.86 | 7.71  | 20   | ++   |
| 843 | PGC1836768              | J164022.2+282818 | 964 2   | 1123 | 967  | 17.47 | 0.16  | -13.30 | -15.65 | 7.76  | 20   | ++   |
| 844 | PGC165693               | J164302.7-204008 | 1203 5  | 1174 | 966  | 15.70 | 2.66  | -17.57 | -20.29 | 7.33  | 21   |      |
| 845 | NGC6207                 | J164303.7+364956 | 852 2   | 1037 | 909  | 11.86 | 0.07  | -18.69 | -21.28 | 6.15  | 20   |      |
| 846 | ESO179-013              | J164720.1-572626 | 839 7   | 675  | 523  | 12.70 | 1.18  | -17.76 | -18.51 | 3.21  | 21   |      |
| 847 | NGC6239                 | J165005.0+424423 | 926 4   | 1130 | 1014 | 12.89 | 0.08  | -17.90 | -20.57 | 5.10  | 20   | ++   |
| 848 | PGC2204813              | J165046.0+424321 | 944 1   | 1149 | 1013 | 16.60 | 0.08  | -14.19 | -16.54 | 5.12  | 20   | ++   |
| 849 | SDSSJ165254.34+360514.9 | J165254.4+360515 | 906 2   | 1097 | 948  | 17.66 | 0.07  | -12.98 | -15.32 | 6.46  | 20   | ++   |
| 850 | UGC10608                | J165421.7+530644 | 1089 4  | 1316 | 1221 | 15.48 | 0.28  | -15.92 | -18.52 | 4.44  | 22   |      |
| 851 | NGC6255                 | J165447.8+363005 | 917 8   | 1110 | 961  | 13.66 | 0.07  | -17.01 | -17.89 | 6.42  | 20   | ++   |
| 852 | PGC2801031              | J165638.5+075955 | 1473 4  | 1573 | 1360 | 17.00 | 0.53  | -14.88 | -17.23 | 4.03  | 20   |      |
| 853 | PGC1751005              | J165816.1+254902 | 709 1   | 873  | 692  | 17.67 | 0.27  | -12.48 | -16.58 | 6.73  | 20   |      |
| 854 | NGC6283                 | J165926.5+495519 | 1093 36 | 1317 | 1207 | 13.83 | 0.09  | -17.36 | -20.00 | 4.88  | 22   |      |
| 855 | HIPASSJ1700-12          | J170006.3-120001 | 1298 5  | 1320 | 1089 | 16.70 | 1.24  | -15.41 | -      | 4.88  | 21   |      |
| 856 | UGC10669                | J170026.2+701727 | 442 2   | 686  | 652  | 17.00 | 0.15  | -12.91 | -15.26 | 3.87  | 22   |      |
| 857 | PGC059579               | J170512.3+672512 | 1109 60 | 1353 | 1307 | 16.91 | 0.16  | -14.51 | -17.92 | 2.57  | 22   |      |
| 858 | SDSSJ170517.35+355222.0 | J170517.4+355222 | 992 1   | 1190 | 1029 | 17.07 | 0.10  | -13.78 | -16.13 | 6.89  | 20   |      |
| 859 | UGC10736                | J170804.7+692751 | 491 3   | 737  | 697  | 14.86 | 0.15  | -15.19 | -17.79 | 4.27  | 22   |      |
| 860 | HIPASSJ1707-60 **       | J170826.2-605138 | 1810 8  | 1644 | 1490 | 18.45 | 0.62  | -13.72 | -      | 3.55  | 24   | +    |
| 861 | PGC2801034              | J171242.1+135428 | 1502 4  | 1638 | 1416 | 17.80 | 0.67  | -14.31 | -16.66 | 3.48  | 20   |      |
| 862 | PGC059804               | J171307.0+591924 | 1028 74 | 1271 | 1187 | 16.14 | 0.10  | -15.02 | -      | 4.51  | 22   | ++   |
| 863 | PGC059862               | J171310.3+591956 | 1157 31 | 1400 | 1317 | 15.38 | 0.10  | -16.00 | -18.35 | 4.67  | 22   | ++   |
| 864 | UGC10806                | J171851.4+495303 | 928 3   | 1163 | 1084 | 13.92 | 0.11  | -17.05 | -19.09 | 4.97  | 22   | ++   |
| 865 | PGC167108               | J171907.7+495122 | 1019 42 | 1254 | 1084 | 17.50 | 0.10  | -13.46 | -15.81 | 4.99  | 22   | ++   |
| 866 | UGC10805                | J171951.1+142400 | 1554 2  | 1697 | 1468 | 15.61 | 0.50  | -16.41 | -18.81 | 3.07  | 20   |      |
| 867 | IC4653                  | J172707.0-605248 | 1899 32 | 1742 | 1577 | 13.23 | 0.36  | -18.80 | -21.51 | 4.89  | 24   |      |
| 868 | PGC084875               | J173637.3+633502 | 1200 42 | 1454 | 1377 | 15.96 | 0.11  | -15.53 | -18.41 | 3.23  | 22   |      |
| 869 | HIPASSJ1738-57          | J173842.9-571525 | 858 8   | 718  | 534  | 16.62 | 0.42  | -13.12 | -      | 2.65  | 21   |      |
| 870 | UGC10974                | J174414.8+673710 | 1462 10 | 1719 | 1658 | 15.14 | 0.21  | -16.85 | -20.66 | 3.09  | 23   | ++   |
| 871 | UGC10991                | J174629.6+672017 | 1463 2  | 1721 | 1656 | 16.14 | 0.22  | -15.85 | -18.20 | 3.18  | 23   | ++   |
| 872 | NGC6503                 | J174926.5+700840 | 39 13   | 297  | 458  | 10.86 | 0.14  | -18.27 | -21.53 | 2.25  | 22   | ++   |
| 873 | UGC11000                | J174926.6+360843 | 1369 1  | 1598 | 1400 | 14.12 | 0.17  | -17.46 | -20.06 | 10.42 | 23   |      |
| 874 | KK242                   | J175248.0+700815 | 426 9   | 685  | 632  | 18.50 | 0.15  | -11.34 | -13.19 | 3.18  | 22   | ++   |
| 875 | NGC6542                 | J175938.6+612134 | 697 9   | 960  | 862  | 14.17 | 0.13  | -16.32 | -19.19 | 5.70  | 22   |      |
| 876 | PGC061243               | J175946.2+364032 | 1436 21 | 1672 | 1468 | 15.44 | 0.17  | -16.25 | -18.78 | 10.84 | 23   |      |
| 877 | UGC11109                | J180414.1+464415 | 1565 8  | 1820 | 1653 | 17.00 | 0.19  | -14.96 | -17.31 | 10.05 | 23   |      |
| 878 | UGC11124                | J180727.5+353350 | 1608 2  | 1847 | 1556 | 13.79 | 0.17  | -18.03 | -19.90 | 10.87 | 23   | ++   |
| 879 | PGC3088568              | J180729.0+353726 | 1530 60 | 1769 | 1556 | 16.54 | 0.17  | -15.27 | -17.62 | 10.89 | 23   | ++   |
| 880 | PGC5065941              | J180745.0+352330 | 1490 60 | 1729 | 1555 | -     | 0.17  | -      | -      | 10.81 | 23   | ++   |
| 881 | PGC2801040              | J181052.1+371453 | 1510 6  | 1754 | 1545 | 17.70 | 0.20  | -14.13 | -16.48 | 11.48 | 23   |      |
| 882 | HIPASSJ1812-21          | J181221.6-213359 | 1529 6  | 1565 | 1270 | -     | 16.77 | -      | -      | 6.67  | 21   |      |
| 883 | PGC061812               | J182306.2-774317 | 1350 66 | 1152 | 1041 | 15.93 | 0.69  | -15.53 | -18.97 | 4.70  | 24   |      |
| 884 | UGC11220                | J182325.6+405642 | 1449 2  | 1706 | 1504 | 16.47 | 0.20  | -15.30 | -17.12 | 11.39 | 23   |      |
| 885 | IC4710                  | J182838.0-665856 | 739 4   | 580  | 539  | 12.51 | 0.38  | -17.21 | -17.25 | 2.04  | 21   |      |
| 886 | PGC166900               | J182859.8+064828 | 1234 50 | 1403 | 1098 | 14.87 | 1.29  | -17.31 | -21.51 | 7.37  | 21   |      |
| 887 | NGC6630                 | J183235.2-631736 | 1818 32 | 1675 | 1492 | 14.60 | 0.47  | -17.43 | -20.50 | 3.94  | 24   |      |
| 888 | NGC6689                 | J183450.3+703126 | 489 3   | 757  | 695  | 13.05 | 0.30  | -17.14 | -19.78 | 3.57  | 22   |      |
| 889 | HIPASSJ1838-22          | J183836.0-224825 | 1656 7  | 1703 | 1391 | -     | 1.35  | -      | -      | 6.44  | 21   |      |
| 890 | HIPASSJ1841-18          | J184106.4-185956 | 1672 5  | 1739 | 1421 | -     | 2.03  | -      | -      | 5.78  | 21   |      |
| 891 | PGC3097195              | J185555.0-031326 | 1580 4  | 1727 | 1395 | -     | 6.35  | -      | -      | 4.42  | 21   |      |
| 892 | PGC3097196              | J190148.0-042951 | 1531 4  | 1676 | 1341 | -     | 3.46  | -      | -      | 3.72  | 21   |      |
| 893 | IC4819                  | J190706.5-592757 | 1842 4  | 1725 | 1515 | 14.26 | 0.26  | -17.58 | -21.04 | 2.19  | 24   |      |
| 894 | PGC203488               | J190800.5-154833 | 1742 39 | 1839 | 1503 | 16.75 | 0.63  | -15.45 | -18.80 | 4.18  | 21   |      |
| 895 | 6dFJ1913...             | J191349.2-154921 | 1744 39 | 1845 | 1507 | 18.20 | 0.56  | -13.93 | -16.28 | 3.88  | 21   |      |
| 896 | HIZOAJ1914+10           | J191502.5+101944 | 655 6   | 865  | 539  | -     | 52.11 | -      | -      | 6.08  | 21   |      |
| 897 | HIPASSJ1916-31          | J191638.4-315124 | 2019 7  | 2042 | 1729 | 14.08 | 0.46  | -18.26 | -21.18 | 9.03  | 21   |      |
| 898 | NGC6789                 | J191641.6+635820 | -167 2  | 118  | 259  | 13.82 | 0.29  | -14.22 | -16.67 | 2.55  | 21   |      |
| 899 | HIPASSJ1919-33          | J191932.8-334602 | 2077 5  | 2092 | 1783 | -     | 0.40  | -      | -      | 9.97  | 21   |      |
| 900 | ESO525-005              | J192645.1-272514 | 1944 6  | 1995 | 1668 | 16.50 | 0.38  | -15.67 | -18.03 | 6.94  | 21   |      |
| 901 | PGC204430               | J193314.8-003710 | 1434 6  | 1612 | 1266 | 17.52 | 1.10  | -14.77 | -17.12 | 3.19  | 21   |      |
| 902 | UGC11458                | J193506.8+695942 | 1370 8  | 1651 | 1576 | 17.00 | 0.77  | -15.44 | -17.79 | 2.72  | 22   |      |
| 903 | IC4869                  | J193602.3-610140 | 1793 4  | 1677 | 1469 | 13.70 | 0.35  | -18.17 | -19.22 | 2.13  | 24   | ++   |
| 904 | ESO142-026              | J193847.5-610943 | 1735 6  | 1619 | 1411 | 15.44 | 0.35  | -16.34 | -18.94 | 2.86  | 24   | ++   |
| 905 | HIPASSJ1940+00          | J194026.0+004006 | 1305 8  | 1492 | 1144 | -     | 1.59  | -      | -      | 4.07  | 21   |      |
| 906 | HIZOAJ1940+11           | J194036.0+115418 | 580 14  | 808  | 477  | -     | 1.87  | -      | -      | 5.53  | 21   |      |
| 907 | ESO594-011              | J194042.4-221614 | 1796 45 | 1878 | 1538 | 16.30 | 0.41  | -15.73 | -20.01 | 4.05  | 21   |      |
| 908 | PGC063536               | J194157.4-290318 | 1982 32 | 2030 | 1703 | 14.30 | 0.56  | -18.10 | -21.26 | 7.42  | 21   |      |
| 909 | UGC11466                | J194258.8+451753 | 820 6   | 1116 | 903  | 13.52 | 0.73  | -17.67 | -21.02 | 4.68  | 22   |      |
| 910 | PGC063566               | J194326.0-011032 | 1418 6  | 1599 | 1249 | 15.76 | 1.13  | -16.54 | -21.06 | 2.99  | 21   |      |
| 911 | ESO460-034              | J194453.3-281123 | 1986 3  | 2040 | 1711 | 16.07 | 0.80  | -16.58 | -18.93 | 7.20  | 21   |      |
| 912 | ESO594-017              | J194822.0-180442 | 1739 9  | 1846 | 1498 | 14.77 | 0.60  | -17.39 | -19.20 | 2.38  | 21   |      |
| 913 | UGC11484                | J194834.7+541212 | 1303 12 | 1602 | 1434 | 16.25 | 0.80  | -16.01 | -18.61 | 5.46  | 23   |      |
| 914 | PGC205272               | J195157.3+013140 | 1274 8  | 1469 | 1120 | 17.64 | 1.01  | -14.30 | -16.90 | 4.49  | 21   |      |
| 915 | ALFAZOAJ1952...         | J195211.8+142824 | 279 6   | 521  | 613  | 17.20 | 1.12  | -13.54 | -15.89 | 4.52  | 21   |      |
| 916 | PGC2801045              | J200054.4+421726 | 785 9   | 1085 | 855  | 17.70 | 2.31  | -14.95 | -17.30 | 3.56  | 22   |      |
| 917 | ESO461-036              | J200357.4-314054 | 431 6   | 474  | 517  | 17.07 | 1.31  | -13.49 | -16.06 | 5.20  | 21   |      |
| 918 | NGC6868:[CMI...         | J200846.8-482200 | 1052 68 | 1008 | 739  | -     | 0.22  | -      | -      | 3.05  | 21   |      |
| 919 | PGC064176               | J200921.2-061715 | 1424 2  | 1594 | 1238 | 15.30 | 0.34  | -16.19 | -20.43 | 2.65  | 25   |      |
| 920 | IC4951                  | J200931.8-615101 | 814 3   | 701  | 493  | 14.03 | 0.17  | -15.29 | -17.96 | 2.80  | 02   |      |
| 921 | PGC1065381              | J201243.2-035421 | 1343 6  | 1525 | 1169 | 16.56 | 1.33  | -15.79 | -17.95 | 3.62  | 25   |      |



| (1)  | (2)           | (3)              | (4)      | (5)  | (6)  | (7)   | (8)   | (9)    | (10)   | (11) | (12) | (13) |
|------|---------------|------------------|----------|------|------|-------|-------|--------|--------|------|------|------|
| 922  | PGC4126690    | J201632.8+071627 | 1841 10  | 2068 | 1723 | -     | 0.86  | -      | -      | 8.78 | 21   |      |
| 923  | PGC1052018    | J202031.8-045358 | 1384 5   | 1563 | 1207 | 16.11 | 0.33  | -15.31 | -17.66 | 3.65 | 25   |      |
| 924  | UGC11557      | J202400.7+601141 | 1388 3   | 1691 | 1555 | 14.39 | 1.02  | -18.27 | -20.92 | 2.48 | 22   |      |
| 925  | PGC408791     | J202608.8-552950 | 893 67   | 815  | 547  | 16.88 | 0.22  | -12.71 | -15.62 | 2.64 | 21   | ++   |
| 926  | PGC064718     | J202733.8-550525 | 831 52   | 756  | 545  | 15.24 | 0.24  | -14.37 | -18.02 | 2.70 | 21   | ++   |
| 927  | UGC11566      | J202812.0+001718 | 1671 35  | 1875 | 1521 | 14.19 | 0.59  | -18.00 | -20.66 | 5.58 | 25   |      |
| 928  | PGC2801049    | J203558.8-011859 | 1730 7   | 1929 | 1575 | 17.10 | 0.52  | -15.09 | -17.44 | 5.89 | 25   |      |
| 929  | PGC329372     | J203857.3-634615 | 1655 4   | 1537 | 1340 | 15.98 | 0.29  | -15.63 | -17.72 | 3.78 | 24   |      |
| 930  | IC5028        | J204322.1-653852 | 1624 5   | 1497 | 1310 | 15.23 | 0.21  | -16.25 | -18.60 | 3.60 | 24   |      |
| 931  | PGC3093573    | J204523.1-123708 | 1074 45  | 1225 | 871  | 16.45 | 0.19  | -14.12 | -17.68 | 7.37 | 21   |      |
| 932  | PGC065330     | J204540.1+281038 | 1099 4   | 1392 | 1103 | 15.74 | 1.20  | -16.35 | -18.71 | 4.29 | 23   |      |
| 933  | PGC162688     | J204847.3-121654 | 843 45   | 997  | 643  | 17.12 | 0.21  | -12.82 | -17.09 | 6.83 | 21   |      |
| 934  | 6dFJ2049...   | J204940.0-324154 | 1742 64  | 1791 | 1471 | 17.66 | 0.30  | -14.16 | -18.26 | 7.54 | 21   |      |
| 935  | IC5052        | J205204.5-691200 | 589 2    | 445  | 424  | 11.67 | 0.22  | -17.37 | -19.94 | 3.62 | 02   |      |
| 936  | 2MASXJ2054... | J205436.0-542656 | 1993 34  | 1925 | 1684 | 16.50 | 0.16  | -15.48 | -18.16 | 3.29 | 21   |      |
| 937  | PGC897218     | J205651.6-163031 | 1452 5   | 1587 | 1238 | 15.85 | 0.24  | -15.54 | -16.39 | 5.38 | 25   |      |
| 938  | UGC11651      | J205715.4+255754 | 1525 1   | 1815 | 1521 | 15.55 | 1.18  | -17.22 | -21.83 | 5.81 | 23   |      |
| 939  | IC5078        | J210231.2-164905 | 1474 2   | 1607 | 1261 | 13.52 | 0.32  | -17.98 | -21.27 | 5.71 | 25   |      |
| 940  | PGC1133627    | J210347.2-004950 | 1411 1   | 1618 | 1269 | 17.44 | 0.31  | -14.07 | -16.42 | 6.84 | 25   | ++   |
| 941  | PGC1139658    | J210455.3-003522 | 1395 1   | 1604 | 1256 | 18.23 | 0.28  | -13.23 | -15.58 | 6.97 | 25   | ++   |
| 942  | PGC2807212    | J210537.3+270911 | 943 10   | 1237 | 948  | 18.10 | 1.05  | -13.52 | -15.87 | 2.15 | 25   |      |
| 943  | ESO187-051    | J210732.8-545709 | 1401 8   | 1331 | 1095 | 14.91 | 0.15  | -16.12 | -18.47 | 4.91 | 24   |      |
| 944  | PGC129680     | J210804.9-471942 | 860 33   | 832  | 563  | 15.69 | 0.15  | -13.90 | -17.24 | 3.79 | 21   |      |
| 945  | PGC066199     | J210856.3+445116 | 1650 60  | 1964 | 1751 | 17.54 | 5.59  | -19.95 | -21.98 | 7.94 | 23   |      |
| 946  | PGC3317929    | J211052.5-340150 | 1769 123 | 1814 | 1501 | 19.52 | 0.37  | -12.42 | -14.76 | 6.15 | 21   |      |
| 947  | PGC066336     | J211216.0+453115 | 700 60   | 1015 | 805  | 16.43 | 3.51  | -17.29 | -20.22 | 3.00 | 22   |      |
| 948  | PGC140953     | J211330.6+464227 | 805 60   | 1120 | 917  | -     | 7.34  | -      | -      | 3.81 | 22   |      |
| 949  | PGC892359     | J211449.1-165210 | 1466 39  | 1601 | 1258 | 15.84 | 0.32  | -15.67 | -17.93 | 5.29 | 25   |      |
| 950  | ESO107-016    | J211606.0-644900 | 1796 11  | 1675 | 1487 | 15.09 | 0.19  | -16.64 | -19.42 | 2.28 | 24   |      |
| 951  | PGC2801054    | J211842.0+261737 | 919 6    | 1213 | 925  | 16.90 | 0.47  | -14.09 | -16.43 | 2.02 | 25   | ++   |
| 952  | PGC066548     | J211858.9+252551 | 935 4    | 1227 | 937  | 15.00 | 0.52  | -16.06 | -19.47 | 2.23 | 25   | ++   |
| 953  | PGC066571     | J212006.0+115507 | 1147 1   | 1403 | 1077 | 16.54 | 0.37  | -14.68 | -17.00 | 5.58 | 25   |      |
| 954  | PGC163084     | J212020.1-574549 | 1263 114 | 1179 | 957  | 16.66 | 0.21  | -14.13 | -18.48 | 4.95 | 24   |      |
| 955  | PGC188521     | J212130.3-490343 | 1701 48  | 1664 | 1405 | 16.52 | 0.18  | -15.08 | -18.57 | 3.47 | 21   |      |
| 956  | PGC066699     | J212436.0-640500 | 1798 57  | 1681 | 1478 | 16.26 | 0.15  | -15.42 | -17.77 | 2.10 | 24   |      |
| 957  | NGC7059       | J212721.5-600052 | 1734 4   | 1639 | 1429 | 12.49 | 0.14  | -19.11 | -21.86 | 2.05 | 24   |      |
| 958  | PGC2802329    | J212739.6+531045 | 1040 12  | 1354 | 1188 | -     | 11.14 | -      | -      | 2.43 | 22   |      |
| 959  | ESO530-051    | J212744.1-234005 | 1860 12  | 1961 | 1632 | 15.51 | 0.17  | -16.40 | -18.88 | 4.97 | 21   |      |
| 960  | NGC7064       | J212903.0-524603 | 803 31   | 746  | 505  | 12.71 | 0.06  | -16.55 | -18.35 | 3.83 | 02   |      |
| 961  | NGC7077       | J212959.6+022452 | 1147 4   | 1370 | 1034 | 14.47 | 0.25  | -16.53 | -19.40 | 6.87 | 25   |      |
| 962  | PGC467523     | J213401.6-502006 | 1589 64  | 1546 | 1296 | 17.29 | 0.13  | -14.09 | -16.44 | 3.14 | 21   |      |
| 963  | NGC7090       | J213628.9-543327 | 850 4    | 784  | 694  | 11.31 | 0.10  | -18.68 | -21.57 | 3.37 | 02   |      |
| 964  | PGC3319496    | J213742.5-160159 | 1139 123 | 1280 | 945  | 19.45 | 0.27  | -11.38 | -13.73 | 5.75 | 21   | +    |
| 965  | UGC11782      | J213809.4+085738 | 1112 3   | 1359 | 1036 | 15.19 | 0.19  | -15.76 | -18.16 | 5.73 | 25   |      |
| 966  | PGC1016598    | J213902.9-073443 | 1283 2   | 1464 | 1127 | 18.36 | 0.17  | -12.75 | -18.02 | 6.07 | 25   |      |
| 967  | PGC163318     | J213935.2-401653 | 1034 59  | 1046 | 762  | 17.25 | 0.09  | -12.93 | -16.59 | 5.08 | 21   |      |
| 968  | PGC1034072    | J214226.9-061954 | 1256 7   | 1443 | 1107 | 15.51 | 0.15  | -15.55 | -17.90 | 6.36 | 25   |      |
| 969  | PGC097237     | J214308.4+445507 | 1582 5   | 1898 | 1695 | -     | 1.24  | -      | -20.79 | 6.50 | 23   |      |
| 970  | PGC3319932    | J214347.4-613235 | 1349 123 | 1246 | 1047 | 18.98 | 0.15  | -11.95 | -14.31 | 5.03 | 24   |      |
| 971  | PGC999560     | J214451.7-084537 | 1287 1   | 1462 | 1128 | 16.07 | 0.18  | -15.05 | -17.40 | 5.74 | 25   |      |
| 972  | PGC129785     | J214455.9-490103 | 1547 39  | 1511 | 1285 | 15.16 | 0.11  | -16.18 | -18.72 | 3.31 | 21   | ++   |
| 973  | ESO236-039    | J214514.7-490032 | 1600 4   | 1564 | 1286 | 15.10 | 0.12  | -16.25 | -18.70 | 3.30 | 21   | ++   |
| 974  | UGC11820      | J214928.5+141351 | 1104 2   | 1368 | 1061 | 15.70 | 0.51  | -15.62 | -16.75 | 4.41 | 25   |      |
| 975  | PGC067479     | J215102.9+061432 | 1443 10  | 1681 | 1360 | 15.56 | 0.22  | -16.02 | -18.59 | 4.42 | 25   |      |
| 976  | ESO532-002    | J215322.4-263443 | 1772 4   | 1858 | 1546 | 16.50 | 0.15  | -15.30 | -15.65 | 3.95 | 21   |      |
| 977  | ESO601-001    | J215642.9-211234 | 1777 39  | 1891 | 1572 | 15.23 | 0.12  | -16.56 | -18.89 | 2.38 | 21   |      |
| 978  | PGC197925     | J215659.5-245149 | 1766 49  | 1861 | 1548 | 16.87 | 0.16  | -14.92 | -17.27 | 3.30 | 21   |      |
| 979  | PGC677866     | J215749.0-331932 | 989 89   | 1039 | 743  | 19.02 | 0.10  | -11.11 | -13.46 | 4.94 | 21   |      |
| 980  | UGC11874      | J220051.9+513419 | 741 4    | 1056 | 892  | 15.40 | 2.60  | -17.64 | -21.14 | 4.87 | 22   |      |
| 981  | NGC7180       | J220218.5-203252 | 1440 88  | 1557 | 1241 | 13.53 | 0.14  | -17.76 | -21.50 | 2.79 | 25   |      |
| 982  | ESO601-007    | J220221.7-210229 | 1789 3   | 1904 | 1582 | 15.21 | 0.15  | -16.62 | -18.21 | 2.23 | 21   |      |
| 983  | NGC7185       | J220256.8-202817 | 1789 9   | 1906 | 1582 | 13.41 | 0.13  | -18.40 | -21.88 | 2.06 | 21   |      |
| 984  | ESO532-014    | J220257.3-222822 | 1715 5   | 1822 | 1524 | 14.98 | 0.11  | -16.72 | -17.81 | 2.25 | 21   | ++   |
| 985  | ESO532-015    | J220308.2-222340 | 1746 9   | 1853 | 1524 | 15.68 | 0.11  | -16.03 | -19.84 | 2.22 | 21   | ++   |
| 986  | PGC509817     | J220319.2-465109 | 1507 50  | 1483 | 1167 | 16.79 | 0.08  | -14.31 | -16.66 | 3.90 | 21   |      |
| 987  | NGC7188       | J220329.0-201905 | 1761 4   | 1879 | 1582 | 13.97 | 0.14  | -17.84 | -20.75 | 2.01 | 21   |      |
| 988  | UGC11891      | J220333.8+434457 | 461 3    | 775  | 576  | 15.36 | 1.52  | -15.65 | -18.00 | 2.92 | 21   |      |
| 989  | ESO237-033    | J220355.1-494244 | 1634 45  | 1593 | 1352 | 16.88 | 0.10  | -14.56 | -17.53 | 2.63 | 21   |      |
| 990  | PGC3244570    | J220705.5-233917 | 1769 89  | 1870 | 1561 | 16.84 | 0.12  | -14.93 | -17.28 | 2.78 | 21   |      |
| 991  | PGC551779     | J220748.5-431204 | 1588 60  | 1583 | 1321 | 16.66 | 0.06  | -14.68 | -17.03 | 3.06 | 21   | +    |
| 992  | ESO288-042    | J220751.0-431640 | 1396 8   | 1391 | 1129 | 15.37 | 0.06  | -15.64 | -16.76 | 3.15 | 21   | +    |
| 993  | PGC168205     | J220805.7+674132 | 1180 5   | 1476 | 1399 | 16.35 | 1.89  | -16.95 | -20.55 | 4.10 | 22   |      |
| 994  | PGC3223120    | J221056.6-295851 | 1529 123 | 1596 | 1301 | 19.28 | 0.08  | -12.05 | -14.40 | 2.29 | 21   |      |
| 995  | PGC3221845    | J221356.6-280551 | 1949 123 | 2026 | 1728 | 18.79 | 0.07  | -13.15 | -15.51 | 4.56 | 21   | +    |
| 996  | AGC321307     | J221404.7+254052 | 1152 4   | 1444 | 1182 | 18.15 | 0.37  | -13.27 | -      | 2.66 | 23   |      |
| 997  | ESO467-029    | J221447.0-294113 | 1732 64  | 1800 | 1507 | 16.23 | 0.07  | -15.42 | -18.84 | 4.33 | 21   |      |
| 998  | PGC3221776    | J221532.3-280342 | 869 123  | 946  | 649  | 19.18 | 0.07  | -10.64 | -12.99 | 3.92 | 21   |      |
| 999  | NGC7250       | J221817.8+403345 | 1167 4   | 1478 | 1273 | 13.20 | 0.66  | -18.67 | -21.01 | 2.46 | 23   |      |
| 1000 | PGC130771     | J221848.9-461303 | 1208 45  | 1185 | 939  | 16.14 | 0.08  | -14.49 | -16.58 | 3.03 | 02   |      |
| 1001 | PGC647204     | J222008.8-353438 | 1499 123 | 1534 | 1258 | 18.64 | 0.05  | -12.60 | -14.95 | 2.41 | 21   |      |
| 1002 | IC5201        | J222057.4-460207 | 915 3    | 894  | 646  | 11.39 | 0.05  | -18.40 | -21.48 | 4.48 | 02   |      |
| 1003 | ESO289-020    | J222111.7-454036 | 912 67   | 892  | 645  | 15.62 | 0.06  | -14.17 | -17.86 | 4.44 | 02   |      |
| 1004 | ESO238-005    | J222230.5-482414 | 706 3    | 671  | 585  | 15.30 | 0.06  | -14.28 | -16.63 | 4.22 | 02   |      |
| 1005 | UGC12009      | J222240.3+375839 | 1237 3   | 1546 | 1334 | 13.74 | 0.53  | -18.10 | -20.44 | 3.54 | 23   |      |

| (1)  | (2)                     | (3)              | (4)      | (5)  | (6)  | (7)   | (8)  | (9)    | (10)   | (11) | (12) | (13) |
|------|-------------------------|------------------|----------|------|------|-------|------|--------|--------|------|------|------|
| 1006 | NGC7259                 | J222305.5-285717 | 1718 26  | 1789 | 1470 | 13.74 | 0.09 | -17.87 | -20.76 | 3.62 | 21   |      |
| 1007 | ESO467-051              | J222317.2-285851 | 1804 6   | 1874 | 1470 | 14.38 | 0.08 | -17.23 | -17.31 | 3.61 | 21   |      |
| 1008 | PGC744475               | J222324.9-281234 | 1027 60  | 1102 | 811  | 18.36 | 0.09 | -11.96 | -14.31 | 4.13 | 21   |      |
| 1009 | 6dFJ2226...             | J222633.6-291728 | 1025 45  | 1094 | 714  | 19.57 | 0.07 | -10.45 | -      | 4.22 | 21   |      |
| 1010 | PGC988084               | J222730.6-093956 | 1698 1   | 1865 | 1549 | 15.99 | 0.22 | -15.86 | -18.21 | 3.10 | 25   | ++   |
| 1011 | PGC068921               | J222741.5-094337 | 1643 2   | 1810 | 1505 | 16.73 | 0.21 | -15.05 | -17.48 | 2.92 | 25   | ++   |
| 1012 | PGC068681               | J223036.8-000637 | 1588 5   | 1796 | 1497 | 17.35 | 0.30 | -14.51 | -16.86 | 5.81 | 25   |      |
| 1013 | PGC1193620              | J223046.5+012343 | 1574 6   | 1788 | 1490 | 17.07 | 0.39 | -14.87 | -17.22 | 5.27 | 25   |      |
| 1014 | PGC1149494              | J223106.0-001144 | 1554 1   | 1761 | 1462 | 17.28 | 0.29 | -14.52 | -16.92 | 5.80 | 25   |      |
| 1015 | PGC085239               | J223213.3-411010 | 1593 23  | 1596 | 1342 | 16.09 | 0.06 | -15.29 | -16.98 | 2.29 | 21   |      |
| 1016 | ESO289-037              | J223319.8-443259 | 1242 30  | 1227 | 983  | 14.74 | 0.06 | -15.97 | -17.96 | 2.19 | 24   |      |
| 1017 | ABELL3888-14...         | J223329.3-372731 | 1008 19  | 1031 | 768  | 18.49 | 0.07 | -11.69 | -      | 3.91 | 02   | +    |
| 1018 | PGC069224               | J223454.6-044206 | 889 5    | 1077 | 779  | 15.84 | 0.18 | -14.48 | -18.43 | 5.73 | 25   |      |
| 1019 | PGC095093               | J223505.5-462738 | 937 96   | 911  | 674  | 14.50 | 0.05 | -15.38 | -16.42 | 4.49 | 02   |      |
| 1020 | ABELL3888-12...         | J223633.3-373005 | 760 13   | 783  | 521  | 18.80 | 0.08 | -10.55 | -      | 2.94 | 02   |      |
| 1021 | PGC069293               | J223635.0-025424 | 1692 2   | 1888 | 1591 | 13.38 | 0.22 | -18.53 | -20.91 | 5.77 | 25   |      |
| 1022 | PGC069415               | J223908.8-044537 | 830 2    | 1016 | 721  | 14.97 | 0.23 | -15.23 | -18.35 | 5.06 | 25   |      |
| 1023 | PGC069416               | J223918.0-014201 | 1706 42  | 1906 | 1613 | 16.36 | 0.19 | -15.55 | -18.30 | 6.37 | 25   |      |
| 1024 | SDSSJ224114.12-003715.1 | J224114.3-003710 | 1774 1   | 1978 | 1687 | 16.81 | 0.25 | -15.26 | -17.60 | 7.00 | 25   |      |
| 1025 | NGC7351                 | J224126.9-042641 | 891 6    | 1078 | 785  | 13.59 | 0.19 | -16.76 | -20.18 | 5.69 | 25   |      |
| 1026 | UGC12151                | J224133.9+002403 | 1763 5   | 1971 | 1681 | 15.43 | 0.30 | -16.68 | -19.03 | 6.61 | 25   |      |
| 1027 | NGC7361                 | J224218.4-300319 | 1251 3   | 1313 | 1058 | 12.88 | 0.07 | -18.00 | -20.41 | 2.13 | 03   |      |
| 1028 | PGC1028063              | J224223.5-065010 | 899 6    | 1075 | 783  | 16.02 | 0.15 | -14.28 | -16.63 | 5.44 | 25   |      |
| 1029 | PGC3225142              | J224252.8-301328 | 1289 89  | 1349 | 1058 | 18.10 | 0.07 | -12.78 | -15.13 | 2.08 | 03   |      |
| 1030 | PGC982181               | J224359.9-100701 | 957 1    | 1119 | 827  | 17.69 | 0.23 | -12.81 | -15.16 | 5.66 | 25   |      |
| 1031 | ESO346-007              | J225323.9-384758 | 926 17   | 938  | 692  | 15.10 | 0.06 | -14.84 | -16.99 | 3.76 | 02   |      |
| 1032 | NGC7406                 | J225356.3-063445 | 1604 5   | 1778 | 1497 | 14.38 | 0.16 | -17.34 | -21.08 | 5.22 | 25   |      |
| 1033 | PGC069990               | J225445.2-265324 | 818 6    | 893  | 624  | 15.27 | 0.12 | -14.51 | -16.45 | 2.65 | 21   |      |
| 1034 | NGC7412A                | J225709.0-424817 | 929 3    | 919  | 686  | 14.51 | 0.04 | -15.39 | -18.00 | 3.94 | 02   | ++   |
| 1035 | NGC7424                 | J225718.4-410414 | 937 9    | 936  | 698  | 11.04 | 0.05 | -18.91 | -20.38 | 3.91 | 02   | ++   |
| 1036 | AF7448.001              | J225935.5+164604 | 360 6    | 620  | 372  | 17.54 | 0.29 | -11.29 | -13.63 | 3.89 | 21   |      |
| 1037 | PGC938611               | J225946.2-132321 | 1217 6   | 1358 | 1082 | 15.92 | 0.21 | -15.14 | -18.28 | 4.27 | 25   |      |
| 1038 | PGC732721               | J230243.7-290904 | 779 60   | 840  | 582  | 17.75 | 0.13 | -11.89 | -14.24 | 2.17 | 02   |      |
| 1039 | NGC7462                 | J230246.5-405007 | 1061 3   | 1060 | 826  | 12.21 | 0.05 | -18.11 | -20.62 | 3.04 | 02   |      |
| 1040 | ESO290-039              | J230329.7-460153 | 1530 5   | 1501 | 1281 | 15.02 | 0.06 | -16.26 | -18.95 | 2.49 | 04   |      |
| 1041 | PGC141060               | J230341.2+234110 | 1155 4   | 1432 | 1204 | 17.08 | 0.60 | -14.61 | -16.96 | 2.90 | 25   |      |
| 1042 | AGC335193               | J230349.0+043113 | 1225 8   | 1443 | 1178 | 17.12 | 0.28 | -14.20 | -      | 5.39 | 25   |      |
| 1043 | AGC335310               | J231102.7+321650 | 1114 8   | 1405 | 1209 | 18.32 | 0.25 | -13.03 | -      | 2.73 | 01   |      |
| 1044 | APPLES1                 | J231503.3-423222 | 674 30   | 661  | 440  | -     | 0.05 | -      | -      | 2.73 | 02   |      |
| 1045 | ESO536-003              | J232216.1-234204 | 1690 7   | 1773 | 1526 | 15.96 | 0.11 | -15.75 | -18.27 | 4.57 | 25   | ++   |
| 1046 | PGC134530               | J232217.8-233308 | 1618 39  | 1702 | 1455 | 15.93 | 0.10 | -15.67 | -16.99 | 4.69 | 25   | ++   |
| 1047 | ESO240-002              | J232359.4-503127 | 1577 6   | 1519 | 1327 | 15.00 | 0.05 | -16.35 | -18.35 | 2.90 | 04   |      |
| 1048 | ESO347-017              | J232656.2-372049 | 691 3    | 701  | 475  | 14.93 | 0.07 | -14.20 | -16.56 | 2.02 | 02   |      |
| 1049 | PGC071479               | J232721.0-232956 | 1759 5   | 1841 | 1599 | 14.99 | 0.10 | -16.81 | -19.01 | 3.90 | 25   |      |
| 1050 | ESO240-004              | J232753.1-510755 | 1576 10  | 1514 | 1326 | 15.69 | 0.06 | -15.66 | -18.59 | 3.11 | 04   |      |
| 1051 | HIPASSJ2331+01          | J233103.8+013410 | 1270 8   | 1466 | 1227 | -     | 0.17 | -      | -      | 4.85 | 25   |      |
| 1052 | PGC086525               | J233230.4+173323 | 1414 8   | 1664 | 1451 | 16.77 | 0.27 | -14.99 | -17.61 | 2.73 | 01   |      |
| 1053 | PGC226770               | J233237.9-805040 | 1880 45  | 1680 | 1596 | 18.68 | 0.56 | -13.58 | -18.87 | 3.66 | 24   |      |
| 1054 | NGC7690                 | J233302.5-514154 | 1502 3   | 1436 | 1253 | 12.94 | 0.05 | -18.28 | -21.69 | 3.88 | 04   |      |
| 1055 | ESO291-031              | J233420.5-455944 | 1491 6   | 1454 | 1257 | 15.47 | 0.04 | -15.75 | -18.10 | 2.97 | 04   |      |
| 1056 | UGC12682                | J233453.4+181336 | 1392 2   | 1643 | 1434 | 14.07 | 0.34 | -17.74 | -20.08 | 2.94 | 01   | ++   |
| 1057 | UGC12681                | J233454.6+180416 | 1465 5   | 1716 | 1506 | 15.20 | 0.34 | -16.72 | -17.81 | 2.47 | 01   | ++   |
| 1058 | ESO291-033              | J233501.9-470150 | 1509 22  | 1467 | 1273 | 16.31 | 0.05 | -14.95 | -18.52 | 2.91 | 04   |      |
| 1059 | PGC4126728              | J233524.0-164124 | 1769 12  | 1882 | 1648 | 13.60 | 0.12 | -18.29 | -      | 2.52 | 25   |      |
| 1060 | ESO605-014              | J233620.6-171612 | 1785 45  | 1895 | 1649 | 15.41 | 0.12 | -16.48 | -18.29 | 2.65 | 25   |      |
| 1061 | ESO605-015              | J233636.2-215142 | 1552 3   | 1638 | 1405 | 16.41 | 0.12 | -15.13 | -18.16 | 4.68 | 25   |      |
| 1062 | PGC071938               | J233739.5+300746 | 1383 2   | 1662 | 1484 | 15.50 | 0.41 | -16.45 | -19.48 | 5.26 | 01   |      |
| 1063 | UGC12713                | J233814.3+304230 | 288 3    | 567  | 392  | 14.82 | 0.27 | -14.10 | -15.04 | 3.59 | 21   |      |
| 1064 | PGC072034               | J233925.5-211809 | 1511 64  | 1599 | 1368 | 15.94 | 0.11 | -15.53 | -19.16 | 4.76 | 25   |      |
| 1065 | ESO605-024              | J234001.0-220529 | 1581 5   | 1665 | 1436 | 16.86 | 0.10 | -14.71 | -17.06 | 4.63 | 25   |      |
| 1066 | PGC3324739              | J234020.6-545155 | 1589 45  | 1505 | 1336 | 16.38 | 0.06 | -14.99 | -17.34 | 4.28 | 04   |      |
| 1067 | ESO606-001              | J234032.7-205638 | 1397 8   | 1487 | 1257 | 16.49 | 0.11 | -14.80 | -17.65 | 4.66 | 25   |      |
| 1068 | UGC12732                | J234039.8+261410 | 747 2    | 1016 | 833  | 14.37 | 0.38 | -16.30 | -16.94 | 3.28 | 25   | ++   |
| 1069 | PGC3094306              | J234056.8-190507 | 1602 39  | 1701 | 1470 | 14.88 | 0.13 | -16.77 | -19.11 | 5.01 | 25   |      |
| 1070 | ESO292-014              | J234235.2-445417 | 1491 3   | 1457 | 1264 | 13.98 | 0.05 | -17.26 | -20.43 | 2.91 | 04   |      |
| 1071 | NGC7741                 | J234354.4+260432 | 752 7    | 1019 | 836  | 11.82 | 0.33 | -18.81 | -20.69 | 3.36 | 25   | ++   |
| 1072 | PGC072271               | J234426.1-164849 | 1571 5   | 1679 | 1451 | 15.76 | 0.11 | -15.84 | -      | 4.92 | 25   |      |
| 1073 | PGC1016288              | J234429.7-073548 | 1832 5   | 1983 | 1755 | 15.99 | 0.14 | -16.05 | -18.65 | 2.11 | 25   |      |
| 1074 | ESO606-007              | J234609.5-192131 | 1790 3   | 1885 | 1660 | 15.42 | 0.10 | -16.46 | -18.82 | 3.27 | 25   |      |
| 1075 | ESO292-023              | J234652.1-470807 | 1671 54  | 1624 | 1440 | 16.98 | 0.06 | -14.56 | -16.90 | 2.22 | 04   |      |
| 1076 | PGC902220               | J234813.3-160714 | 1772 39  | 1881 | 1658 | 15.73 | 0.11 | -16.16 | -18.51 | 2.44 | 25   |      |
| 1077 | AGC333210               | J234841.8+255440 | 1612 5   | 1877 | 1700 | 19.19 | 0.38 | -13.03 | -      | 4.40 | 01   |      |
| 1078 | UGC12791                | J234849.3+261314 | 791 2    | 1056 | 880  | 15.74 | 0.26 | -14.93 | -17.28 | 3.15 | 25   |      |
| 1079 | AGC334513               | J234850.4+233527 | 1662 6   | 1921 | 1739 | 18.89 | 0.26 | -13.25 | -      | 3.89 | 01   | ++   |
| 1080 | PGC1700470              | J234946.7+240800 | 1649 4   | 1910 | 1730 | 18.18 | 0.26 | -13.95 | -16.30 | 4.05 | 01   | ++   |
| 1081 | PGC812517               | J234951.7-223256 | 1026 7   | 1103 | 885  | 16.09 | 0.10 | -14.43 | -16.90 | 4.77 | 03   |      |
| 1082 | ESO149-003              | J235202.9-523438 | 574 4    | 499  | 512  | 15.01 | 0.06 | -14.28 | -16.63 | 3.46 | 02   |      |
| 1083 | PGC4581795              | J235419.3+105647 | 943 5    | 1162 | 963  | 17.91 | 0.39 | -13.08 | -      | 3.92 | 25   |      |
| 1084 | PGC072872               | J235527.0-061414 | 1243 64  | 1394 | 1180 | 15.97 | 0.12 | -15.20 | -19.20 | 6.46 | 25   |      |
| 1085 | PGC3194675              | J235552.5-291149 | 1259 123 | 1300 | 1095 | 19.34 | 0.06 | -11.60 | -13.95 | 3.76 | 03   |      |
| 1086 | ESO241-006              | J235615.1-432539 | 1453 12  | 1422 | 1238 | 14.40 | 0.06 | -16.81 | -19.00 | 3.39 | 04   |      |
| 1087 | ESO012-010              | J235628.8-813403 | 1940 4   | 1736 | 1659 | 14.47 | 0.58 | -17.89 | -20.56 | 3.86 | 24   |      |
| 1088 | ESO078-010              | J235711.3-644054 | 1905 87  | 1770 | 1639 | 14.92 | 0.08 | -16.92 | -19.08 | 4.53 | 04   |      |

**J000535.9-412856:** triplet with J000619.9-413000 and J000625.4-413024?  
**J000619.9-413000:** triplet with J000535.9-412856 and J000625.4-413024?  
**J000625.4-413024:** triplet with J000535.9-412856 and J000619.9-413000?  
**J000651.6-415023:** pair with J000652.8-412530?  
**J000652.8-412530:** pair with J000651.6-415023?  
**J001354.1+124826:** pair with J001400.8+125750?  
**J001400.8+125750:** pair with J001354.1+124826?  
**J010908.0+010716:** pair with J010910.1+011728?  
**J010910.1+011728:** pair with J010908.0+010716?  
**J011250.5+015207:** member of group NGC428 (J011255.7+005854)?  
**J011250.7+010249:** member of group NGC428  
**J011255.7+005854** (NGC428): center of void group  
**J011339.4+005230:** member of group NGC428  
**J011420.4+005501:** member of group NGC428  
**J015345.7-234528:** pair with J015346.2-230646?  
**J015346.2-230646:** pair with J015345.7-234528?  
**J020010.1+284952:** pair with J020116.9+285014?  
**J020116.9+285014:** pair with J020010.1+284952?  
**J022705.1-323242:** pair with J022756.7-324543?  
**J022756.7-324543:** pair with J022705.1-323242?  
**J023928.0-555906:** pair with J024009.5-562034?  
**J024009.5-562034:** pair with J023928.0-555906?  
**J024325.6+164359:** pair with J024326.8+163946?  
**J024326.8+163946:** pair with J024325.6+164359?  
**J024340.1+230524:** pair with J024447.3+225001?  
**J024447.3+225001:** pair with J024340.1+230524?  
**J025512.7-361758:** pair with J025539.4-362008?  
**J025539.4-362008:** pair with J025512.7-361758?  
**J031001.2-532009:** pair with J031016.3-531953?  
**J031016.3-531953:** pair with J031001.2-532009?  
**J031702.3+033858:** pair with J031718.4+033643?  
**J031718.4+033643:** pair with J031702.3+033858?  
**J040331.3-015541:** pair with J040427.2-021117?  
**J040427.2-021117:** pair with J040331.3-015541?  
**J041312.4+132519:** pair with J041314.4+132109  
**J041314.4+132109:** pair with J041312.4+132519  
**J045129.2-613903:** pair with J045455.4-613353?  
**J045455.4-613353:** pair with J045129.2-613903?  
**J050300.3-252806:** pair with J050320.0-252525  
**J050320.0-252525:** pair with J050300.3-252806  
**J060008.3-311734:** pair with J060010.7-314714?  
**J060010.7-314714:** pair with J060008.3-311734?  
**J061554.3-574332:** pair with J061608.5-574551  
**J061608.5-574551:** pair with J061554.3-574332  
**J064427.6-175557:** pair with J064552.9-181243  
**J064552.9-181243:** pair with J064427.6-175557  
**J070024.6-041314:** pair with J070028.9-041220  
**J070028.9-041220:** pair with J070024.6-041314  
**J070359.2+562911:** pair with J070450.6+563113?  
**J070450.6+563113:** pair with J070359.2+562911?  
**J070623.4+302051:** pair with J070627.5+301920  
**J070627.5+301920:** pair with J070623.4+302051  
**J070918.3+442248:** pair with J071013.6+442726  
**J071013.6+442726:** pair with J070918.3+442248  
**J072301.4+362117:** triplet with J072313.5+362213 and J072320.6+362441  
**J072313.5+362213:** triplet with J072301.4+362117 and J072320.6+362441  
**J072320.6+362441:** triplet with J072301.4+362117 and J072313.5+362213  
**J074155.4+164809:** pair with J074231.7+163340  
**J074231.7+163340:** pair with J074155.4+164809  
**J074443.7+250826:** pair with J074455.5+250602  
**J074455.5+250602:** pair with J074443.7+250826  
**J074656.4+511743:** pair with J074731.8+511130

**J074731.8+511130:** pair with J074656.4+511743  
**J081314.7+455924:** pair with J081358.9+454431  
**J081358.9+454431:** pair with J081314.7+455924  
**J082555.5+353232:** pair with J082605.6+353525  
**J082605.6+353525:** pair with J082555.5+353232  
**J085233.8+135028:** pair with J085240.9+135157  
**J085240.9+135157:** pair with J085233.8+135028  
**J085900.3+391235:** pair with J085947.0+392304  
**J085947.0+392304:** pair with J085900.3+391235  
**J092000.6+395333:** pair with J092147.9+400904?  
**J092147.9+400904:** pair with J092000.6+395333?  
**J093359.7+551445:** pair with J093402.1+551426 (IZw18)  
**J093402.1+551426:** pair with J093359.7+551445 (IZw18C)  
**J094258.7+331556:** pair with J094332.4+332658  
**J094332.4+332658:** pair with J094258.7+331556  
**J094401.9-003832:** pair with J094407.2-003930  
**J094407.2-003930:** pair with J094401.9-003832  
**J094747.6+390503:** triplet with J094750.3+390832 and J094758.4+390510  
**J094750.3+390832:** triplet with J094747.6+390503 and J094758.4+390510  
**J094758.4+390510:** triplet with J094747.6+390503 and J094750.3+390832  
**J095019.5+312722:** pair with J095022.4+312916  
**J095022.4+312916:** pair with J095019.5+312722  
**J095208.2+291411:** pair with J095241.9+292141  
**J095241.9+292141:** pair with J095208.2+291411  
**J095641.1+290051:** pair with J095645.7+284933 (DDO68)  
**J095645.7+284933:** pair with J095641.1+290051 (DDO68C)  
**J095853.4+474413:** pair with J095918.7+473658  
**J095918.7+473658:** pair with J095853.4+474413  
**J101547.9+374459:** triplet with J101622.0+374647 and J101624.5+375446  
**J101622.0+374647:** triplet with J101547.9+374459 and J101624.5+375446  
**J101624.5+375446:** triplet with J101547.9+374459 and J101622.0+374647  
**J102931.0-351535:** quartet with J102953.0-352231, J103018.3-351149 and J103025.8-350629  
**J102953.0-352231:** quartet with J102931.0-351535, J103018.3-351149 and J103025.8-350629  
**J103018.3-351149:** quartet with J102931.0-351535, J102953.0-352231 and J103025.8-350629  
**J103025.8-350629:** quartet with J102931.0-351535, J102953.0-352231 and J103018.3-351149  
**J111307.9-691546:** pair with J111941.3-690514?  
**J111941.3-690514:** pair with J111307.9-691546?  
**J123438.4+734000:** pair with J123532.5+734029  
**J123532.5+734029:** pair with J123438.4+734000  
**J124732.9-535647:** pair with J124737.3-533300?  
**J124737.3-533300:** pair with J124732.9-535647?  
**J124957.8+051841:** pair with J124959.2+054916?  
**J124959.2+054916:** pair with J124957.8+051841?  
**J125956.6-192441:** not in NGC5068 (J131854.9-210221) group. Their D(TRGB) differ by  $\sim 2$  Mpc.  
**J130222.8-492841:** pair with J130223.6-492824  
**J130223.6-492824:** pair with J130222.8-492841  
**J133922.3+311458:** pair with J133947.9+311726  
**J133947.9+311726:** pair with J133922.3+311458  
**J133931.6+392559:** pair with J133945.0+390809  
**J133945.0+390809:** pair with J133931.6+392559  
**J134134.8+383145:** pair with J134142.4+382957  
**J134142.4+382957:** pair with J134134.8+383145  
**J134722.1+381810:** triplet with J134745.0+381816 and J134745.5+381533  
**J134745.0+381816:** triplet with J134722.1+381810 and J134745.5+381533  
**J134745.5+381533:** triplet with J134722.1+381810 and J134745.0+381816  
**J141853.5+091729:** pair with J141944.7+092145  
**J141944.7+092145:** pair with J141853.5+091729  
**J142110.4-291504:** pair with J142117.1-291548  
**J142117.1-291548:** pair with J142110.4-291504  
**J142810.9+133306:** pair with J142818.4+134649  
**J142818.4+134649:** pair with J142810.9+133306  
**J143039.4+071630:** pair with J143048.7+070926

**J143048.7+070926:** pair with J143039.4+071630  
**J143220.8+095601:** pair with J143243.9+095329?  
**J143243.9+095329:** pair with J143220.8+095601?  
**J143533.3+125430:** pair with J143539.9+131012?  
**J143539.9+131012:** pair with J143533.3+125430?  
**J144003.5+340600:** triplet with J144026.2+335920 and J144031.6+341601  
**J144026.2+335920:** triplet with J144003.5+340600 and J144031.6+341601  
**J144031.6+341601:** triplet with J144003.5+340600 and J144026.2+335920  
**J144412.8+423744:** pair with J144449.8+424254  
**J144449.8+424254:** pair with J144412.8+423744  
**J144536.3+341044:** pair with J144621.1+342214  
**J144621.1+342214:** pair with J144536.3+341044  
**J144728.4+124554:** pair with J144842.6+122726  
**J144842.6+122726:** pair with J144728.4+124554  
**J145056.6+353419:** pair with J145114.4+353232  
**J145114.4+353232:** pair with J145056.6+353419  
**J145938.3+444023:** pair with J150109.3+444153  
**J150109.3+444153:** pair with J145938.3+444023  
**J153515.8+305151:** quartet with J153545.4+310809, J153618.9+304333 and J153619.5+304056  
**J153545.4+310809:** quartet with J153515.8+305151, J153618.9+304333 and J153619.5+304056  
**J153618.9+304333:** quartet with J153515.8+305151, J153545.4+310809 and J153619.5+304056  
**J153619.5+304056:** quartet with J153515.8+305151, J153545.4+310809 and J153618.9+304333  
**J164021.4+284556:** pair with J164022.2+282818  
**J164022.2+282818:** pair with J164021.4+284556  
**J165005.0+424423:** pair with J165046.0+424321?  
**J165046.0+424321:** pair with J165005.0+424423?  
**J165254.4+360515:** pair with J165447.8+363005?  
**J165447.8+363005:** pair with J165254.4+360515?  
**J171307.0+591924:** pair with J171851.4+495303?  
**J171310.3+591956:** pair with J171307.0+591924?  
**J171851.4+495303:** pair with J171907.7+495122?  
**J171907.7+495122:** pair with J171851.4+495303?  
**J174414.8+673710:** pair with J174629.6+672017  
**J174629.6+672017:** pair with J174414.8+673710  
**J174926.5+700840:** pair with J175248.0+700815??  
**J175248.0+700815:** pair with J174926.5+700840??  
**J180727.5+353350:** triplet with J180729.0+353726 and J180745.0+352330  
**J180729.0+353726:** triplet with J180727.5+353350 and J180745.0+352330  
**J180745.0+352330:** triplet with J180727.5+353350 and J180729.0+353726  
**J193602.3-610140:** pair with J193847.5-610943  
**J193847.5-610943:** pair with J193602.3-610140  
**J202608.8-552950:** pair with J202733.8-550525  
**J202733.8-550525:** pair with J202608.8-552950  
**J210347.2-004950:** pair with J210455.3-003522?  
**J210455.3-003522:** pair with J210347.2-004950?  
**J211842.0+261737:** pair with J211858.9+252551?  
**J211858.9+252551:** pair with J211842.0+261737?  
**J214455.9-490103:** pair with J214514.7-490032?  
**J214514.7-490032:** pair with J214455.9-490103?  
**J220257.3-222822:** pair with J220308.2-222340?  
**J220308.2-222340:** pair with J220257.3-222822?  
**J220748.5-431204:** pair with J220751.0-431640?  
**J220751.0-431640:** pair with J220748.5-431204?  
**J232216.1-234204:** pair with J232217.8-233308?  
**J232217.8-233308:** pair with J232216.1-234204?

Table A2: Main parameters of 'outer' subsample galaxies in the nearby voids

| Nu.  | Name       | RA (J2000)       | Dec.     | $V_{\text{hel}} \pm \sigma_V$ | $V_{\text{LG}}$ | $V_{\text{dist}}$ | $B_{\text{tot}}$ | $A_B$  | $M_B$  | $M_K$ | $D_{\text{NN}}$ | Void | Notes |
|------|------------|------------------|----------|-------------------------------|-----------------|-------------------|------------------|--------|--------|-------|-----------------|------|-------|
| (1)  | (2)        | (3)              | (4)      | (5)                           | (6)             | (7)               | (8)              | (9)    | (10)   | (11)  | (12)            | (13) |       |
| 1089 | PGC771694  | J000103.0-260521 | 400 59   | 455                           | 455             | 18.81             | 0.07             | -17.32 | -12.58 | 1.11  | 21              |      |       |
| 1090 | ESO409-015 | J000531.9-280554 | 732 6    | 774                           | 636             | 15.13             | 0.07             | -14.65 | -17.90 | 1.47  | 03              |      |       |
| 1091 | NGC0055    | J001453.6-391148 | 129 1    | 111                           | 153             | 8.39              | 0.06             | -18.28 | -20.14 | 1.69  | 10              |      |       |
| 1092 | NGC0059    | J001525.1-212640 | 366 3    | 436                           | 351             | 13.13             | 0.09             | 99.99  | -18.33 | 1.34  | 21              |      |       |
| 1093 | UGC00156   | J001648.2+122100 | 1136 4   | 1348                          | 1180            | 14.91             | 0.55             | -16.68 | -19.03 | 1.59  | 03              | ++   |       |
| 1094 | PGC3197756 | J001736.3-312618 | 749 123  | 769                           | 589             | 19.28             | 0.08             | -10.34 | -12.69 | 1.18  | 03              |      |       |
| 1095 | NGC0063    | J001745.5+112701 | 1162 4   | 1371                          | 1180            | 12.70             | 0.48             | -18.82 | -21.82 | 1.82  | 03              | ++   |       |
| 1096 | PGC132768  | J002304.2-275537 | 1536 6   | 1570                          | 1394            | 15.60             | 0.08             | -15.89 | -19.99 | 0.96  | 03              |      |       |
| 1097 | ESO294-010 | J002633.4-415120 | 113 4    | 77                            | 142             | 15.56             | 0.02             | -10.90 | -12.36 | 1.85  | 10              |      |       |
| 1098 | PGC198152  | J002732.7-263419 | 1491 8   | 1530                          | 1358            | 16.50             | 0.06             | -14.91 | -16.70 | 1.16  | 03              |      |       |
| 1099 | PGC776357  | J003137.5-254007 | 1469 64  | 1510                          | 1343            | 18.41             | 0.06             | -12.98 | -15.33 | 1.39  | 03              |      |       |
| 1100 | PGC795900  | J003625.3-235321 | 1479 39  | 1525                          | 1363            | 16.35             | 0.08             | -15.09 | -17.44 | 1.59  | 03              |      |       |
| 1101 | PGC002323  | J003849.1-241322 | 1541 10  | 1585                          | 1426            | 15.20             | 0.07             | -16.32 | -19.75 | 1.27  | 03              |      |       |
| 1102 | PGC3236227 | J004209.8-265838 | 1439 123 | 1467                          | 1314            | 19.19             | 0.05             | -12.14 | -14.49 | 1.69  | 03              |      |       |
| 1103 | ESO540-016 | J004214.7-180942 | 1554 6   | 1624                          | 1469            | 14.36             | 0.09             | -17.25 | -19.04 | 1.95  | 03              |      |       |
| 1104 | ESO411-014 | J004726.5-281906 | 1559 89  | 1578                          | 1432            | 16.28             | 0.06             | -15.25 | -19.02 | 1.01  | 03              |      |       |
| 1105 | PGC199449  | J011129.2-322933 | 1619 89  | 1603                          | 1489            | 16.81             | 0.10             | -14.84 | -17.19 | 1.49  | 04              |      |       |
| 1106 | PISCESB    | J011911.7+110718 | 616 3    | 783                           | 651             | 17.61             | 0.24             | -12.39 | -14.74 | 1.50  | 25              |      |       |
| 1107 | UGC00891   | J012119.1+122442 | 638 2    | 808                           | 728             | 14.68             | 0.13             | -15.44 | -17.79 | 0.88  | 25              |      |       |
| 1108 | ESO352-067 | J012357.4-334807 | 1475 29  | 1446                          | 1347            | 15.53             | 0.14             | -15.94 | -18.00 | 1.67  | 04              |      |       |
| 1109 | UGC01085   | J013118.9+074716 | 652 2    | 797                           | 727             | 16.75             | 0.19             | -13.44 | -15.79 | 1.14  | 03              |      |       |
| 1110 | AGC114716  | J013525.3+032624 | 1565 8   | 1690                          | 1623            | 18.32             | 0.16             | -13.57 | 99.99  | 1.68  | 03              |      |       |
| 1111 | PGC006228  | J014107.1-053405 | 1501 6   | 1585                          | 1519            | 14.01             | 0.15             | -17.73 | -20.39 | 1.79  | 03              |      |       |
| 1112 | ESO245-005 | J014503.9-433555 | 394 2    | 308                           | 334             | 12.80             | 0.07             | -15.57 | -18.05 | 1.81  | 10              |      |       |
| 1113 | IC1729     | J014755.3-265332 | 1503 10  | 1488                          | 1327            | 13.47             | 0.08             | -17.91 | -21.58 | 1.47  | 03              | ++   |       |
| 1114 | PGC764267  | J014839.3-264518 | 1409 89  | 1394                          | 1328            | 17.71             | 0.07             | -13.66 | -18.07 | 1.52  | 03              | ++   |       |
| 1115 | ESO477-005 | J014849.5-270828 | 1352 38  | 1336                          | 1328            | 15.20             | 0.08             | -16.19 | -17.57 | 1.46  | 03              | ++   |       |
| 1116 | PGC132930  | J015938.8-292859 | 1459 50  | 1425                          | 1373            | 16.25             | 0.07             | -15.20 | -18.55 | 1.82  | 04              |      |       |
| 1117 | UGC01703   | J021255.1+324849 | 40 20    | 234                           | 314             | 17.50             | 0.42             | -11.09 | -13.44 | 1.99  | 08              |      |       |
| 1118 | PGC1002828 | J021541.2-083029 | 1386 12  | 1428                          | 1413            | 18.06             | 0.13             | -13.51 | -15.86 | 1.80  | 03              |      |       |
| 1119 | PGC729204  | J021747.5-292703 | 1240 54  | 1191                          | 1164            | 18.55             | 0.09             | -12.55 | -14.90 | 1.91  | 03              |      |       |
| 1120 | AGC748863  | J023055.1+135900 | 1475 4   | 1594                          | 1619            | 99.99             | 0.64             | 99.99  | 99.99  | 1.96  | 05              |      |       |
| 1121 | PGC1805856 | J023850.0+272156 | 1463 3   | 1622                          | 1666            | 17.28             | 0.61             | -15.12 | -17.47 | 1.19  | 05              |      |       |
| 1122 | PGC3312132 | J023901.4-475140 | 989 123  | 855                           | 839             | 19.37             | 0.07             | -11.01 | -13.36 | 1.96  | 02              |      |       |
| 1123 | AGC122219  | J024055.6+264005 | 1483 4   | 1637                          | 1684            | 17.95             | 0.53             | -14.40 | 99.99  | 1.22  | 05              |      |       |
| 1124 | PGC2807108 | J024504.0+320940 | 1581 2   | 1749                          | 1804            | 17.00             | 0.81             | -15.77 | 99.99  | 1.70  | 05              |      |       |
| 1125 | PGC010813  | J025104.6+042713 | 1012 3   | 1077                          | 1126            | 15.32             | 0.29             | -15.91 | -17.81 | 1.27  | 05              |      |       |
| 1126 | AGC123057  | J025141.5+320610 | 1464 4   | 1627                          | 1691            | 19.90             | 0.99             | -12.91 | 99.99  | 1.85  | 05              |      |       |
| 1127 | AGC124628  | J025445.0+050028 | 1007 8   | 1070                          | 1125            | 17.63             | 0.56             | -13.87 | 99.99  | 1.53  | 05              |      |       |
| 1128 | ESO356-026 | J030021.7-365516 | 1612 32  | 1503                          | 1523            | 15.07             | 0.09             | -16.62 | -19.16 | 1.69  | 04              |      |       |
| 1129 | PGC282435  | J030525.2-685614 | 1365 3   | 1160                          | 1141            | 14.93             | 0.17             | -16.22 | -18.76 | 1.43  | 02              |      |       |
| 1130 | ESO357-007 | J031024.3-330915 | 1117 3   | 1013                          | 1051            | 14.70             | 0.07             | -16.16 | -18.12 | 1.61  | 03              |      |       |
| 1131 | PGC707865  | J031615.3-311233 | 1112 50  | 1012                          | 1060            | 18.11             | 0.09             | -12.79 | -15.14 | 1.29  | 03              |      |       |
| 1132 | PGC2797190 | J032529.7+675312 | 1391 11  | 1613                          | 1692            | 99.99             | 3.36             | 99.99  | 99.99  | 1.68  | 06              |      |       |
| 1133 | PGC701288  | J032819.2-314611 | 869 89   | 757                           | 819             | 17.20             | 0.07             | -13.12 | -15.47 | 1.99  | 03              |      |       |
| 1134 | UGC02773   | J033207.3+474739 | 220 6    | 398                           | 159             | 14.85             | 2.45             | -14.29 | -17.13 | 1.46  | 08              |      |       |
| 1135 | IC1980     | J033659.0-575826 | 1452 27  | 1257                          | 1279            | 14.94             | 0.11             | -16.38 | -19.75 | 1.46  | 04              |      |       |
| 1136 | ESO054-021 | J034949.9-713805 | 1432 3   | 1208                          | 1206            | 12.78             | 0.22             | -18.53 | -21.15 | 1.34  | 24              |      |       |
| 1137 | PGC3313894 | J035549.5-493109 | 989 64   | 803                           | 868             | 17.45             | 0.03             | -12.96 | -15.31 | 1.74  | 02              | ++   |       |
| 1138 | ESO302-021 | J035552.6-404105 | 789 5    | 627                           | 705             | 15.61             | 0.04             | -14.35 | -17.38 | 1.15  | 10              |      |       |
| 1139 | UGC02890   | J035604.4+725518 | 1162 4   | 1380                          | 954             | 14.59             | 0.99             | -16.98 | -19.84 | 0.94  | 22              |      |       |
| 1140 | PGC014125  | J035605.6-492840 | 1005 41  | 819                           | 868             | 15.19             | 0.04             | -15.23 | -17.43 | 1.74  | 02              | ++   |       |
| 1141 | PGC383392  | J035849.3-575907 | 1469 123 | 1263                          | 1301            | 17.07             | 0.11             | -14.30 | -16.65 | 0.61  | 04              |      |       |
| 1142 | NGC1522    | J040608.0-524006 | 904 6    | 705                           | 763             | 13.97             | 0.06             | -16.19 | -18.37 | 1.73  | 02              |      |       |
| 1143 | ESO359-024 | J041057.5-354951 | 847 5    | 689                           | 794             | 15.43             | 0.05             | -14.80 | -17.25 | 1.45  | 10              |      |       |
| 1144 | ESO359-029 | J041250.6-330012 | 873 10   | 722                           | 742             | 14.83             | 0.08             | -15.28 | -16.58 | 1.97  | 10              |      |       |
| 1145 | NGC1556    | J041744.8-500952 | 985 4    | 785                           | 860             | 13.47             | 0.09             | -16.97 | -19.59 | 1.80  | 02              |      |       |
| 1146 | PGC103193  | J041907.6-453507 | 1406 39  | 1215                          | 1304            | 16.27             | 0.05             | -15.04 | -17.66 | 0.94  | 13              |      |       |
| 1147 | ESO251-003 | J042841.5-461916 | 1392 5   | 1194                          | 1289            | 16.21             | 0.05             | -15.08 | -17.43 | 1.24  | 13              |      |       |
| 1148 | PGC015315  | J042959.5-514154 | 1470 30  | 1259                          | 1340            | 14.59             | 0.05             | -16.78 | -20.30 | 1.17  | 13              |      |       |
| 1149 | PGC015535  | J043353.9-654153 | 1235 5   | 1002                          | 1040            | 16.00             | 0.18             | -14.95 | -17.30 | 1.34  | 02              |      |       |
| 1150 | PGC132228  | J043611.5-323739 | 1128 39  | 960                           | 1100            | 15.81             | 0.09             | -15.17 | -18.52 | 1.64  | 07              |      |       |
| 1151 | ESO551-020 | J043750.3-200354 | 1511 45  | 1383                          | 1544            | 15.57             | 0.17             | -16.22 | -18.30 | 1.45  | 07              |      |       |
| 1152 | ESO551-023 | J043831.4-195808 | 1493 45  | 1364                          | 1545            | 15.13             | 0.16             | -16.66 | -20.76 | 1.42  | 07              |      |       |
| 1153 | ESO202-048 | J043949.1-473138 | 1368 5   | 1160                          | 1262            | 14.84             | 0.04             | -16.39 | -18.72 | 1.79  | 13              |      |       |
| 1154 | NGC1679    | J044955.6-315756 | 1053 2   | 876                           | 1033            | 12.65             | 0.09             | -18.20 | -20.88 | 1.74  | 07              |      |       |
| 1155 | ESO552-031 | J045803.4-190726 | 1668 3   | 1525                          | 1721            | 16.57             | 0.18             | -15.48 | -18.33 | 1.90  | 07              |      |       |
| 1156 | NGC1809    | J050205.4-693404 | 1301 2   | 1057                          | 1093            | 13.20             | 1.03             | -18.71 | -20.04 | 1.53  | 24              |      |       |
| 1157 | NGC1853    | J051216.5-572357 | 1410 3   | 1169                          | 1260            | 13.74             | 0.08             | -17.52 | -20.80 | 1.25  | 13              |      |       |
| 1158 | PGC017965  | J055017.4-101753 | 898 3    | 745                           | 1013            | 17.40             | 3.54             | -16.85 | -20.97 | 1.88  | 07              | ++   |       |
| 1159 | PGC148081  | J055125.9-101444 | 864 6    | 710                           | 1014            | 16.51             | 3.89             | -18.09 | -20.46 | 1.82  | 07              | ++   |       |
| 1160 | PGC5057320 | J055204.6-110825 | 906 7    | 748                           | 1013            | 16.00             | 2.80             | -17.51 | 99.99  | 1.84  | 07              | ++   |       |
| 1161 | PGC018027  | J055209.3-110724 | 905 5    | 747                           | 1013            | 16.73             | 2.84             | -16.82 | -18.74 | 1.83  | 07              | ++   |       |
| 1162 | PGC148136  | J055802.3-125548 | 911 6    | 742                           | 1012            | 15.70             | 2.06             | -17.07 | -18.54 | 1.73  | 07              | ++   |       |
| 1163 | ESO488-053 | J055919.2-253218 | 1628 39  | 1419                          | 1659            | 17.59             | 0.14             | -14.33 | -16.78 | 1.48  | 11              |      |       |
| 1164 | PGC3097696 | J055921.0-130520 | 956 4    | 785                           | 1055            | 17.70             | 2.26             | -15.36 | -17.71 | 1.91  | 07              |      |       |
| 1165 | ESO555-039 | J060901.2-21-    |          |                               |                 |                   |                  |        |        |       |                 |      |       |

| (1)  | (2)                     | (3)              | (4)     | (5)  | (6)  | (7)   | (8)   | (9)    | (10)   | (11) | (12) | (13) |
|------|-------------------------|------------------|---------|------|------|-------|-------|--------|--------|------|------|------|
| 1170 | HIPASSJ0705-20          | J070545.5-205933 | 765 5   | 527  | 823  | 99.99 | 2.66  | 99.99  | 99.99  | 1.14 | 10   |      |
| 1171 | UGC03998                | J074521.3+560914 | 988 3   | 1078 | 1311 | 16.50 | 0.25  | -15.02 | -17.37 | 1.94 | 12   |      |
| 1172 | HIZOAJ0747-31           | J074741.8-310116 | 1603 14 | 1322 | 1599 | 99.99 | 4.12  | 99.99  | 99.99  | 1.90 | 13   |      |
| 1173 | ESO561-002              | J075525.6-212031 | 939 5   | 676  | 987  | 99.99 | 1.48  | 99.99  | 99.99  | 1.53 | 12   |      |
| 1174 | HIPASSJ0801-21          | J080125.2-215956 | 734 8   | 468  | 778  | 99.99 | 1.09  | 99.99  | 99.99  | 1.54 | 08   |      |
| 1175 | UGC04173                | J080711.1+800734 | 860 2   | 1056 | 1162 | 14.64 | 0.12  | -16.59 | -17.30 | 1.60 | 22   |      |
| 1176 | ESO035-021              | J080955.4-743041 | 1241 5  | 964  | 1014 | 17.17 | 0.78  | -14.33 | -16.68 | 1.65 | 24   |      |
| 1177 | PGC023301               | J081839.5-252309 | 1140 54 | 860  | 1160 | 99.99 | 0.63  | 99.99  | -19.68 | 1.43 | 14   |      |
| 1178 | UGC04426                | J082828.5+415124 | 396 2   | 400  | 720  | 15.17 | 0.16  | -14.96 | -17.61 | 1.70 | 09   |      |
| 1179 | ESO431-015              | J083302.0-302347 | 1127 5  | 833  | 1114 | 16.13 | 0.73  | -15.52 | -17.55 | 1.51 | 14   |      |
| 1180 | PGC023999               | J083324.3+544620 | 740 1   | 813  | 1055 | 16.51 | 0.19  | -14.48 | -16.83 | 1.37 | 09   |      |
| 1181 | UGC04454                | J083721.4+803253 | 869 21  | 1065 | 1169 | 15.56 | 0.09  | -15.55 | -17.23 | 1.93 | 22   |      |
| 1182 | ESO090-004              | J083837.1-642032 | 1878 6  | 1579 | 1690 | 15.10 | 0.67  | -17.39 | 99.99  | 1.62 | 13   |      |
| 1183 | ESO036-006              | J083847.0-750911 | 1141 3  | 863  | 909  | 14.29 | 0.56  | -16.75 | -19.10 | 1.91 | 24   |      |
| 1184 | ESO496-010              | J084906.0-261918 | 809 9   | 520  | 627  | 14.83 | 0.43  | -15.27 | -18.62 | 1.55 | 08   |      |
| 1185 | PGC1094087              | J085100.2-022201 | 1587 39 | 1369 | 1718 | 16.63 | 0.08  | -15.30 | -16.87 | 0.79 | 12   |      |
| 1186 | ESO090-015              | J090205.6-645416 | 1677 3  | 1377 | 1483 | 13.90 | 0.80  | -18.44 | -21.56 | 1.79 | 13   |      |
| 1187 | PGC086668               | J090253.7+200430 | 484 3   | 366  | 645  | 17.12 | 0.12  | -12.74 | -15.09 | 1.64 | 08   |      |
| 1188 | PGC2806961              | J090853.7+143458 | 335 4   | 189  | 700  | 18.01 | 0.17  | -12.06 | -14.41 | 1.57 | 08   |      |
| 1189 | SDSSJ091018.20+583602.5 | J091018.2+583602 | 1186 5  | 1275 | 1495 | 19.15 | 0.16  | -12.56 | -14.82 | 1.92 | 12   |      |
| 1190 | SDSSJ092114.98+094352.2 | J092115.0+094352 | 1382 4  | 1212 | 1557 | 17.98 | 0.20  | -13.87 | -17.97 | 1.72 | 12   |      |
| 1191 | PGC686082               | J092203.3-324717 | 1094 8  | 789  | 1052 | 17.04 | 0.81  | -14.56 | -16.91 | 1.32 | 13   |      |
| 1192 | NGC2883                 | J092518.4-340612 | 1180 3  | 873  | 1129 | 13.65 | 0.96  | -18.25 | -20.51 | 1.76 | 13   |      |
| 1193 | [PT2011]53              | J092610.1+334312 | 532 4   | 484  | 792  | 17.33 | 0.08  | -12.92 | -15.27 | 1.92 | 12   |      |
| 1194 | NGC2915                 | J092611.8-763735 | 465 3   | 189  | 313  | 13.19 | 1.19  | -16.16 | -18.56 | 1.85 | 10   |      |
| 1195 | ESO373-001              | J092650.1-324748 | 1186 8  | 881  | 1142 | 16.40 | 0.61  | -15.18 | -17.65 | 1.73 | 13   |      |
| 1196 | ESO434-005              | J092725.5-320036 | 1086 5  | 782  | 1046 | 15.24 | 0.56  | -16.11 | -18.46 | 0.99 | 13   |      |
| 1197 | ESO373-006              | J093150.1-340816 | 1045 8  | 738  | 991  | 16.30 | 0.68  | -15.04 | -16.28 | 1.25 | 13   |      |
| 1198 | PGC027157               | J093343.1+333601 | 1566 1  | 1517 | 1823 | 15.68 | 0.08  | -16.39 | -18.08 | 1.71 | 12   |      |
| 1199 | UGC05105                | J093520.0+355449 | 1543 8  | 1507 | 1806 | 16.31 | 0.07  | -15.73 | -18.08 | 1.78 | 12   |      |
| 1200 | 6dFJ0935...             | J093521.6-134852 | 800 44  | 538  | 853  | 16.43 | 0.19  | -14.10 | -16.45 | 1.94 | 12   |      |
| 1201 | PGC027591               | J094012.8+293530 | 502 1   | 432  | 745  | 16.32 | 0.08  | -13.80 | -16.15 | 1.47 | 12   |      |
| 1202 | UGC05151                | J094027.0+482016 | 771 1   | 803  | 1059 | 13.85 | 0.10  | -17.06 | -19.41 | 1.06 | 12   |      |
| 1203 | IC0549                  | J094043.2+035733 | 1301 14 | 1104 | 1440 | 15.17 | 0.17  | -16.47 | -18.95 | 1.40 | 12   |      |
| 1204 | PGC1137164              | J094446.2-004118 | 1228 1  | 1012 | 1342 | 16.44 | 0.28  | -15.17 | -17.52 | 1.84 | 14   |      |
| 1205 | UGC05245                | J094734.4-020159 | 1416 4  | 1194 | 1522 | 15.41 | 0.19  | -16.37 | -19.00 | 1.69 | 14   |      |
| 1206 | SDSSJ094847.46+275225.4 | J094847.5+275225 | 1317 2  | 1237 | 1549 | 17.14 | 0.11  | -14.60 | -18.70 | 1.66 | 12   |      |
| 1207 | PGC028311               | J095017.0+271818 | 1427 2  | 1344 | 1656 | 17.58 | 0.10  | -14.30 | -15.56 | 1.98 | 12   |      |
| 1208 | SDSSJ095729.39+274524.3 | J095729.4+274524 | 1182 2  | 1102 | 1409 | 18.10 | 0.08  | -13.41 | -15.76 | 1.88 | 12   |      |
| 1209 | UGC05373                | J100000.0-051956 | 301 1   | 111  | 111  | 11.92 | 0.13  | -14.13 | -15.54 | 1.16 | 08   |      |
| 1210 | PGC028991               | J100107.0+365522 | 1458 1  | 1428 | 1754 | 16.89 | 0.05  | -15.06 | -17.41 | 1.68 | 12   | ++   |
| 1211 | PGC090975               | J100110.1+005431 | 1266 8  | 1057 | 1379 | 17.69 | 0.10  | -13.79 | -16.72 | 1.21 | 12   |      |
| 1212 | PGC029004               | J100114.4+370415 | 1467 1  | 1438 | 1753 | 16.81 | 0.06  | -15.16 | -17.66 | 1.74 | 12   | ++   |
| 1213 | UGC05391                | J100141.2+371452 | 1568 5  | 1540 | 1753 | 15.17 | 0.07  | -16.80 | -18.26 | 1.82 | 12   |      |
| 1214 | UGC05394                | J100147.9+362955 | 1431 2  | 1399 | 1684 | 16.16 | 0.06  | -15.72 | -18.75 | 1.70 | 12   |      |
| 1215 | NGC3109                 | J100306.9-260934 | 403 2   | 110  | 81   | 10.39 | 0.29  | -15.13 | -15.56 | 1.04 | 10   | ++   |
| 1216 | PGC029194               | J100404.0-271955 | 361 3   | 66   | 66   | 15.78 | 0.34  | -9.33  | -12.07 | 0.86 | 10   | ++   |
| 1217 | NGC3118                 | J100711.5+330139 | 1337 2  | 1286 | 1577 | 14.37 | 0.08  | -17.39 | -19.77 | 1.79 | 12   |      |
| 1218 | UGC05456                | J100719.5+102146 | 541 2   | 374  | 779  | 13.74 | 0.17  | -16.58 | -18.52 | 1.69 | 12   |      |
| 1219 | UGC05460                | J100809.2+515040 | 1095 4  | 1147 | 1379 | 14.33 | 0.05  | -17.10 | -20.02 | 1.64 | 12   |      |
| 1220 | PGC029653               | J101100.8-044134 | 324 1   | 94   | 94   | 12.32 | 0.19  | -13.42 | -15.77 | 1.01 | 08   | ++   |
| 1221 | AGC208583               | J102144.8+180520 | 264 4   | 137  | 137  | 17.36 | 0.11  | -9.11  | -11.46 | 1.43 | 08   | ++   |
| 1222 | PGC083041               | J102902.8-354029 | 1865 25 | 1559 | 1777 | 17.89 | 0.34  | -14.38 | -18.48 | 1.64 | 13   |      |
| 1223 | ESO214-018              | J104054.1-482539 | 1014 10 | 703  | 880  | 99.99 | 1.23  | 99.99  | -17.38 | 1.13 | 13   |      |
| 1224 | ESO501-079              | J104126.0-232303 | 1196 4  | 914  | 1162 | 14.21 | 0.19  | -16.99 | -21.86 | 1.44 | 14   |      |
| 1225 | PGC096512               | J113447.0-591346 | 1433 19 | 1137 | 1218 | 99.99 | 3.25  | 99.99  | -21.29 | 1.86 | 13   |      |
| 1226 | HIZOAJ1149-62           | J114938.4-621102 | 512 14  | 221  | 221  | 99.99 | 26.32 | 99.99  | 99.99  | 0.91 | 10   |      |
| 1227 | ESO039-002              | J115020.6-752215 | 1828 4  | 1557 | 1567 | 13.84 | 1.76  | -19.58 | -18.70 | 1.08 | 15   |      |
| 1228 | UGC06817                | J115053.0+385249 | 248 1   | 254  | 193  | 13.46 | 0.11  | -13.76 | -15.26 | 1.86 | 08   |      |
| 1229 | HIZOAJ1209-62           | J120920.8-622913 | 1449 14 | 1164 | 1212 | 99.99 | 17.30 | 99.99  | 99.99  | 1.32 | 15   |      |
| 1230 | PGC039849               | J122043.9+143752 | 596 4   | 496  | 496  | 16.84 | 0.16  | -12.48 | -14.83 | 1.91 | 18   |      |
| 1231 | NGC4826                 | J122844.1+224915 | 643 2   | 587  | 482  | 13.12 | 0.09  | -16.07 | -18.56 | 1.50 | 18   | ++   |
| 1232 | AGC229379               | J123034.0+231220 | 624 8   | 571  | 748  | 18.68 | 0.08  | -11.45 | 99.99  | 1.90 | 18   | ++   |
| 1233 | NGC4437                 | J123245.5+000652 | 1128 2  | 971  | 610  | 11.19 | 0.10  | -18.53 | -22.00 | 1.98 | 18   |      |
| 1234 | PGC2687514              | J124644.2+662757 | 1446 2  | 1601 | 1700 | 18.52 | 0.11  | -13.42 | -17.52 | 1.36 | 17   |      |
| 1235 | UGC07990                | J125027.2+282110 | 516 10  | 500  | 500  | 16.60 | 0.06  | -12.63 | -14.98 | 1.73 | 18   |      |
| 1236 | SDSSJ125133.00+194322.9 | J125133.0+194323 | 1152 1  | 1095 | 1238 | 17.02 | 0.09  | -14.21 | -16.56 | 1.35 | 16   |      |
| 1237 | UGC08011                | J125221.1+213747 | 765 3   | 718  | 860  | 16.04 | 0.16  | -14.48 | -16.83 | 0.86 | 18   | ++   |
| 1238 | NGC4757                 | J125250.1-101836 | 847 51  | 664  | 788  | 15.00 | 0.18  | -15.34 | -19.74 | 1.73 | 18   |      |
| 1239 | SDSSJ125259.05+222455.8 | J125259.1+222456 | 749 2   | 705  | 846  | 17.21 | 0.14  | -13.25 | -15.60 | 0.81 | 18   | ++   |
| 1240 | PGC043851               | J125356.8-120621 | 823 2   | 635  | 755  | 14.86 | 0.24  | -15.45 | -17.80 | 1.31 | 18   |      |
| 1241 | PGC430271               | J125503.1-532423 | 1992 58 | 1720 | 1761 | 16.97 | 1.54  | -16.48 | -19.46 | 1.61 | 15   |      |
| 1242 | UGC08091                | J125840.2+141303 | 217 2   | 140  | 153  | 14.70 | 0.11  | -12.02 | -14.37 | 1.74 | 21   |      |
| 1243 | PGC044532               | J125901.8+345139 | 837 4   | 856  | 727  | 12.86 | 0.05  | -17.18 | -19.53 | 1.54 | 18   |      |
| 1244 | PGC044982               | J130214.4-171416 | 749 2   | 549  | 425  | 15.08 | 0.35  | -15.01 | -17.63 | 1.69 | 21   | ++   |
| 1245 | KK177                   | J130241.8+215953 | 267 60  | 228  | 352  | 16.62 | 0.16  | -11.96 | -16.06 | 0.46 | 20   |      |
| 1246 | PGC045084               | J130316.8-172523 | 744 2   | 544  | 425  | 13.48 | 0.34  | -15.76 | -18.95 | 1.67 | 18   | ++   |
| 1247 | PGC1709453              | J130336.8+243133 | 834 2   | 808  | 934  | 16.31 | 0.07  | -14.30 | -17.15 | 0.99 | 20   |      |
| 1248 | PGC1832164              | J130402.7+281833 | 740 4   | 732  | 857  | 17.06 | 0.04  | -13.33 | -15.68 | 0.92 | 20   |      |
| 1249 | PGC045416               | J130656.0+144827 | 971 3   | 901  | 1022 | 16.24 | 0.11  | -14.60 | -16.95 | 1.95 | 20   |      |
| 1250 | PGC045512               | J130756.7-164121 | 955 8   | 761  | 855  | 14.79 | 0.35  | -15.90 | -17.82 | 1.80 | 21   |      |
| 1251 | [STE2000]B13...         | J130812.3+290517 | 827 6   | 825  | 944  | 17.70 | 0.04  | -12.90 | 99.99  | 1.44 | 20   |      |
| 1252 | PGC045858               | J131217.7+264109 | 792 7   | 781  | 896  | 14.53 | 0.06  | -15.98 | -19.21 | 1.09 | 20   |      |
| 1253 | AGC239104               | J131318.8+312449 | 800 8   | 812  | 924  | 19.00 | 0.05  | -11.56 | 99.99  | 1.77 | 20   |      |

| (1)  | (2)                     | (3)              | (4)     | (5)  | (6)  | (7)   | (8)   | (9)    | (10)   | (11) | (12) | (13) |
|------|-------------------------|------------------|---------|------|------|-------|-------|--------|--------|------|------|------|
| 1254 | PGC200295               | J131410.8+390855 | 1148 1  | 1195 | 1303 | 15.72 | 0.06  | -15.60 | -18.62 | 1.99 | 16   |      |
| 1255 | NGC5068                 | J131854.9-210221 | 671 2   | 471  | 376  | 10.64 | 0.44  | -18.36 | -20.76 | 0.90 | 18   | ++   |
| 1256 | SDSSJ132047.16+220216.5 | J132047.2+220217 | 789 1   | 763  | 866  | 18.04 | 0.08  | -12.42 | -14.77 | 1.63 | 20   |      |
| 1257 | PGC169720               | J132500.1-242523 | 1594 31 | 1389 | 1448 | 16.82 | 0.38  | -15.05 | -18.46 | 1.59 | 19   |      |
| 1258 | PGC952909               | J132509.5-122544 | 1170 5  | 1003 | 1065 | 16.03 | 0.19  | -14.99 | -17.84 | 1.50 | 21   |      |
| 1259 | PGC135826               | J132616.1+022732 | 1029 4  | 921  | 1007 | 16.80 | 0.11  | -14.00 | -16.35 | 1.94 | 18   | ++   |
| 1260 | NGC5147                 | J132619.7+020602 | 1090 2  | 980  | 1066 | 12.28 | 0.12  | -18.66 | -21.11 | 1.81 | 18   | ++   |
| 1261 | ESO576-059              | J132635.1-221417 | 1426 5  | 1228 | 1288 | 15.37 | 0.34  | -16.20 | -18.55 | 1.73 | 19   |      |
| 1262 | UGC08450                | J132701.2+100321 | 1050 2  | 974  | 1073 | 16.15 | 0.12  | -14.80 | -17.15 | 1.45 | 20   |      |
| 1263 | PGC047160               | J132724.6+452619 | 1263 1  | 1347 | 1438 | 16.19 | 0.08  | -15.37 | -18.02 | 0.91 | 17   |      |
| 1264 | AGC233559               | J132847.3+105741 | 1092 5  | 1022 | 1110 | 19.12 | 0.18  | -11.97 | 99.99  | 1.10 | 20   |      |
| 1265 | UGC08489                | J132938.7+452316 | 1293 1  | 1378 | 1466 | 14.61 | 0.07  | -16.98 | -18.02 | 1.19 | 17   | ++   |
| 1266 | SDSSJ133108.40+445407.3 | J133108.4+445408 | 1303 2  | 1386 | 1473 | 18.35 | 0.06  | -13.23 | -17.33 | 1.20 | 17   | ++   |
| 1267 | UGC08538                | J133314.7+455014 | 1330 2  | 1418 | 1503 | 16.84 | 0.08  | -14.81 | -17.71 | 1.73 | 17   | ++   |
| 1268 | UGC08542                | J133331.8+383620 | 1190 4  | 1247 | 1333 | 15.86 | 0.03  | -15.48 | -18.05 | 1.85 | 16   |      |
| 1269 | UGC08588                | J133542.7+455546 | 1446 4  | 1536 | 1618 | 15.35 | 0.08  | -16.45 | -18.88 | 1.05 | 17   |      |
| 1270 | UGC08638                | J133919.3+244629 | 275 1   | 274  | 313  | 14.48 | 0.06  | -13.73 | -16.63 | 1.30 | 20   |      |
| 1271 | UGC08651                | J133953.8+404421 | 202 2   | 272  | 227  | 14.62 | 0.03  | -12.87 | -15.61 | 1.39 | 21   |      |
| 1272 | SDSSJ134715.99+131037.8 | J134716.0+131038 | 1101 2  | 1055 | 1117 | 18.25 | 0.09  | -12.76 | -15.11 | 1.48 | 20   |      |
| 1273 | PGC166177               | J134731.2+392229 | 1276 6  | 1345 | 1415 | 17.30 | 0.04  | -14.18 | -16.65 | 1.93 | 16   |      |
| 1274 | PGC947953               | J134909.3-124545 | 1394 6  | 1244 | 1283 | 16.42 | 0.31  | -15.11 | -15.93 | 1.88 | 19   |      |
| 1275 | UGC08756                | J135035.9+423229 | 1327 5  | 1411 | 1477 | 14.50 | 0.06  | -17.09 | -21.10 | 1.93 | 16   |      |
| 1276 | ESO383-092              | J135042.0-355454 | 1410 4  | 1193 | 1204 | 15.41 | 0.33  | -16.01 | -18.72 | 1.78 | 19   |      |
| 1277 | UGC08760                | J135051.2+380116 | 191 2   | 256  | 240  | 14.49 | 0.07  | -13.16 | -15.51 | 1.34 | 21   |      |
| 1278 | UGC08833                | J135448.5+355016 | 224 2   | 283  | 232  | 15.30 | 0.05  | -12.26 | -15.20 | 1.48 | 21   |      |
| 1279 | ESO510-015              | J135503.3-231252 | 1364 8  | 1185 | 1204 | 16.47 | 0.33  | -14.95 | -18.22 | 1.97 | 19   |      |
| 1280 | SDSSJ135737.29+392853.5 | J135737.3+392854 | 1381 6  | 1457 | 1515 | 17.20 | 0.09  | -14.47 | -16.82 | 1.84 | 16   | ++   |
| 1281 | PGC2152660              | J140357.3+393604 | 1397 3  | 1477 | 1528 | 17.24 | 0.04  | -14.40 | -16.75 | 1.36 | 16   | ++   |
| 1282 | PGC1383447              | J140704.4+104245 | 1183 1  | 1143 | 1173 | 17.39 | 0.10  | -13.74 | -16.09 | 1.80 | 20   |      |
| 1283 | PGC166185               | J140710.4+350340 | 62 2    | 126  | 148  | 17.23 | 0.06  | -9.37  | -12.00 | 1.68 | 21   |      |
| 1284 | AGC243830               | J141443.5+100429 | 1218 4  | 1181 | 1199 | 99.99 | 0.10  | 99.99  | 99.99  | 1.92 | 20   |      |
| 1285 | UGC09128                | J141556.5+230320 | 153 2   | 172  | 166  | 14.56 | 0.10  | -12.32 | -14.67 | 1.97 | 21   |      |
| 1286 | AGC243881               | J141750.7+065023 | 1248 4  | 1200 | 1211 | 17.45 | 0.14  | -13.79 | 99.99  | 1.63 | 20   |      |
| 1287 | ESO222-004              | J142340.2-493918 | 1556 3  | 1332 | 1295 | 99.99 | 1.37  | 99.99  | 99.99  | 1.80 | 15   |      |
| 1288 | ESO222-012              | J143918.6-521333 | 1508 10 | 1288 | 1235 | 15.64 | 2.33  | -17.83 | -21.04 | 1.63 | 15   |      |
| 1289 | PGC052413               | J144015.2-061146 | 1739 64 | 1658 | 1624 | 15.44 | 0.27  | -16.57 | -19.12 | 1.64 | 19   |      |
| 1290 | ESO327-014              | J144254.8-380051 | 1236 5  | 1050 | 995  | 16.36 | 0.37  | -14.68 | -17.53 | 1.70 | 19   |      |
| 1291 | SDSSJ144303.81+535457.5 | J144303.8+535457 | 838 52  | 995  | 1012 | 17.67 | 0.05  | -13.09 | -15.44 | 1.28 | 20   |      |
| 1292 | PGC3076856              | J145112.7-501240 | 1276 5  | 1067 | 1003 | 15.26 | 1.37  | -16.80 | -17.46 | 1.82 | 21   |      |
| 1293 | SDSSJ145808.78+064447.4 | J145808.8+064448 | 1666 2  | 1653 | 1608 | 18.24 | 0.14  | -13.61 | -15.96 | 1.97 | 16   | ++   |
| 1294 | PGC053512               | J145837.9+064631 | 1676 1  | 1664 | 1607 | 16.10 | 0.13  | -15.75 | -18.35 | 1.98 | 16   | ++   |
| 1295 | ESO274-001              | J151413.4-464833 | 523 2   | 336  | 208  | 11.72 | 1.09  | -16.64 | -18.89 | 1.15 | 21   |      |
| 1296 | HIPASSJ1534-56          | J153422.5-562813 | 1555 8  | 1357 | 1257 | 99.99 | 47.64 | 99.99  | 99.99  | 1.85 | 15   |      |
| 1297 | NGC5964                 | J153736.2+055826 | 1447 3  | 1468 | 1350 | 13.61 | 0.26  | -17.98 | -20.85 | 1.30 | 20   |      |
| 1298 | UGC10031                | J154545.5+613321 | 889 4   | 1096 | 1075 | 17.00 | 0.06  | -13.90 | -16.30 | 1.67 | 22   |      |
| 1299 | PGC3097722              | J160540.8-043419 | 1612 4  | 1616 | 1458 | 18.20 | 1.21  | -14.51 | -16.86 | 1.67 | 19   |      |
| 1300 | UGC10229                | J160944.0-000655 | 1505 2  | 1531 | 1370 | 15.74 | 0.52  | -16.14 | -16.85 | 1.41 | 20   |      |
| 1301 | AGC268216               | J161220.5+063237 | 1723 4  | 1778 | 1620 | 17.68 | 0.23  | -14.28 | 99.99  | 1.85 | 20   |      |
| 1302 | PGC2801026              | J161347.7+542215 | -75 10  | 132  | 140  | 16.73 | 0.04  | -9.72  | -12.07 | 1.67 | 21   |      |
| 1303 | PGC264615               | J161354.9-721446 | 383 11  | 170  | 170  | 17.94 | 0.38  | -9.28  | -11.63 | 1.12 | 21   |      |
| 1304 | PGC058114               | J162604.3+025424 | 1536 4  | 1589 | 1409 | 15.20 | 0.29  | -16.52 | -21.11 | 1.80 | 20   |      |
| 1305 | PGC058179               | J162721.0-602731 | 1155 4  | 974  | 842  | 14.00 | 0.87  | -17.18 | -16.93 | 1.34 | 21   |      |
| 1306 | NGC6237                 | J164622.0+702132 | 1132 3  | 1371 | 1344 | 14.29 | 0.15  | -17.19 | -17.90 | 1.75 | 17   |      |
| 1307 | PGC3082691              | J164819.4-103139 | 1579 6  | 1597 | 1380 | 16.10 | 3.28  | -18.56 | -19.83 | 1.91 | 19   |      |
| 1308 | UGC10554                | J164821.3-013708 | 1562 4  | 1617 | 1404 | 15.58 | 0.83  | -16.68 | -19.14 | 1.26 | 20   |      |
| 1309 | UGC10636                | J165619.4+702648 | 1326 4  | 1569 | 1538 | 16.57 | 0.19  | -15.24 | -17.59 | 1.40 | 17   |      |
| 1310 | HIPASSJ1700-07          | J170008.1-072323 | 1556 6  | 1598 | 1368 | 99.99 | 2.40  | 99.99  | 99.99  | 1.73 | 21   |      |
| 1311 | HIPASSJ1721-21          | J172152.0-212137 | 351 8   | 350  | 100  | 99.99 | 3.32  | 99.99  | 99.99  | 1.37 | 21   |      |
| 1312 | PGC365379               | J173100.2-601138 | 1565 8  | 1412 | 1242 | 17.22 | 0.37  | -14.31 | -16.91 | 1.46 | 24   |      |
| 1313 | IC4662                  | J174709.1-643824 | 306 3   | 143  | 186  | 11.82 | 0.30  | -15.51 | -17.55 | 1.32 | 21   |      |
| 1314 | UGC111030               | J175434.2+025251 | 1757 2  | 1886 | 1605 | 15.11 | 0.83  | -17.43 | -20.68 | 1.73 | 21   |      |
| 1315 | HIZOAJ1827-06A          | J182733.1-064933 | 1738 14 | 1851 | 1536 | 99.99 | 7.73  | 99.99  | 99.99  | 1.96 | 21   | ++   |
| 1316 | HIPASSJ1827-06          | J182736.3-062724 | 1740 8  | 1855 | 1540 | 99.99 | 6.95  | 99.99  | 99.99  | 1.84 | 21   | ++   |
| 1317 | HIZOAJ1832-03           | J183223.1-032150 | 1704 14 | 1835 | 1518 | 99.99 | 10.94 | 99.99  | 99.99  | 1.82 | 21   |      |
| 1318 | HIPASSJ1905-67          | J190539.5-670731 | 411 8   | 261  | 261  | 99.99 | 0.26  | 99.99  | 99.99  | 1.67 | 21   | ++   |
| 1319 | UGC11411                | J190842.4+701702 | 69 32   | 345  | 480  | 15.27 | 0.51  | -14.33 | -15.37 | 1.56 | 22   |      |
| 1320 | HIPASSJ1913-67          | J191253.3-670554 | 426 6   | 277  | 277  | 99.99 | 0.30  | 99.99  | 99.99  | 1.81 | 21   | ++   |
| 1321 | PGC063556               | J194311.8-065621 | 1501 9  | 1657 | 1320 | 14.34 | 1.27  | -18.22 | -20.69 | 1.07 | 21   | ++   |
| 1322 | NGC6821                 | J194424.1-065000 | 1523 5  | 1680 | 1320 | 13.62 | 1.37  | -19.03 | -21.25 | 1.11 | 21   | ++   |
| 1323 | UGC11539                | J201831.4+624128 | 1392 10 | 1691 | 1569 | 14.97 | 0.84  | -17.53 | -21.81 | 1.66 | 22   |      |
| 1324 | UGC11707                | J211431.8+264405 | 906 2   | 1200 | 913  | 14.50 | 0.71  | -16.69 | -18.16 | 1.77 | 25   |      |
| 1325 | UGC11771                | J213527.5+232806 | 1662 4  | 1951 | 1661 | 16.64 | 0.44  | -15.58 | -18.68 | 1.91 | 23   |      |
| 1326 | ESO146-002A             | J215755.5-601828 | 1686 3  | 1589 | 1389 | 16.39 | 0.15  | -15.16 | -17.51 | 1.07 | 24   |      |
| 1327 | IC1420                  | J220231.6+194501 | 1633 24 | 1911 | 1521 | 14.35 | 0.34  | -17.58 | -20.51 | 0.81 | 23   |      |
| 1328 | ESO601-014              | J220415.3-200246 | 1772 4  | 1892 | 1582 | 16.93 | 0.12  | -14.87 | -17.22 | 1.93 | 21   |      |
| 1329 | IC5162                  | J220803.2-524251 | 1736 6  | 1679 | 1451 | 15.03 | 0.16  | -16.62 | -19.29 | 1.77 | 21   |      |
| 1330 | UGC12029                | J222447.7+225818 | 1250 3  | 1533 | 1271 | 17.00 | 0.24  | -14.44 | -16.79 | 1.63 | 25   |      |
| 1331 | ESO468-020              | J224043.8-304758 | 92 5    | 150  | 165  | 15.89 | 0.06  | -10.94 | -15.04 | 1.95 | 21   |      |
| 1332 | PGC069702               | J224700.4+215345 | 1405 2  | 1682 | 1435 | 15.64 | 0.21  | -16.04 | -17.95 | 1.31 | 01   |      |
| 1333 | AGC322482               | J225210.4+210104 | 1422 8  | 1695 | 1450 | 17.66 | 0.44  | -14.27 | 99.99  | 1.84 | 01   |      |
| 1334 | AGC321194               | J225704.0+254330 | 1050 4  | 1333 | 1105 | 17.43 | 0.69  | -14.16 | 99.99  | 1.66 | 25   |      |
| 1335 | UGC12340                | J230433.8+270921 | 1056 2  | 1340 | 1123 | 15.75 | 0.27  | -15.46 | -18.06 | 1.65 | 25   |      |
| 1336 | PGC749455               | J231758.1-274907 | 750 54  | 813  | 567  | 18.41 | 0.10  | -11.14 | -13.49 | 1.64 | 02   |      |
| 1337 | PGC5065954              | J232554.2+183245 | 1507 6  | 1763 | 1545 | 17.49 | 0.19  | -14.33 | 99.99  | 1.71 | 01   |      |



| (1)  | (2)           | (3)              | (4)     | (5)  | (6)  | (7)   | (8)  | (9)    | (10)   | (11) | (12) | (13) |
|------|---------------|------------------|---------|------|------|-------|------|--------|--------|------|------|------|
| 1338 | AGC335244     | J233055.1+181236 | 1499 8  | 1752 | 1538 | 18.40 | 0.29 | -13.51 | 99.99  | 1.93 | 01   |      |
| 1339 | IC5332        | J233427.5-360605 | 704 3   | 719  | 479  | 11.31 | 0.07 | -17.85 | -20.00 | 1.79 | 02   | ++   |
| 1340 | NGC7713       | J233615.0-375618 | 693 3   | 697  | 484  | 11.49 | 0.07 | -17.69 | -19.92 | 1.92 | 02   | ++   |
| 1341 | ESO347-029    | J233626.6-384703 | 1568 4  | 1568 | 1357 | 13.66 | 0.08 | -17.76 | -20.39 | 1.61 | 04   |      |
| 1342 | PGC071920     | J233705.7-093553 | 1781 6  | 1926 | 1689 | 15.94 | 0.12 | -16.00 | -18.35 | 1.83 | 25   |      |
| 1343 | ESO240-012    | J233849.6-515135 | 1855 6  | 1786 | 1608 | 14.36 | 0.07 | -17.42 | -20.19 | 1.75 | 04   | ++   |
| 1344 | PGC129996     | J233941.2-514255 | 1964 45 | 1896 | 1717 | 15.66 | 0.05 | -16.25 | -18.34 | 1.05 | 04   | ++   |
| 1345 | PGC3192333    | J234133.8-353023 | 630 89  | 645  | 485  | 18.86 | 0.06 | -10.31 | -12.66 | 1.62 | 02   | ++   |
| 1346 | PGC680341     | J234147.5-330841 | 510 89  | 537  | 322  | 16.59 | 0.05 | -11.69 | -14.04 | 1.38 | 21   |      |
| 1347 | 6dFJ2343...   | J234304.1-513141 | 1949 45 | 1881 | 1704 | 99.99 | 0.06 | 99.99  | 99.99  | 1.22 | 04   |      |
| 1348 | UGC12771      | J234532.8+171513 | 1291 3  | 1535 | 1336 | 16.48 | 0.25 | -15.08 | -17.43 | 1.99 | 25   |      |
| 1349 | PGC2807157    | J234534.4+384304 | -134 2  | 154  | 186  | 16.70 | 0.53 | -10.86 | -13.26 | 1.97 | 21   |      |
| 1350 | ESO149-001    | J234748.7-570421 | 1901 16 | 1804 | 1646 | 13.53 | 0.07 | -18.30 | -20.90 | 1.74 | 04   |      |
| 1351 | PGC582812     | J234824.9-404522 | 1578 45 | 1563 | 1367 | 16.91 | 0.05 | -14.50 | -18.72 | 1.70 | 04   |      |
| 1352 | ESO348-009    | J234923.4-374623 | 647 2   | 648  | 447  | 14.81 | 0.06 | -14.18 | -16.53 | 1.97 | 02   |      |
| 1353 | NGC7764       | J235053.8-404349 | 1693 15 | 1678 | 1484 | 12.64 | 0.07 | -18.97 | -21.24 | 1.55 | 04   |      |
| 1354 | 2MASXJ2355... | J235531.7-555413 | 1866 67 | 1772 | 1616 | 99.99 | 0.06 | 99.99  | -18.87 | 1.99 | 04   |      |

**J001648.2+122100:** pair with J001745.5+112701

**J001745.5+112701:** pair with J001648.2+122100

**J014755.3-265332:** triplet with J014839.3-264518 and J014849.5-270828

**J014839.3-264518:** triplet with J014755.3-265332 and J014849.5-270828

**J014849.5-270828:** triplet with J014755.3-265332 and J014839.3-264518

**J035549.5-493109:** pair with J035605.6-492840

**J035605.6-492840:** pair with J035549.5-493109

**J055017.4-101753:** main galaxy of quintet with J055125.9-101444, J055204.6-110825, J055209.3-110724, J055802.3-125548

**J055125.9-101444:** member of the same quintet

**J055204.6-110825:** member of the same quintet

**J055209.3-110724:** member of the same quintet

**J055802.3-125548:** member of the same quintet

**J100000.0+051956 (SEXTANSB):** member of group NGC3109 (J100306.9-260934)

**J100107.0+365522:** pair with J100114.4+370415

**J100114.4+370415:** pair with J100107.0+365522

**J100306.9-260934 (NGC3109):** main galaxy of group with SEXTANSB, ANTLIA, SEXTANSA, Leo P

**J100404.0-271955 (ANTLIA):** member of group NGC3109

**J101100.8-044134 (SEXTANSA):** member of group NGC3109

**J102144.8+180520 (Leo P):** member of group NGC3109

**J122844.1+224915:** pair with J123034.0+231220?

**J123034.0+231220:** pair with J122844.1+224915?

**J125221.1+213747:** pair with J125146.0+214403 and J125259.1+222456?

**J125259.1+222456:** pair with J125146.0+214403 and J125221.1+213747?

**J130214.4-171416:** triplet with J130316.8-172523 and J131854.9-210221

**J130316.8-172523:** triplet with J130214.4-171416 and J131854.9-210221

**J131854.9-210221:** triplet with J130214.4-171416 and J130316.8-172523

**J132616.1+022732:** pair with J132619.7+020602

**J132619.7+020602:** pair with J132616.1+022732

**J132938.7+452316:** triplet with J133108.4+445408 and J133314.7+455014?

**J133108.4+445408:** triplet with J132938.7+452316 and J133314.7+455014?

**J133314.7+455014:** triplet with J132938.7+452316 and J133108.4+445408?

**J135737.3+392854:** pair with J140357.3+393604

**J140357.3+393604:** pair with J135737.3+392854

**J145808.8+064448:** pair with J145837.9+064631

**J145837.9+064631:** pair with J145808.8+064448

**J182733.1-064933:** pair with J182736.3-062724

**J182736.3-062724:** pair with J182733.1-064933

**J190539.5-670731:** pair with J191253.3-670554

**J191253.3-670554:** pair with J190539.5-670731

**J194311.8-065621:** pair with J194424.1-065000

**J194424.1-065000:** pair with J194311.8-065621

**J233427.5-360605:** triplet with J233615.0-375618 and J234133.8-353023

**J233615.0-375618:** triplet with J233427.5-360605 and J234133.8-353023

**J234133.8-353023:** triplet with J233427.5-360605 and J233615.0-375618

**J233849.6-515135:** pair with J233941.2-514255?

**J233941.2-514255:** pair with J233849.6-515135?

## A2 3D views of the Nearby Voids from Table 1.

In Figures A1–A6 of the Appendix we present 3D views in supergalactic coordinates  $SGX, SGY, SGZ$  of all 25 voids from Table 2 in cubes with the side length of 50 Mpc, which includes the adopted main sphere with  $R = 25$  Mpc. These views allow one to get the first impression of the void sizes and positions relative to the Local Sheet, concentrated to the  $SGZ = 0$  plane.

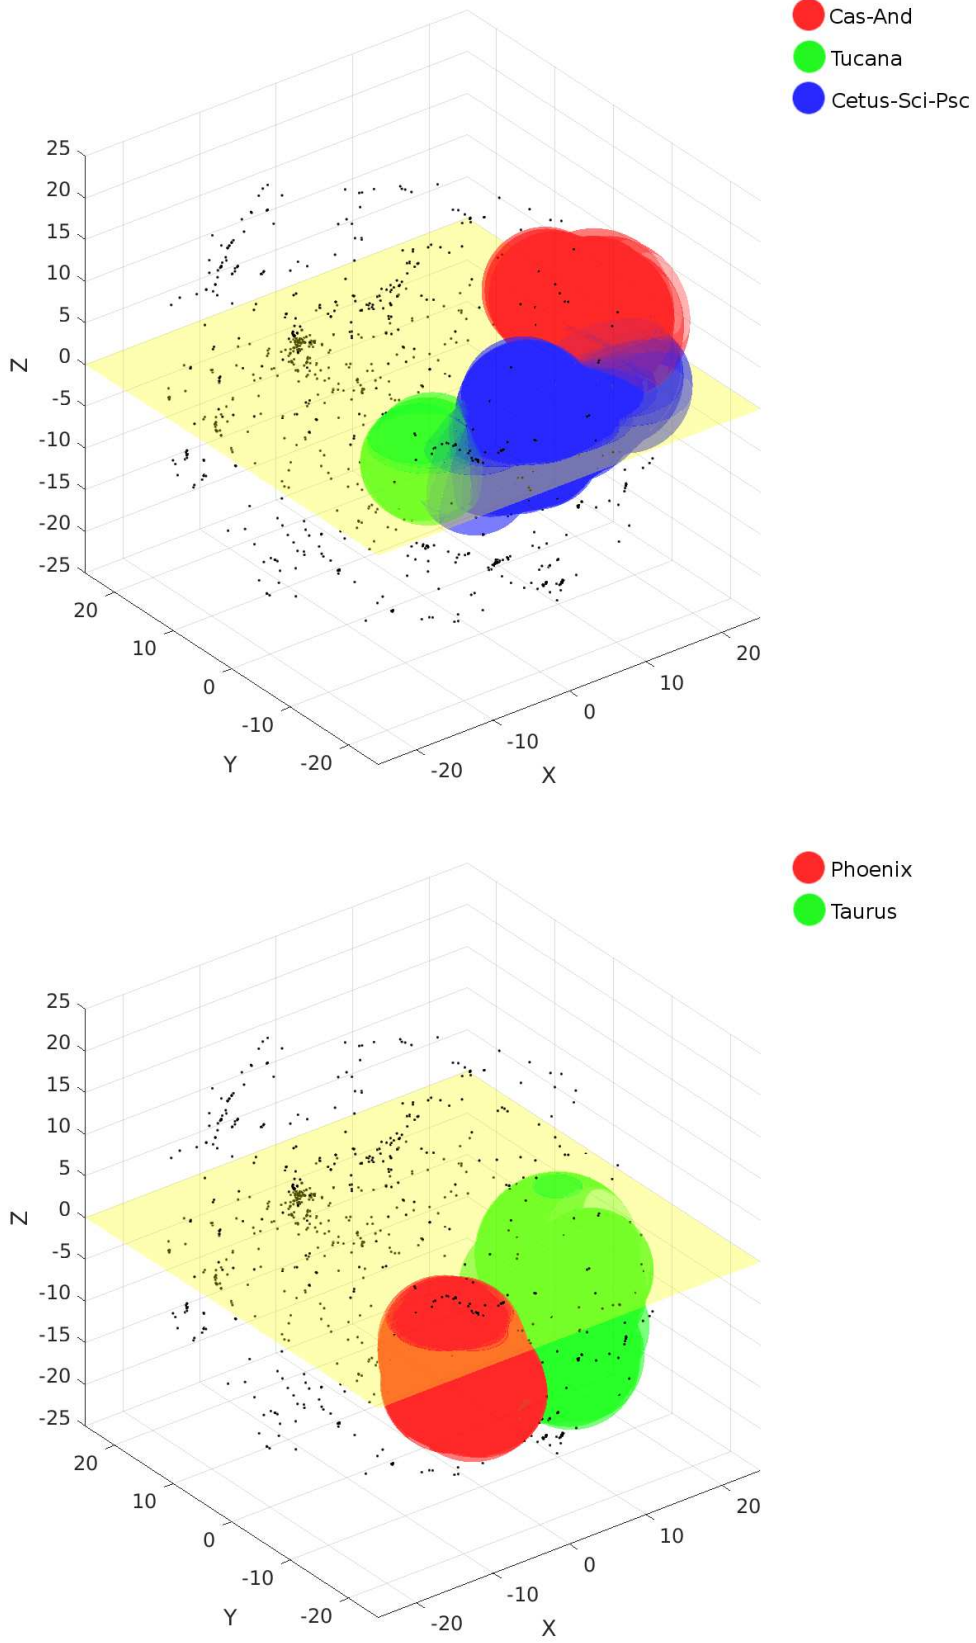

**Figure A1. Top panel:** The 3D view in supergalactic coordinates of the nearby voids described in Sect. ??, Cas-And, Tuc, Cet-Scu-Psc. The position of plane  $SGZ = 0$  is shown in aid to eye. **Bottom panel.** Similar view of two voids: Pho and Tau.

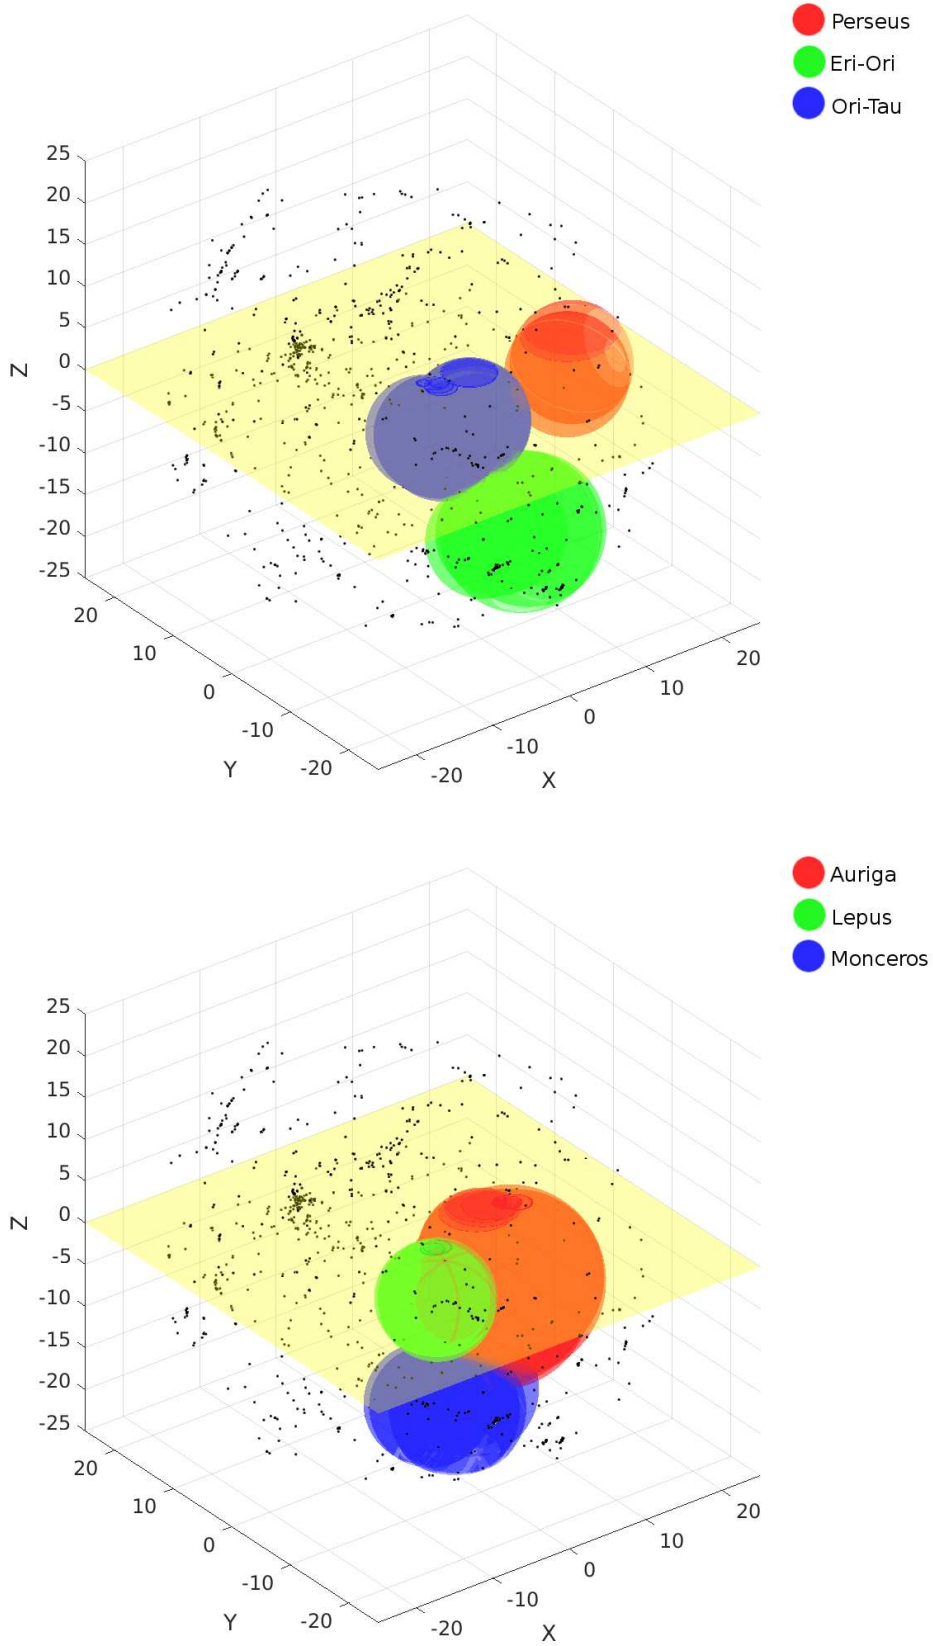

**Figure A2. Top panel:** The 3D view in supergalactic coordinates of the three nearby voids described in Sect. ??, Per, Eri-Ori, Ori-Tau. The position of plane  $SGZ = 0$  is shown in aid to eye. **Bottom panel.** Similar view of three other voids: Aur, Lep and Mon.

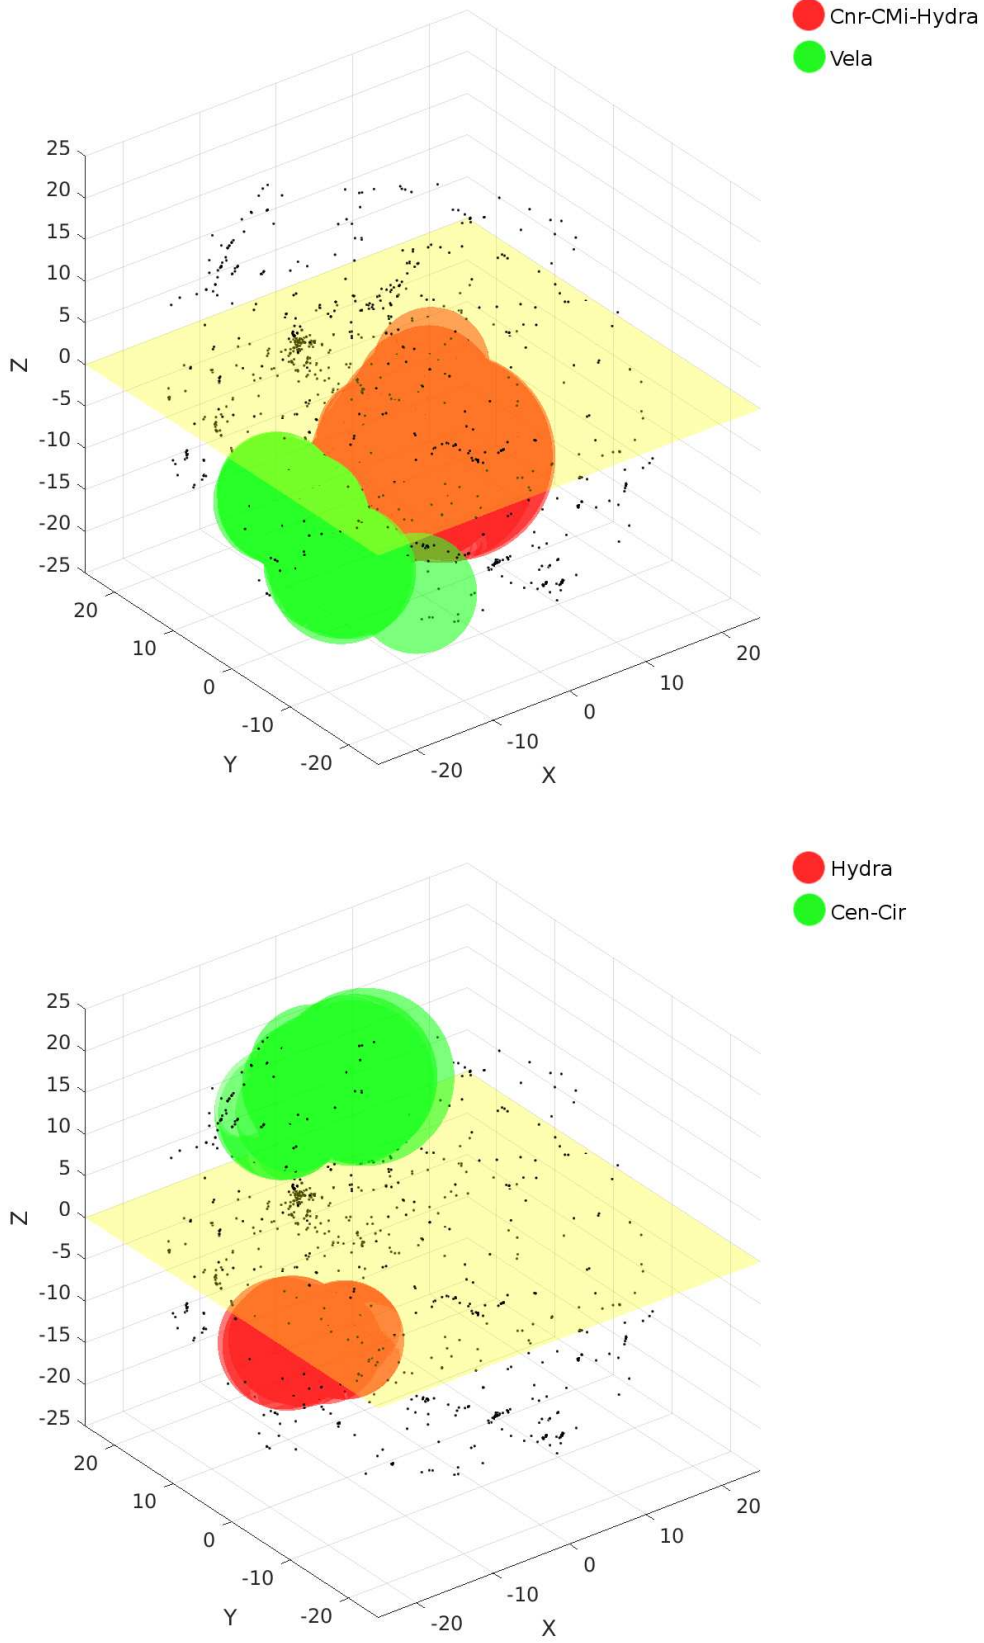

**Figure A3. Top panel:** The 3D view in supergalactic coordinates of the two nearby voids described in Sect. ??, Cnr-CMi-Hyd and Vela. The position of plane  $SGZ = 0$  is shown in aid to eye. **Bottom panel.** Similar view of two other voids: Hyd and Cen-Cir.

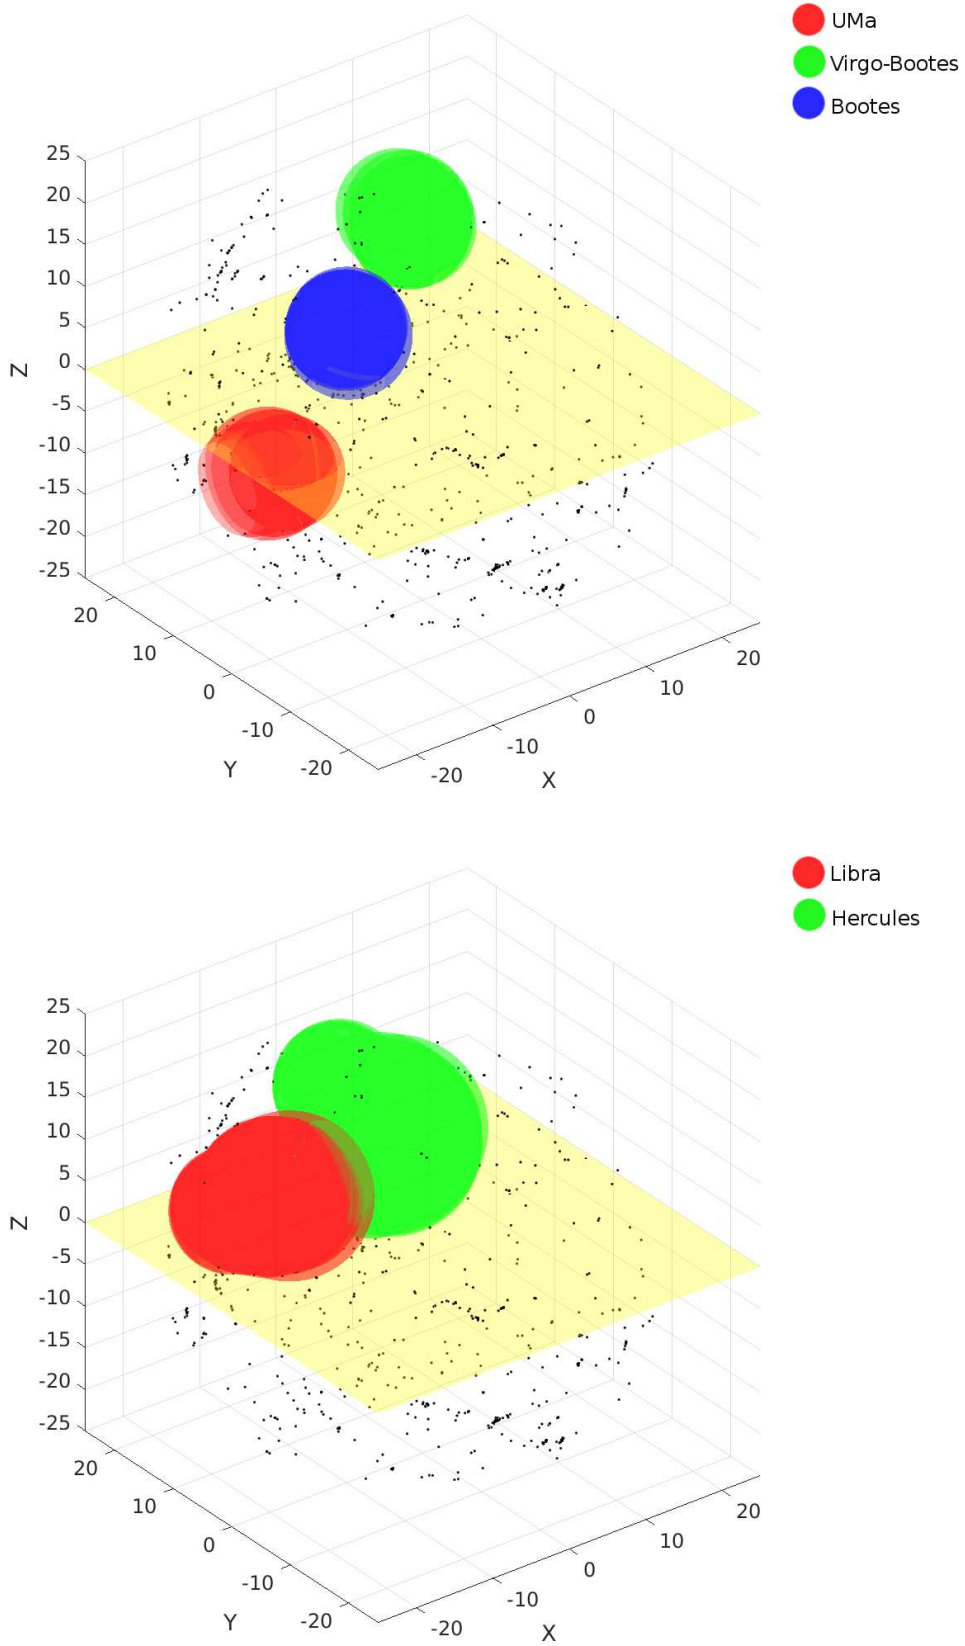

**Figure A4. Top panel:** The 3D view in the supergalactic coordinates of the three nearby voids described in Sect. ??, UMa, Vir-Boo and Boo. The position of plane  $SGZ = 0$  is shown in aid to eye. **Bottom panel.** Similar view of two other voids: Lib and Her.

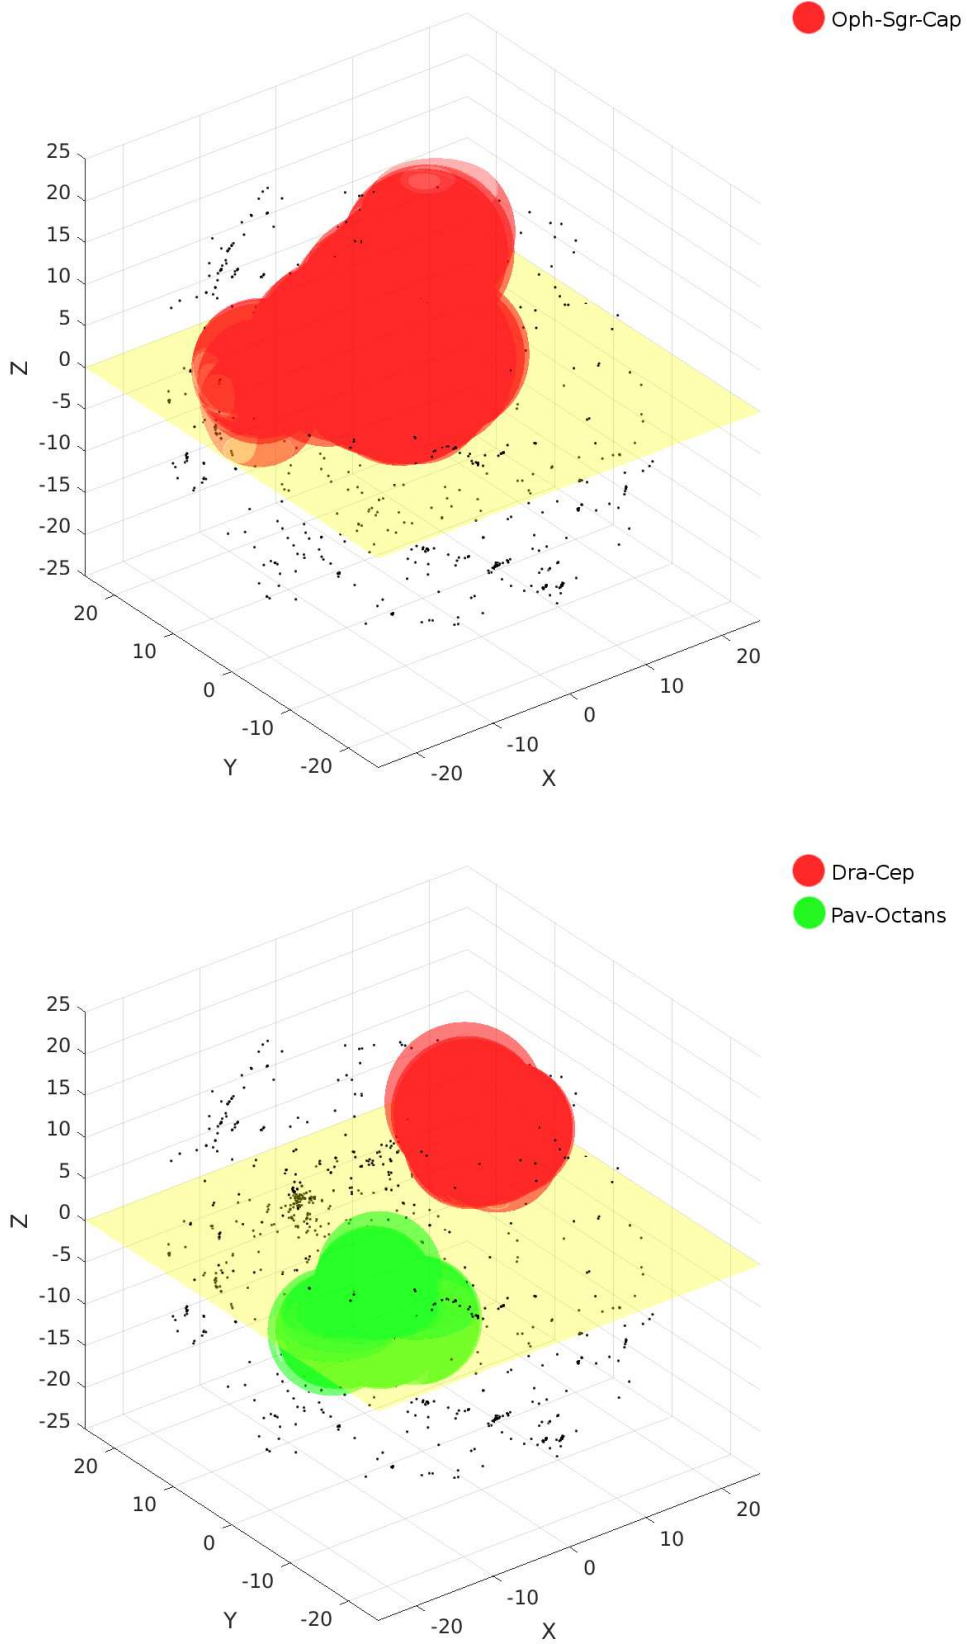

**Figure A5. Top panel:** The 3D view in the supergalactic coordinates of the largest nearby voids described in Sect. ??, Oph-Sgr-Cap, which includes the nearby part of the Local Void and its environs. The position of plane  $SGZ = 0$  is shown in aid to eye. **Bottom panel.** Similar view of two other voids: Dra-Cep and Pav-Oct.



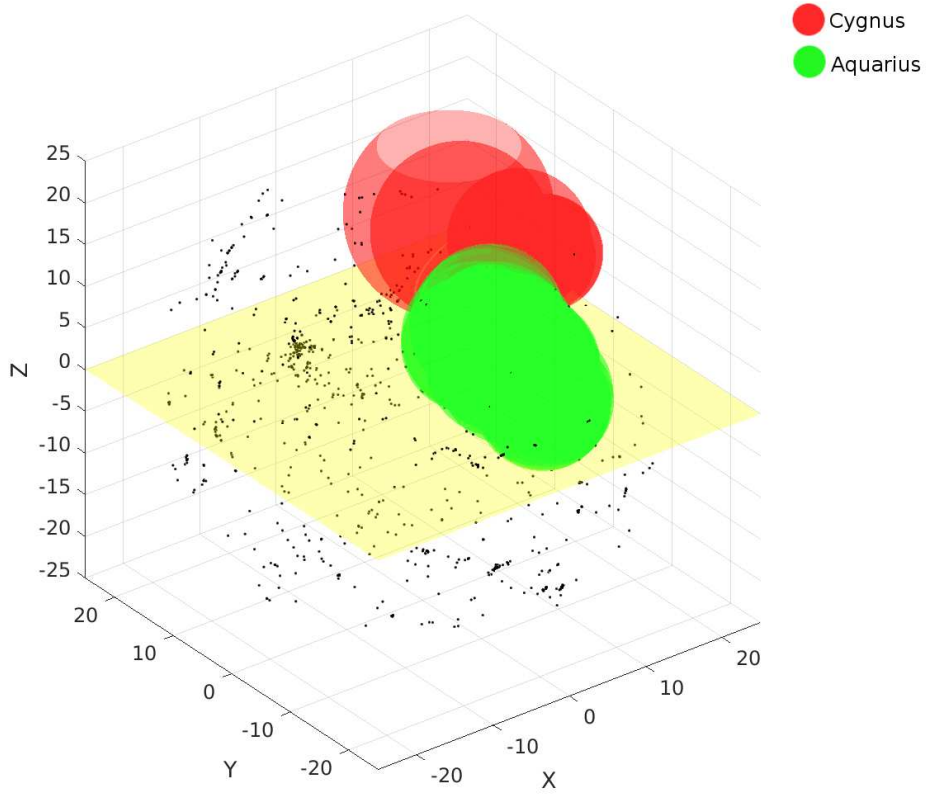

**Figure A6.** The 3D view in supergalactic coordinates of the two voids described in Sect. ??, Cyg and Aqu. The position of plane  $SGZ = 0$  is shown in aid to eye.



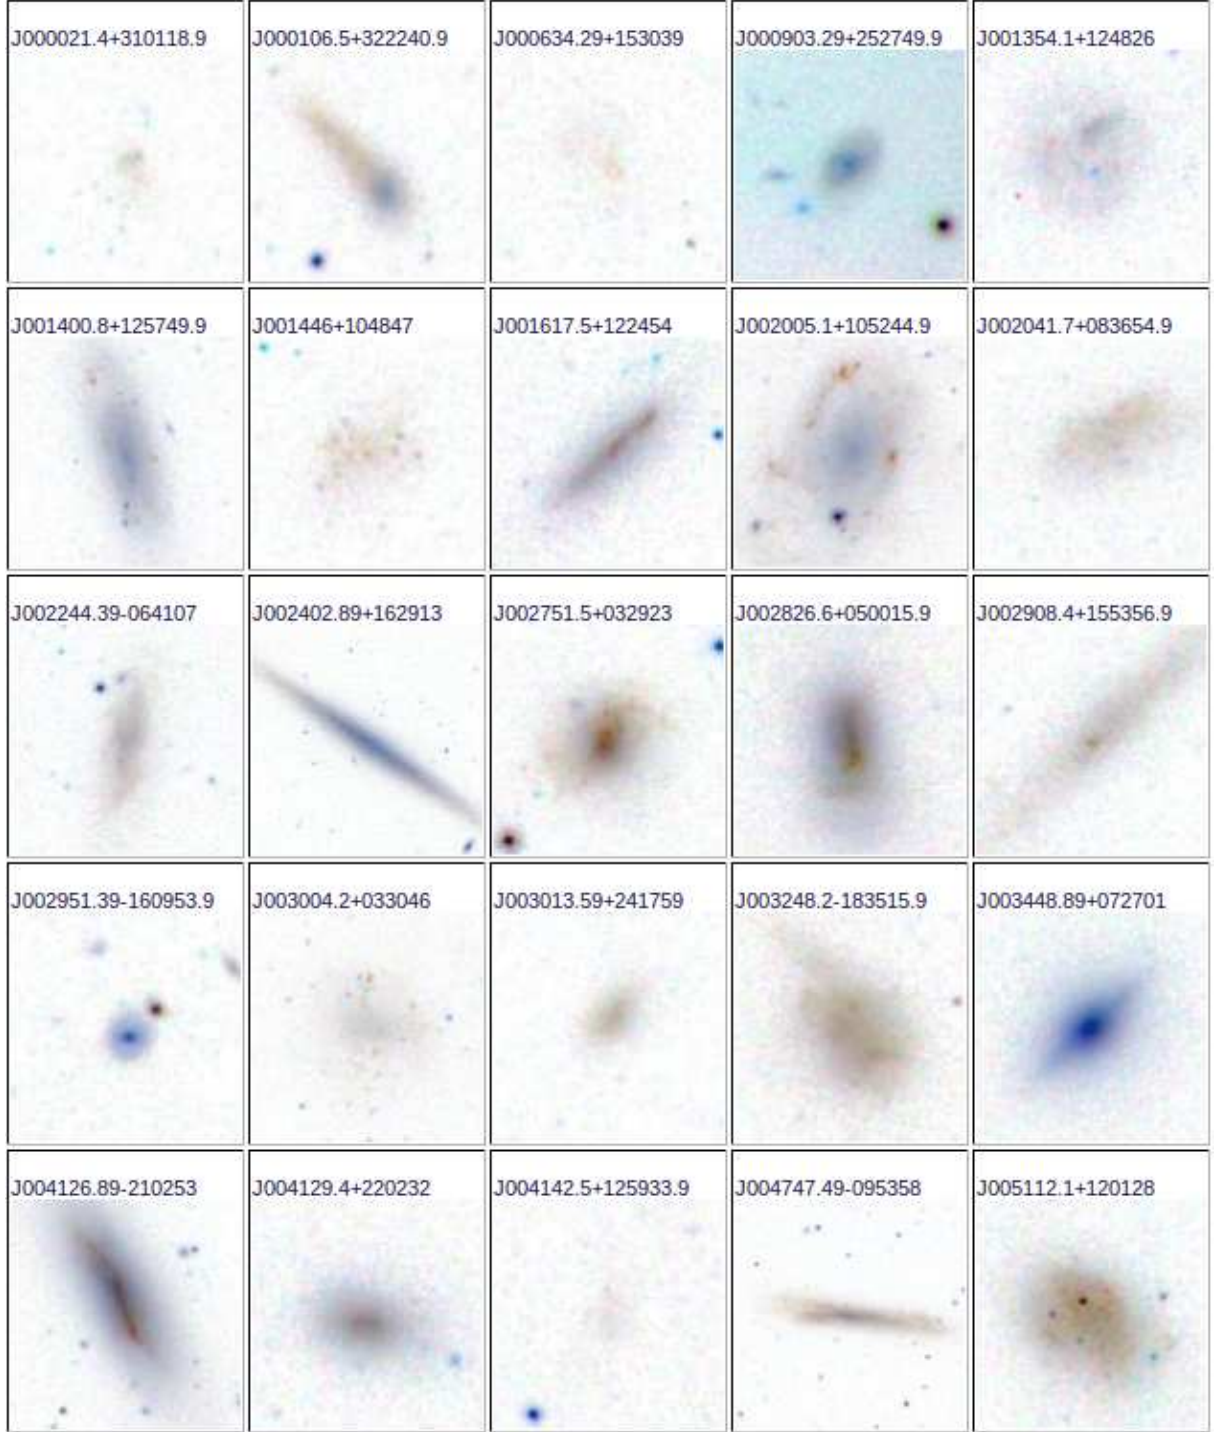

**Figure A7.** Mosaics of the first 25 'inner' nearby void galaxies in the R.A. order prepared from the SDSS colour images. The side of the chart is 50".

### A3 Finding charts of the Nearby Void Galaxy catalog, the 'inner' and 'outer' parts

We present the finding charts of the Nearby Void Galaxy sample in four mosaics. Figures A7–A65 are for finding charts of galaxies of the 'inner' part (1088 objects with  $D_{\text{NN}} \geq 2.0$  Mpc) divided into those falling within the SDSS footprint sky regions (487 objects, Figures A7–A25) and the remaining 601 'inner' galaxies residing outside the SDSS zone (Figures A26–A65), for which we use digitized DSS1/DSS2 images.

Two more categories relate to the 'outer' void galaxies (266 objects with  $D_{\text{NN}} < 2.0$  Mpc). Figures A66–A70 show 110 galaxies falling in the SDSS footprint, while Figures A71–A81 show the finding charts of the remaining 156 'outer' objects similar to the 'inner' sample.

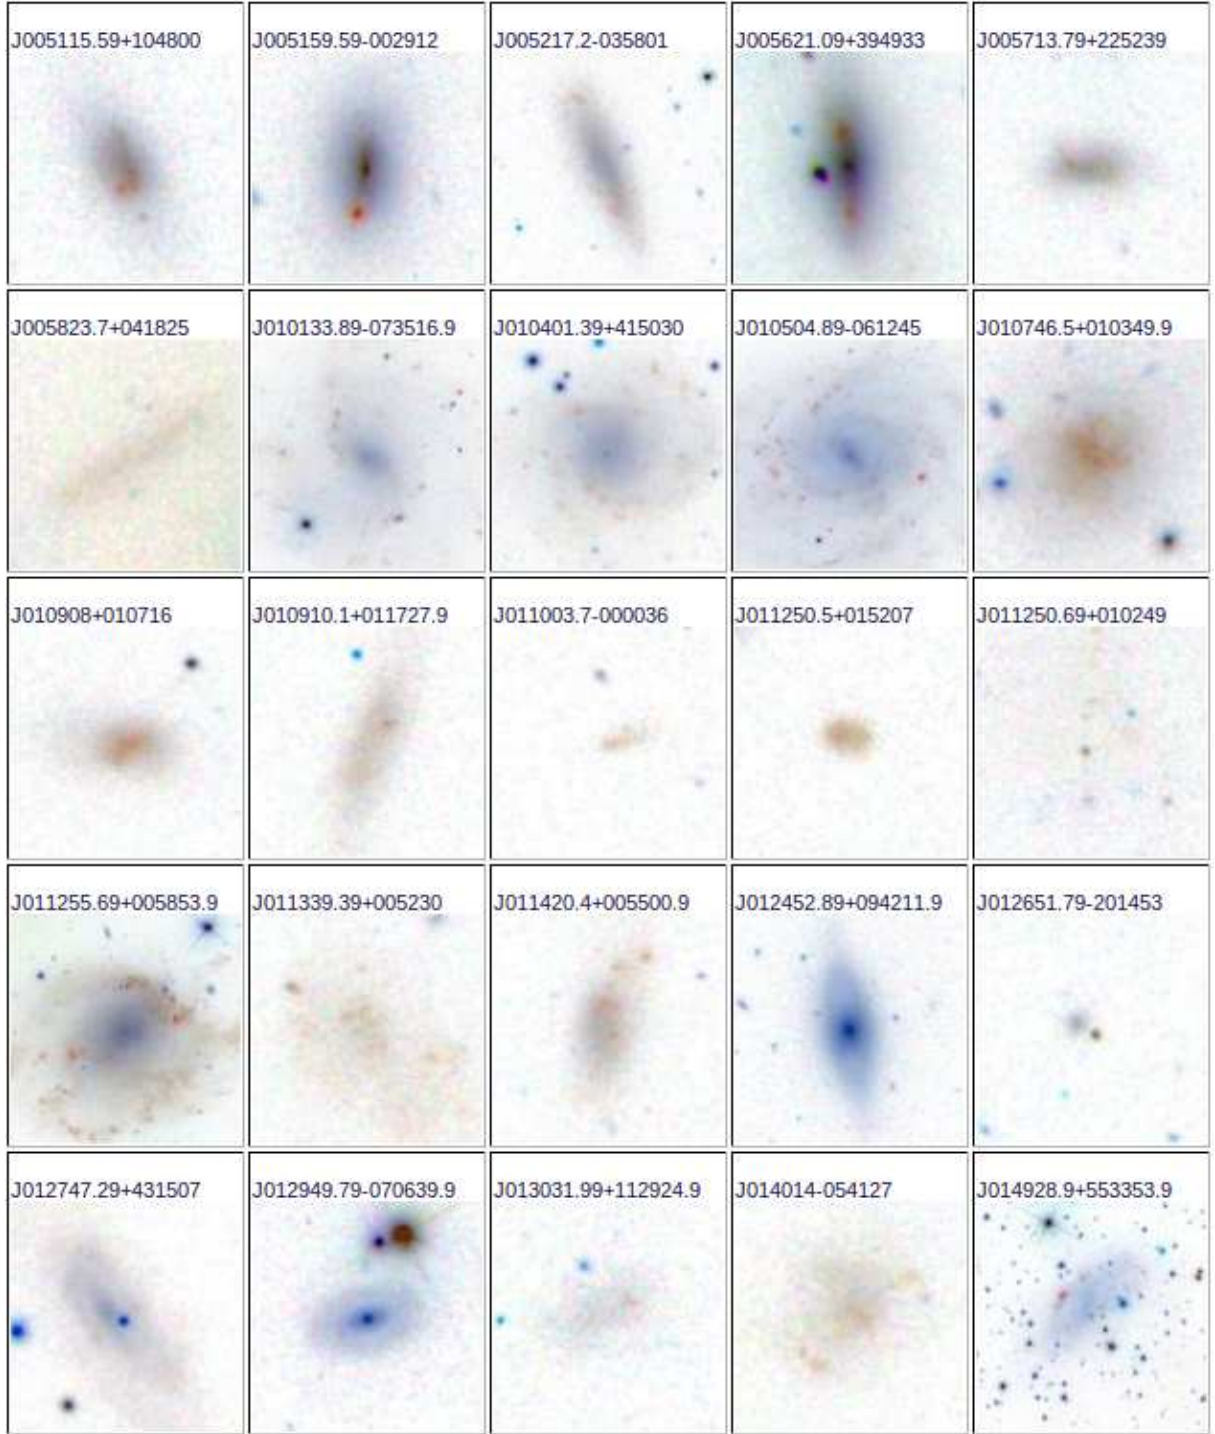

**Figure A8.** Mosaics of the next 25 'inner' nearby void galaxies prepared from the SDSS colour images. The side of the chart is 50".

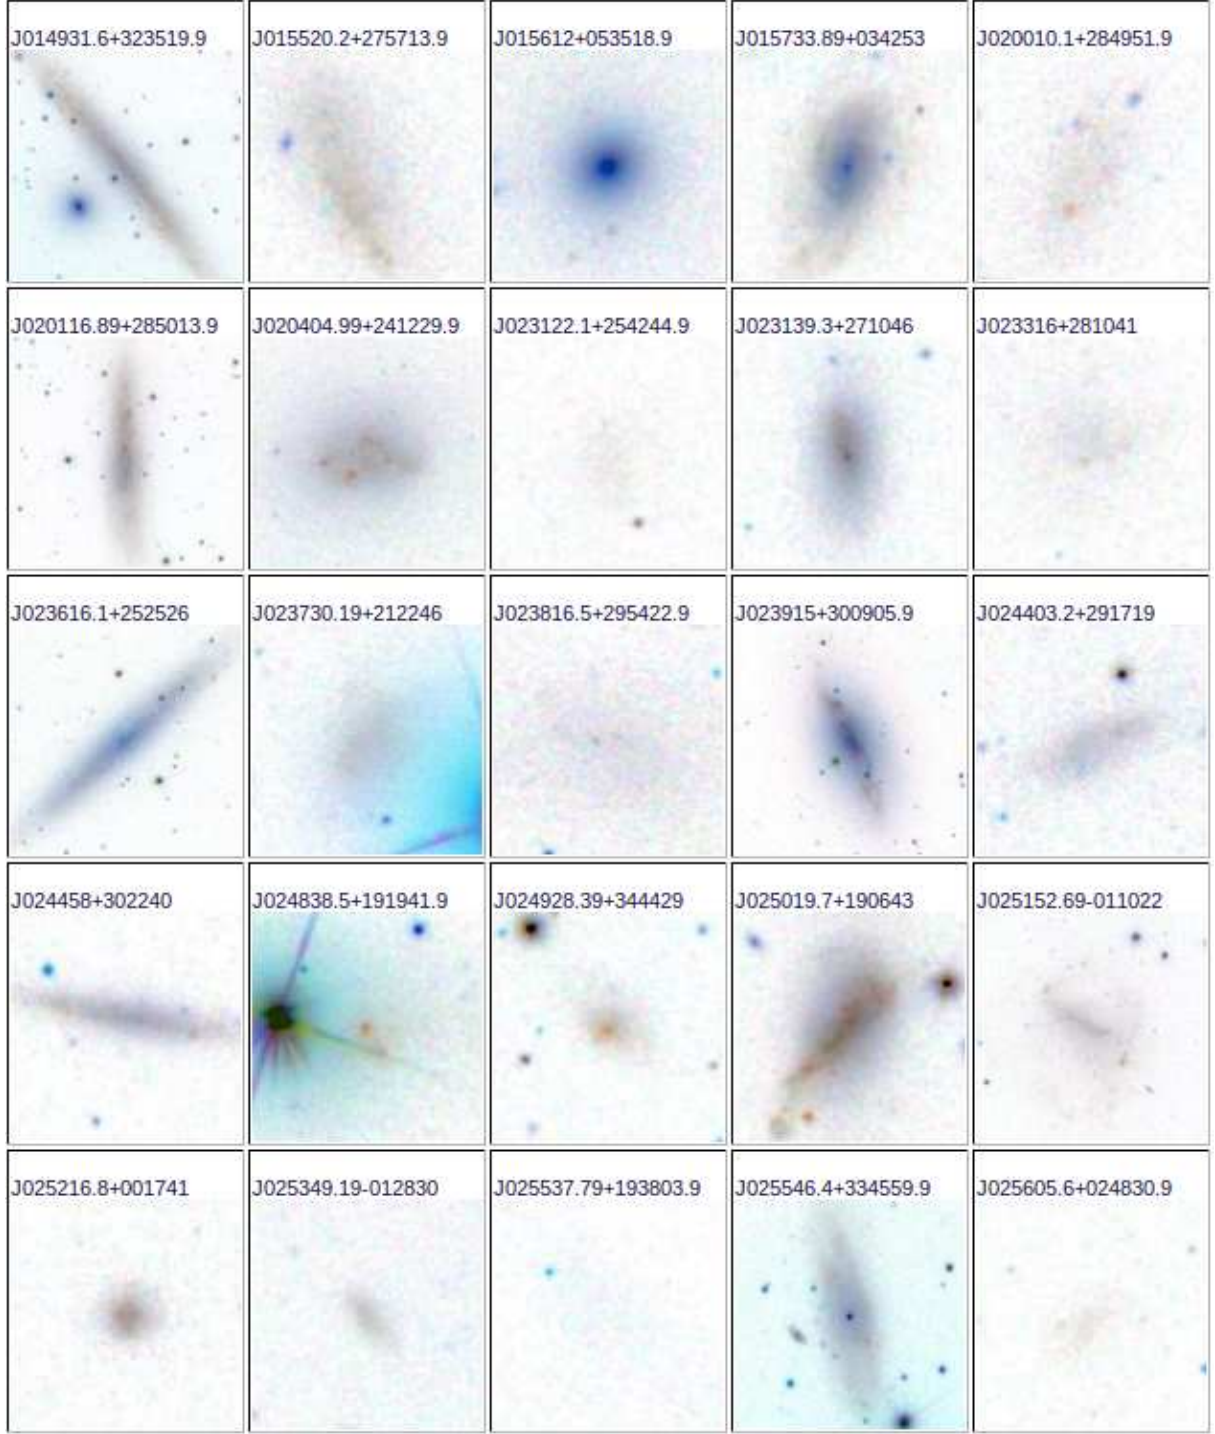

**Figure A9.** Mosaics of the next 25 'inner' nearby void galaxies prepared from the SDSS colour images. The side of the chart is 50".



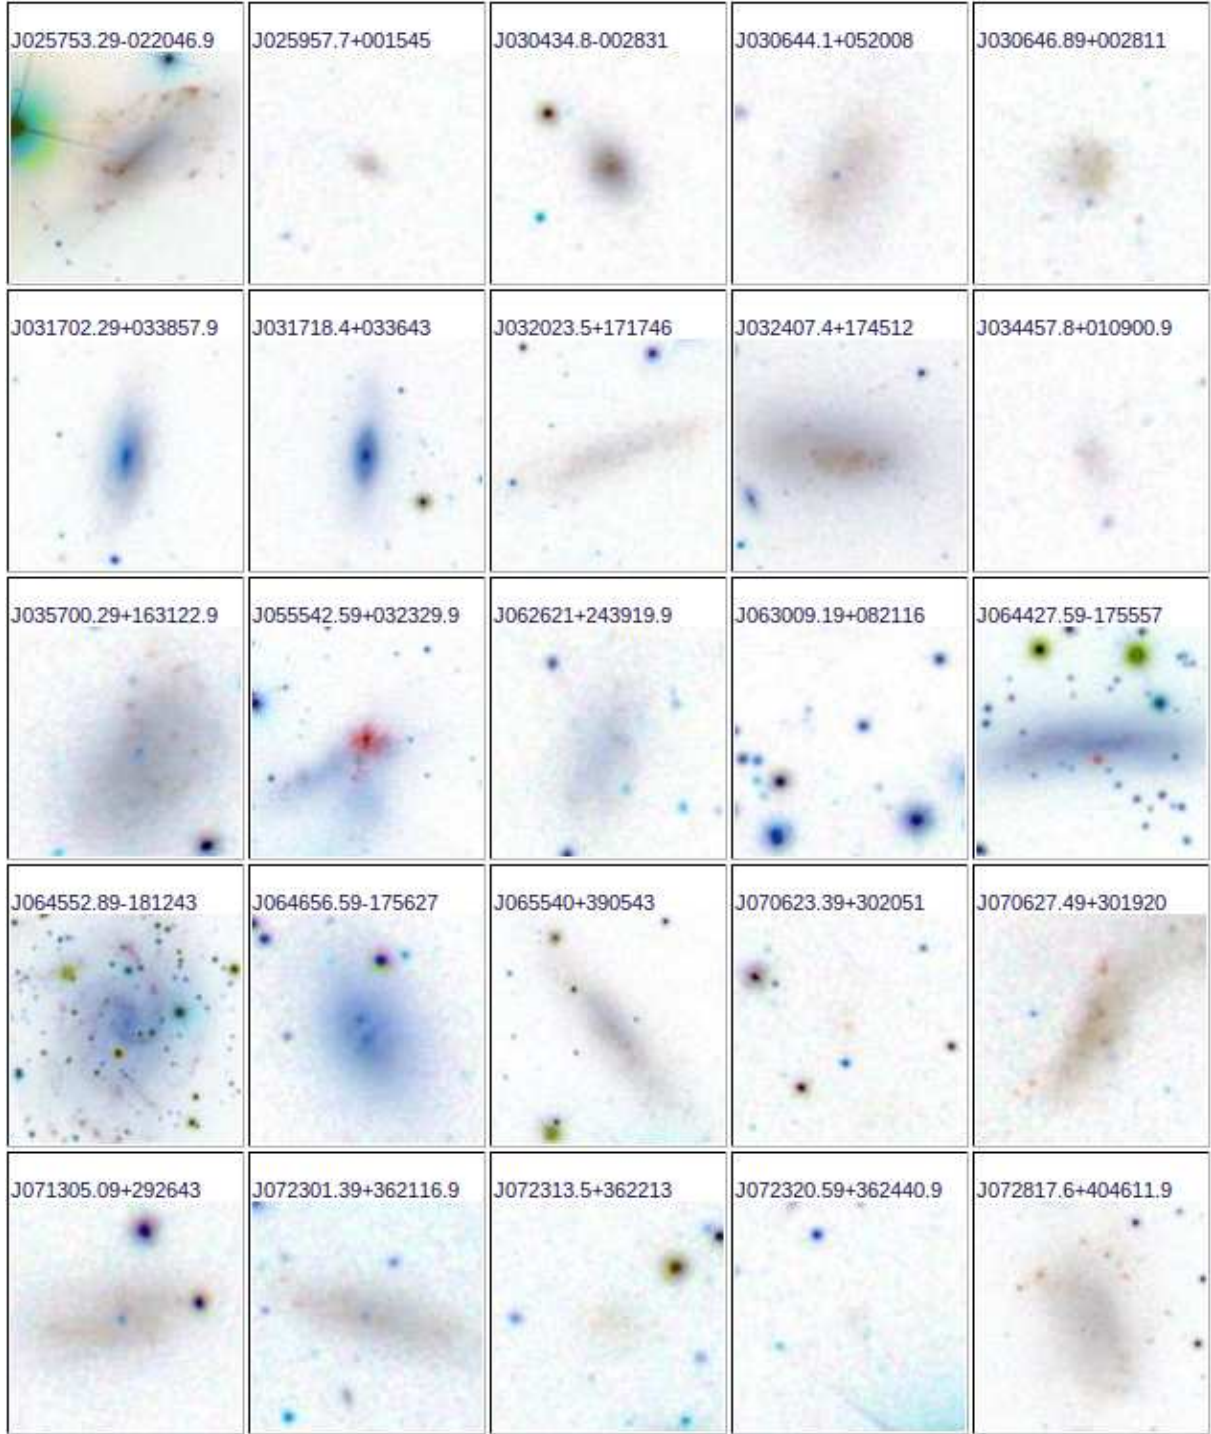

**Figure A10.** Mosaics of the next 25 'inner' nearby void galaxies prepared from the SDSS colour images. The side of the chart is 50".

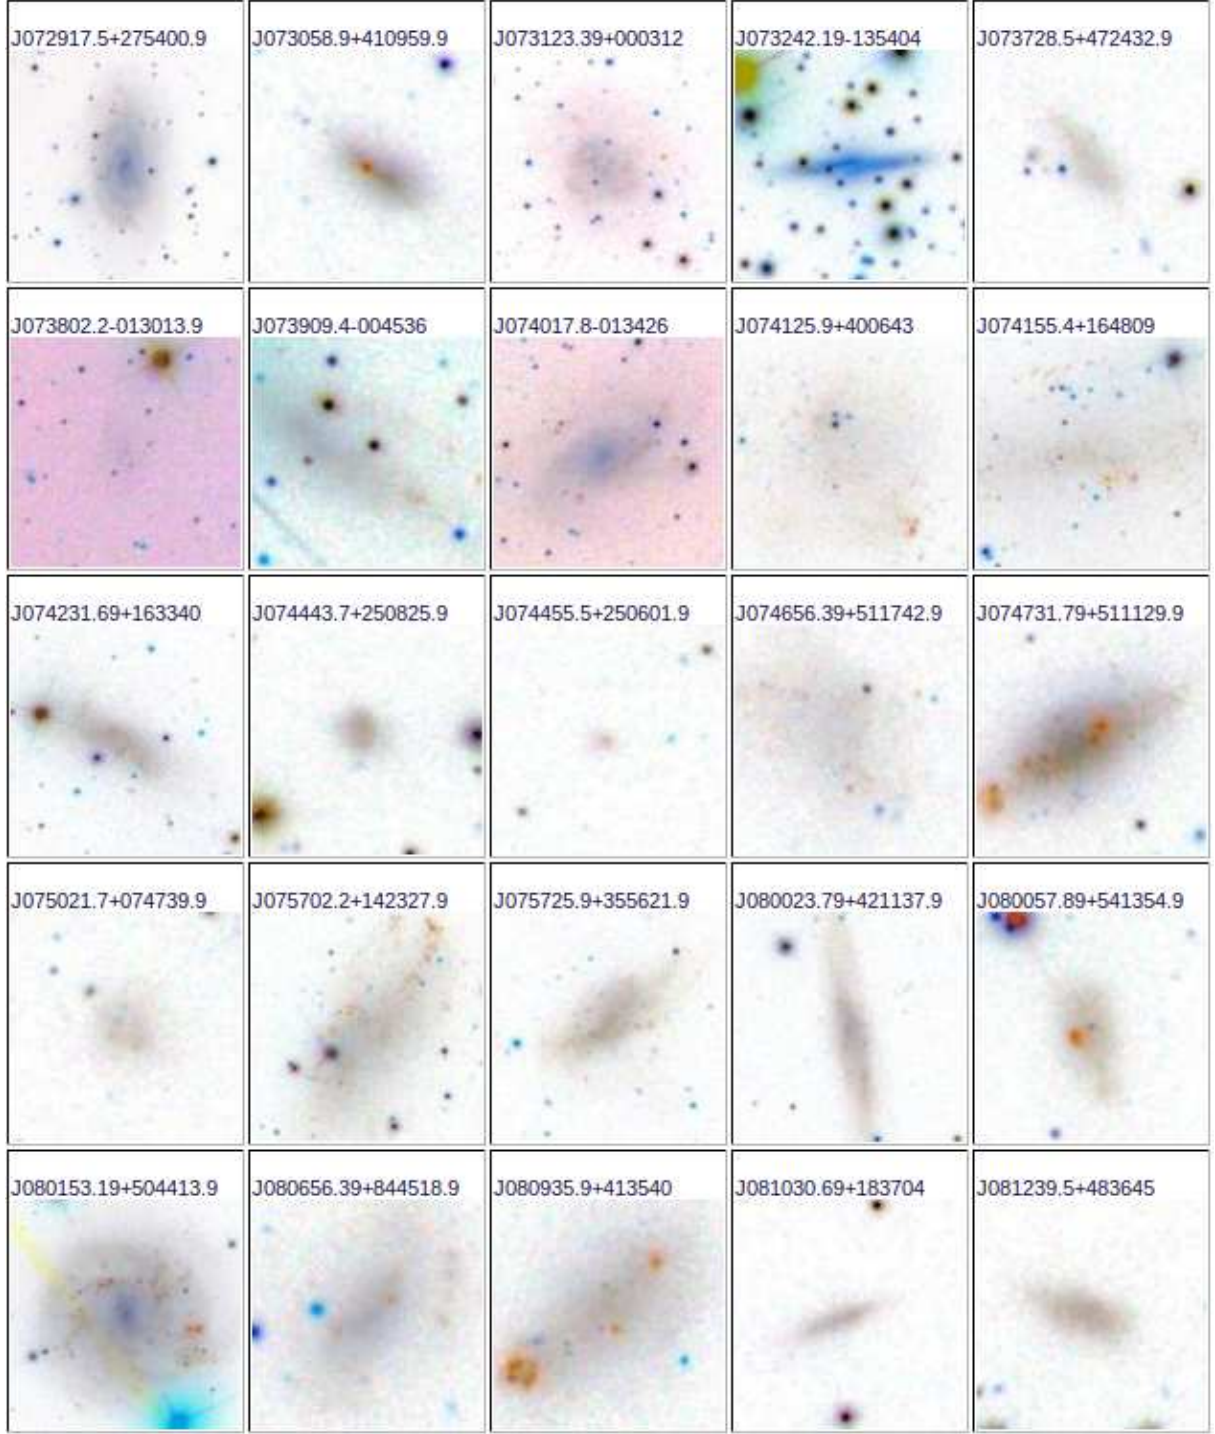

**Figure A11.** Mosaics of the next 25 'inner' nearby void galaxies prepared from the SDSS colour images. The side of the chart is 50".

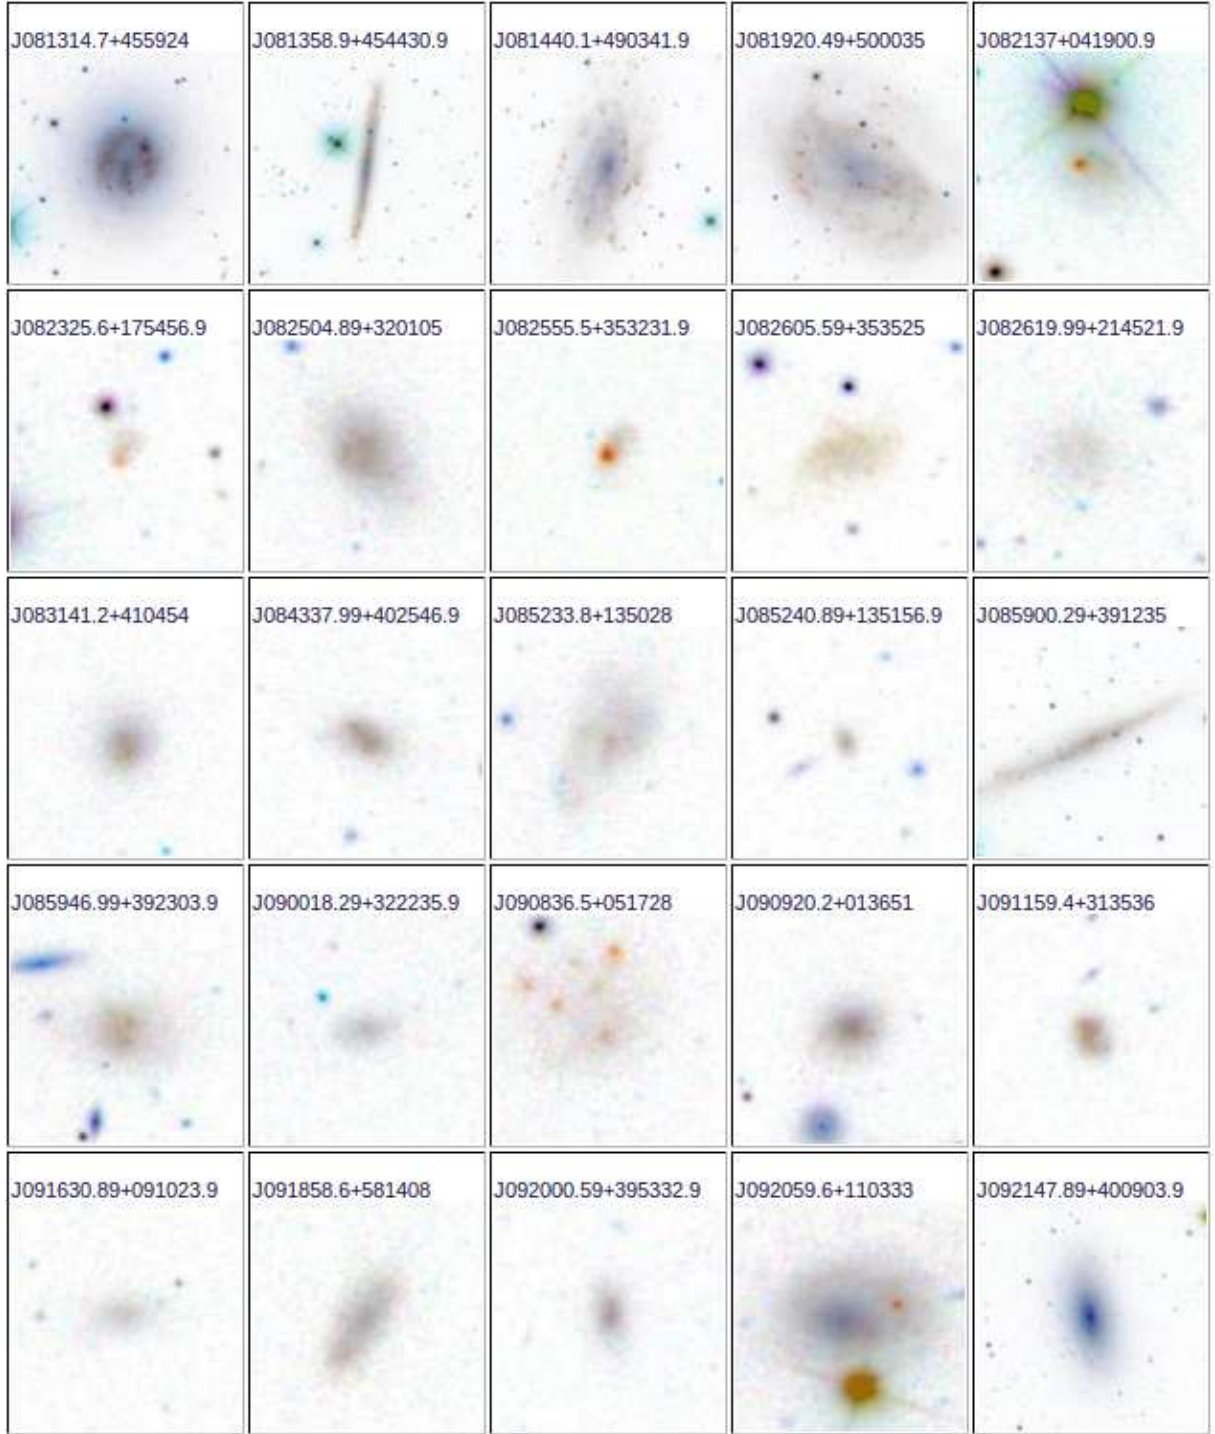

**Figure A12.** Mosaics of the next 25 'inner' nearby void galaxies prepared from the SDSS colour images. The side of the chart is 50".



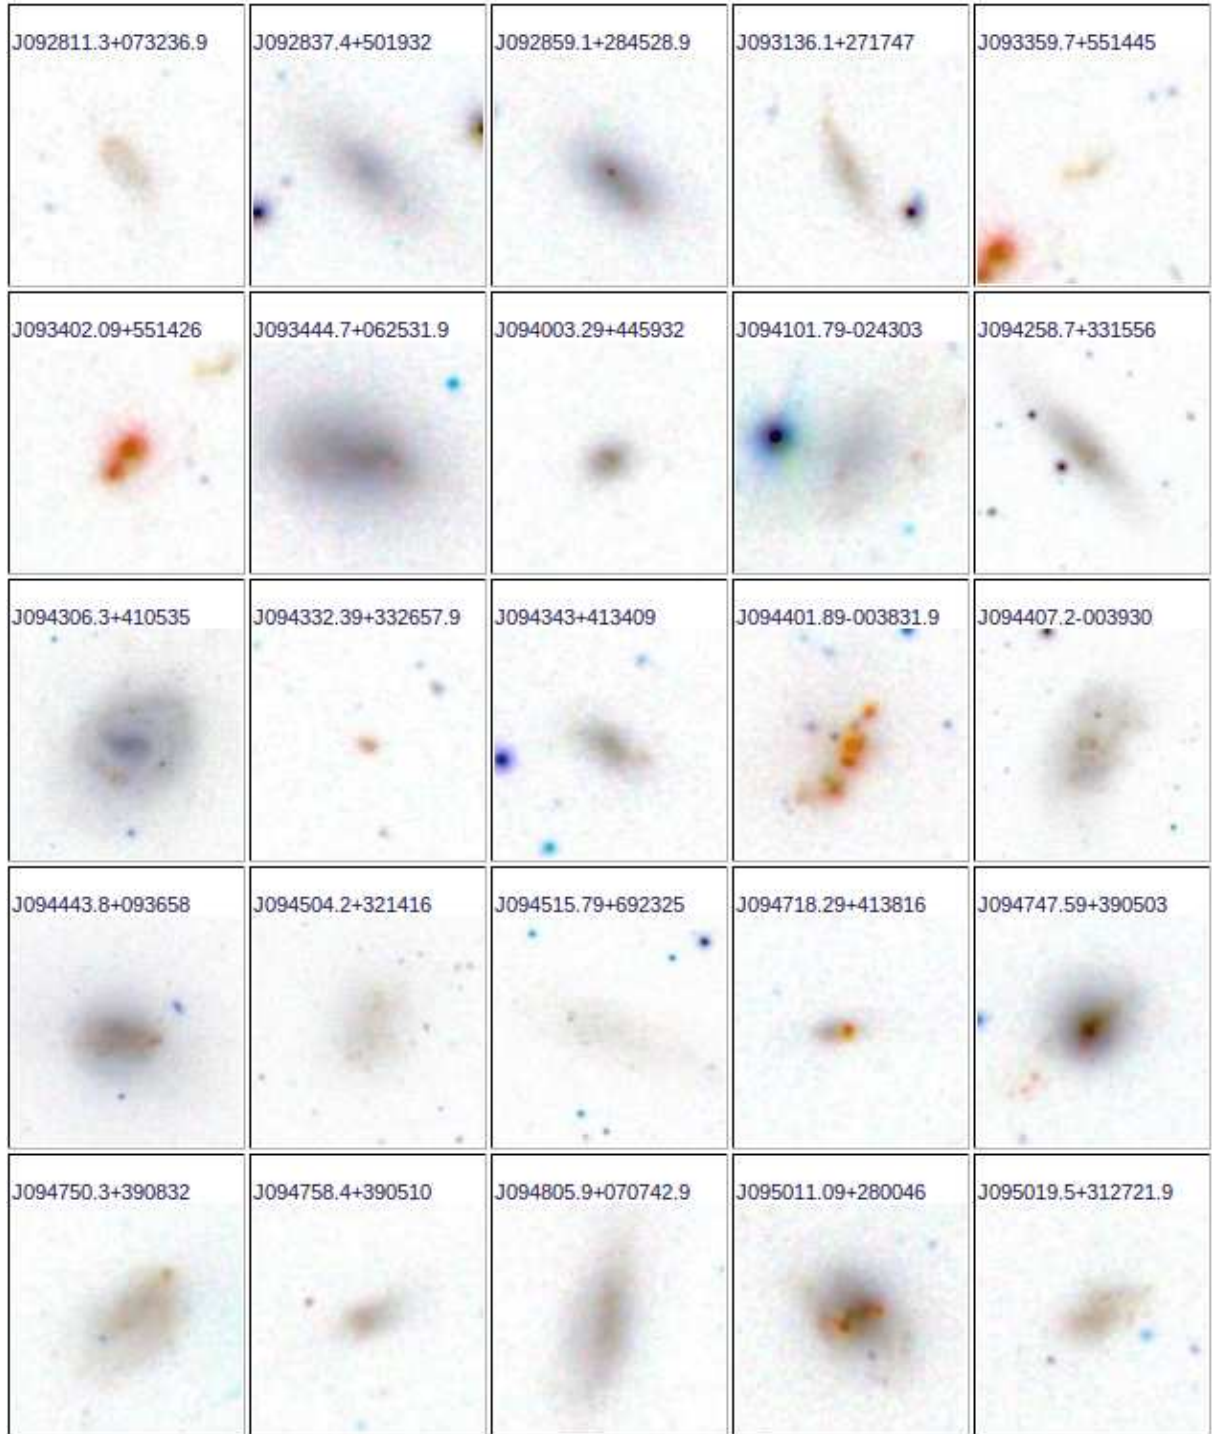

**Figure A13.** Mosaics of the next 25 'inner' nearby void galaxies prepared from the SDSS colour images. The side of the chart is 50".

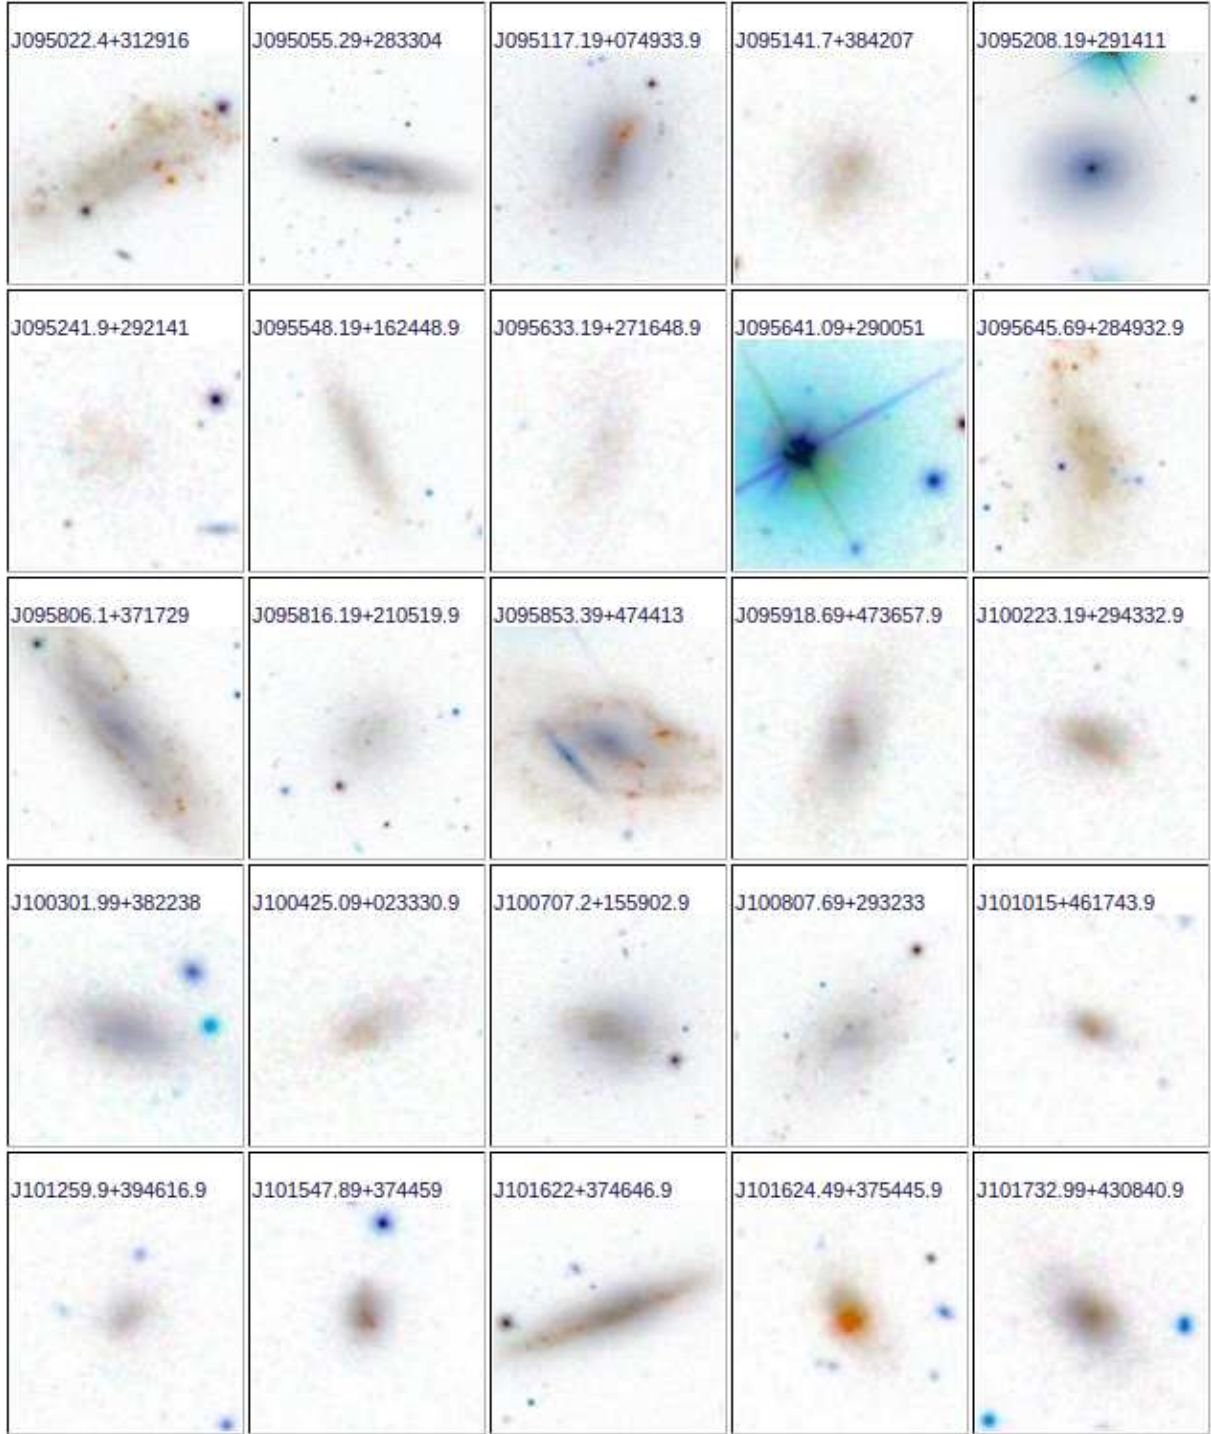

**Figure A14.** Mosaics of the next 25 'inner' nearby void galaxies prepared from the SDSS colour images. The side of the chart is 50".



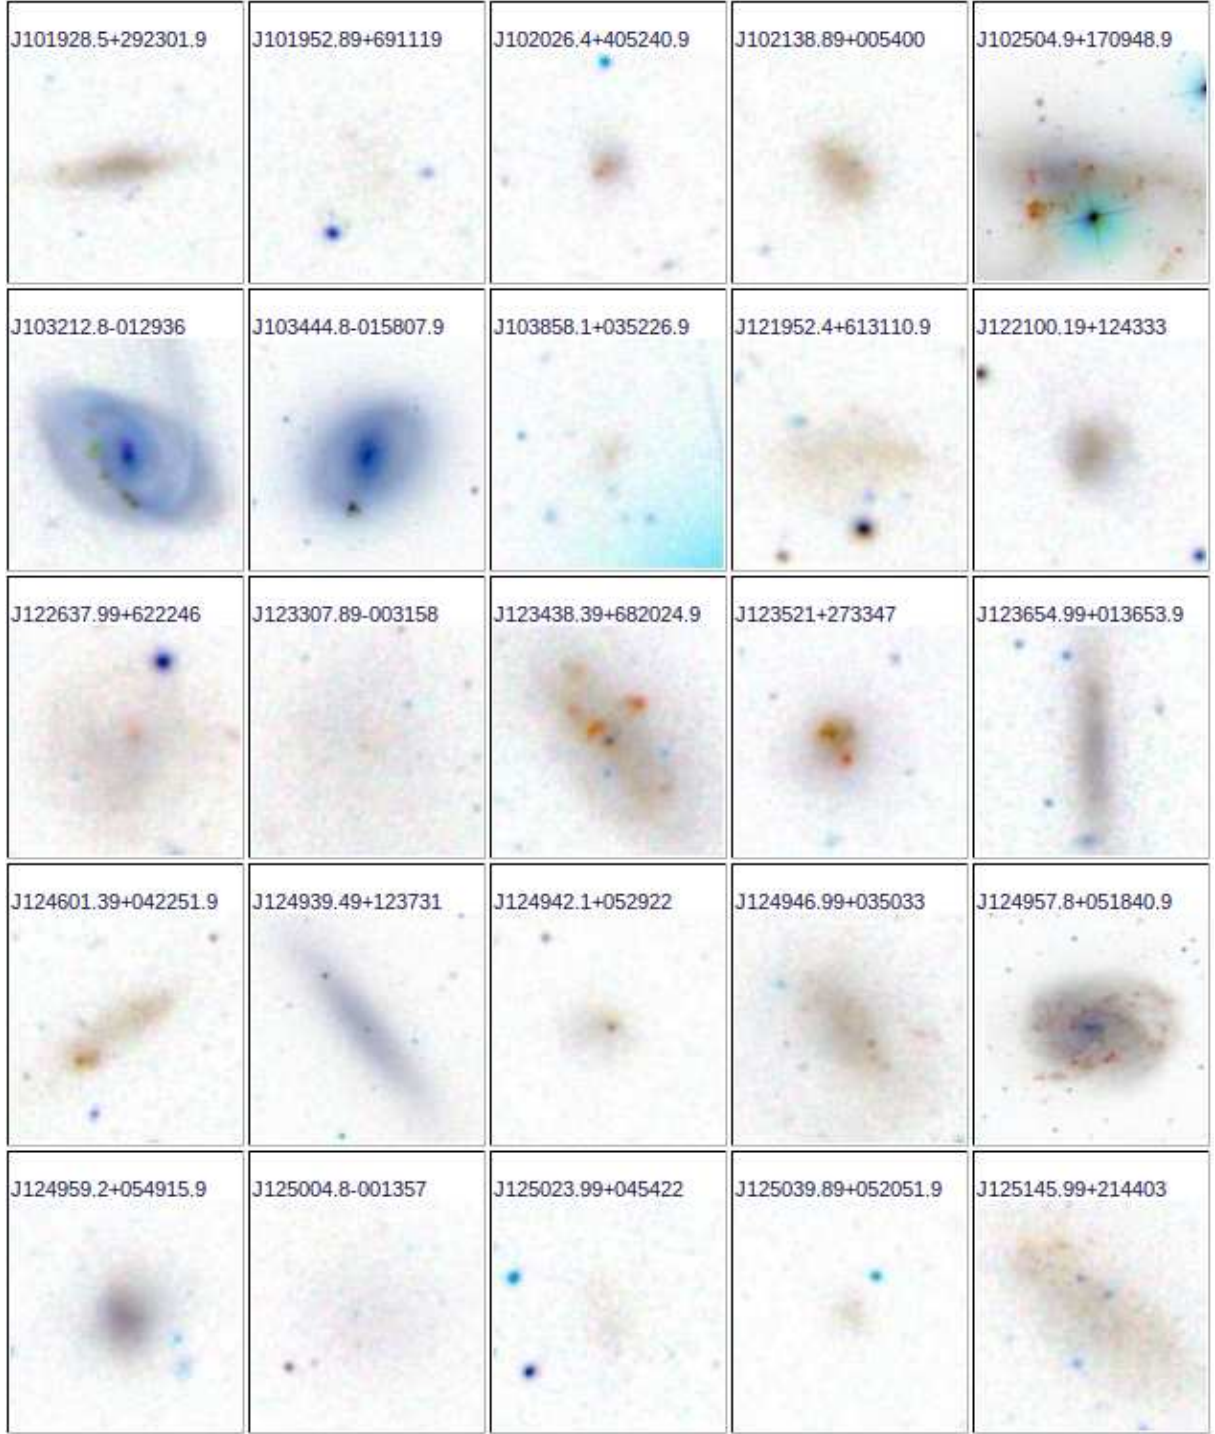

**Figure A15.** Mosaics of the next 25 'inner' nearby void galaxies prepared from the SDSS colour images. The side of the chart is 50".

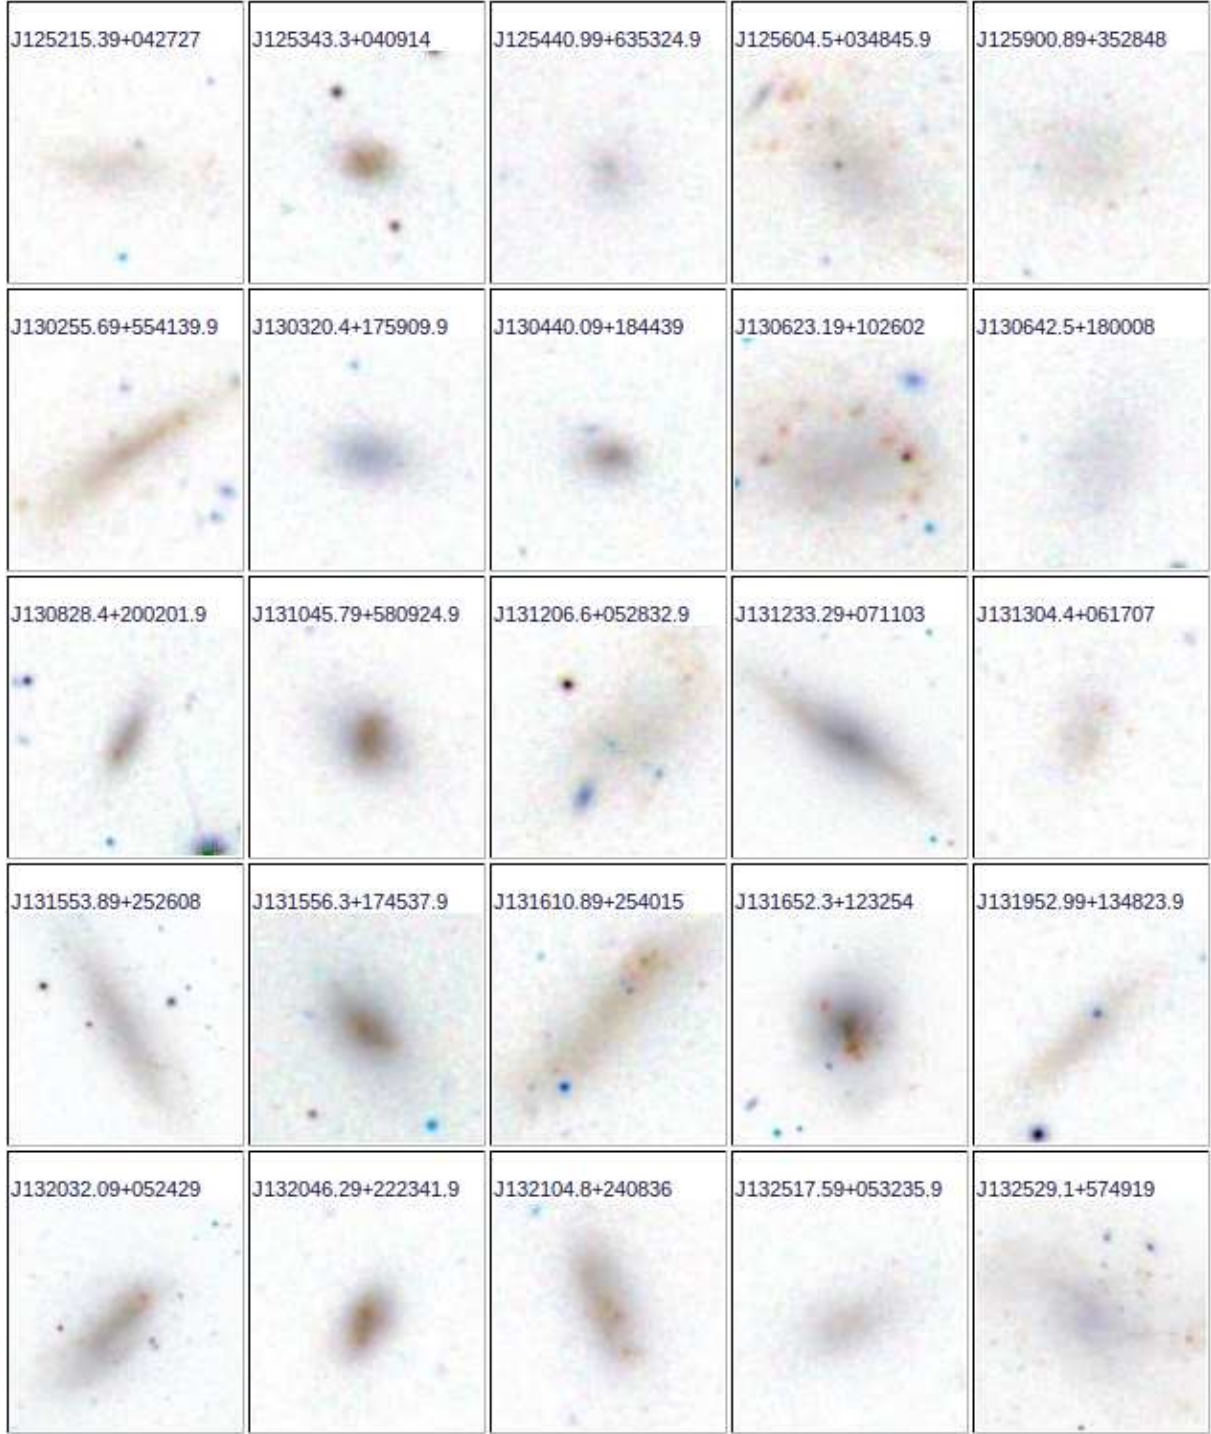

**Figure A16.** Mosaics of the next 25 'inner' nearby void galaxies prepared from the SDSS colour images. The side of the chart is 50".

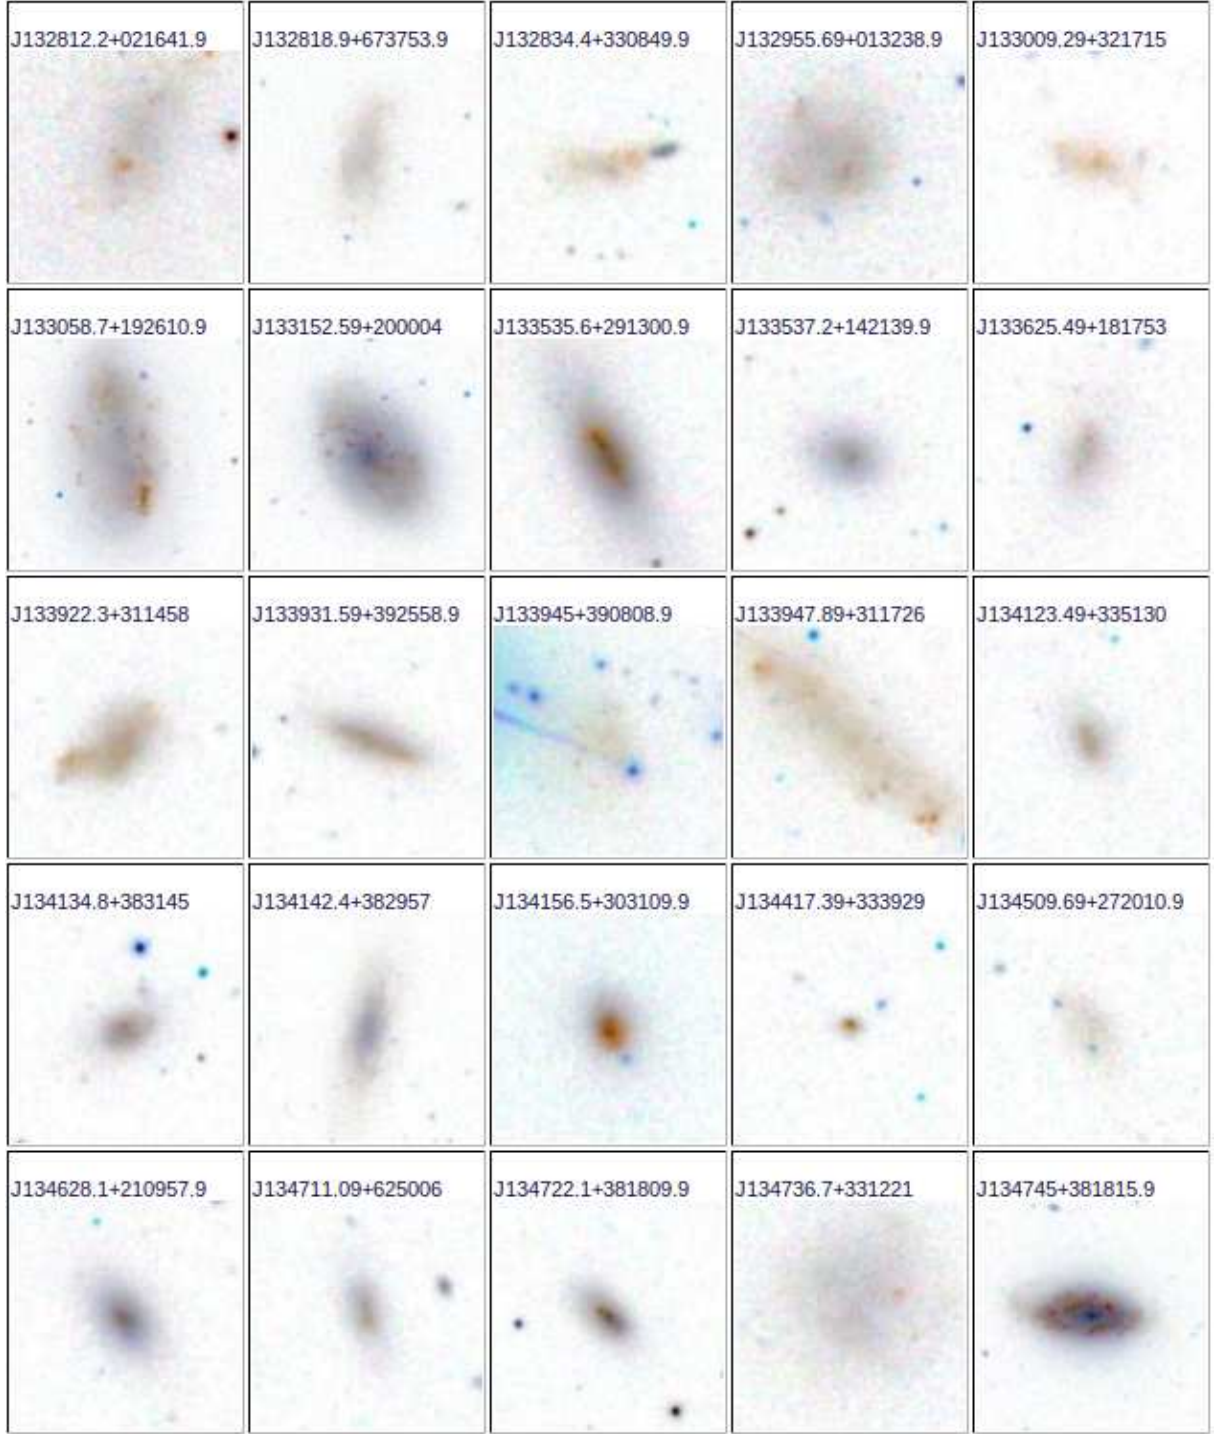

**Figure A17.** Mosaics of the next 25 'inner' nearby void galaxies prepared from the SDSS colour images. The side of the chart is 50".



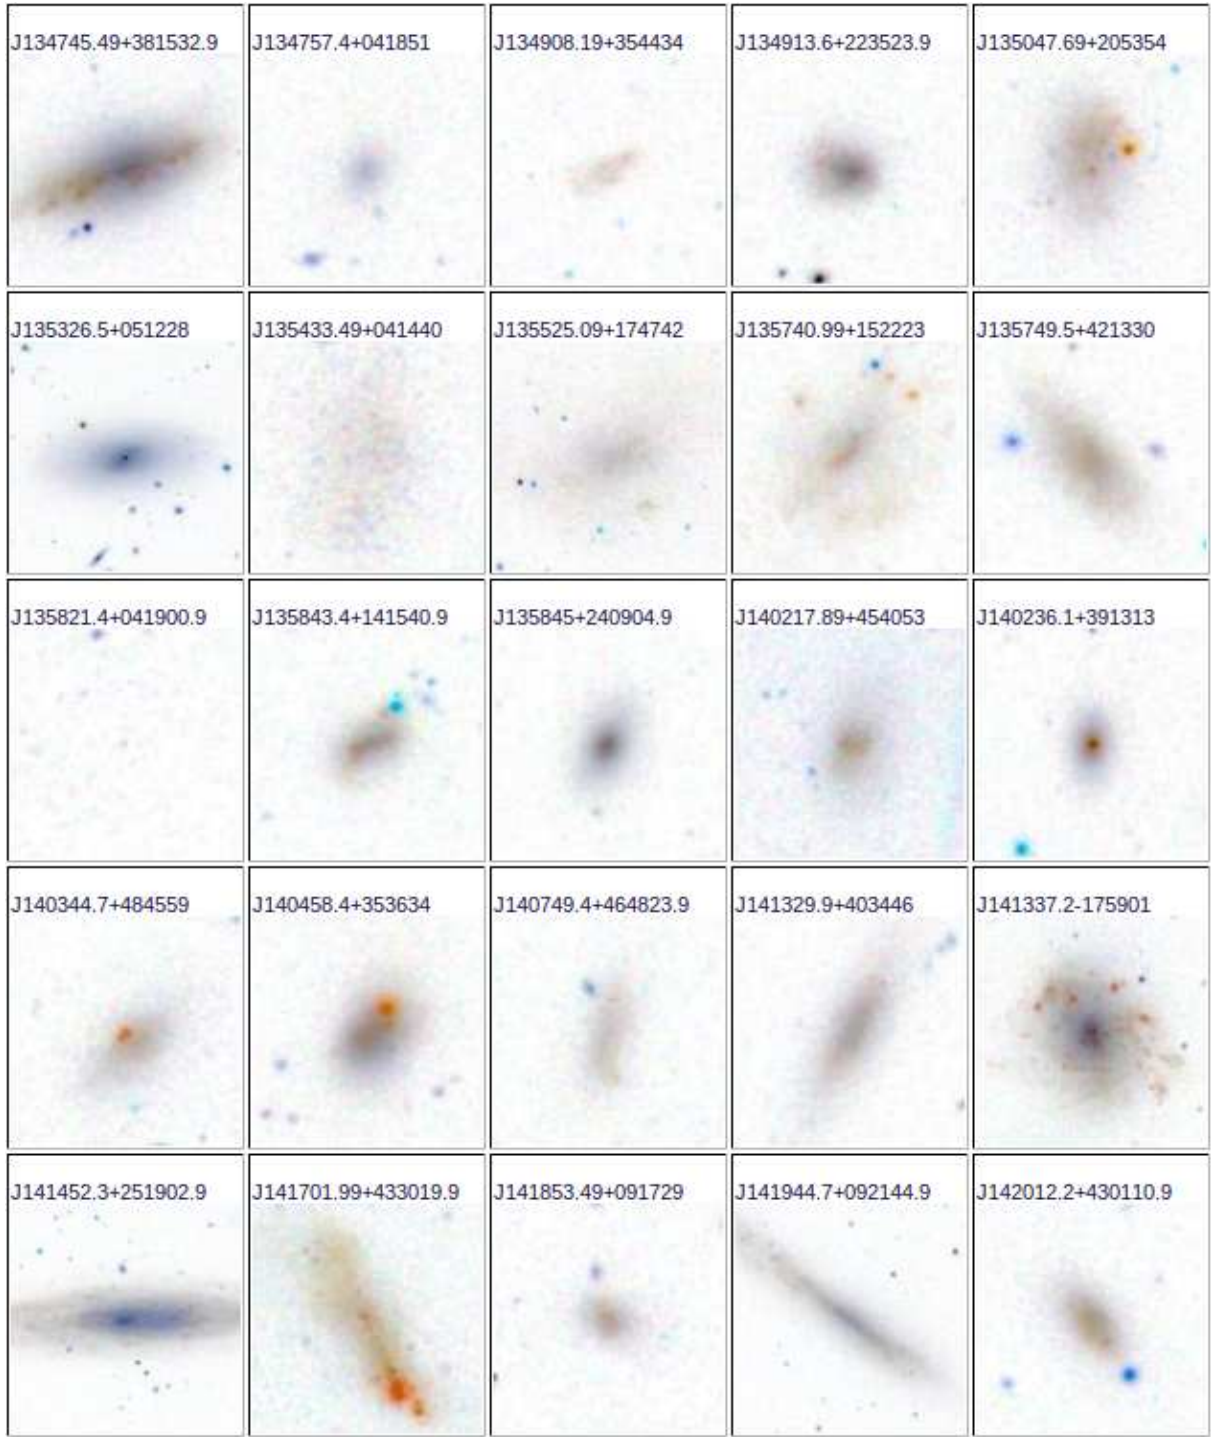

**Figure A18.** Mosaics of the next 25 'inner' nearby void galaxies prepared from the SDSS colour images. The side of the chart is 50".

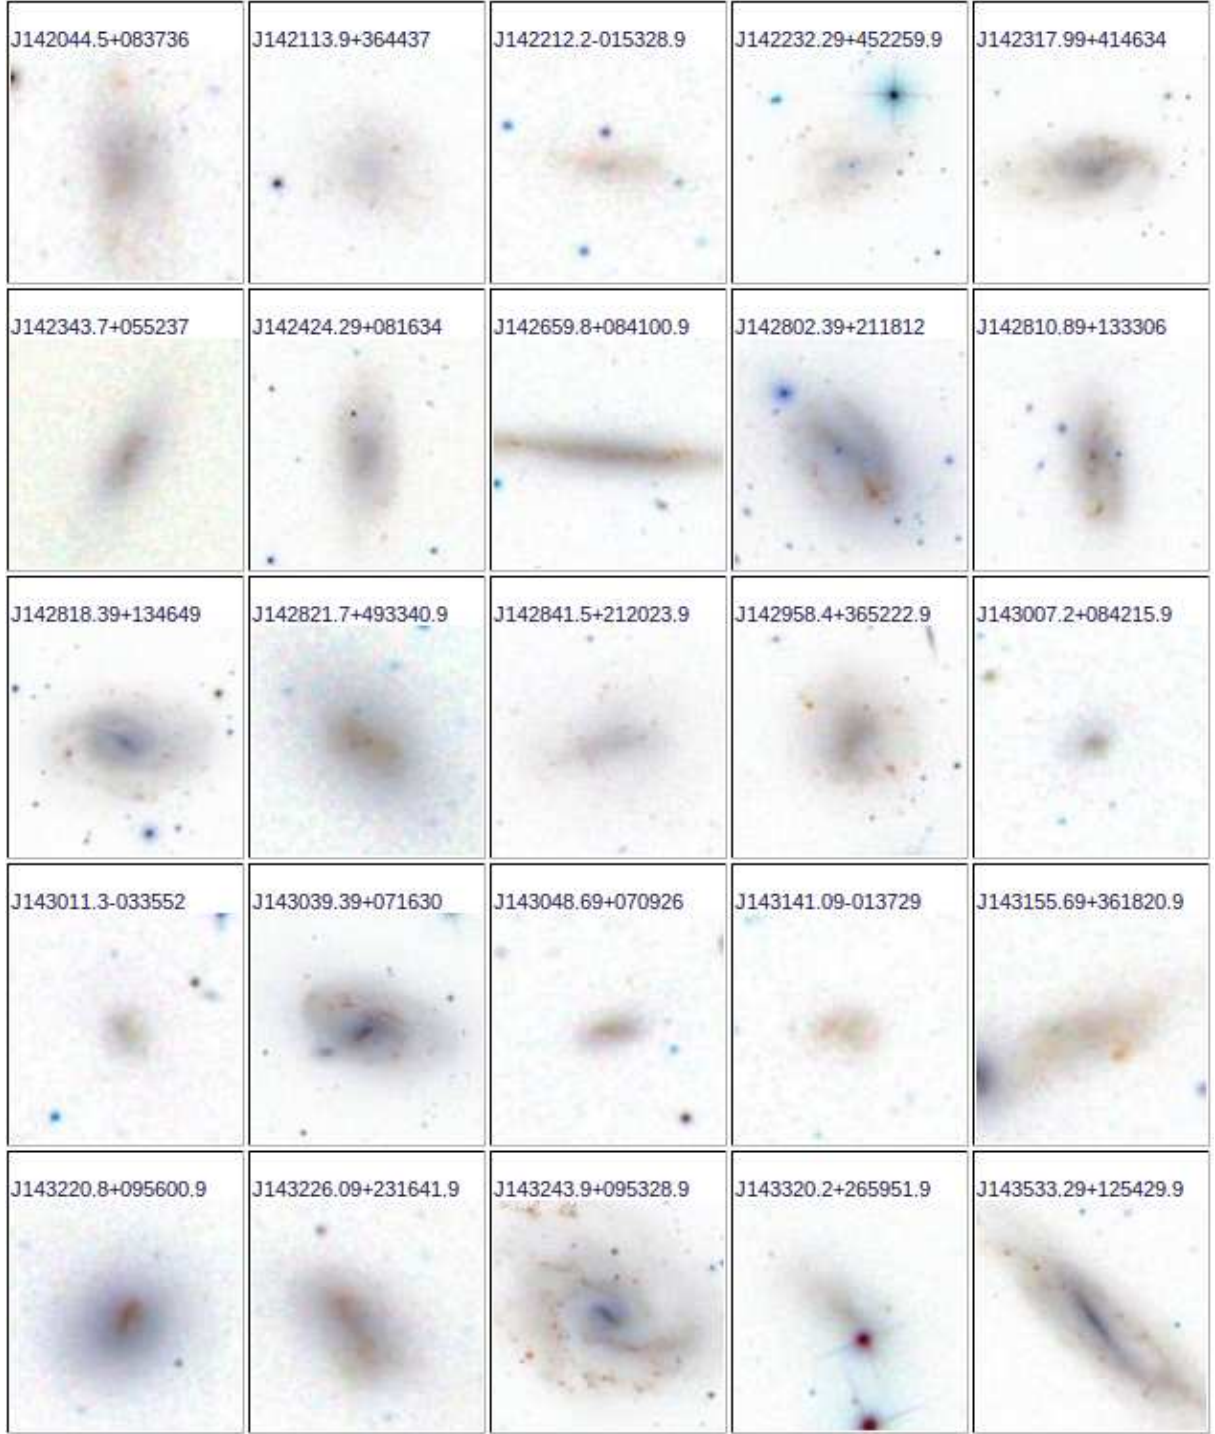

**Figure A19.** Mosaics of the next 25 'inner' nearby void galaxies prepared from the SDSS colour images. The side of the chart is 50".

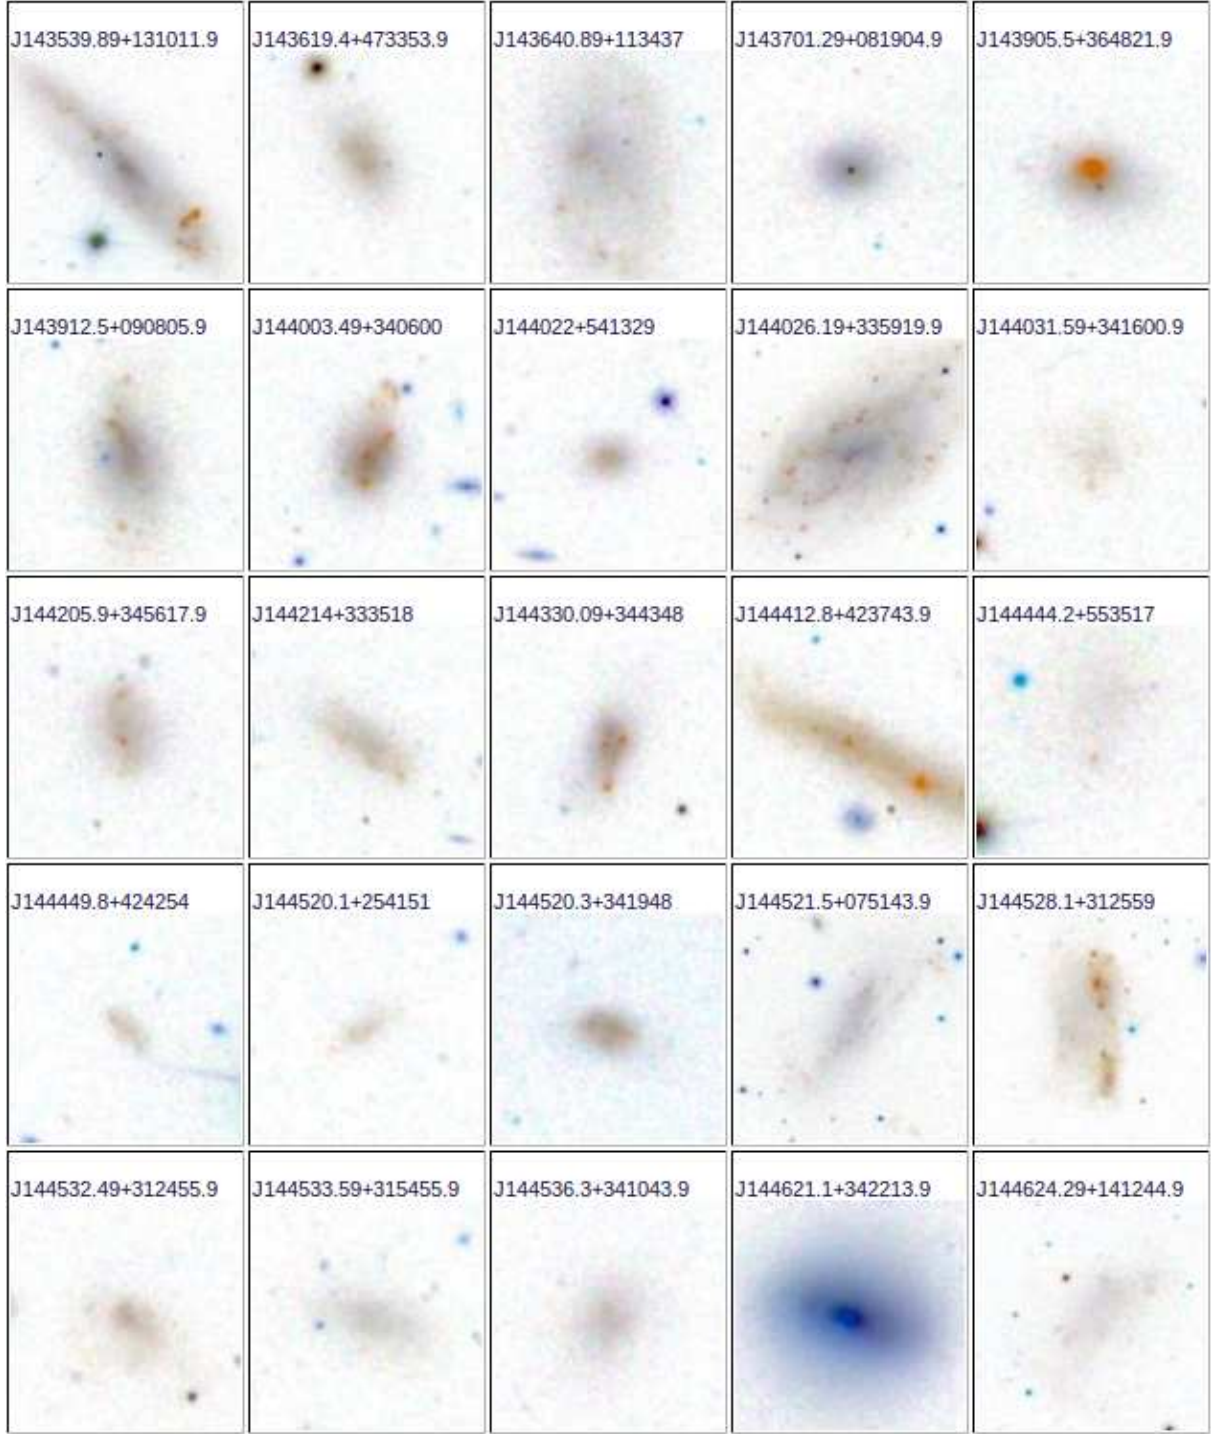

**Figure A20.** Mosaics of the next 25 'inner' nearby void galaxies prepared from the SDSS colour images. The side of the chart is 50".



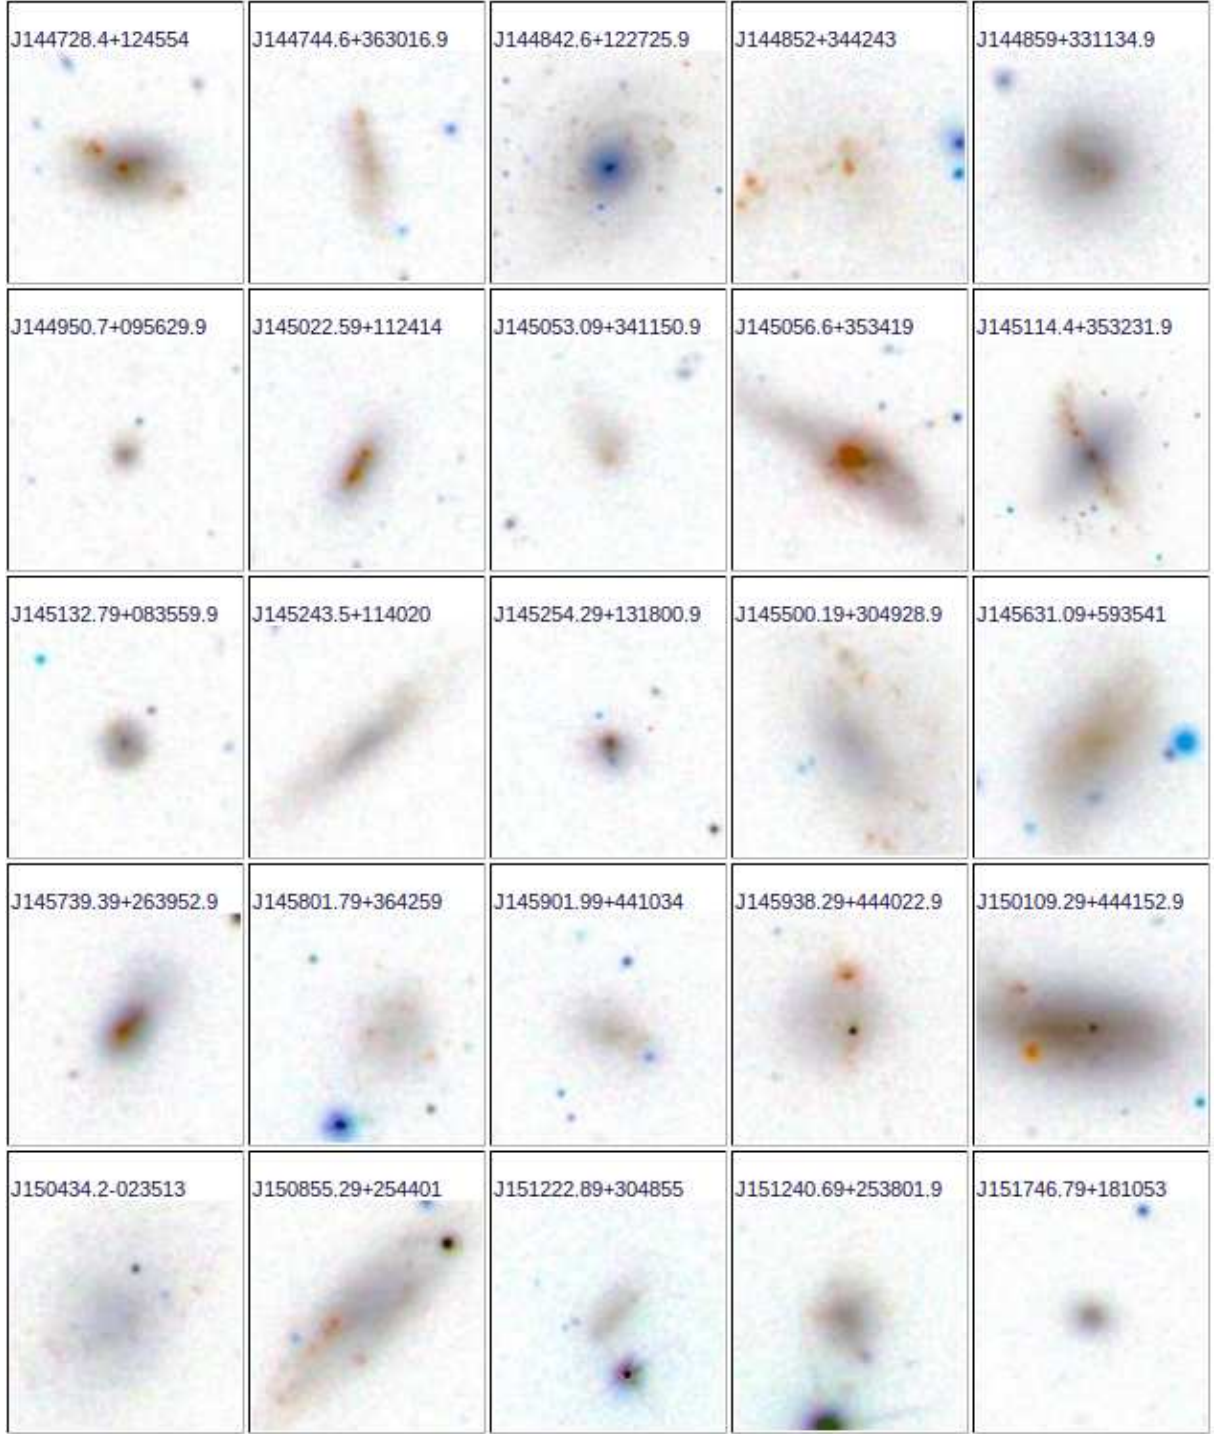

**Figure A21.** Mosaics of the next 25 'inner' nearby void galaxies prepared from the SDSS colour images. The side of the chart is 50".

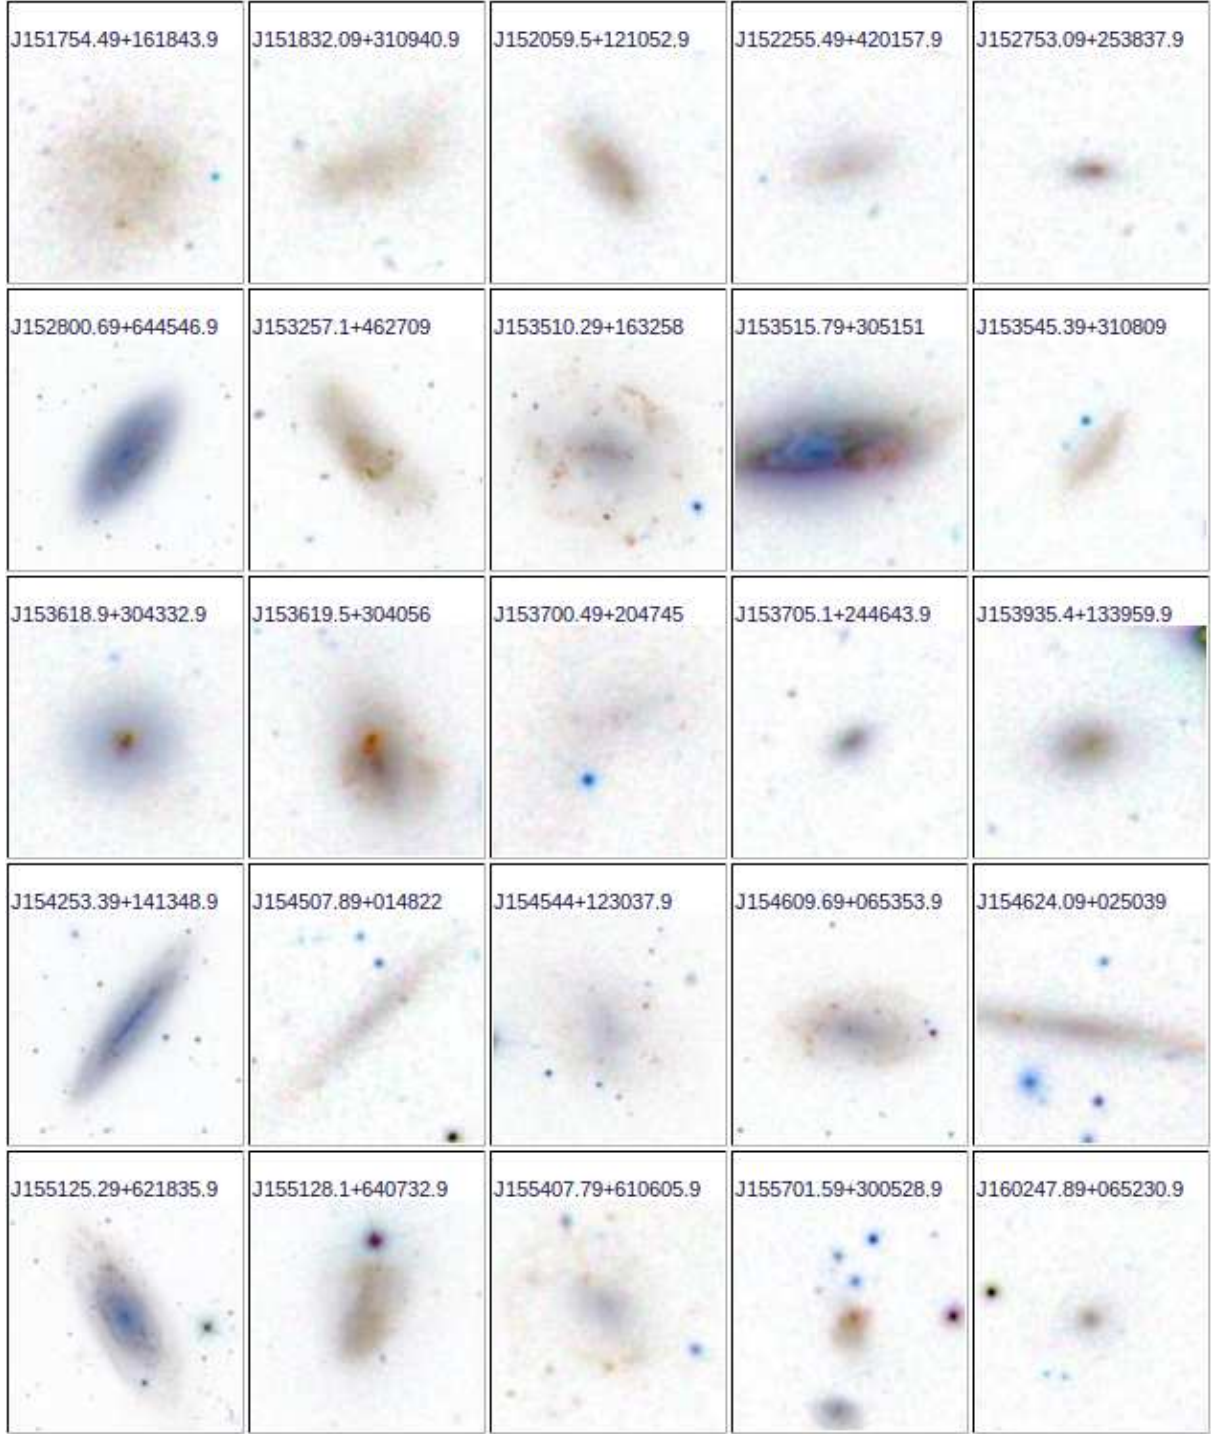

**Figure A22.** Mosaics of the next 25 'inner' nearby void galaxies prepared from the SDSS colour images. The side of the chart is 50".



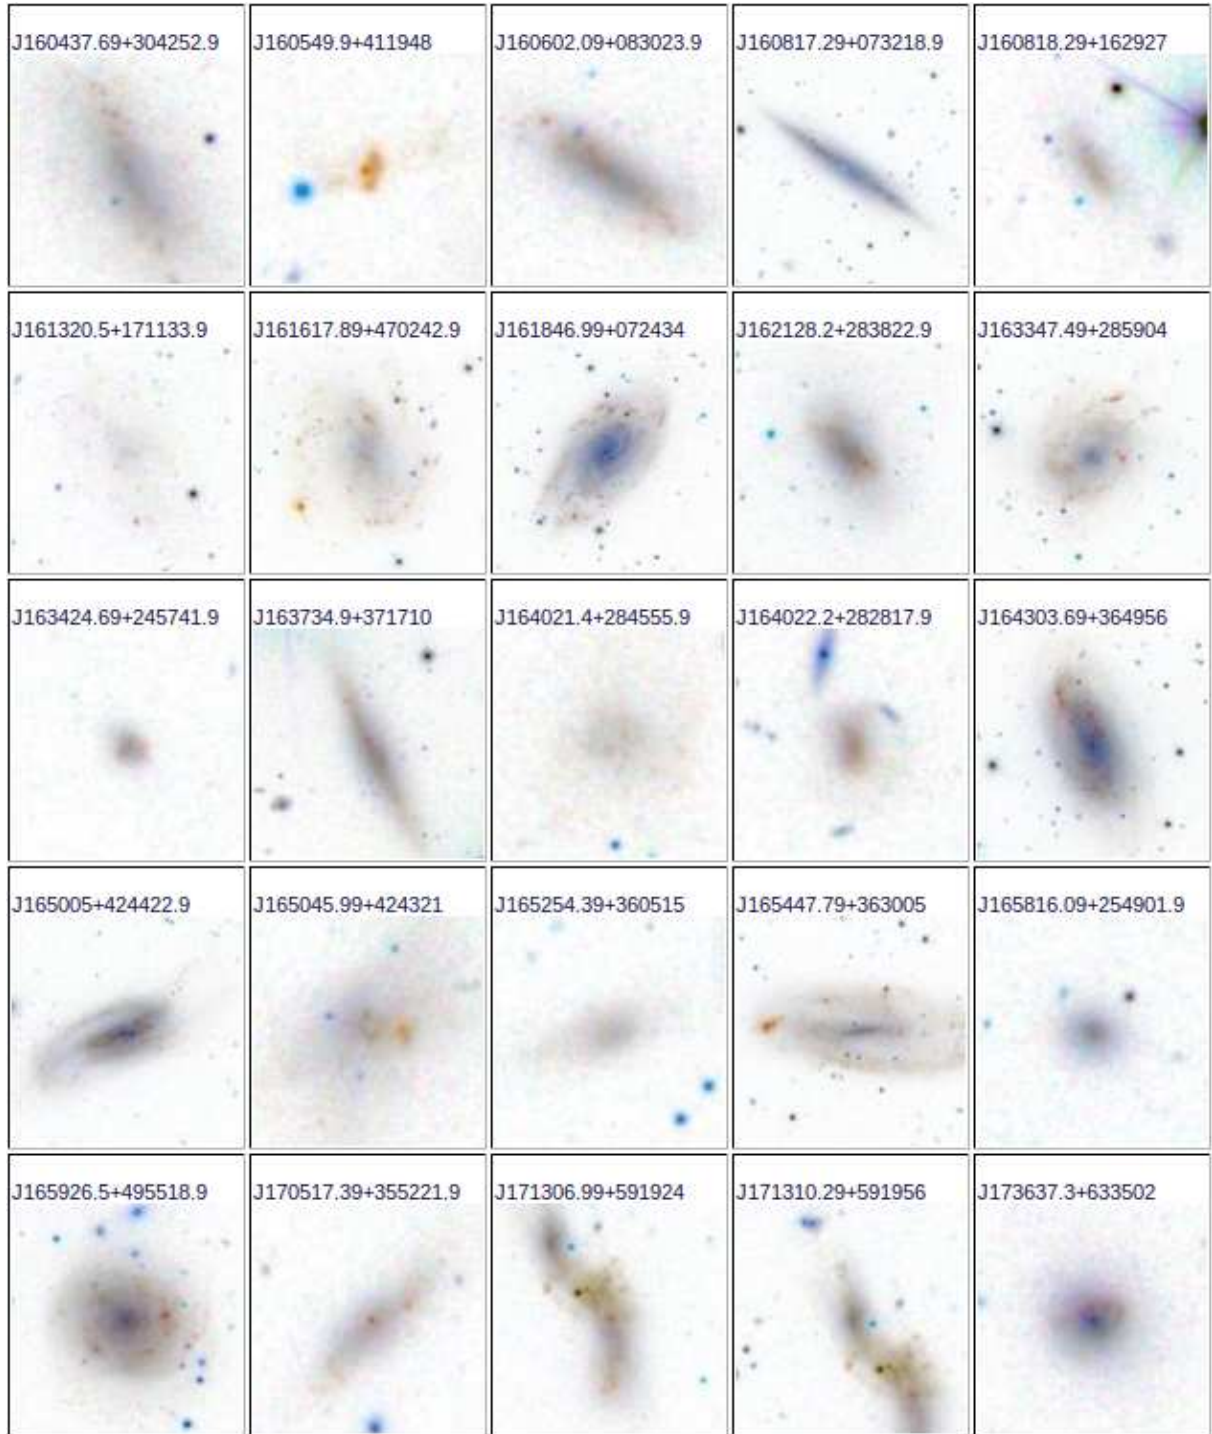

**Figure A23.** Mosaics of the next 25 'inner' nearby void galaxies prepared from the SDSS colour images. The side of the chart is 50".

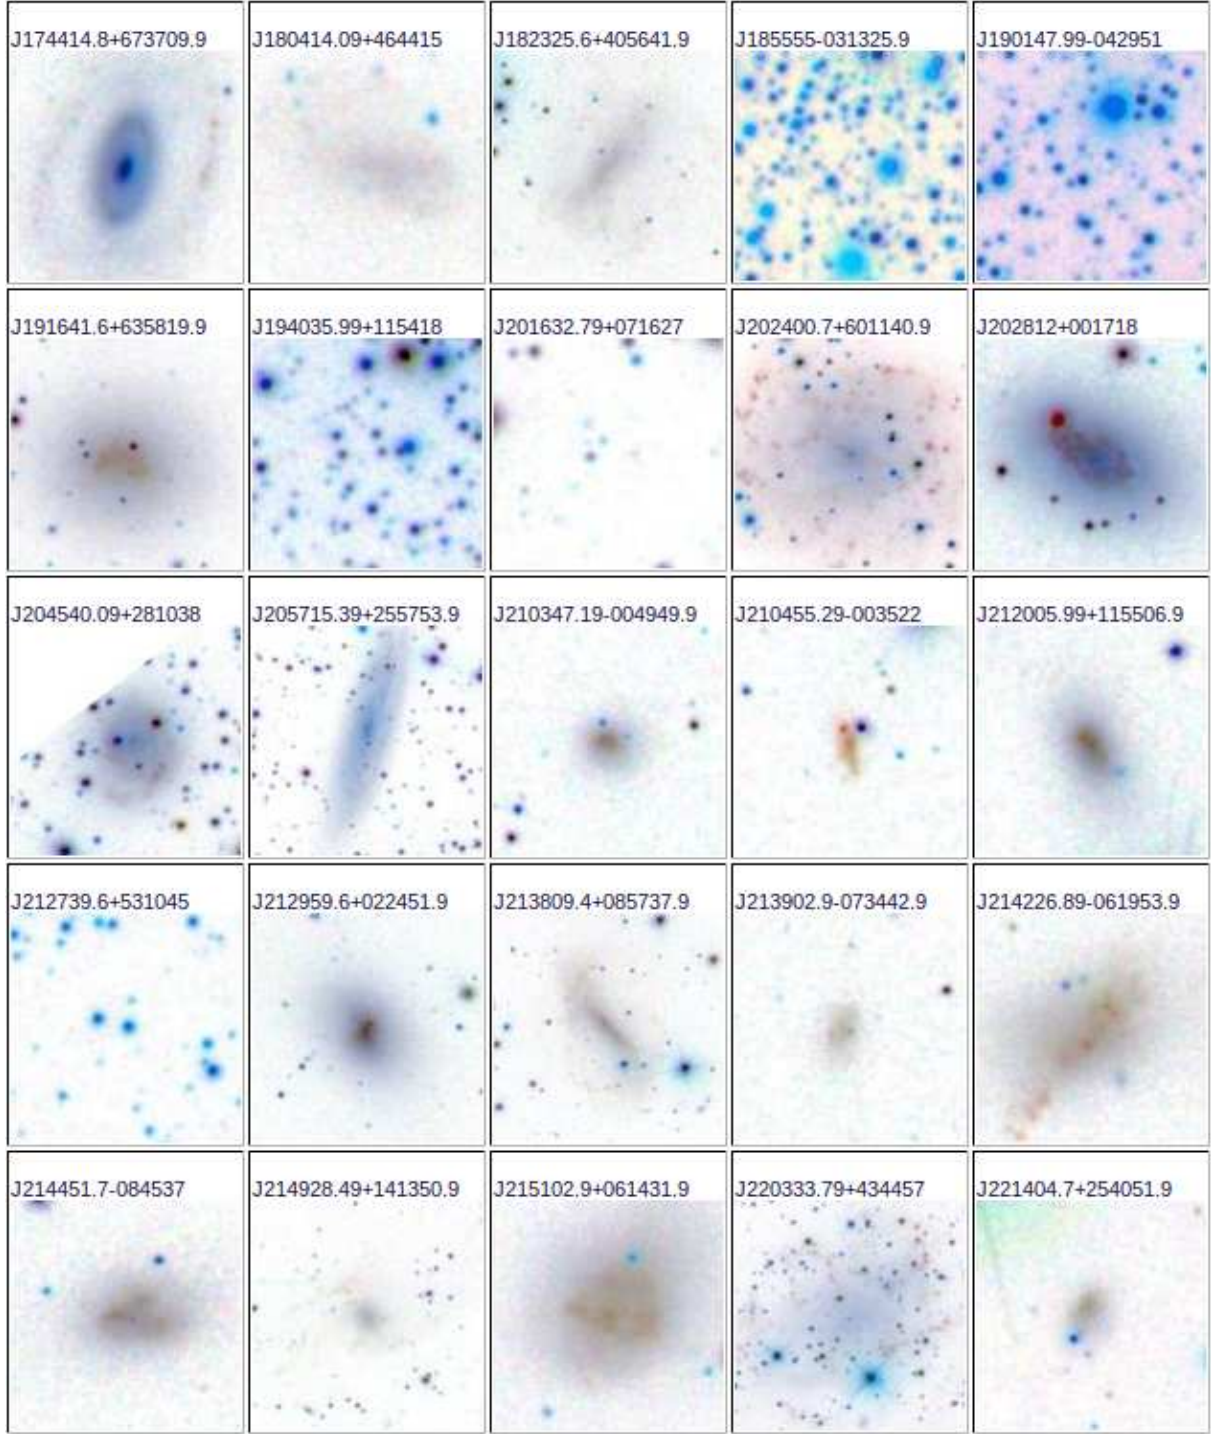

**Figure A24.** Mosaics of the next 25 'inner' nearby void galaxies prepared from the SDSS colour images. The side of the chart is 50".

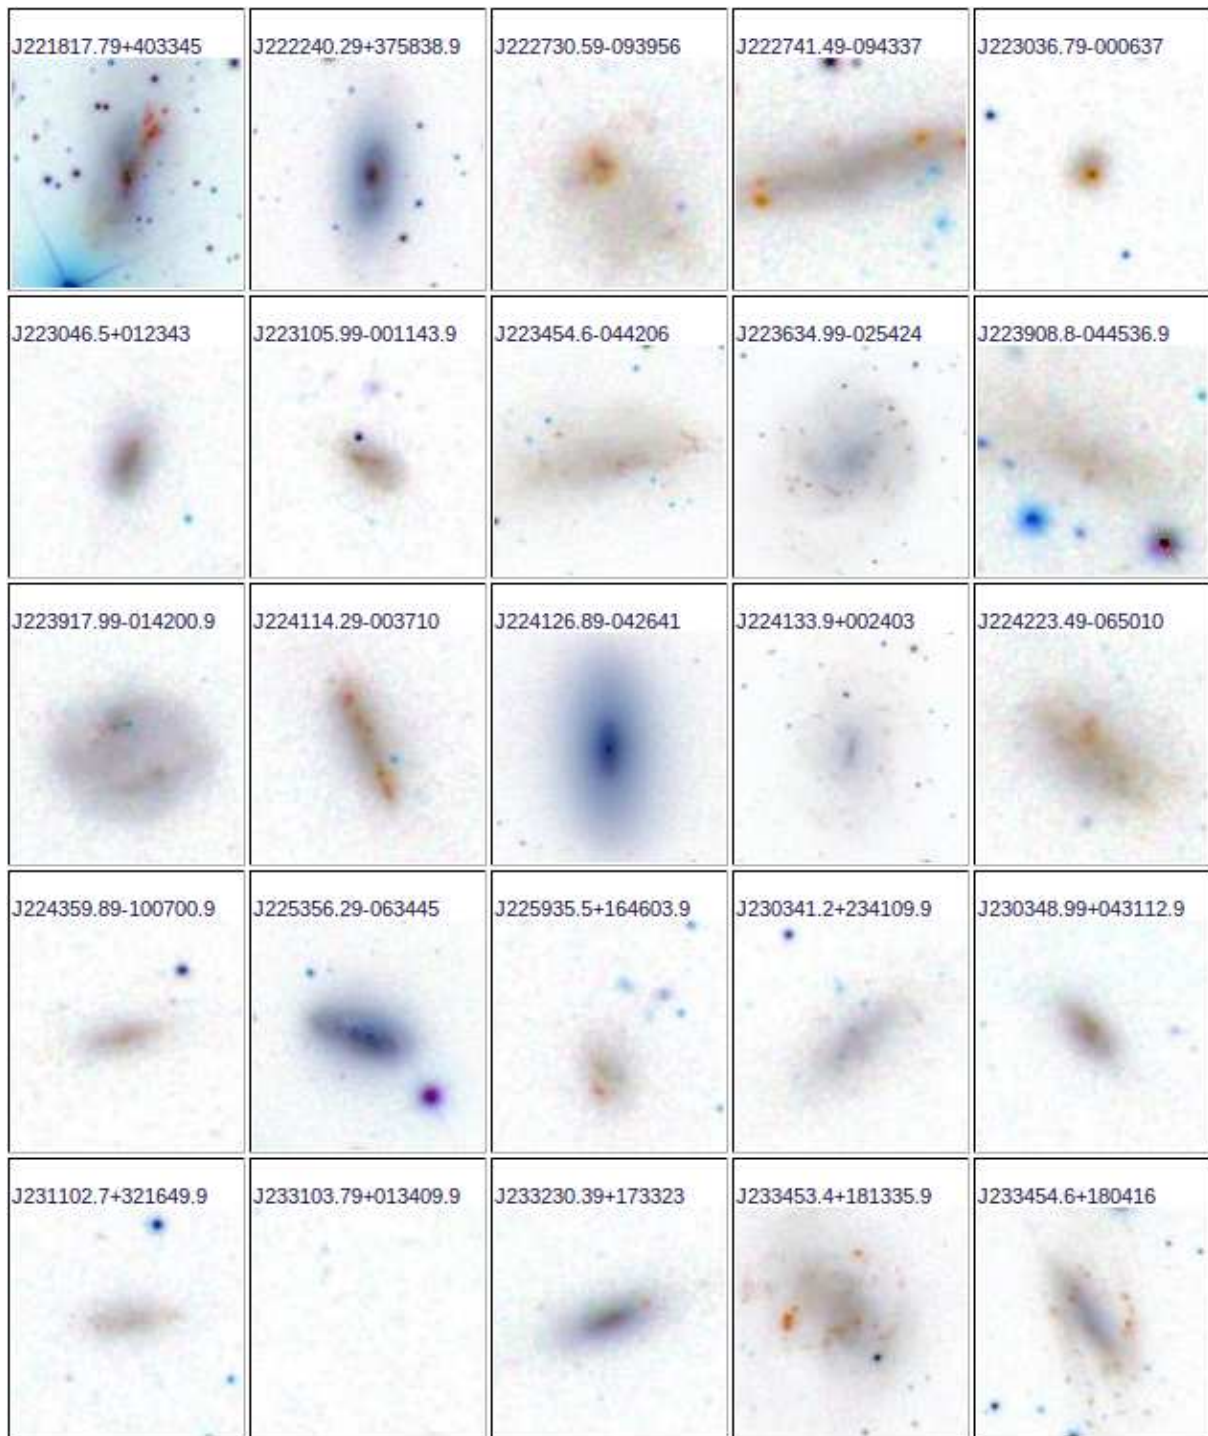

**Figure A25.** Mosaics of the last 25 'inner' nearby void galaxies prepared from the SDSS colour images. The side of the chart is 50".



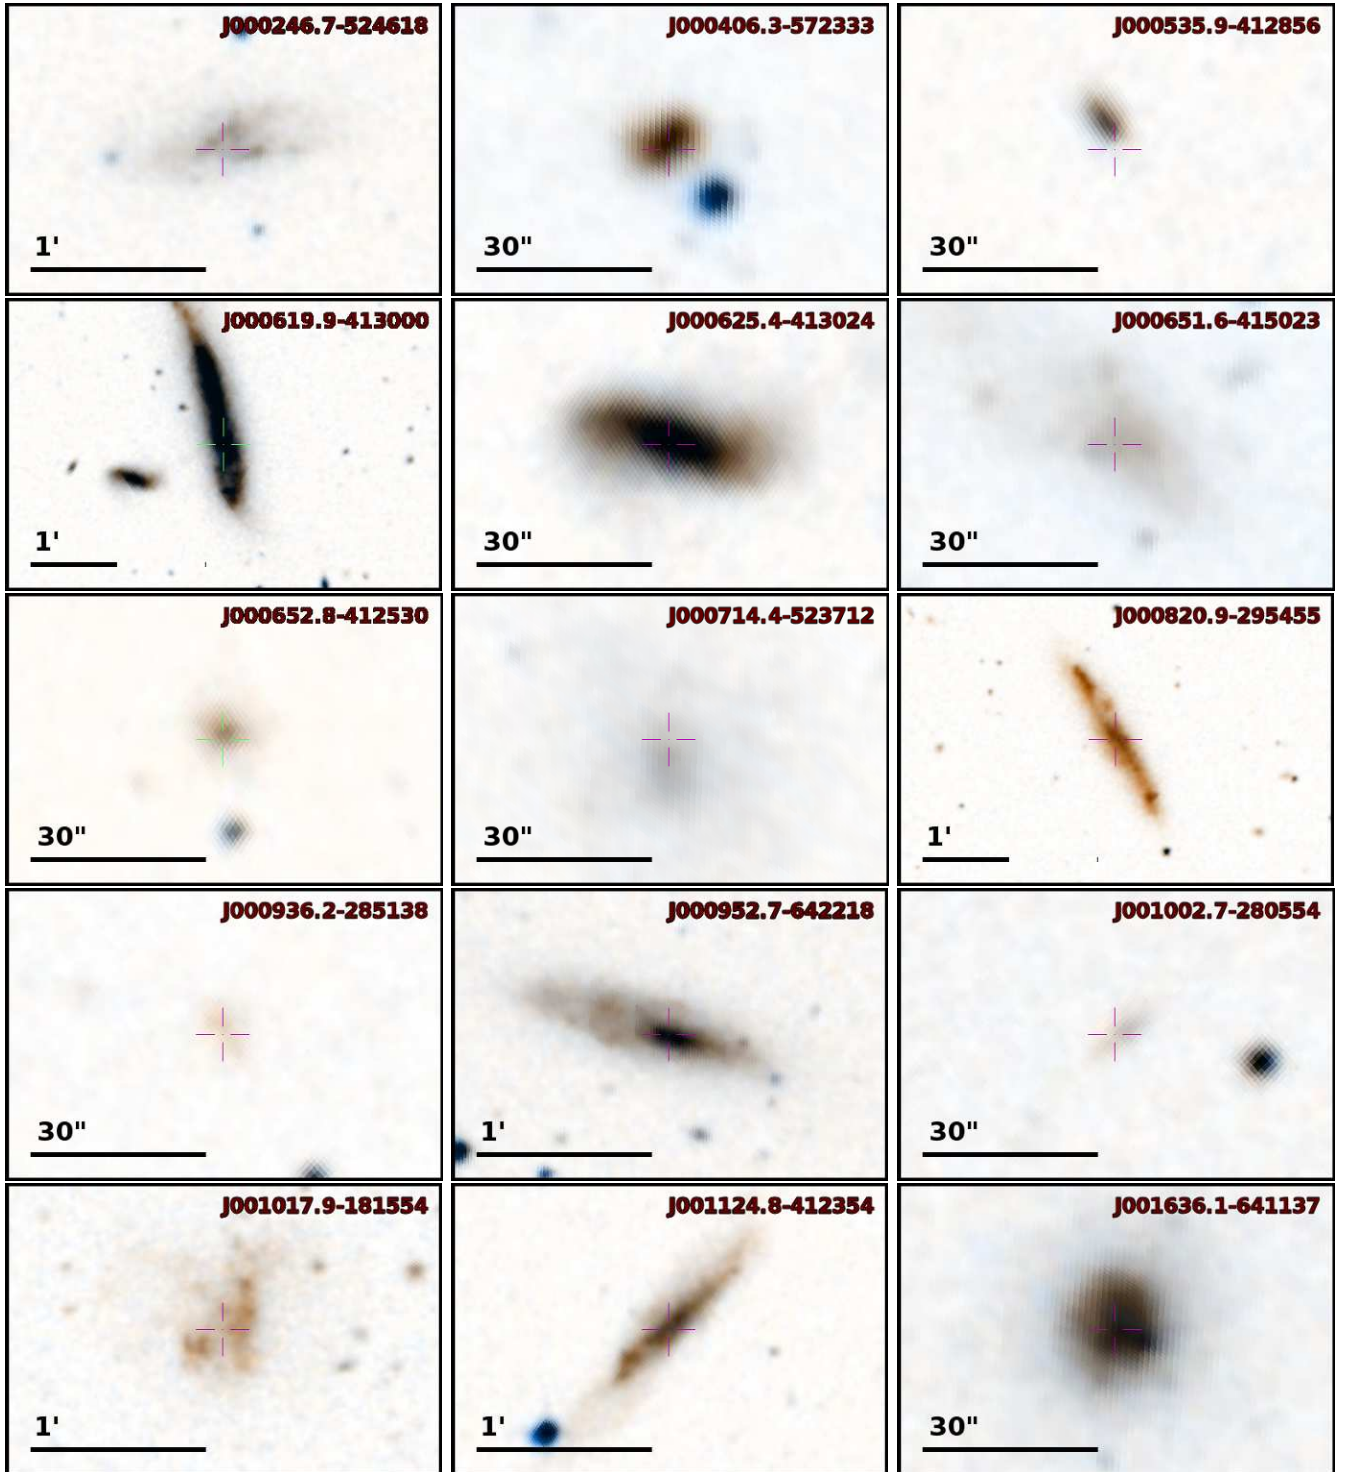

Figure A26. Nearby Void inner galaxies outside the SDSS footprint.

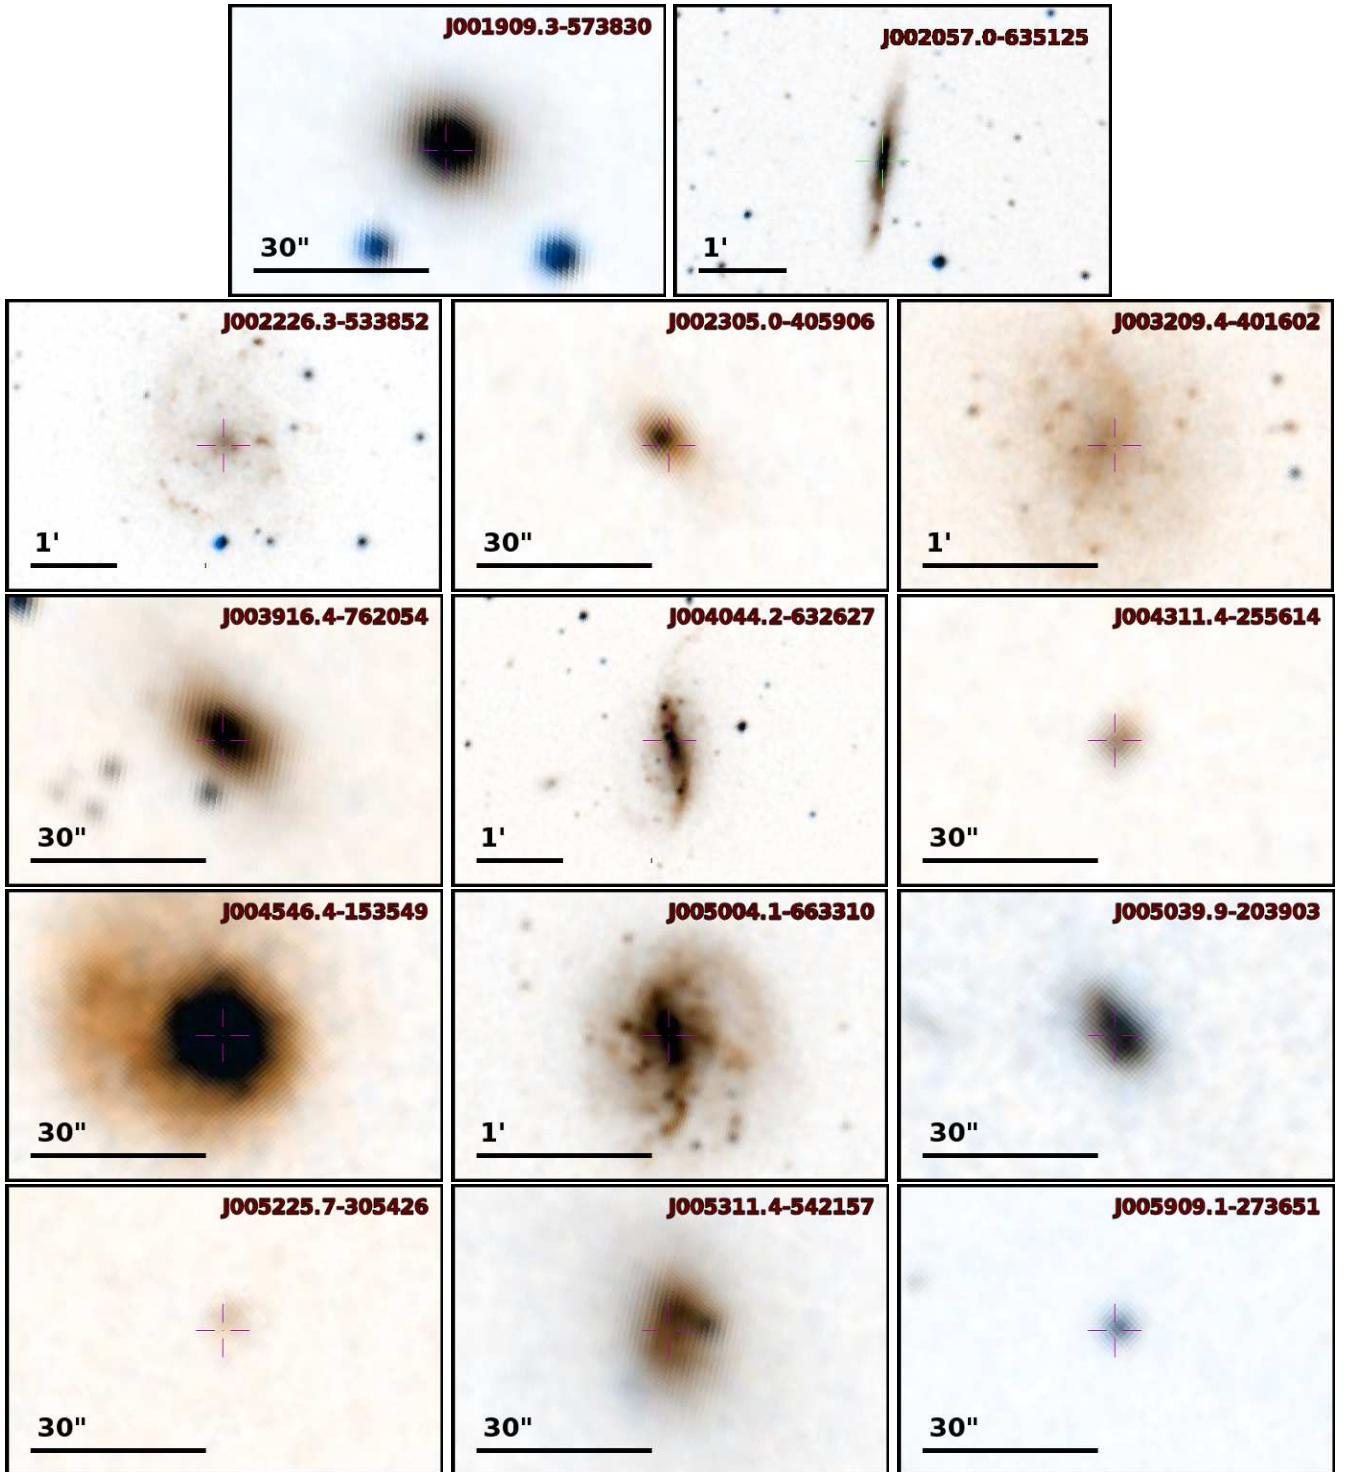

Figure A27. Nearby Void inner galaxies outside the SDSS footprint.

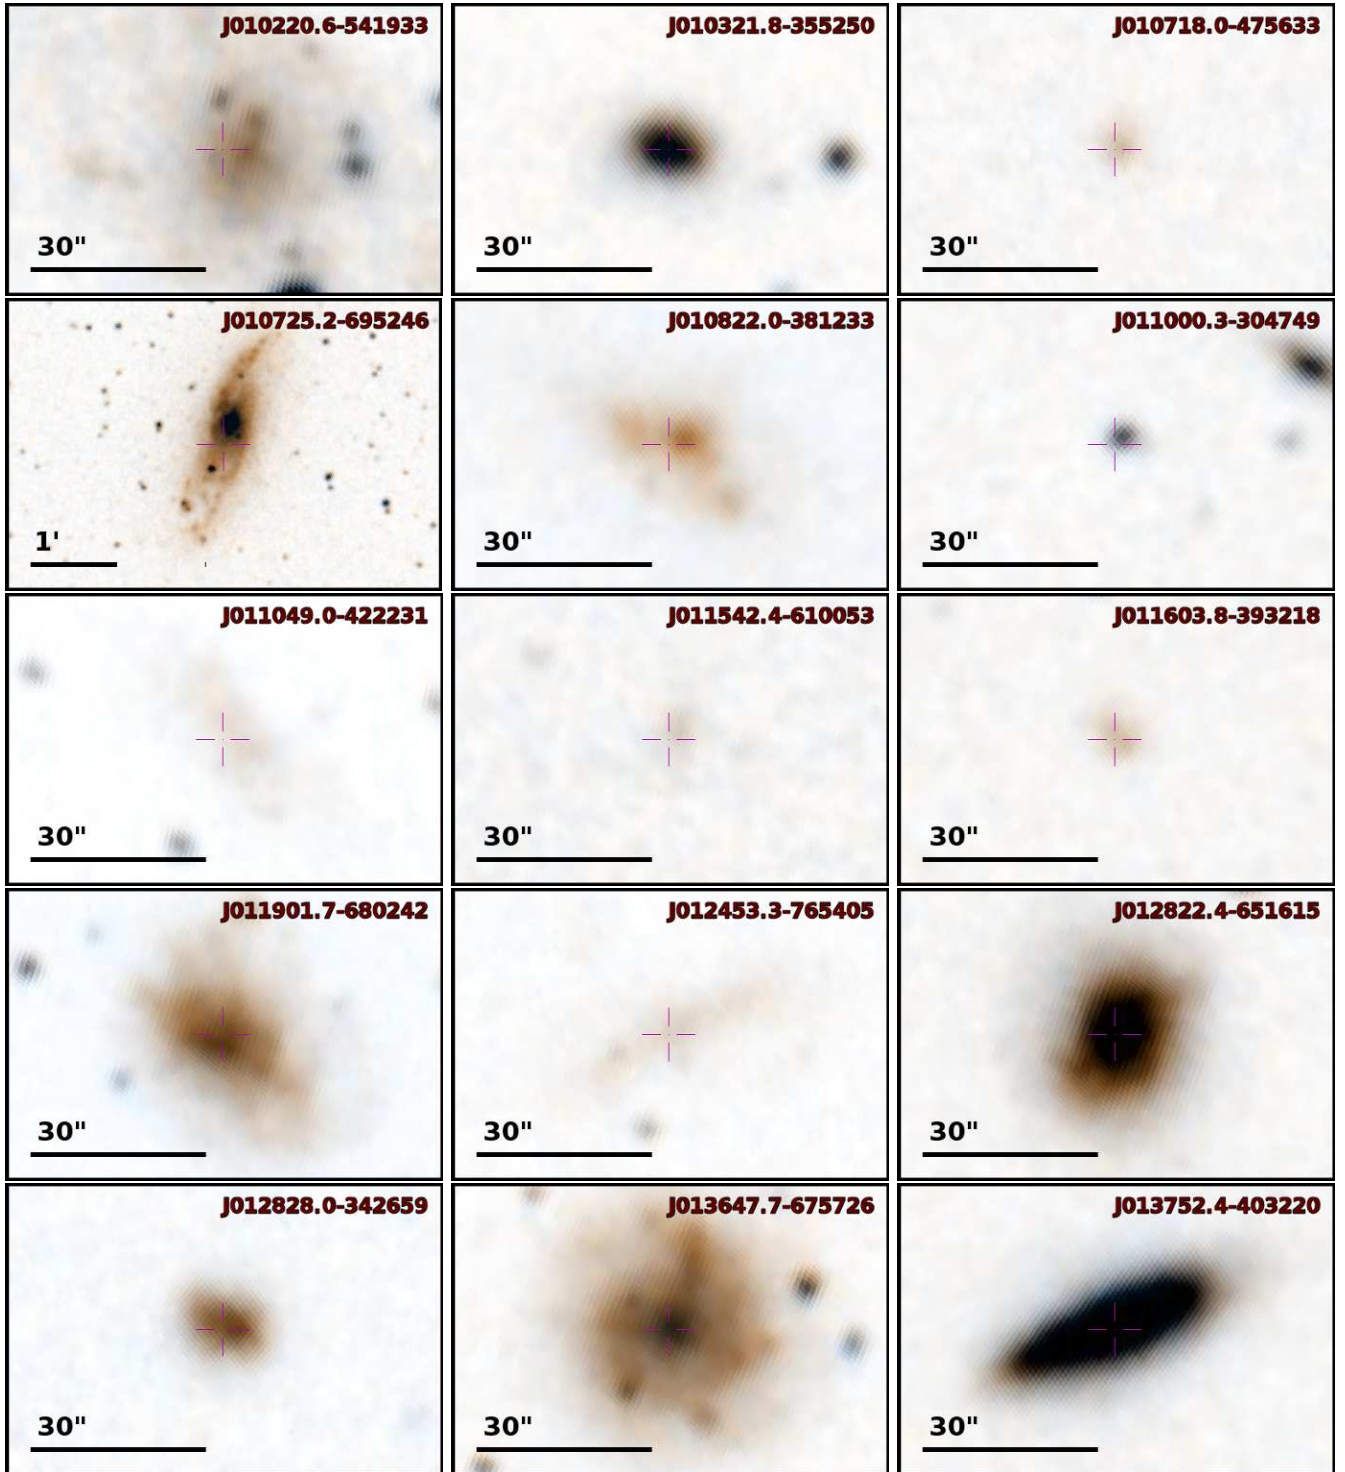

Figure A28. Nearby Void inner galaxies outside the SDSS footprint.



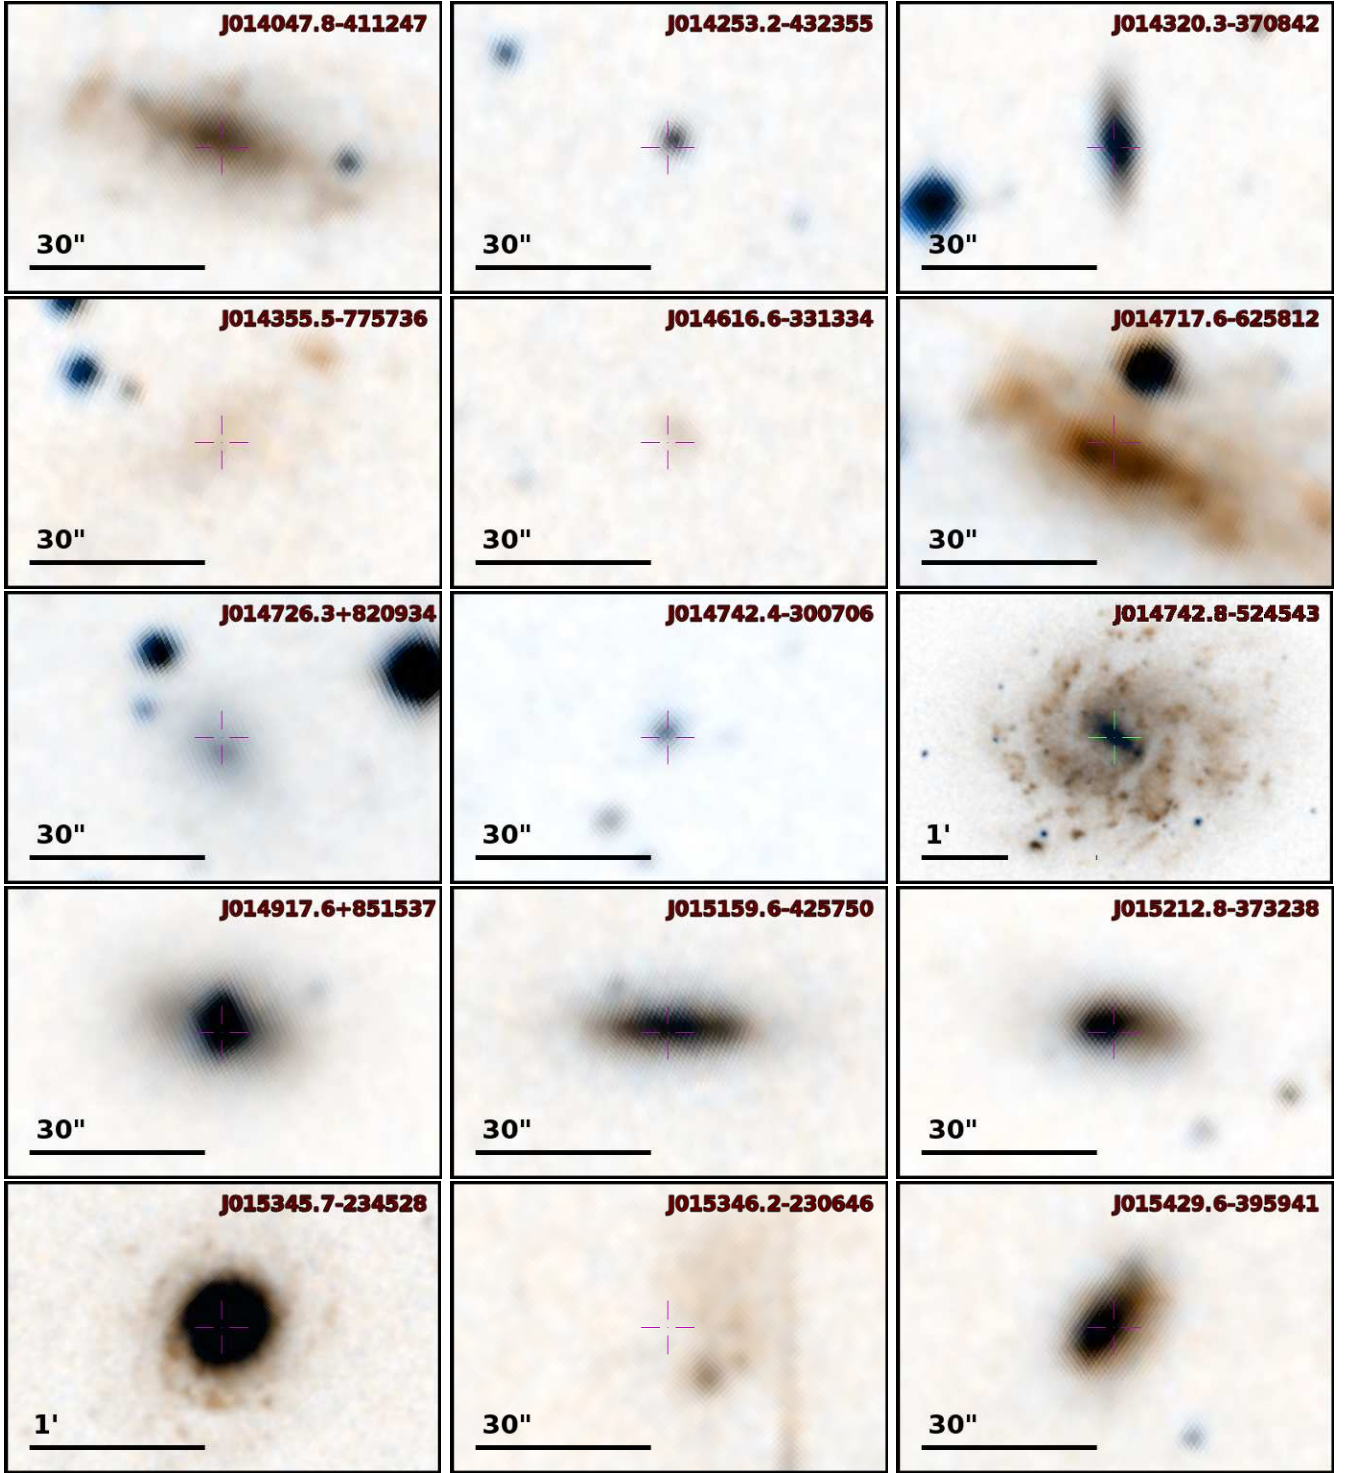

Figure A29. Nearby Void inner galaxies outside the SDSS footprint.



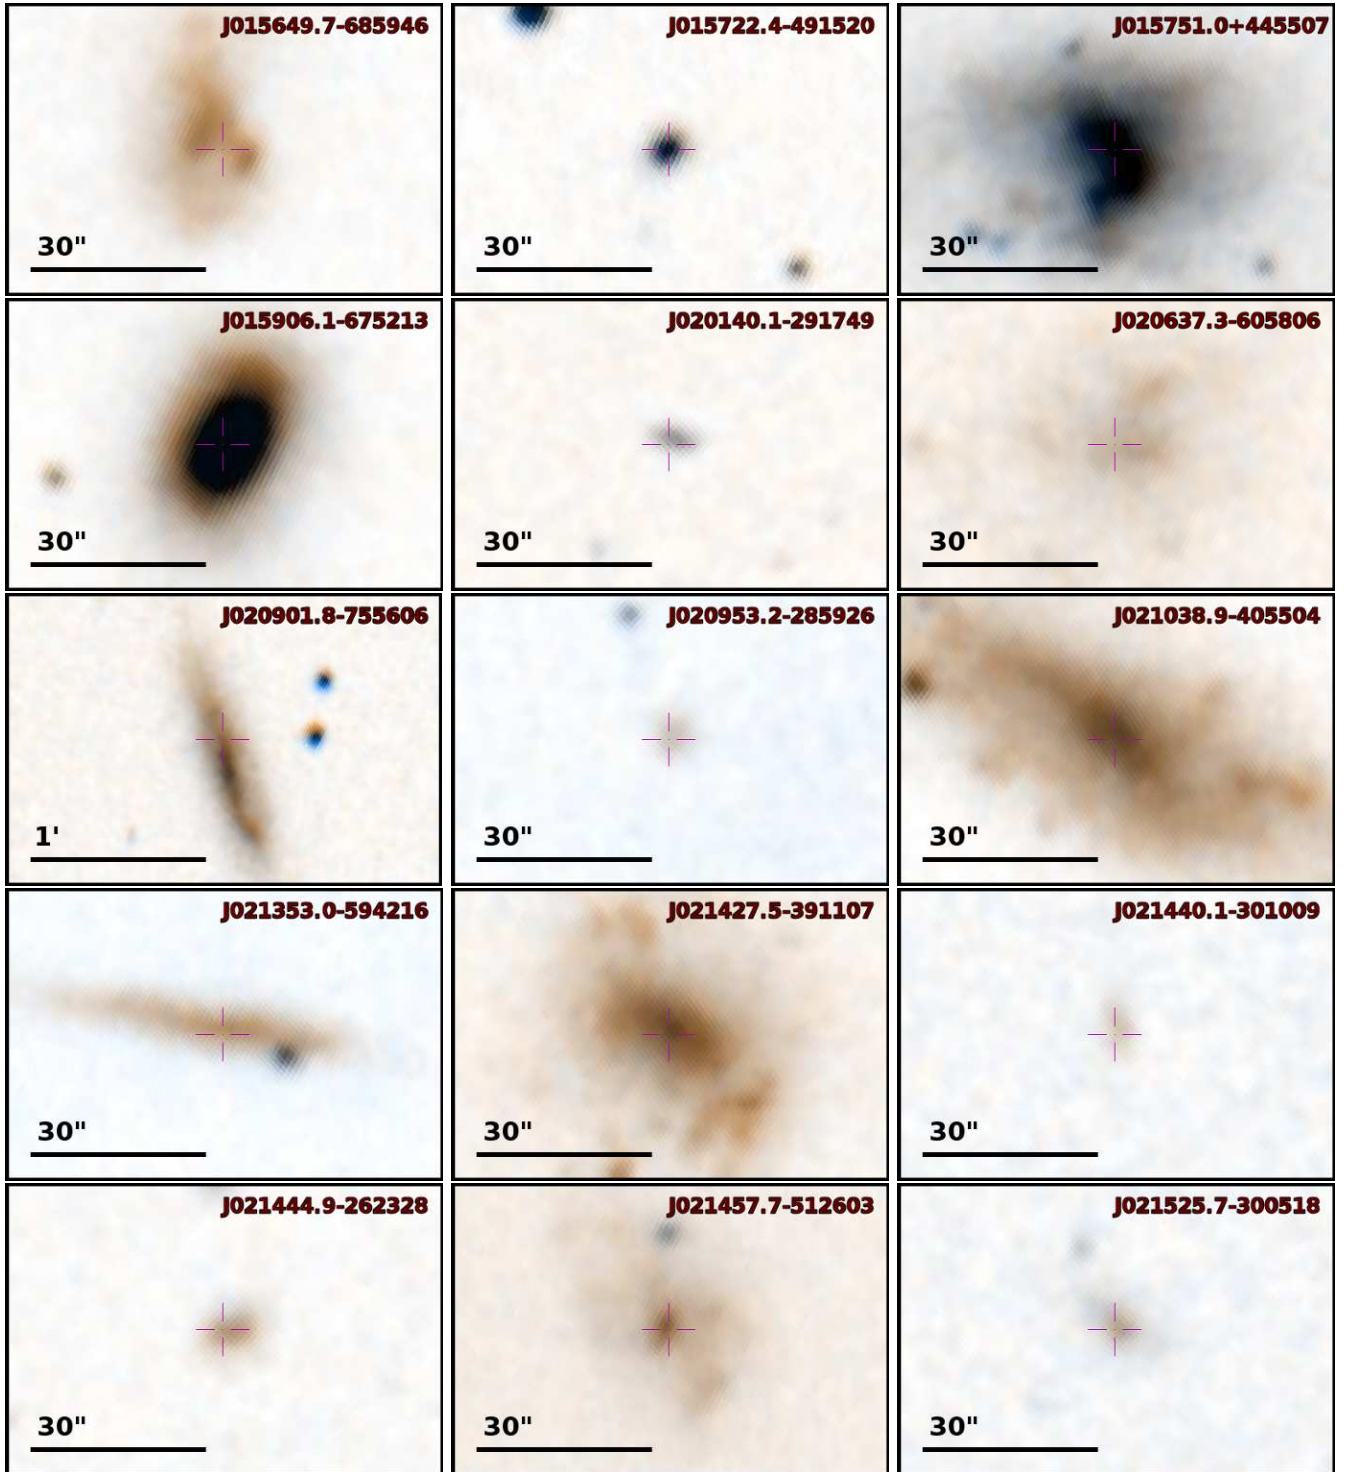

Figure A30. Nearby Void inner galaxies outside the SDSS footprint.

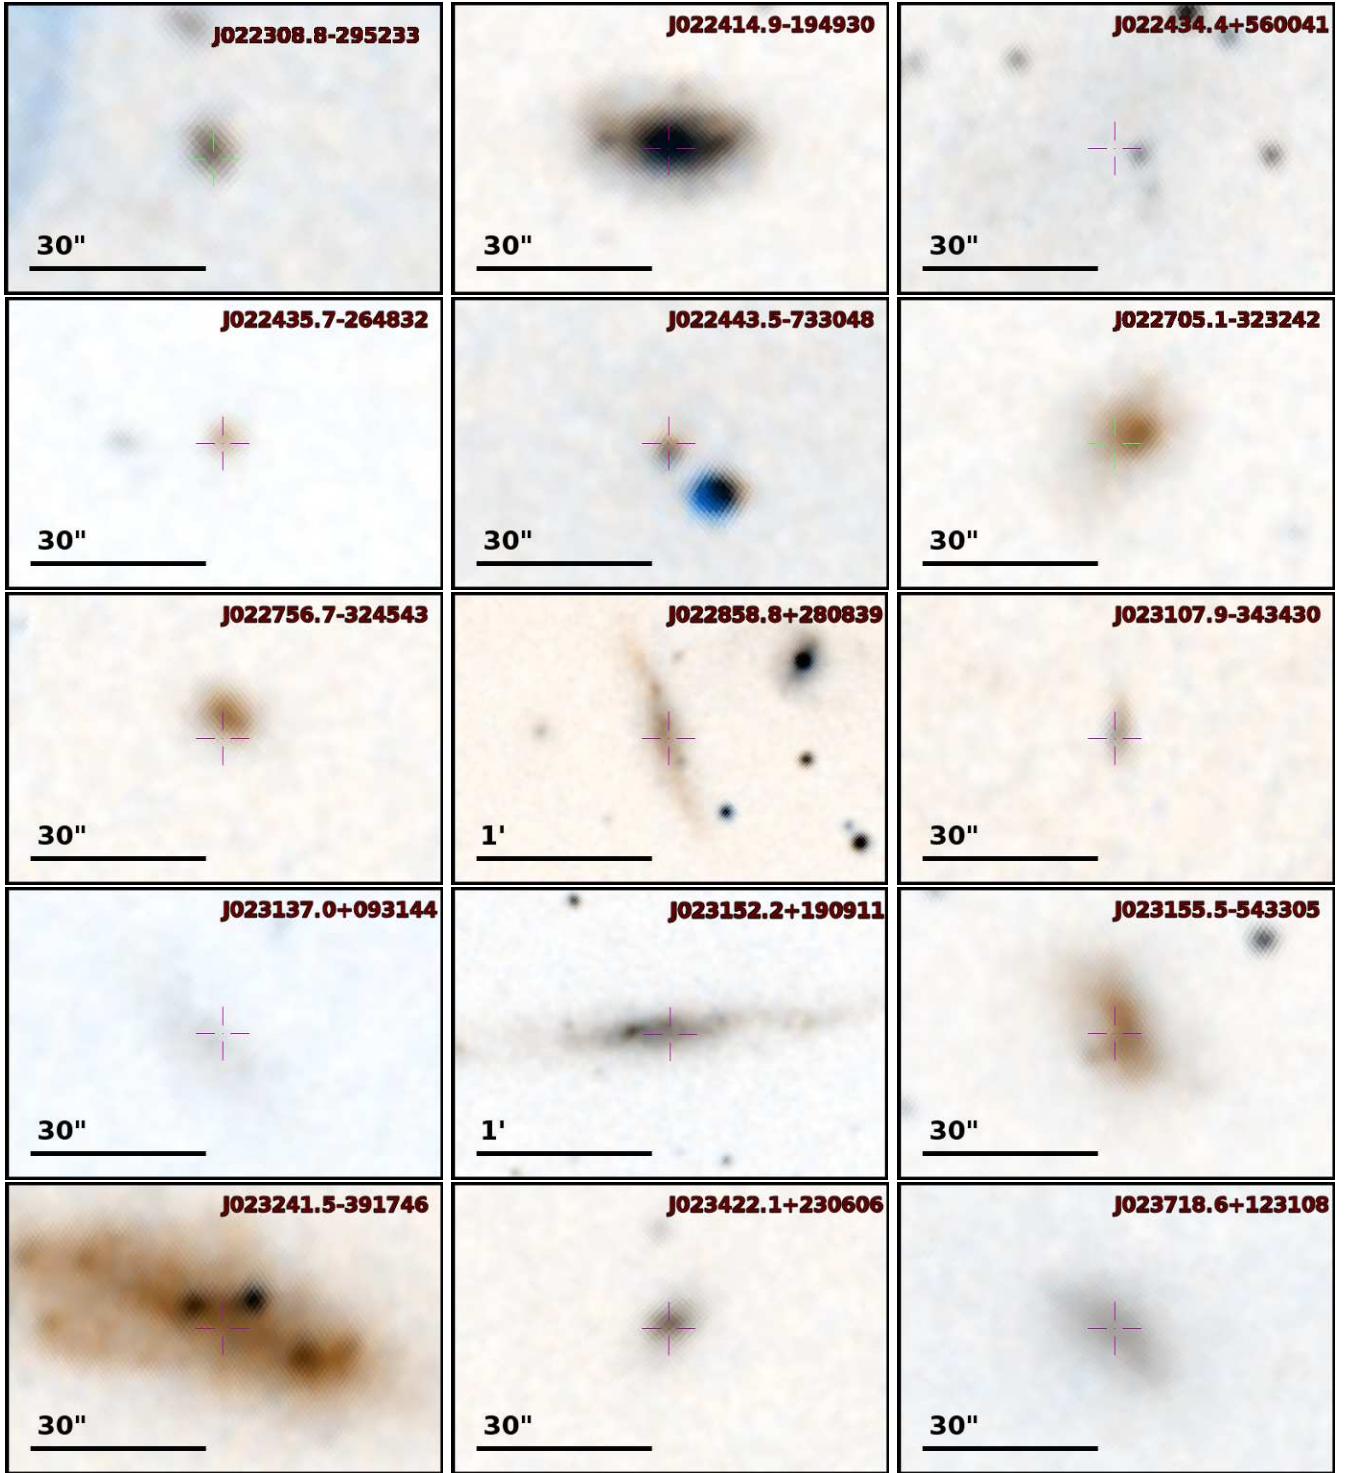

Figure A31. Nearby Void inner galaxies outside the SDSS footprint.

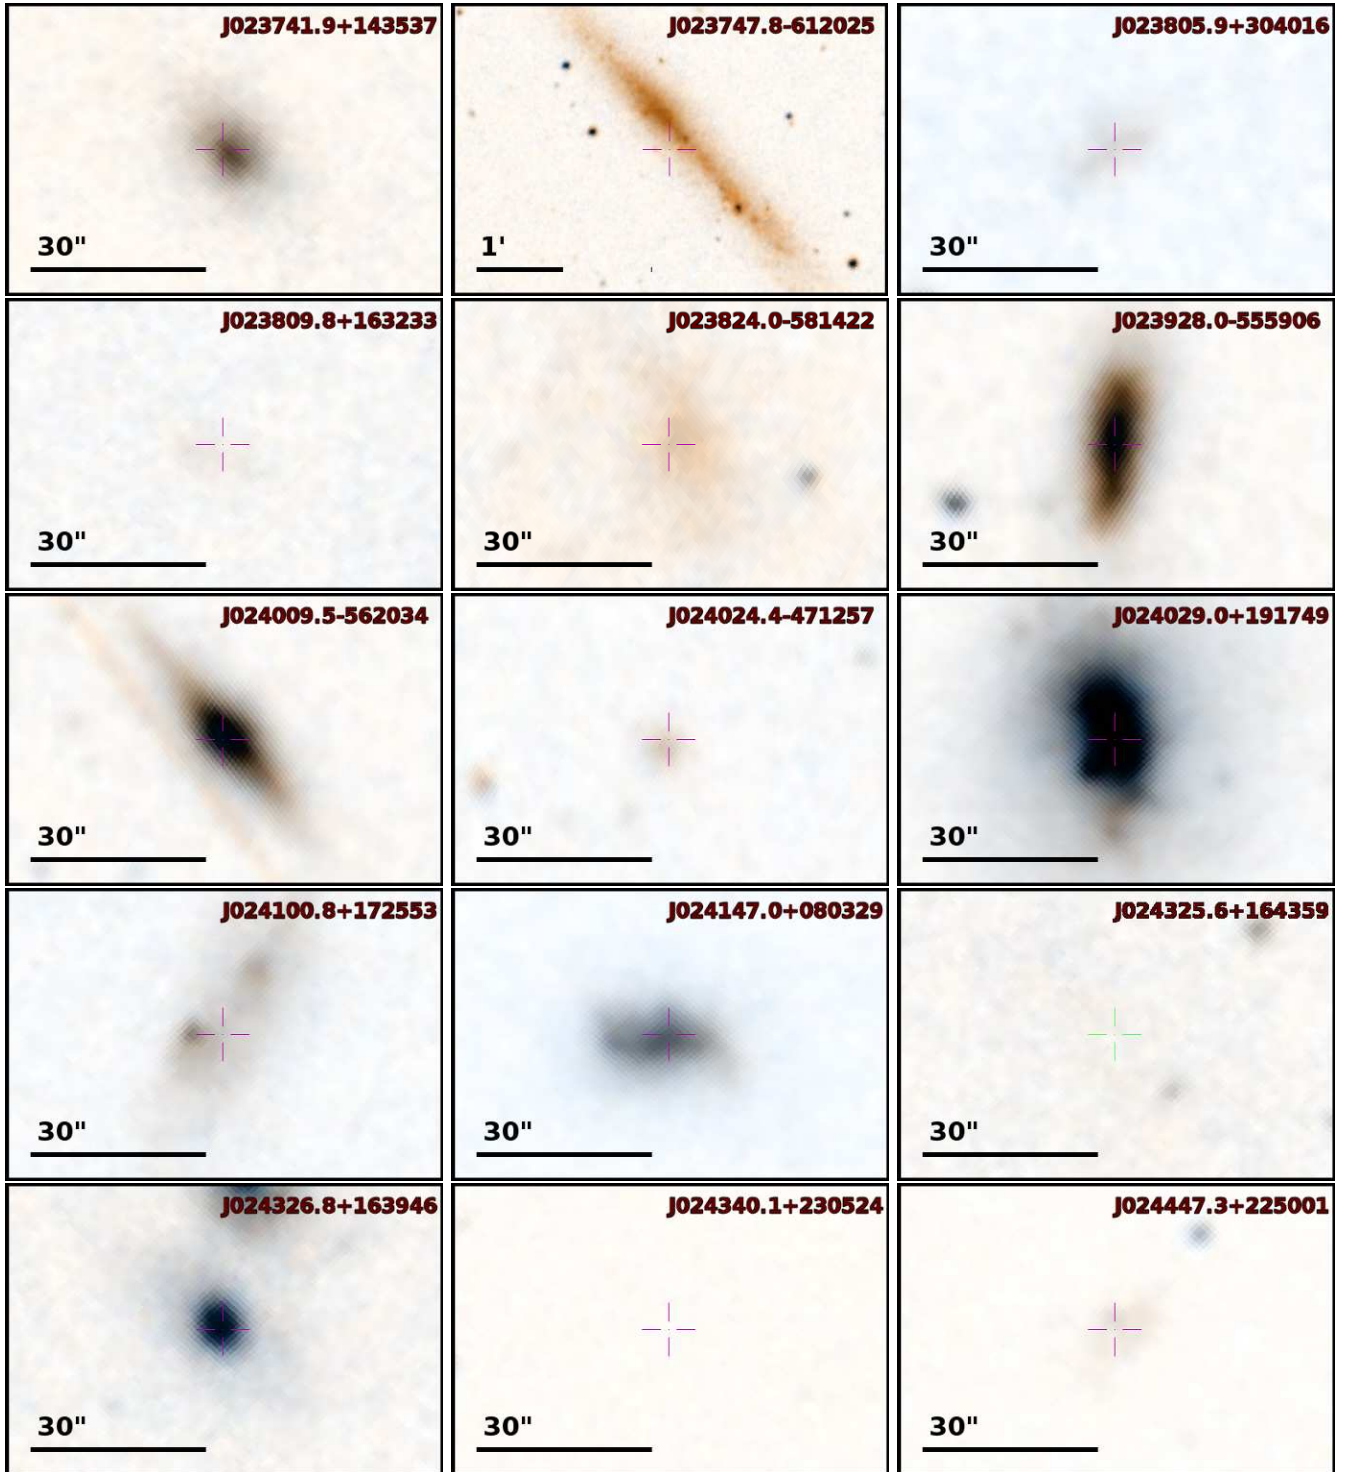

Figure A32. Nearby Void inner galaxies outside the SDSS footprint.



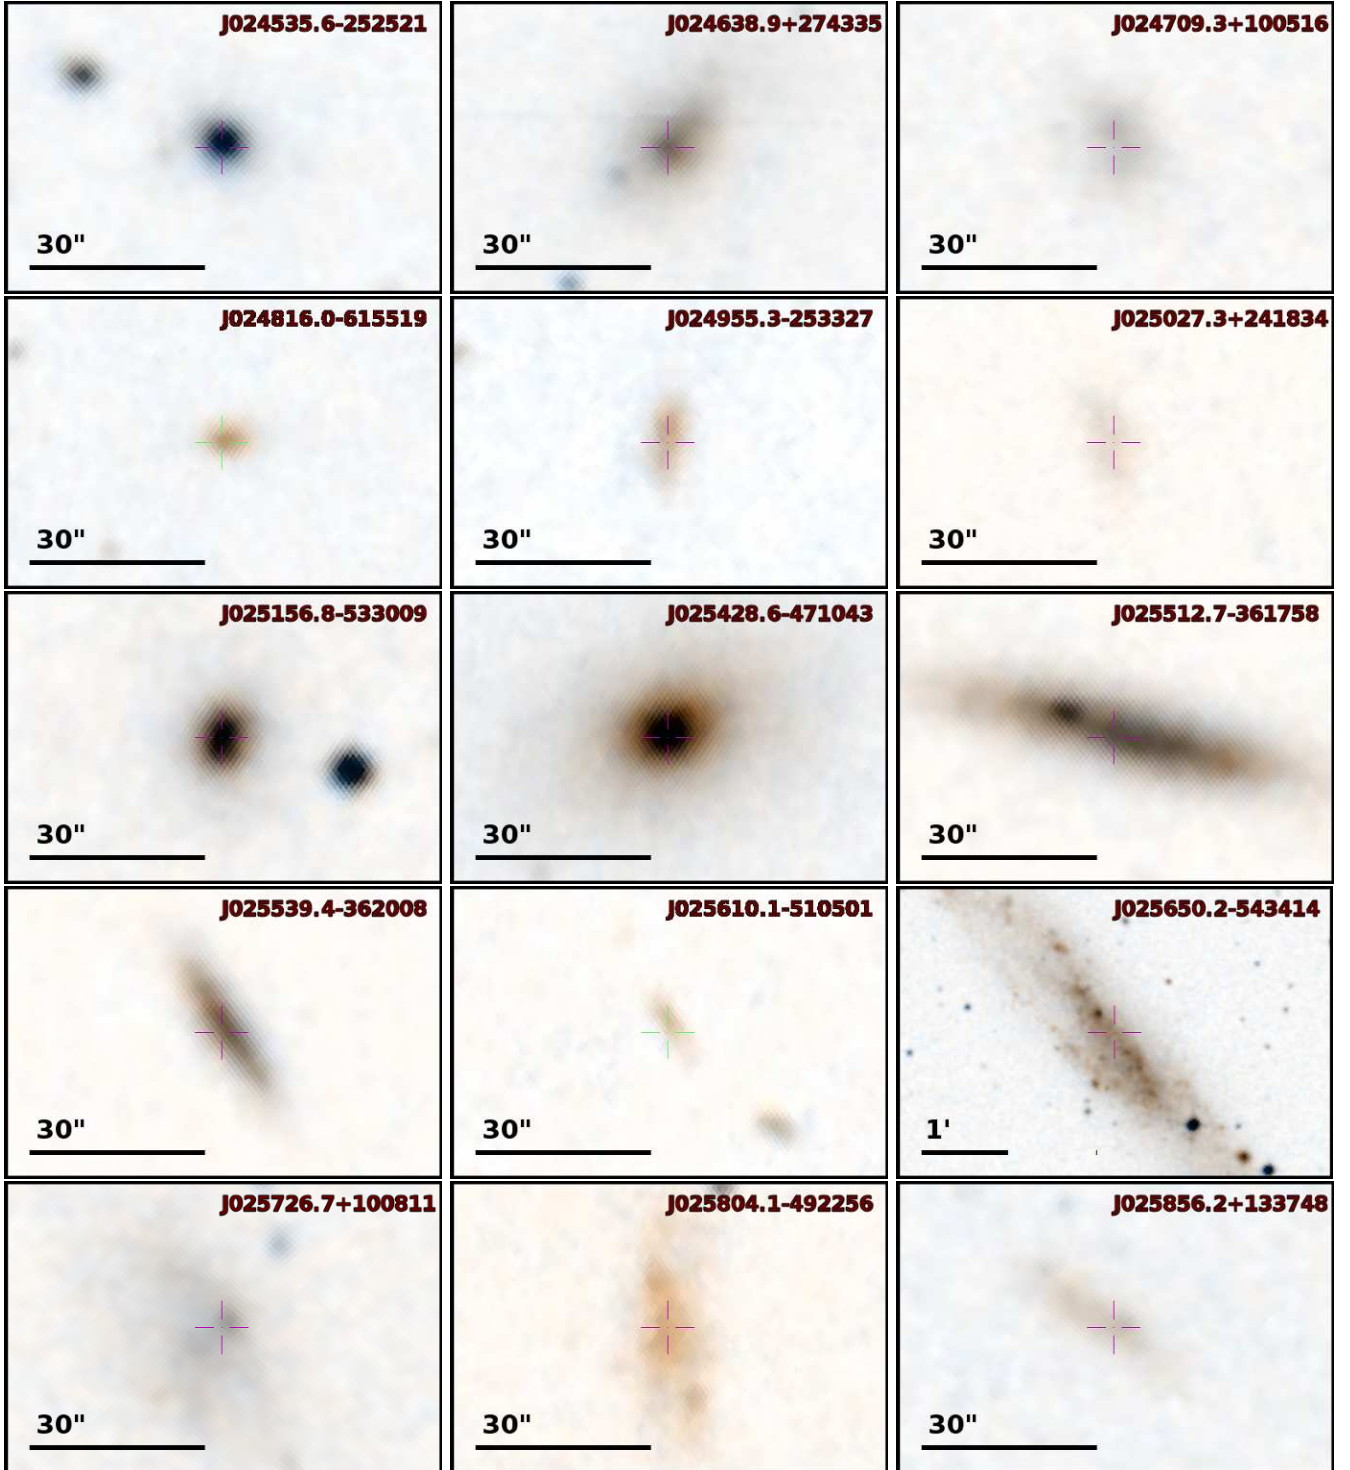

Figure A33. Nearby Void inner galaxies outside the SDSS footprint.

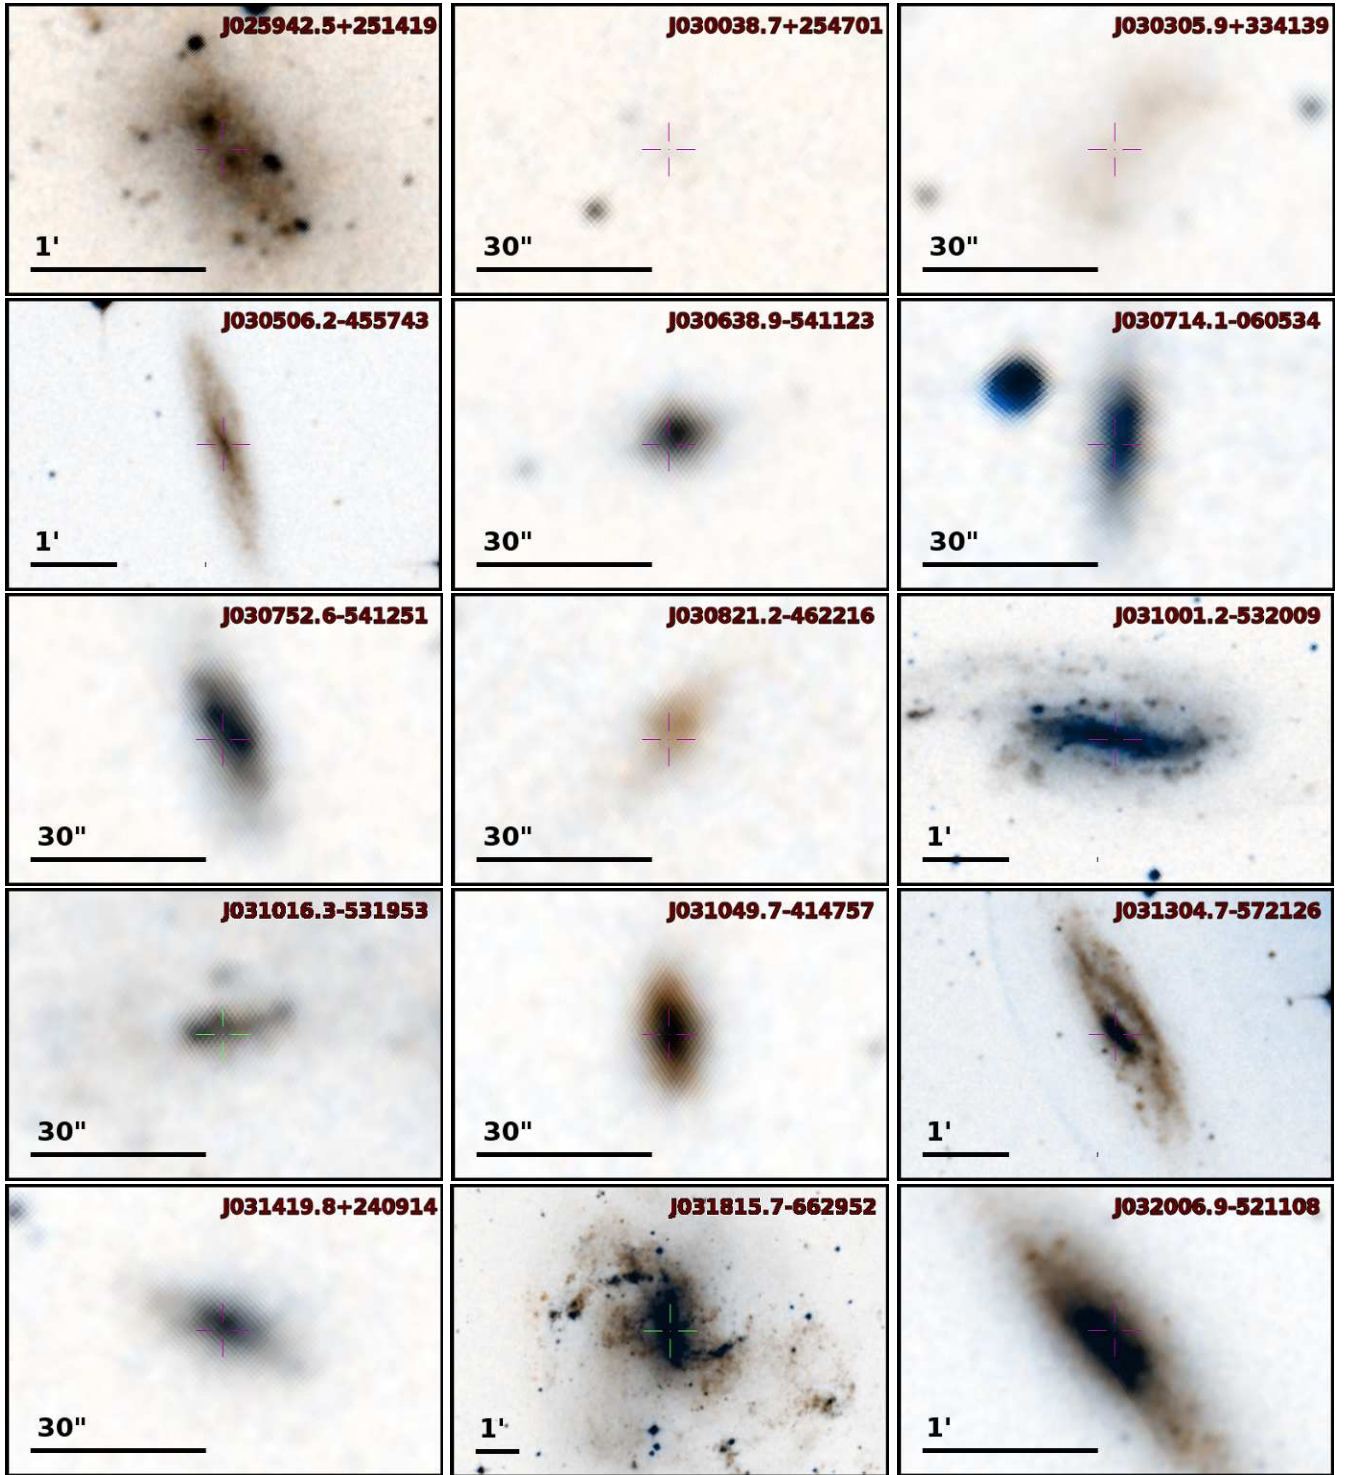

Figure A34. Nearby Void inner galaxies outside the SDSS footprint.

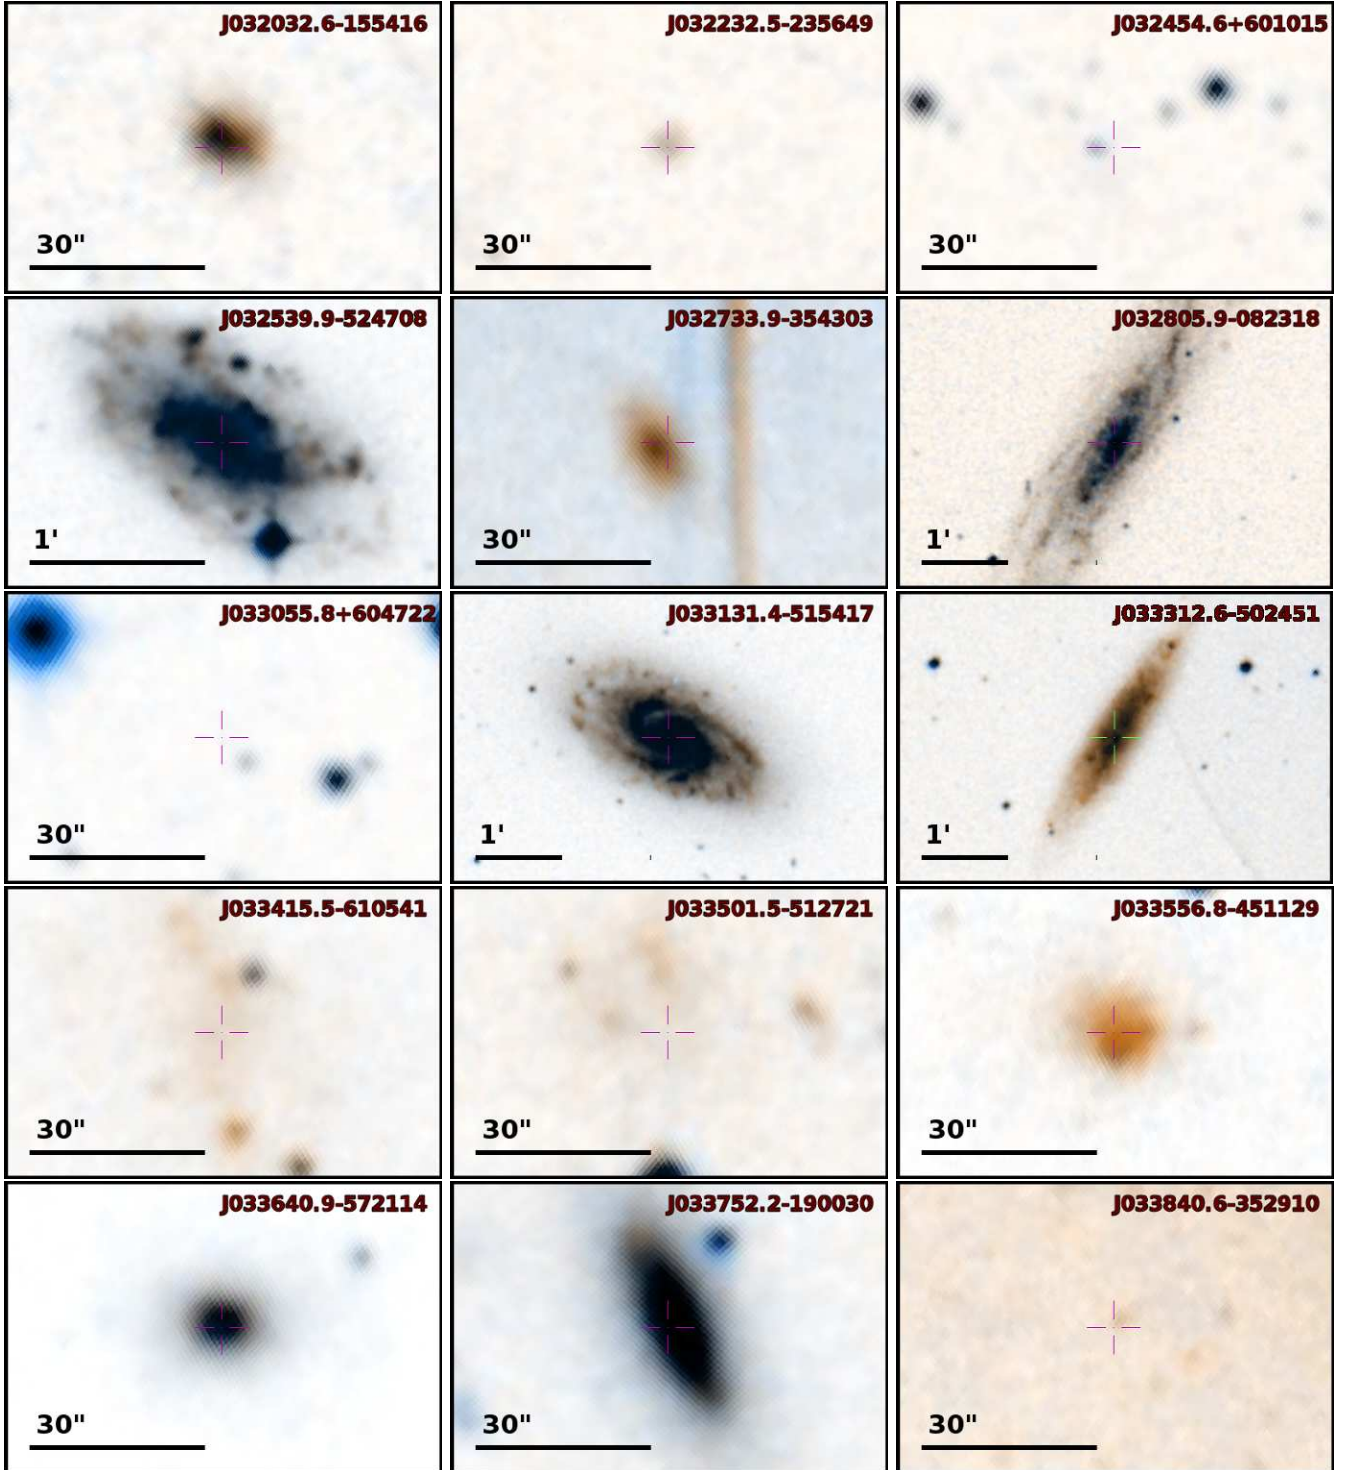

Figure A35. Nearby Void inner galaxies outside the SDSS footprint.



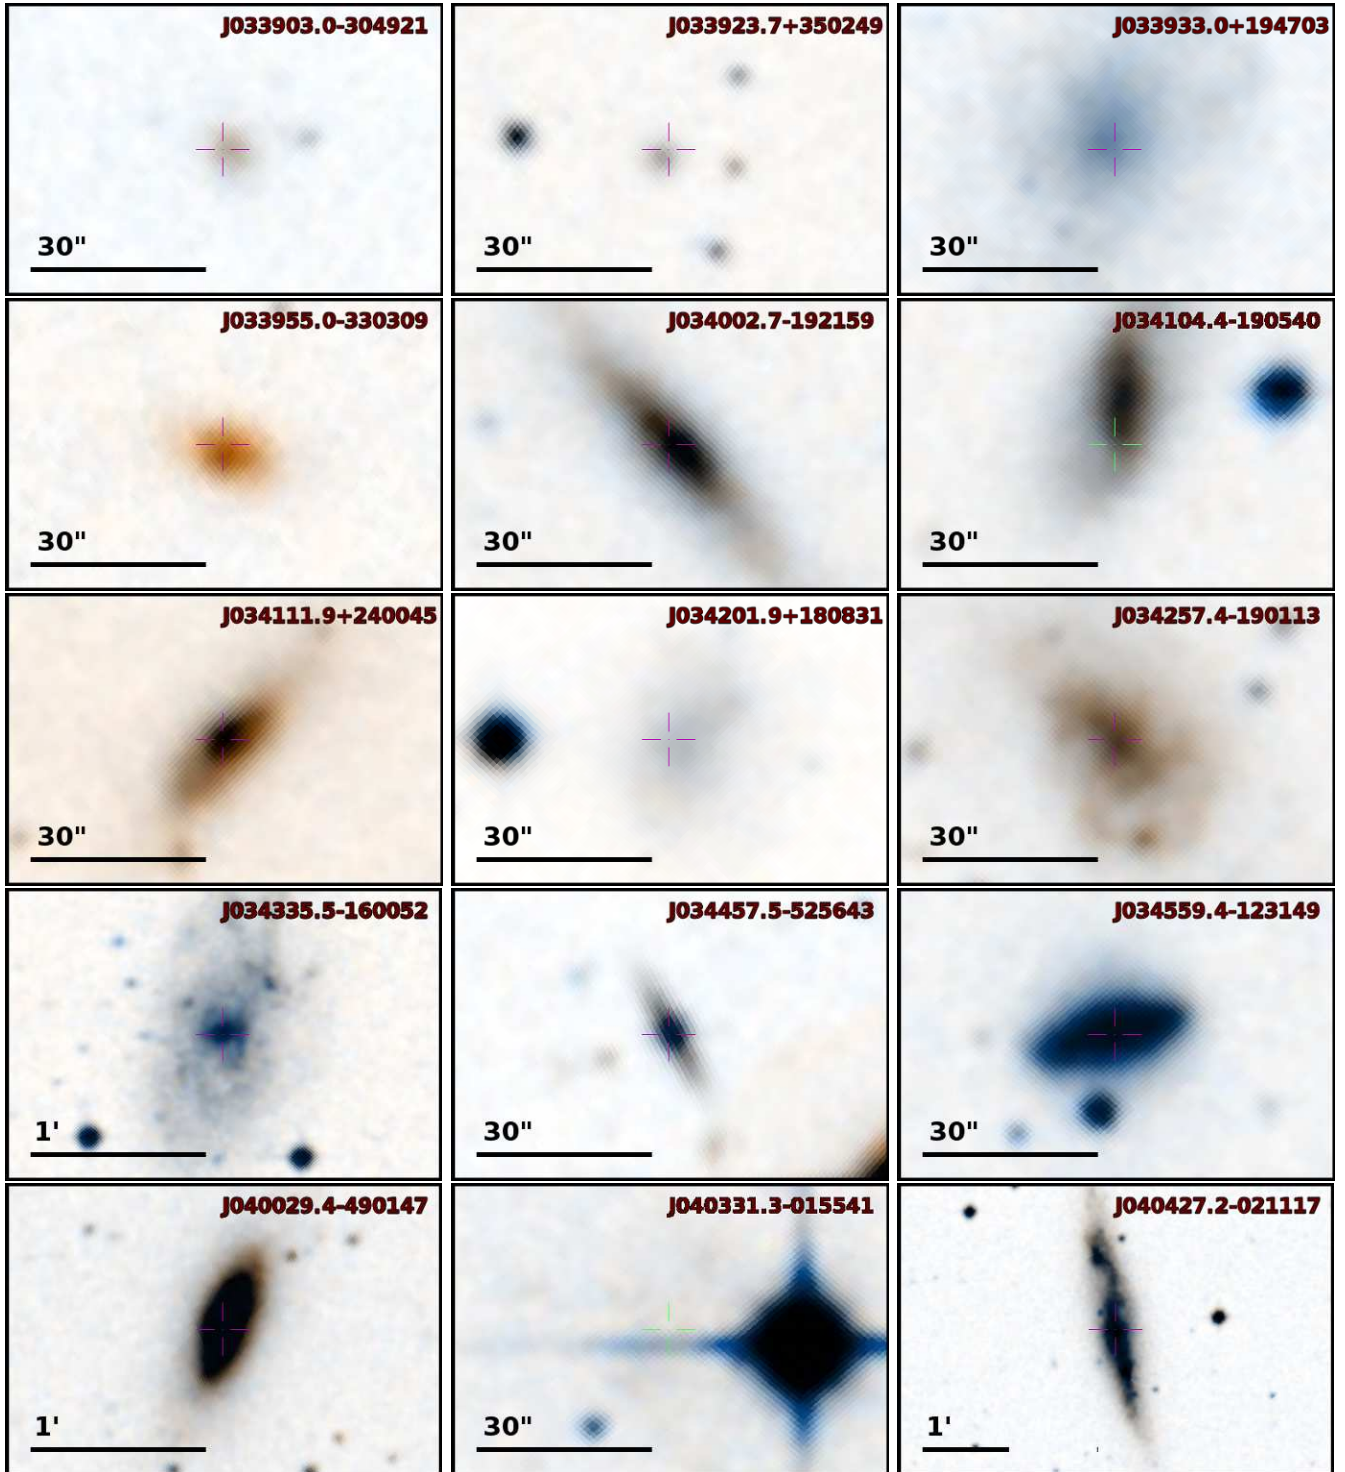

Figure A36. Nearby Void inner galaxies outside the SDSS footprint.



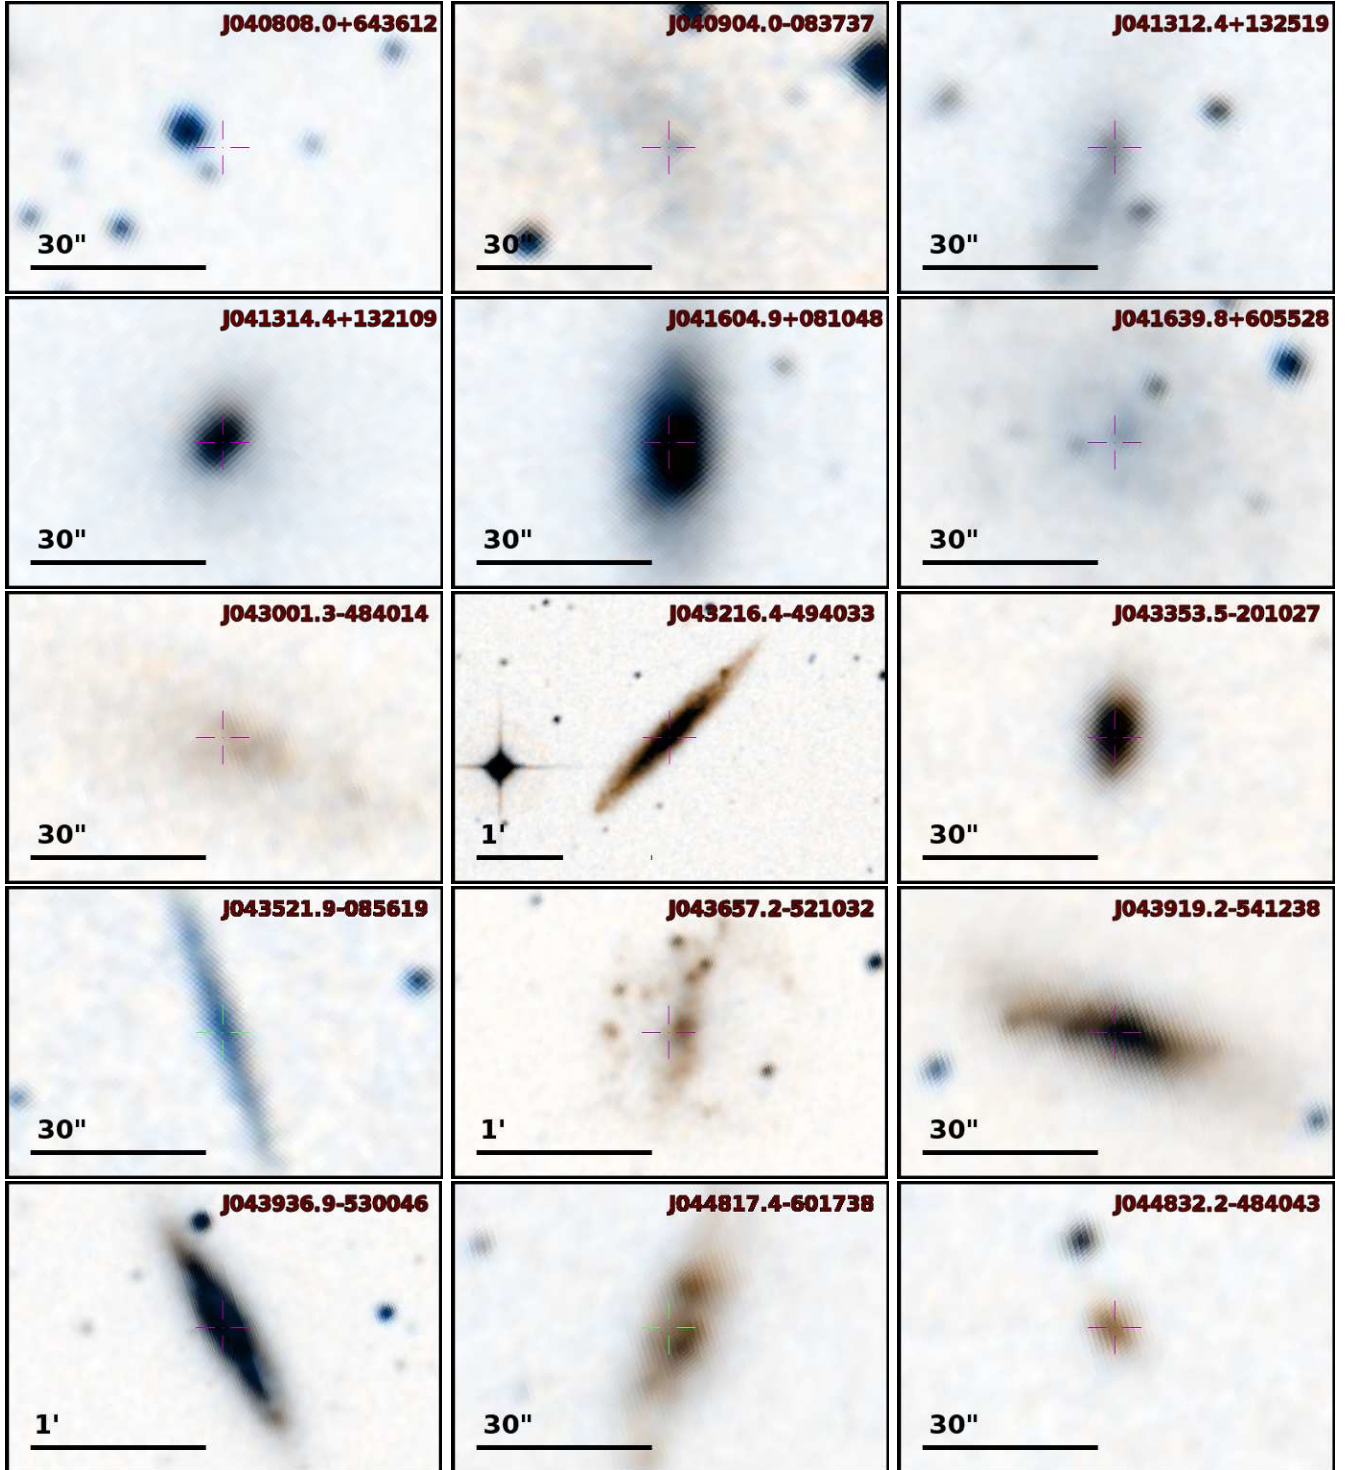

Figure A37. Nearby Void inner galaxies outside the SDSS footprint.

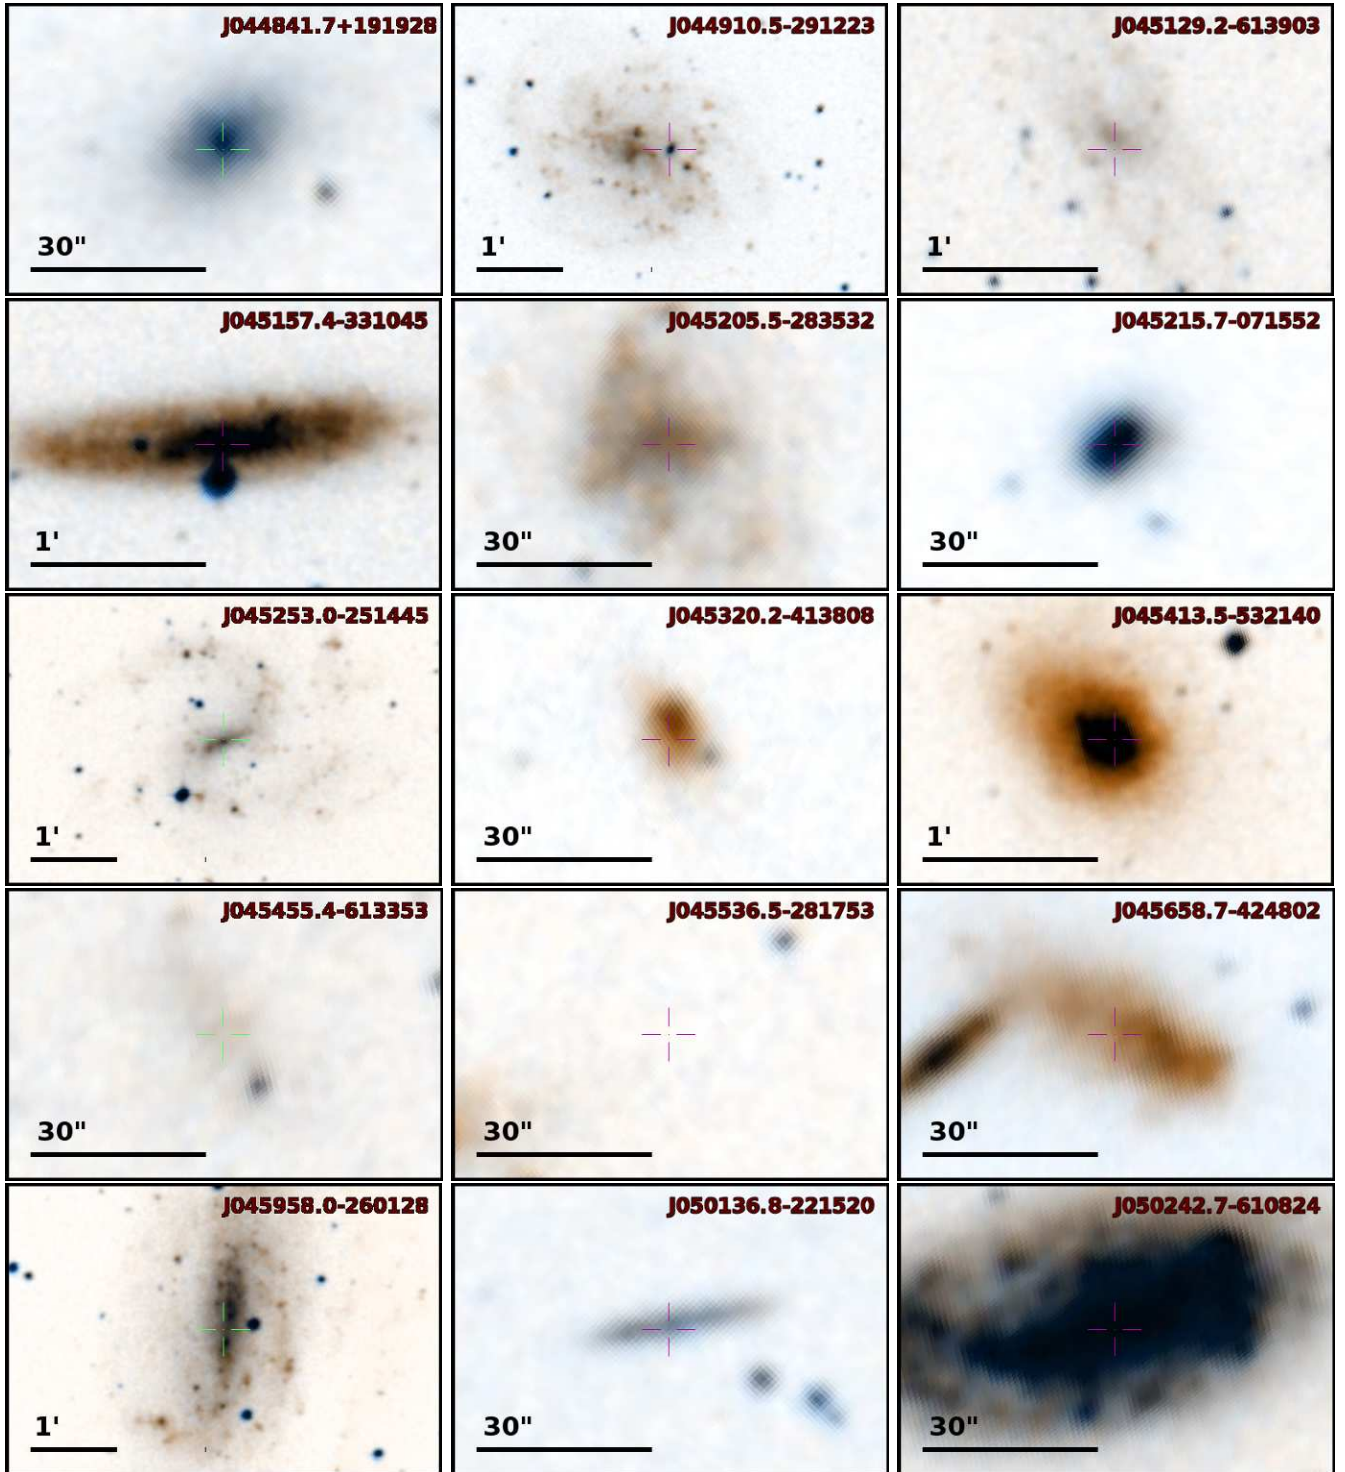

Figure A38. Nearby Void inner galaxies outside the SDSS footprint.

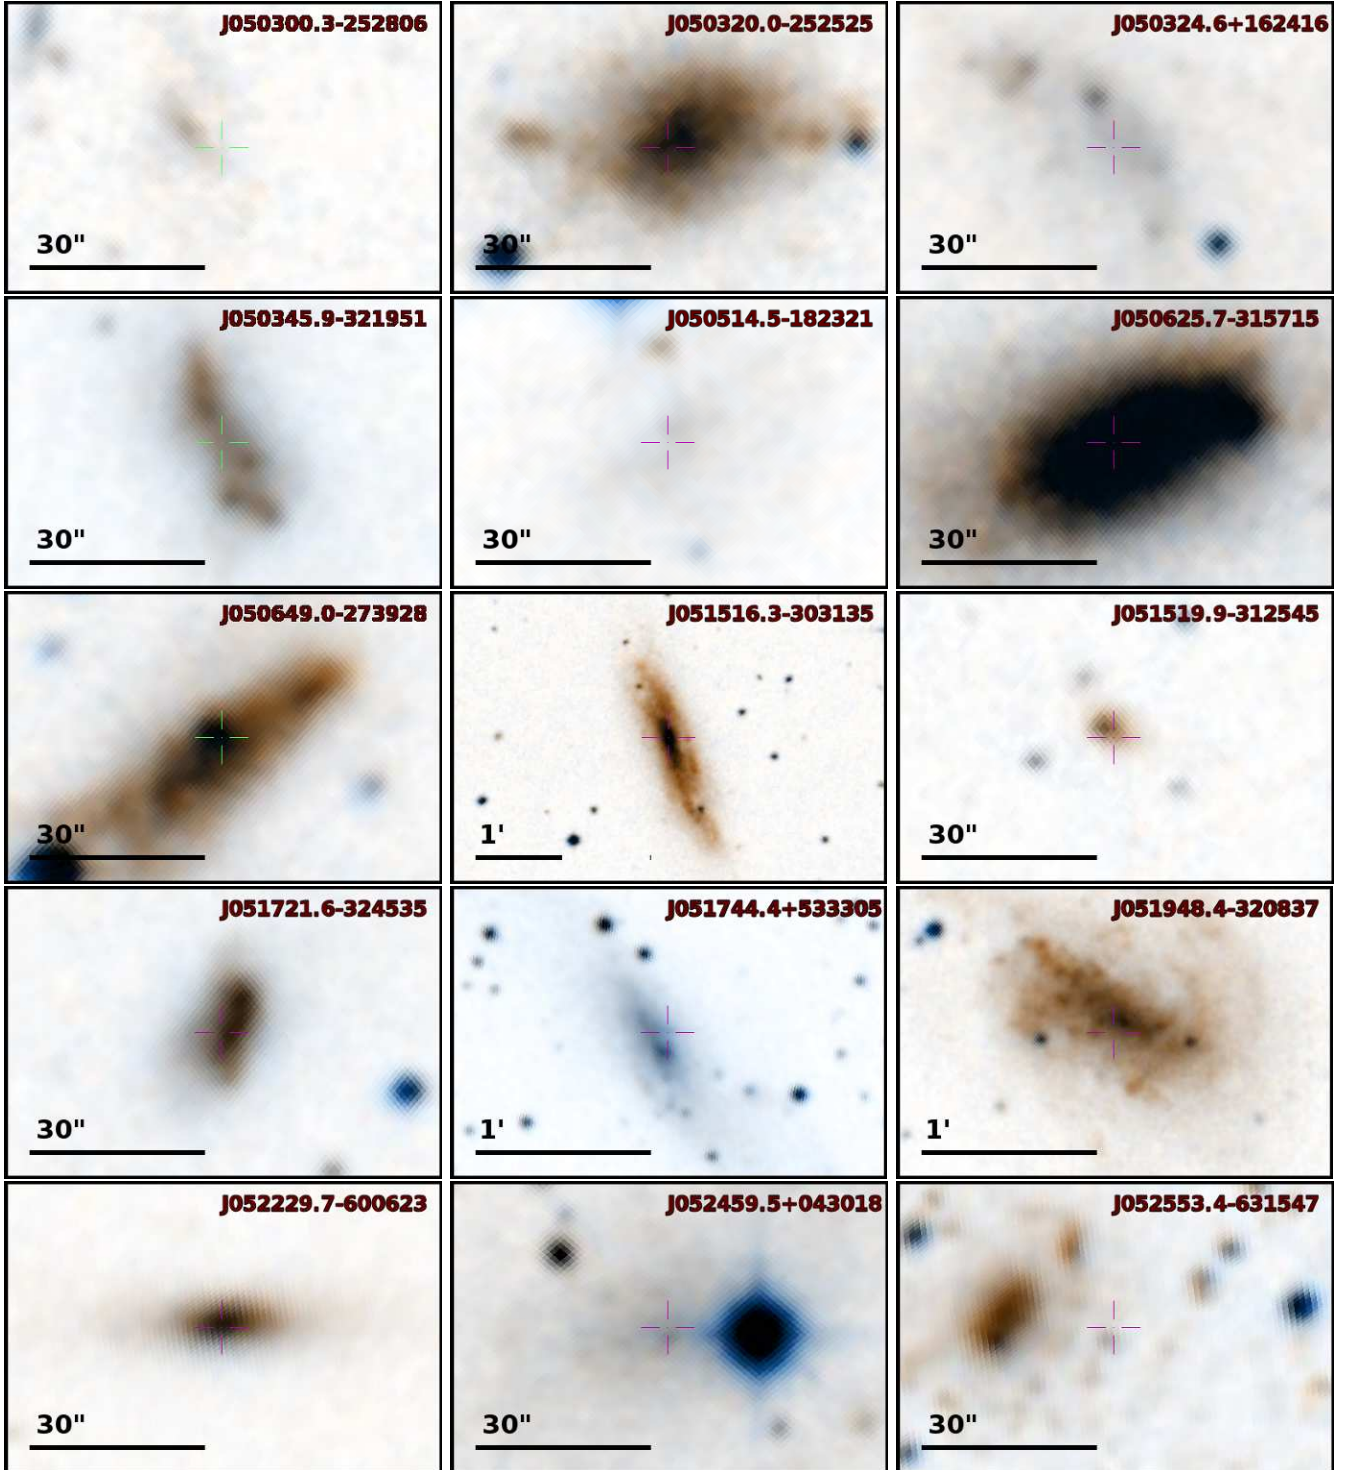

Figure A39. Nearby Void inner galaxies outside the SDSS footprint.



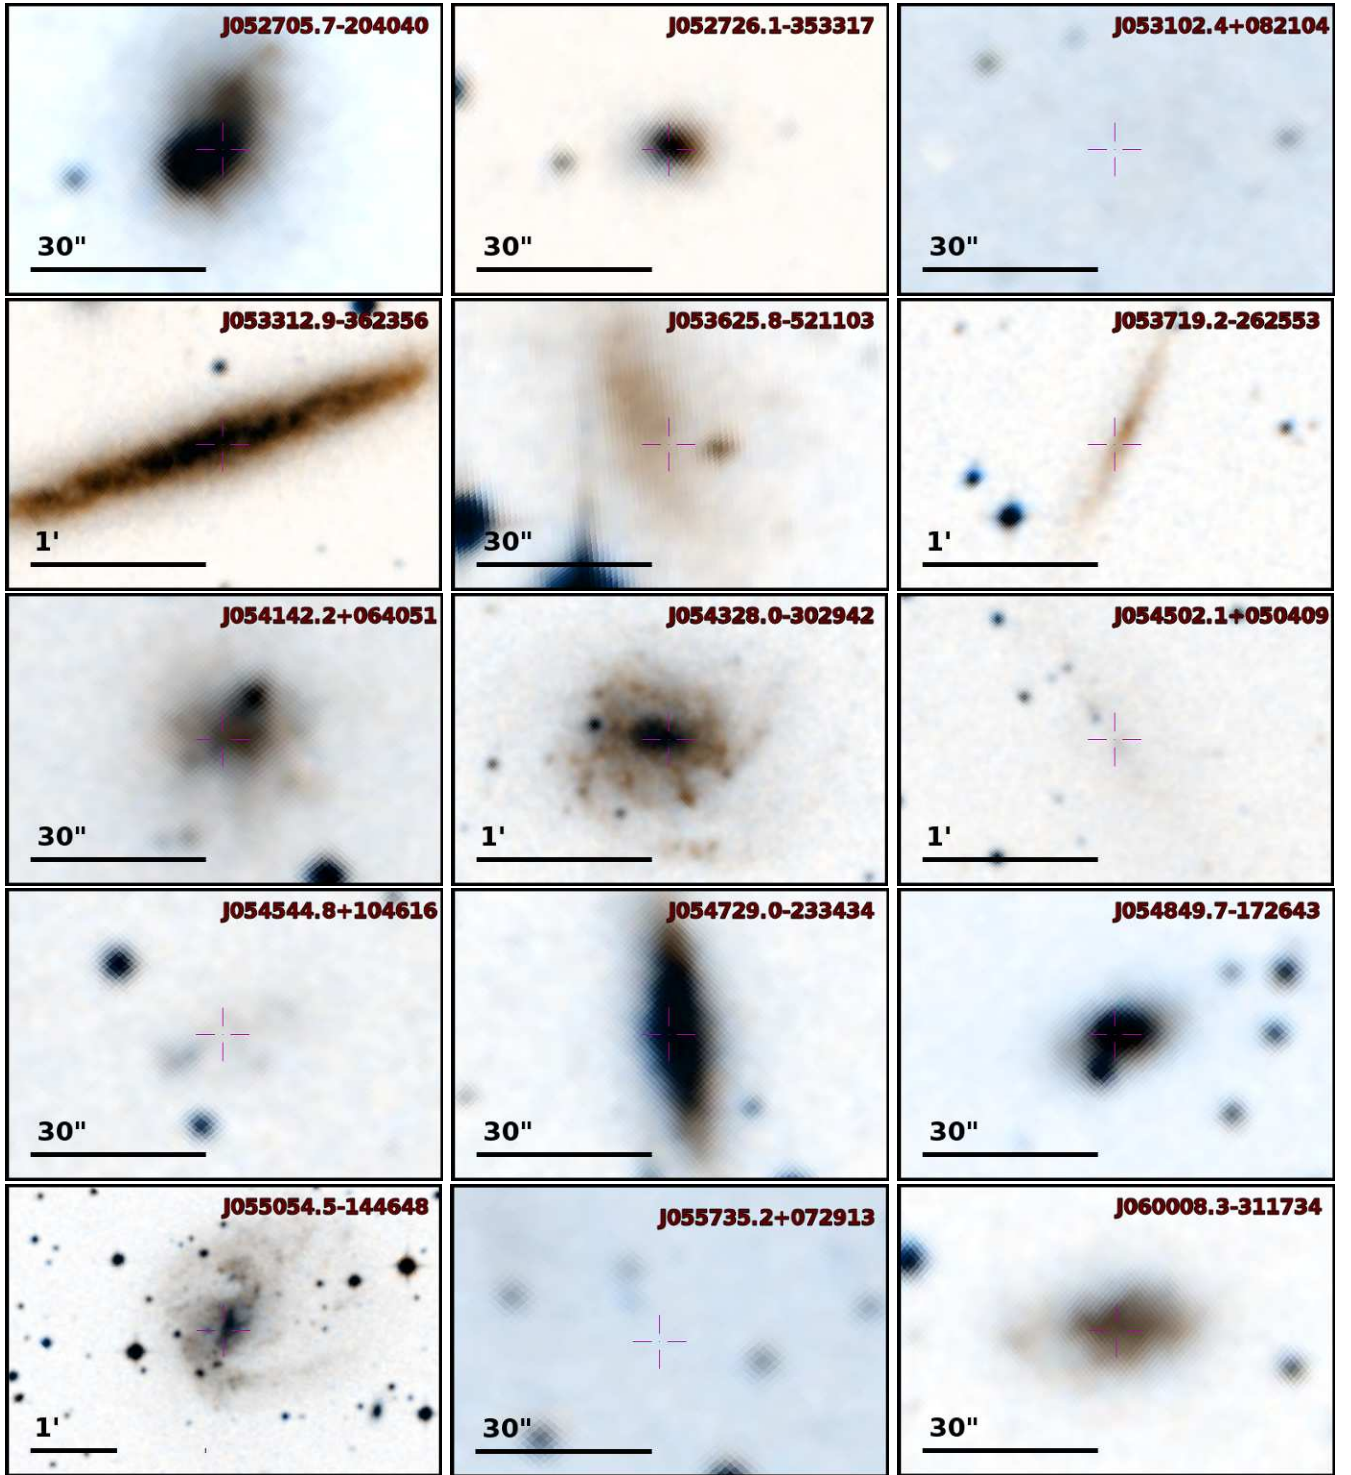

Figure A40. Nearby Void inner galaxies outside the SDSS footprint.

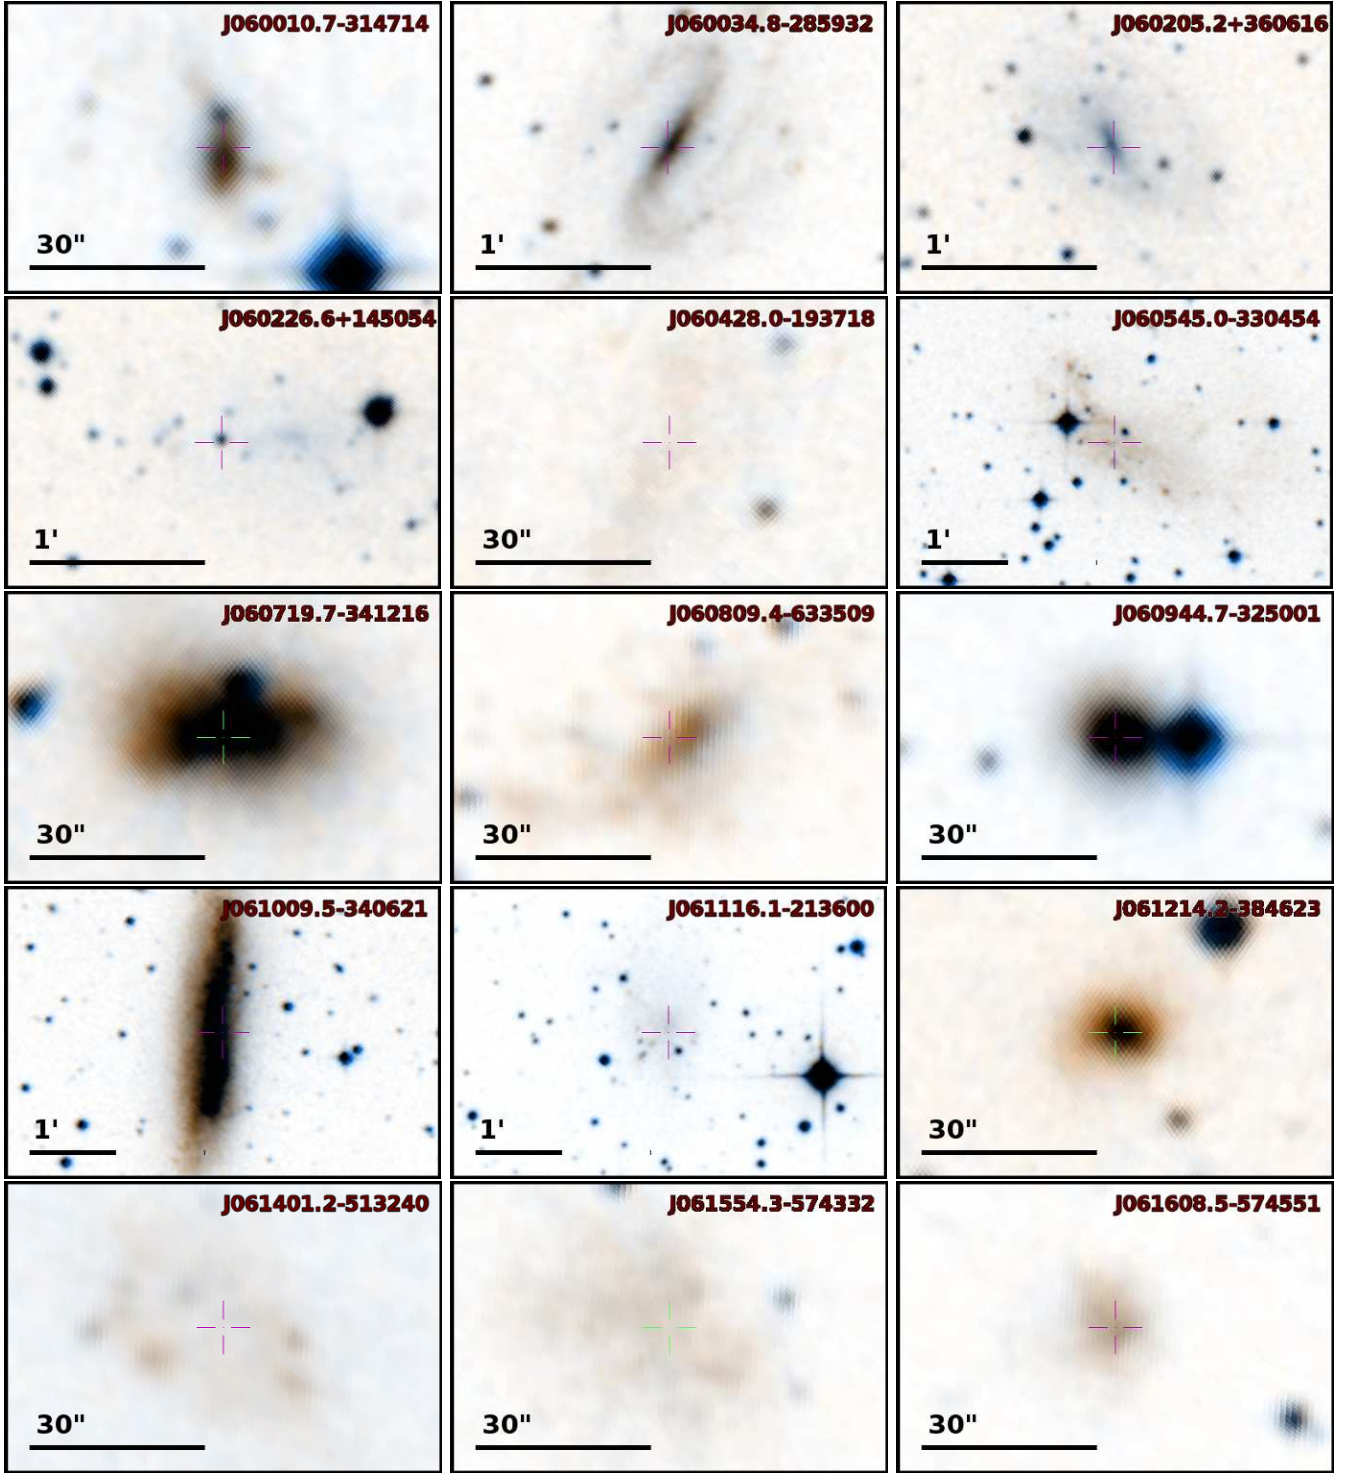

Figure A41. Nearby Void inner galaxies outside the SDSS footprint.

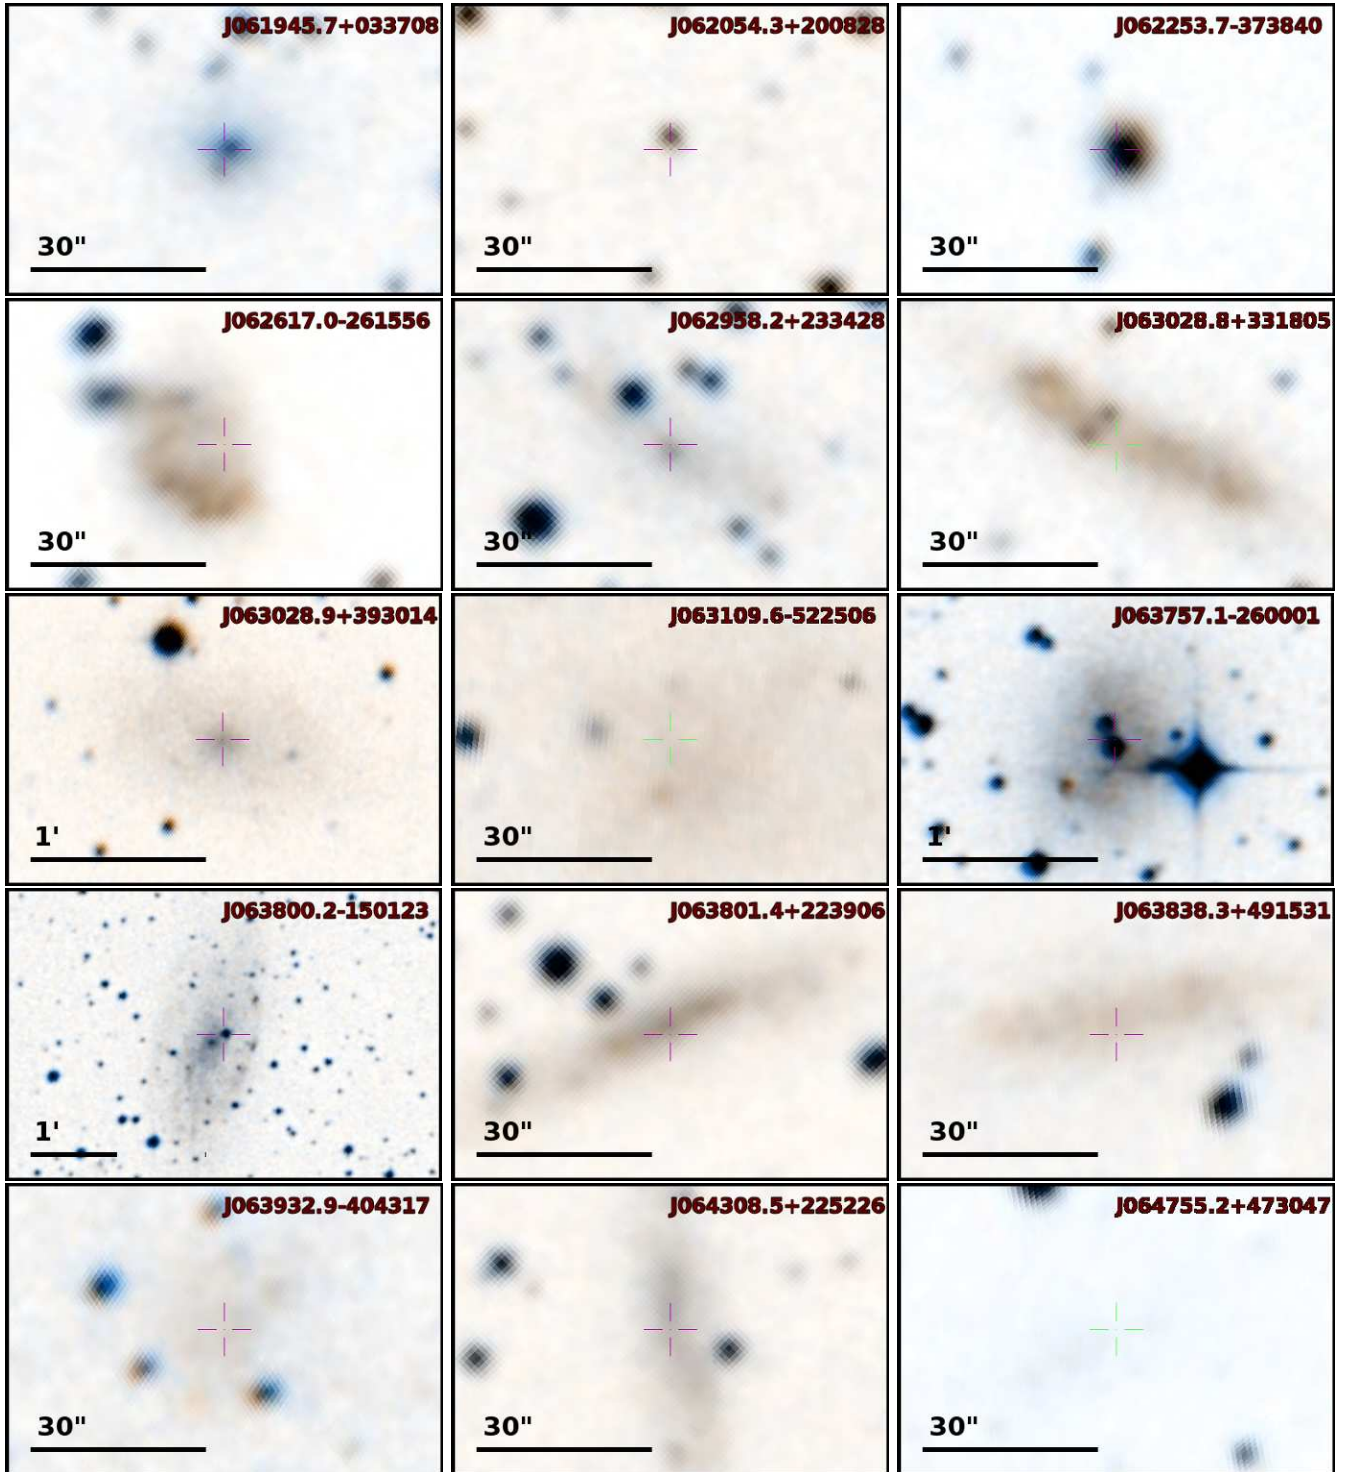

Figure A42. Nearby Void inner galaxies outside the SDSS footprint.



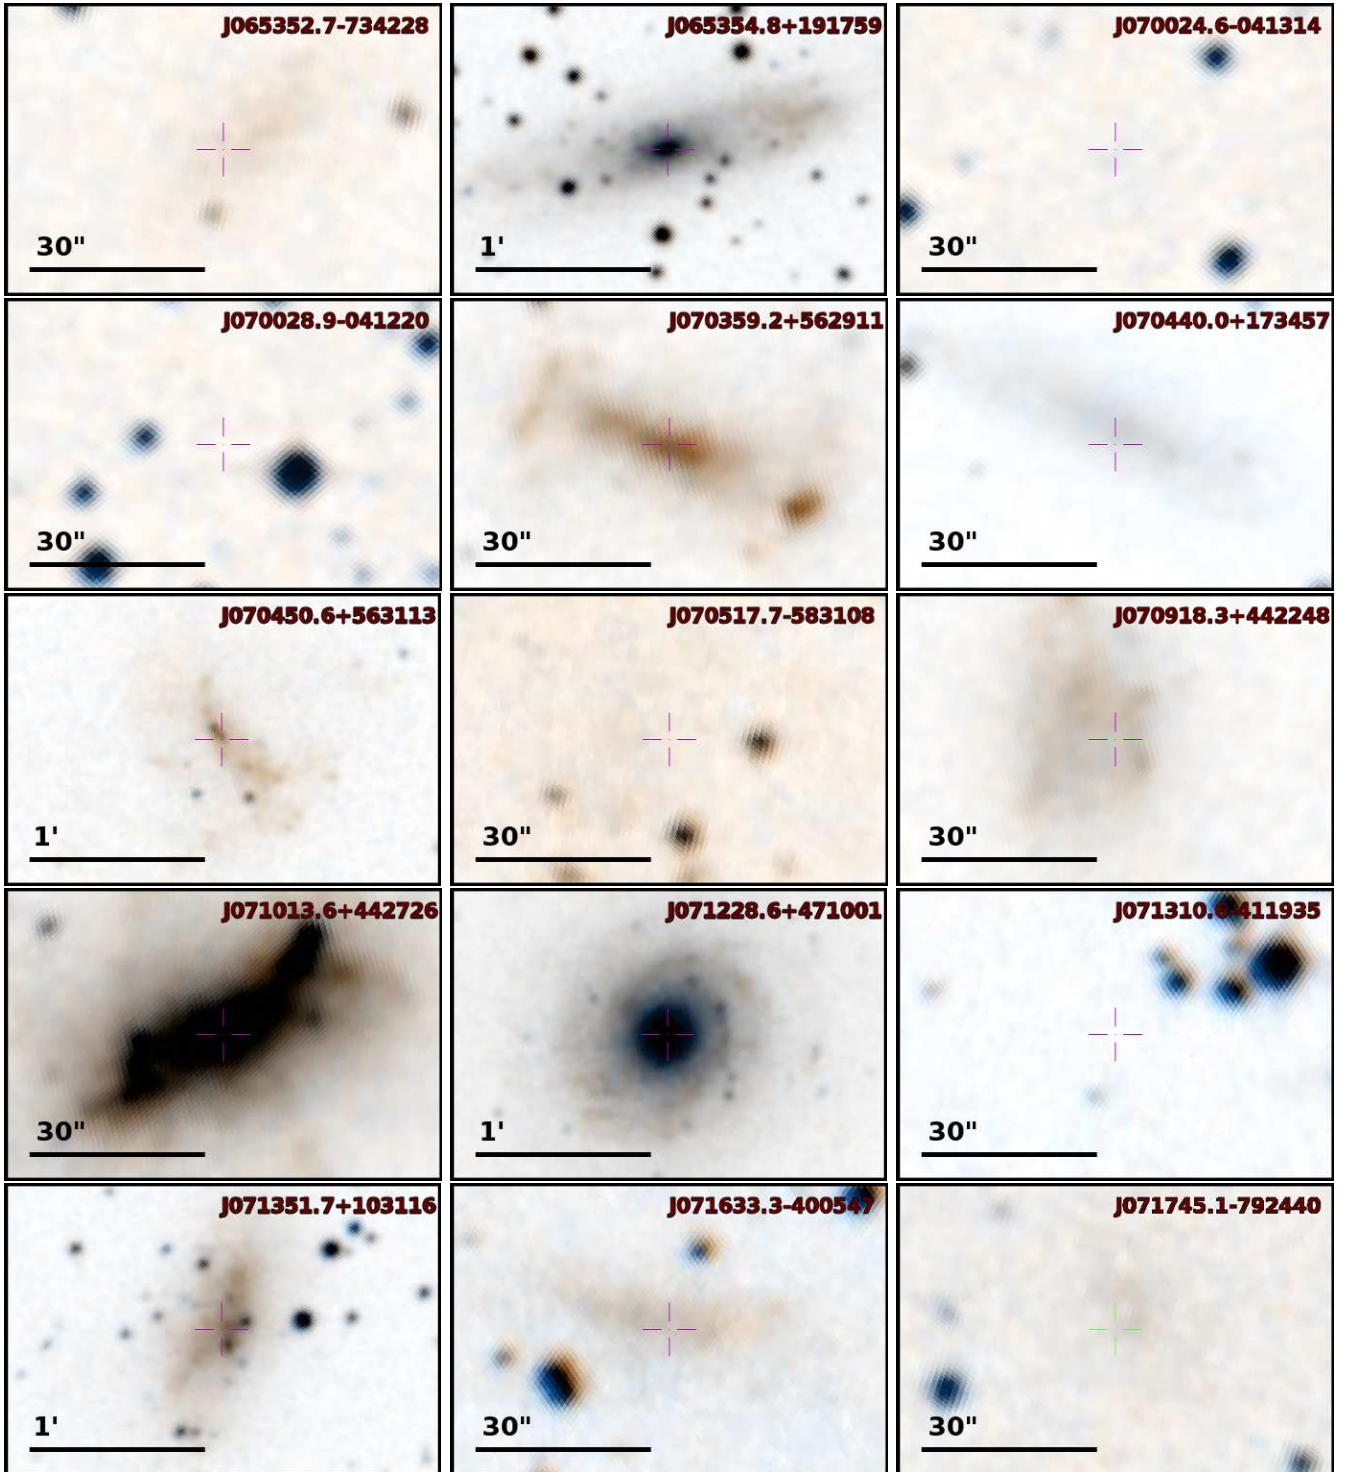

Figure A43. Nearby Void inner galaxies outside the SDSS footprint.



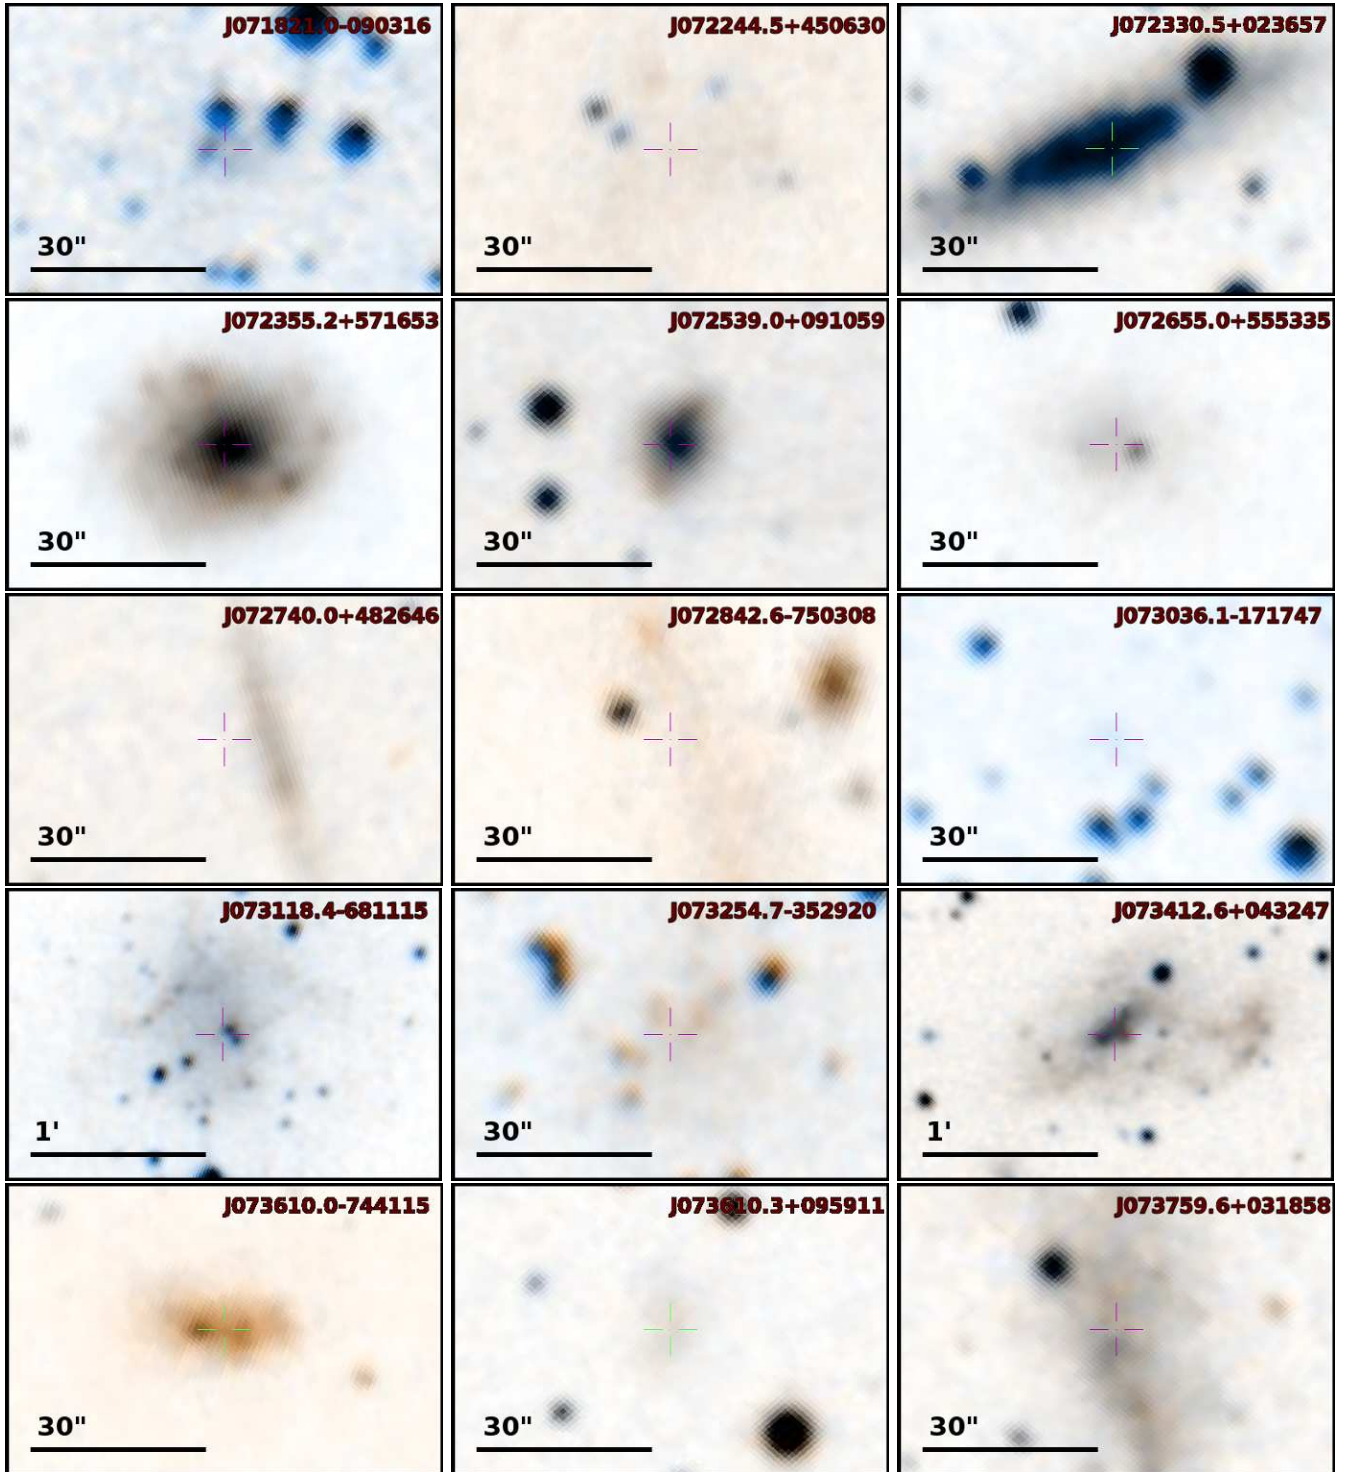

Figure A44. Nearby Void inner galaxies outside the SDSS footprint.

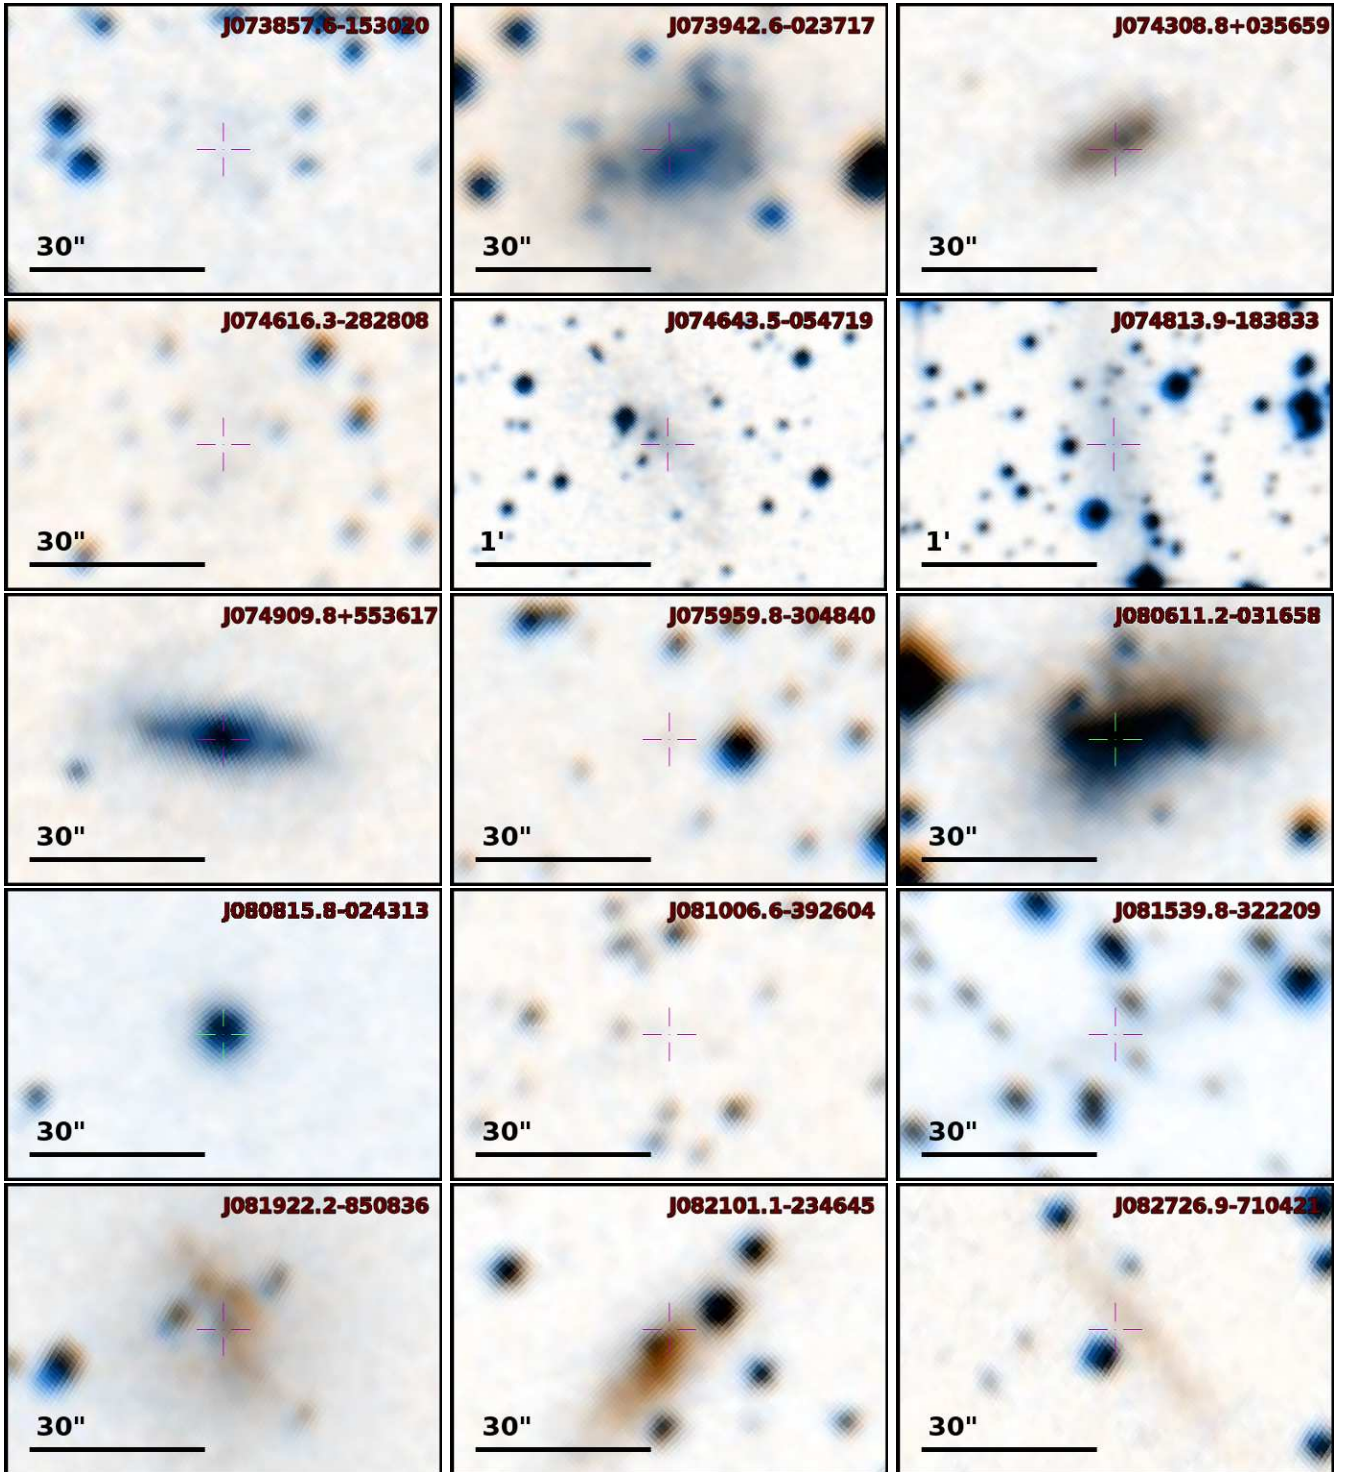

Figure A45. Nearby Void inner galaxies outside the SDSS footprint.



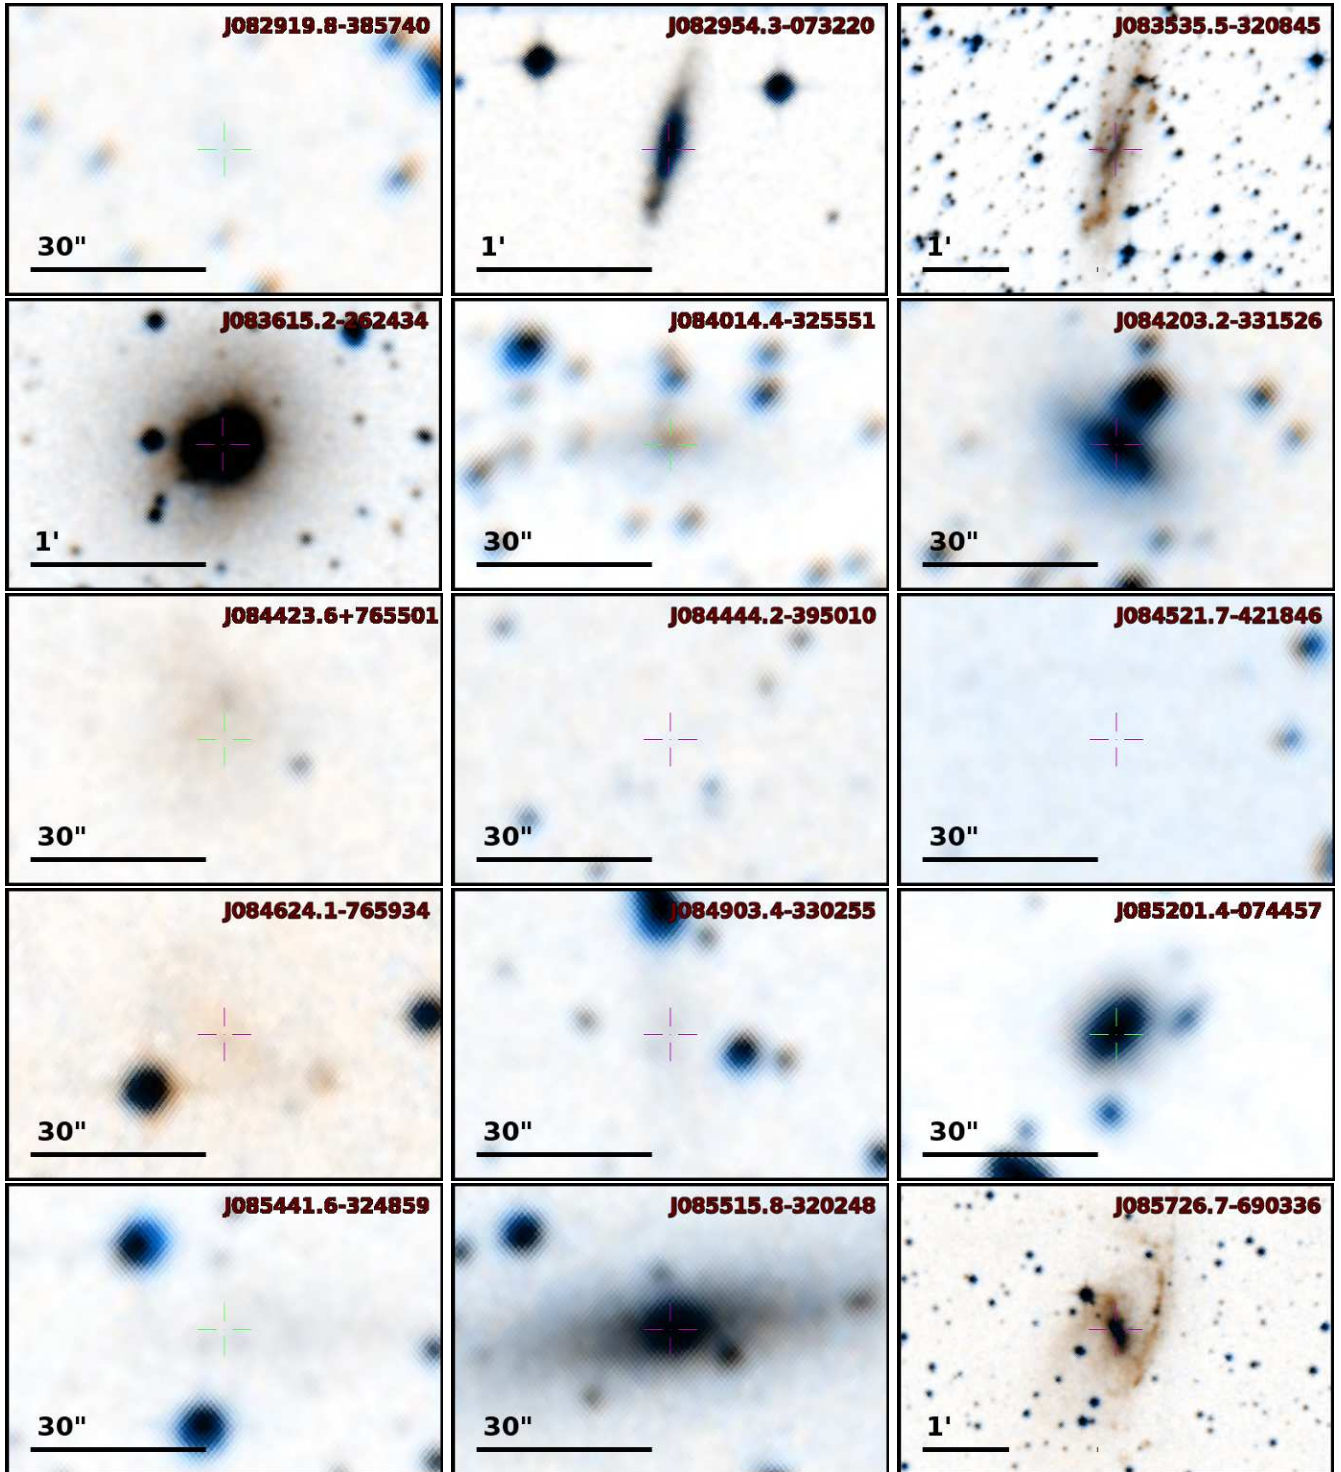

Figure A46. Nearby Void inner galaxies outside the SDSS footprint.

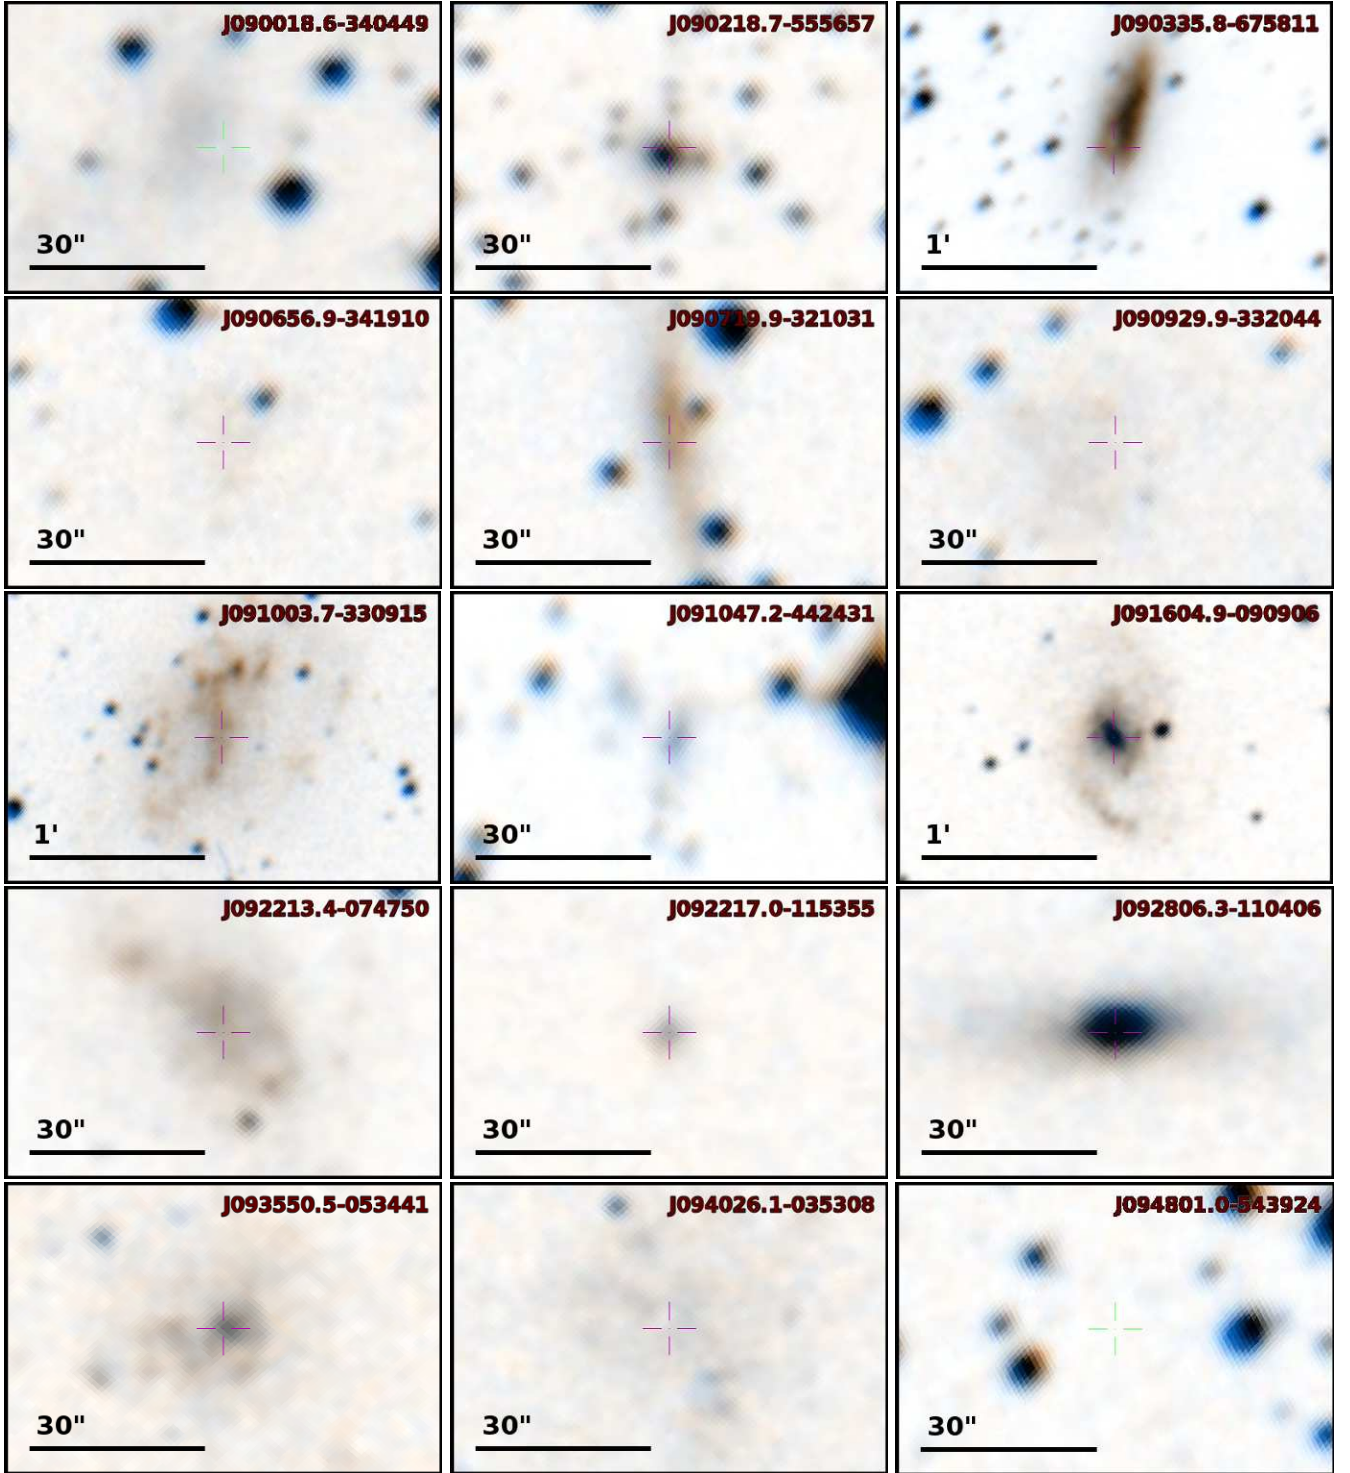

Figure A47. Nearby Void inner galaxies outside the SDSS footprint.



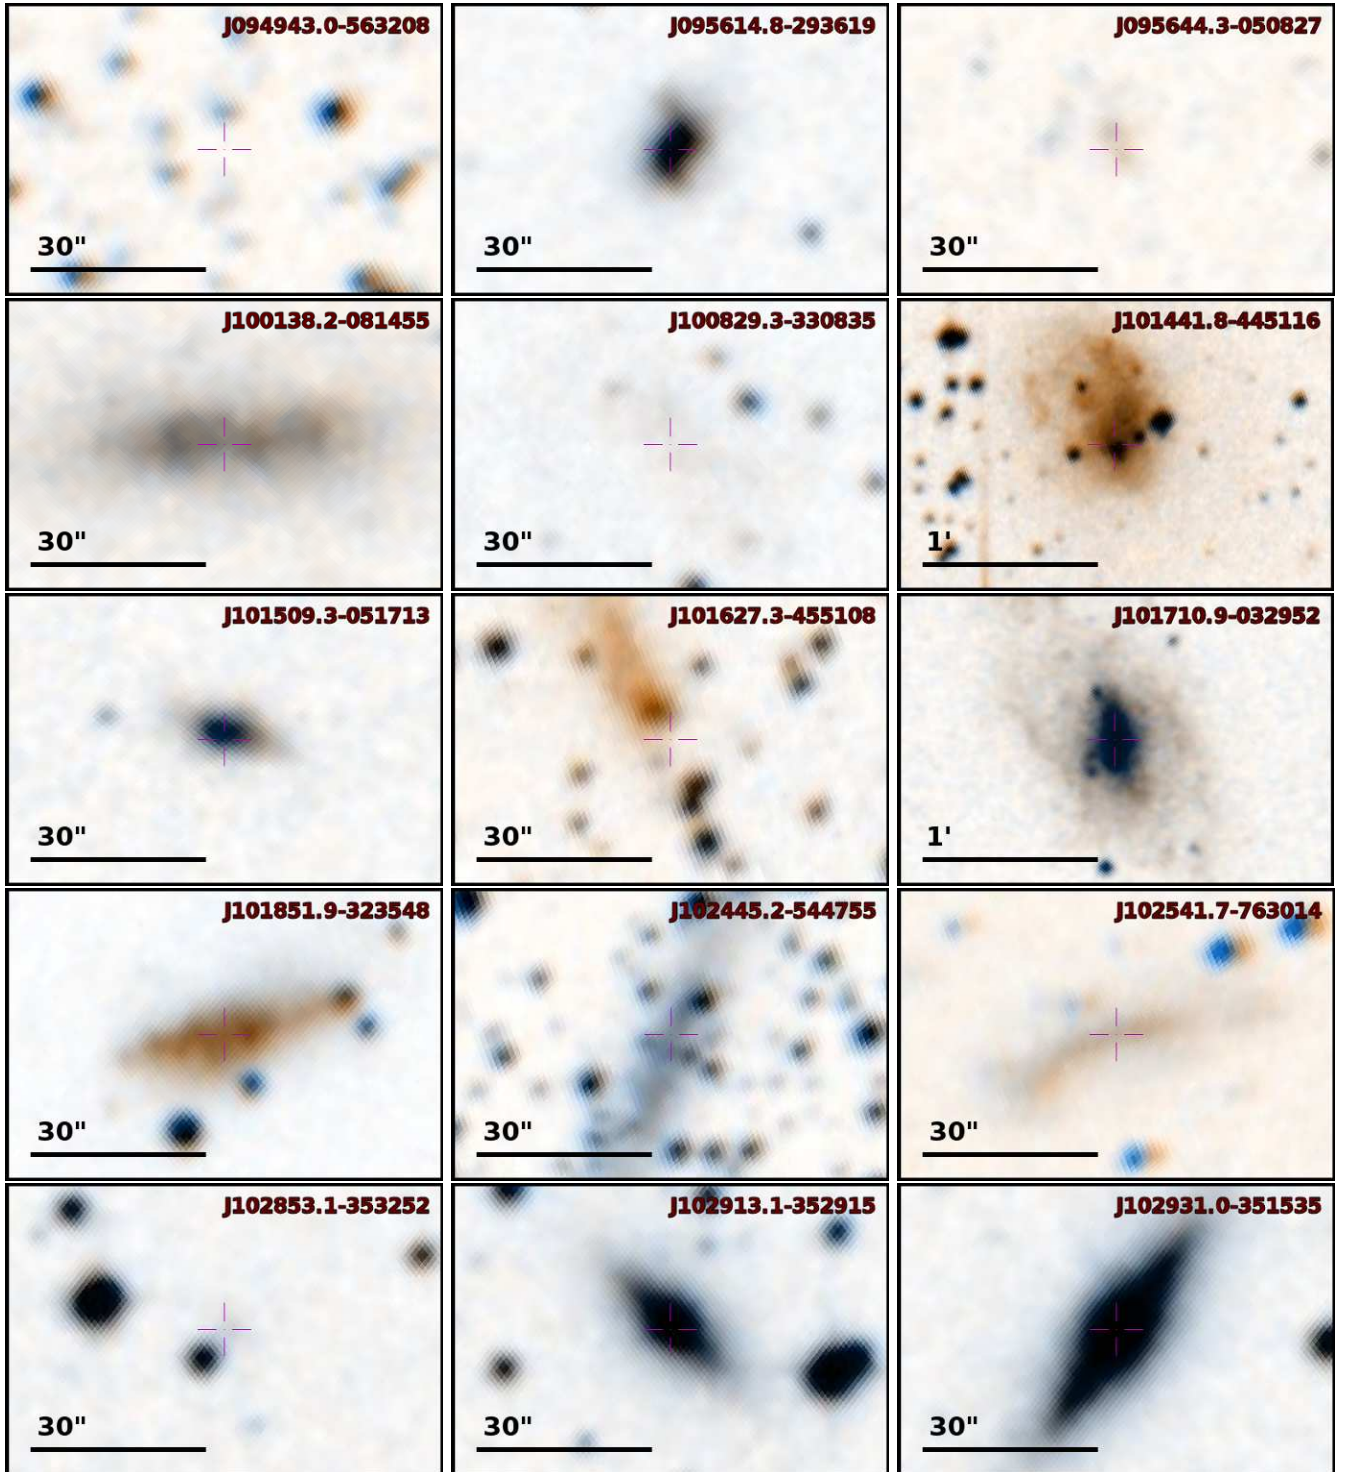

Figure A48. Nearby Void inner galaxies outside the SDSS footprint.



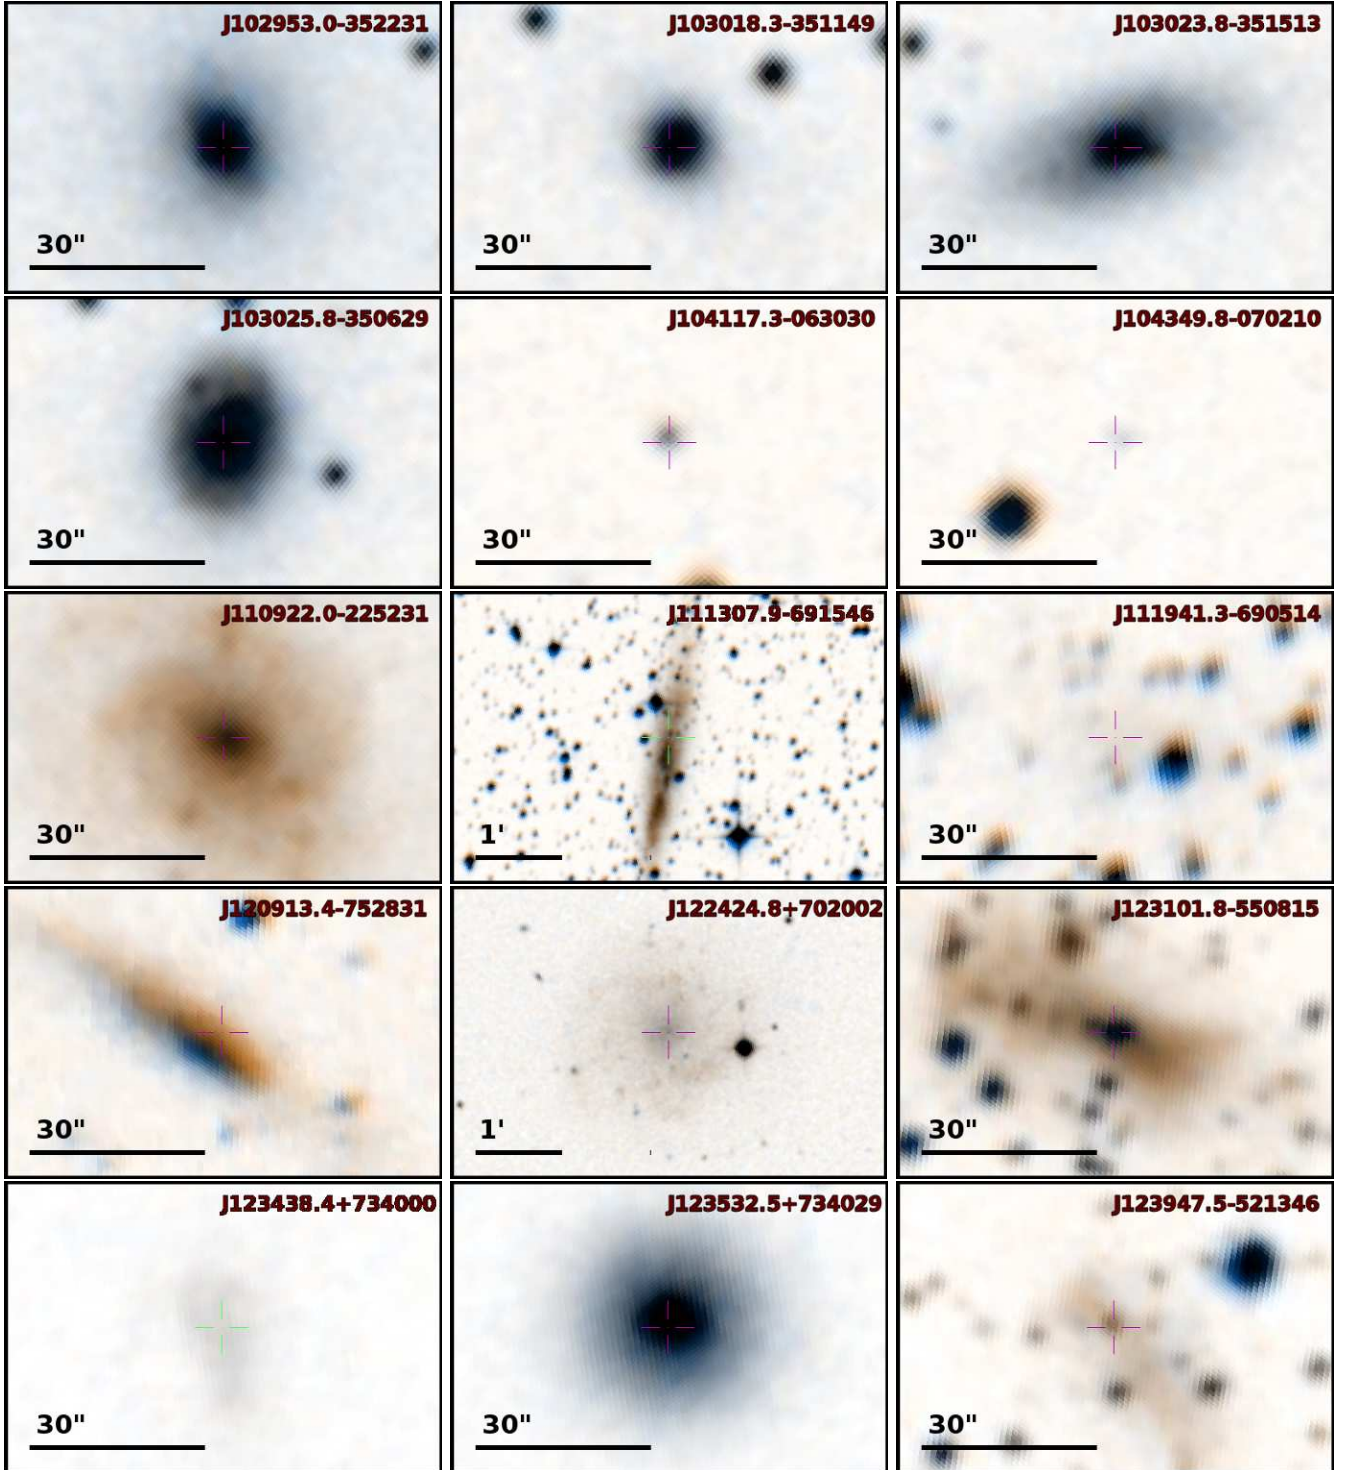

Figure A49. Nearby Void inner galaxies outside the SDSS footprint.

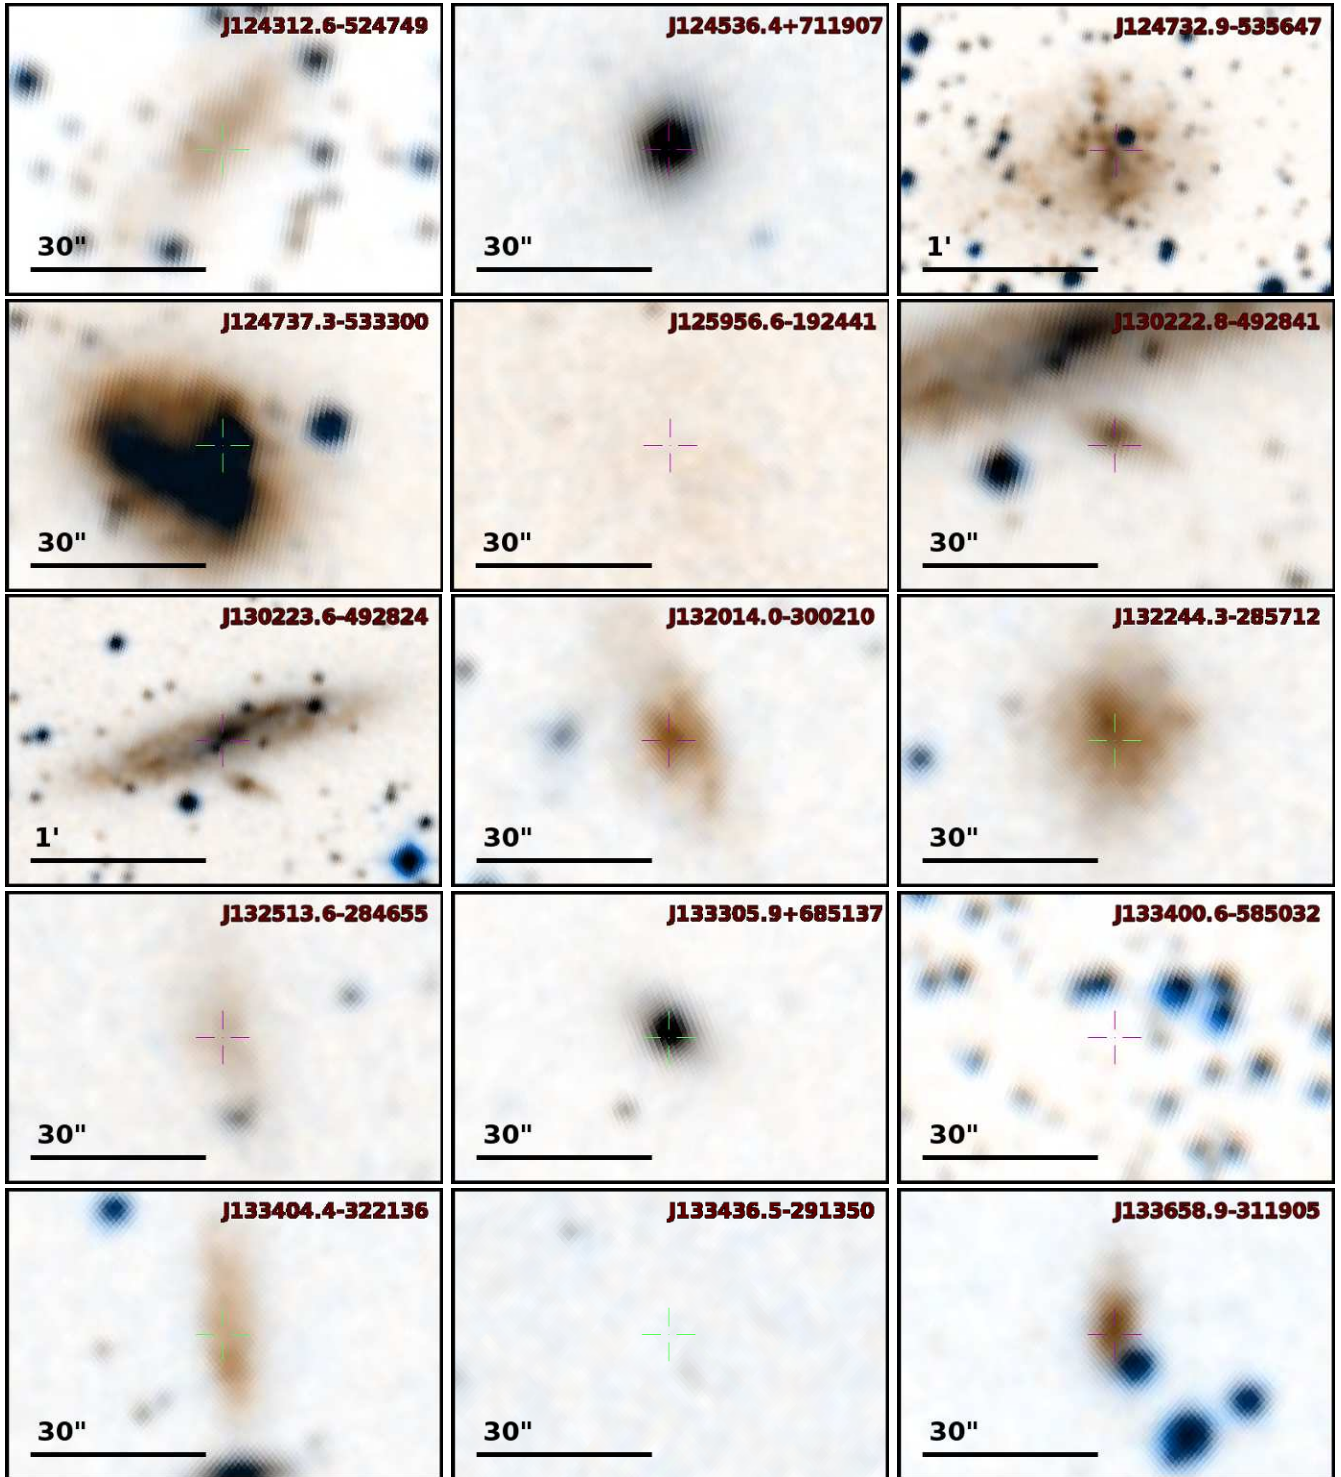

Figure A50. Nearby Void inner galaxies outside the SDSS footprint.

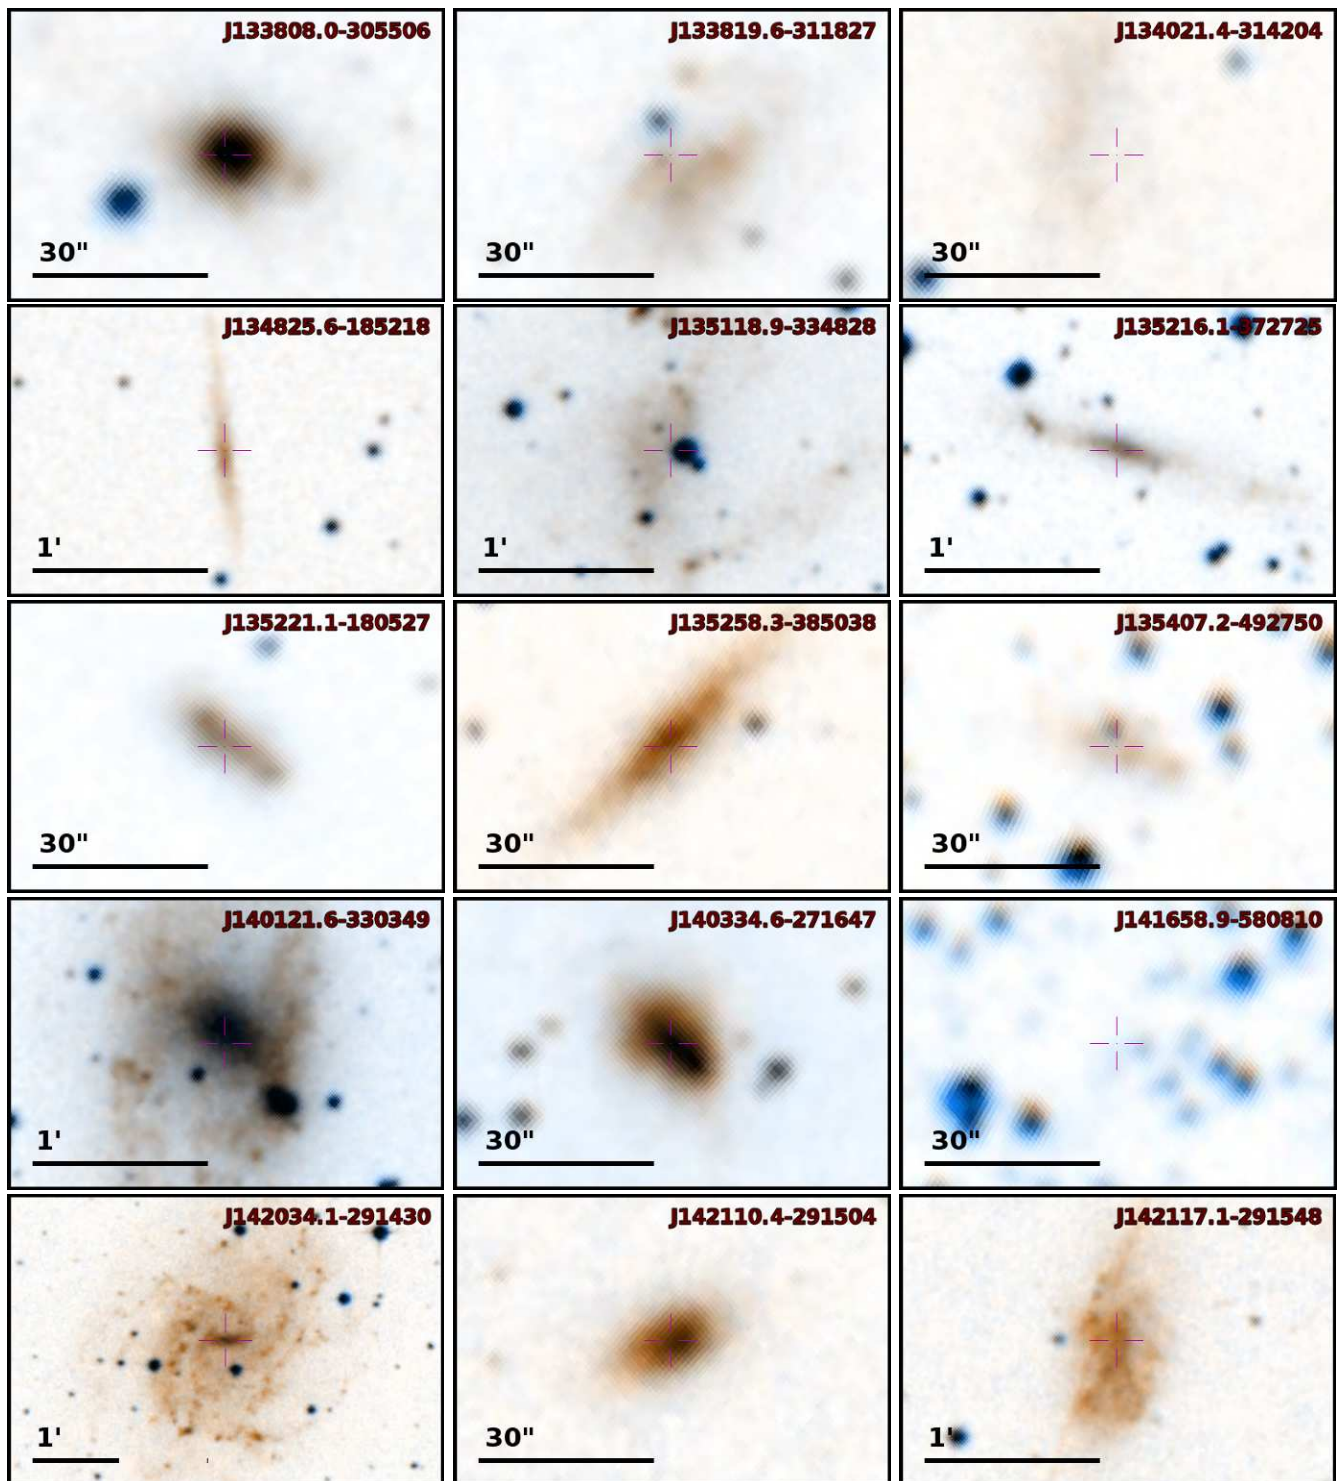

Figure A51. Nearby Void inner galaxies outside the SDSS footprint.



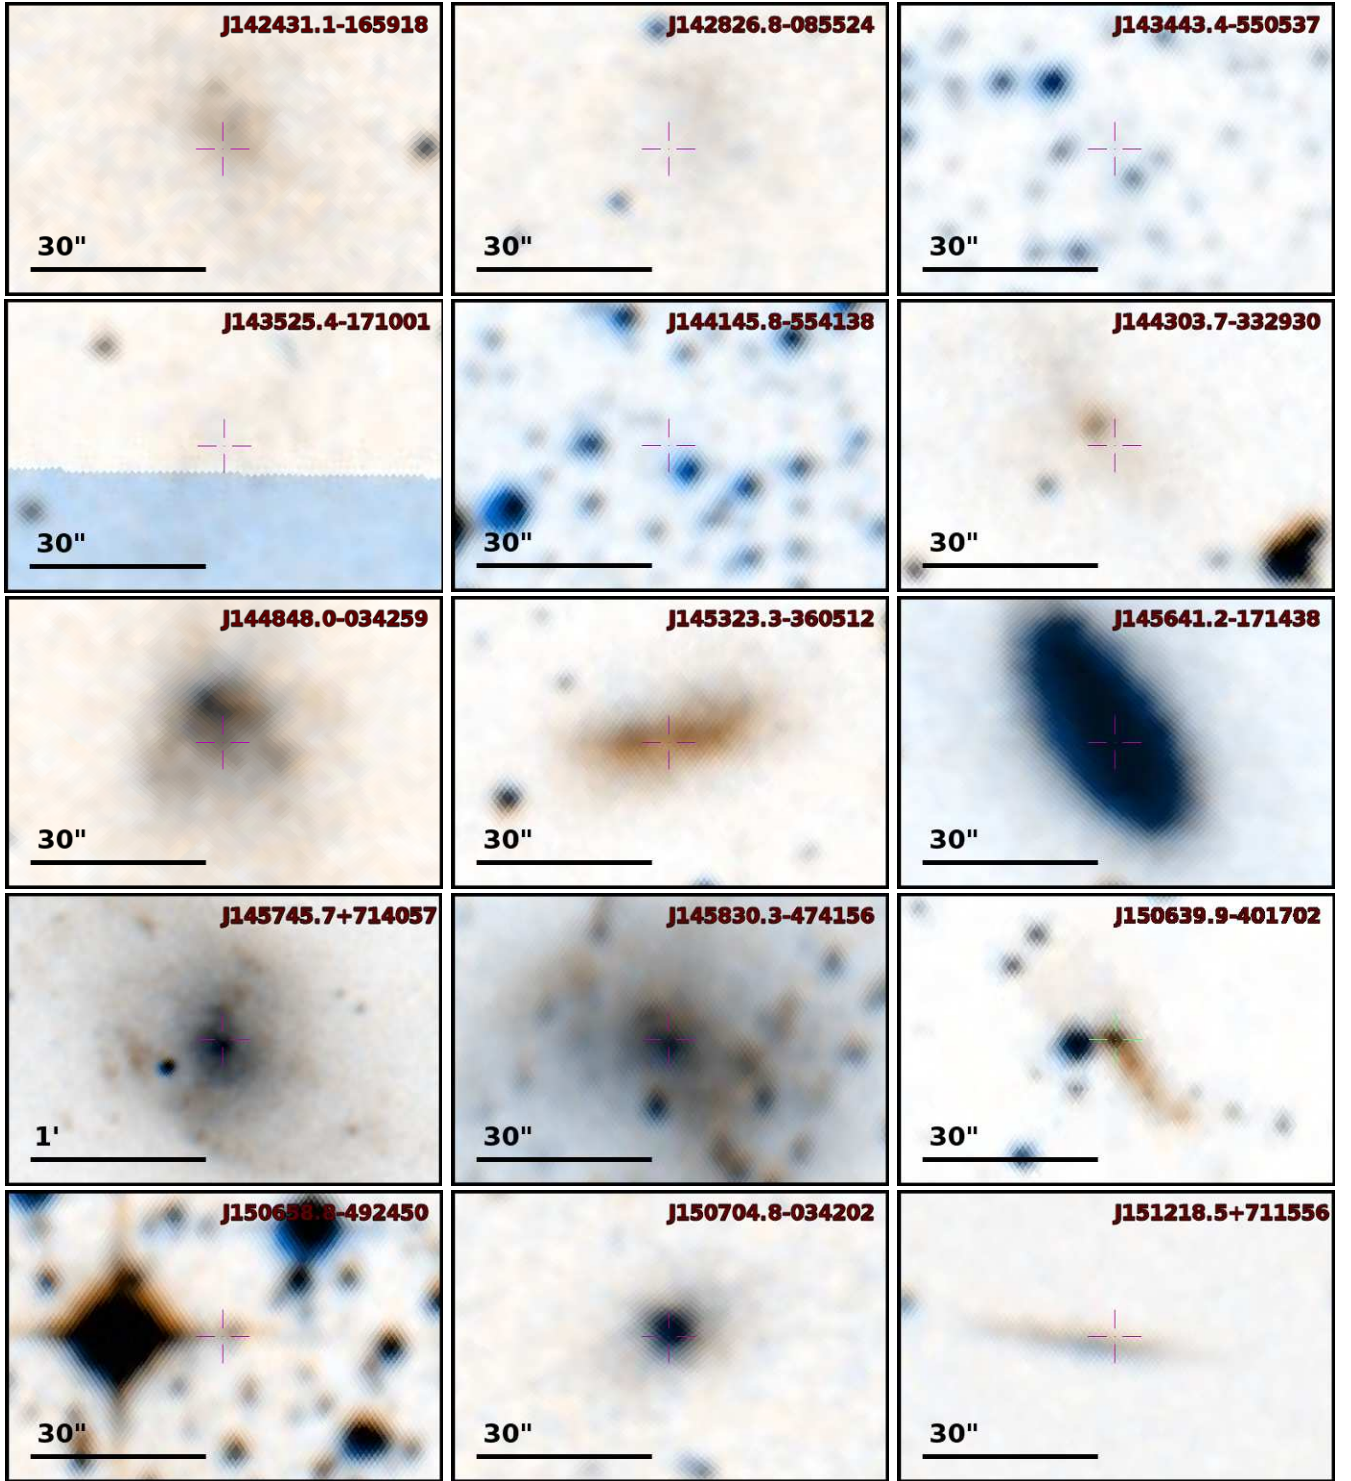

Figure A52. Nearby Void inner galaxies outside the SDSS footprint.

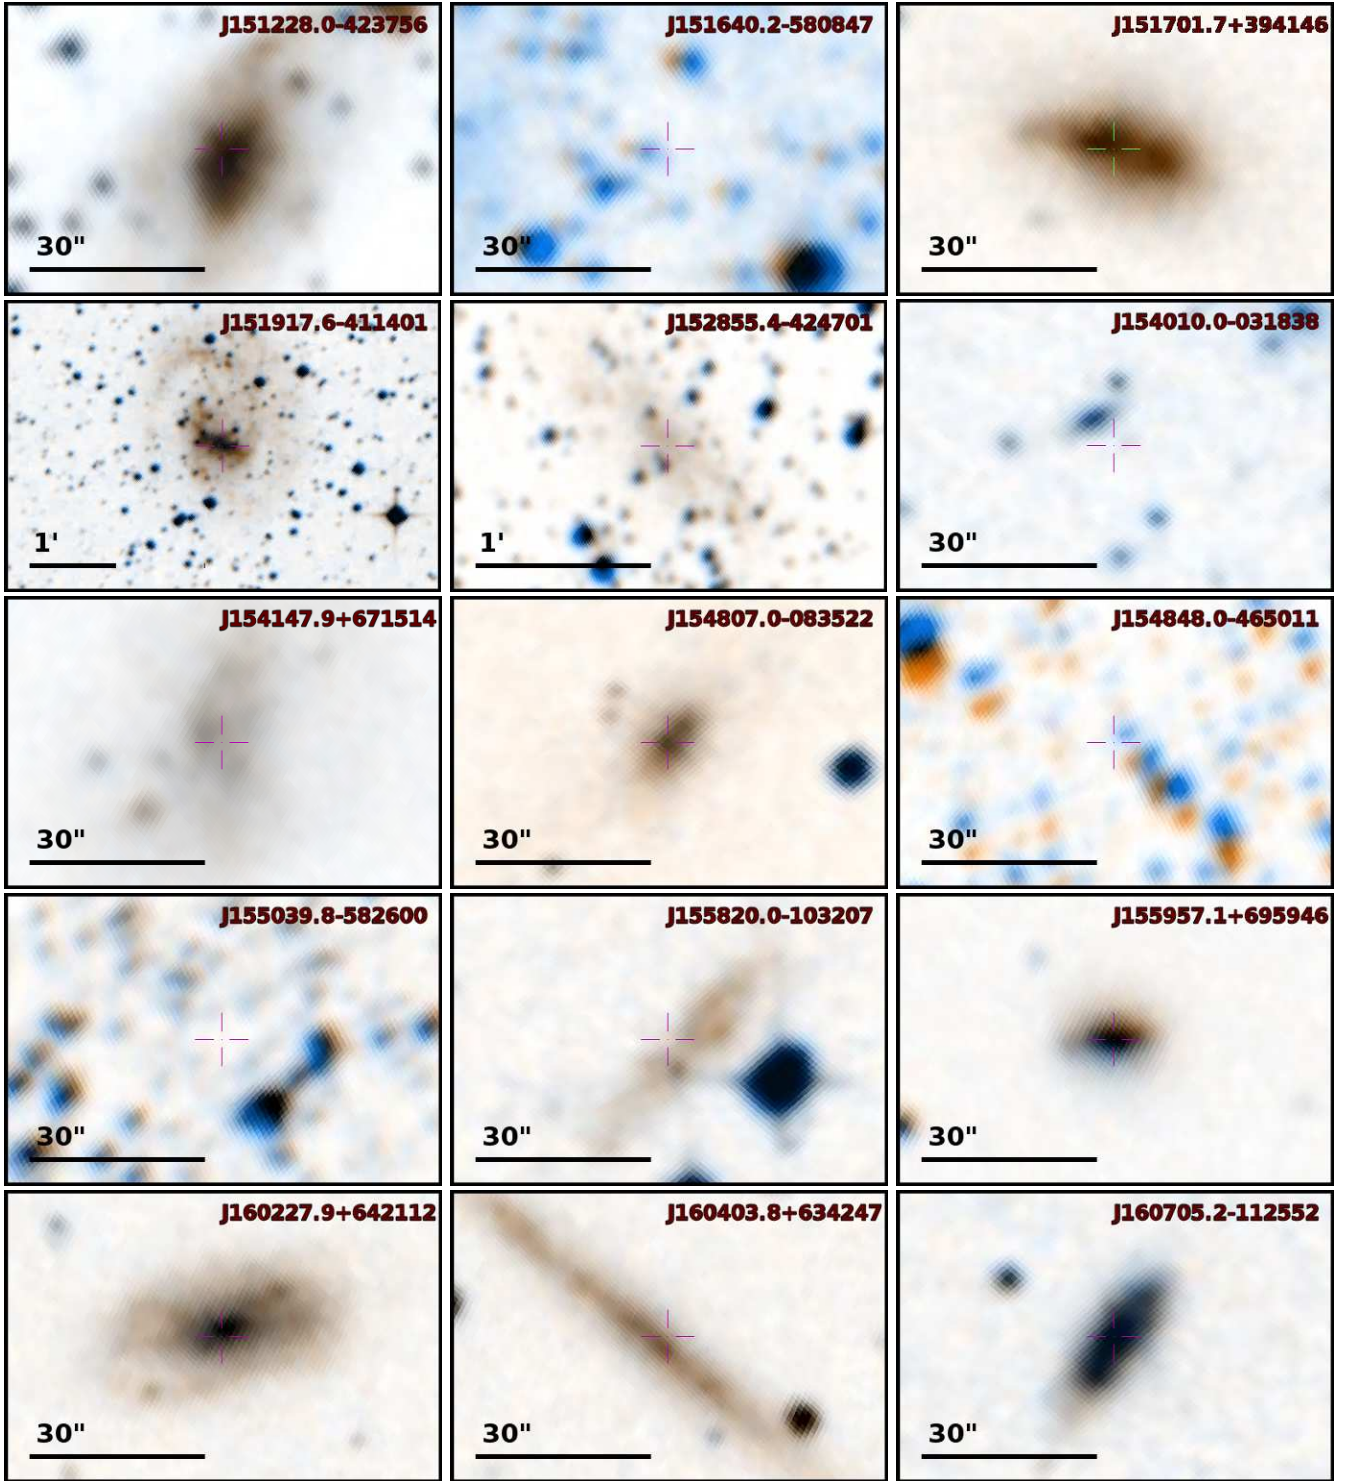

Figure A53. Nearby Void inner galaxies outside the SDSS footprint.



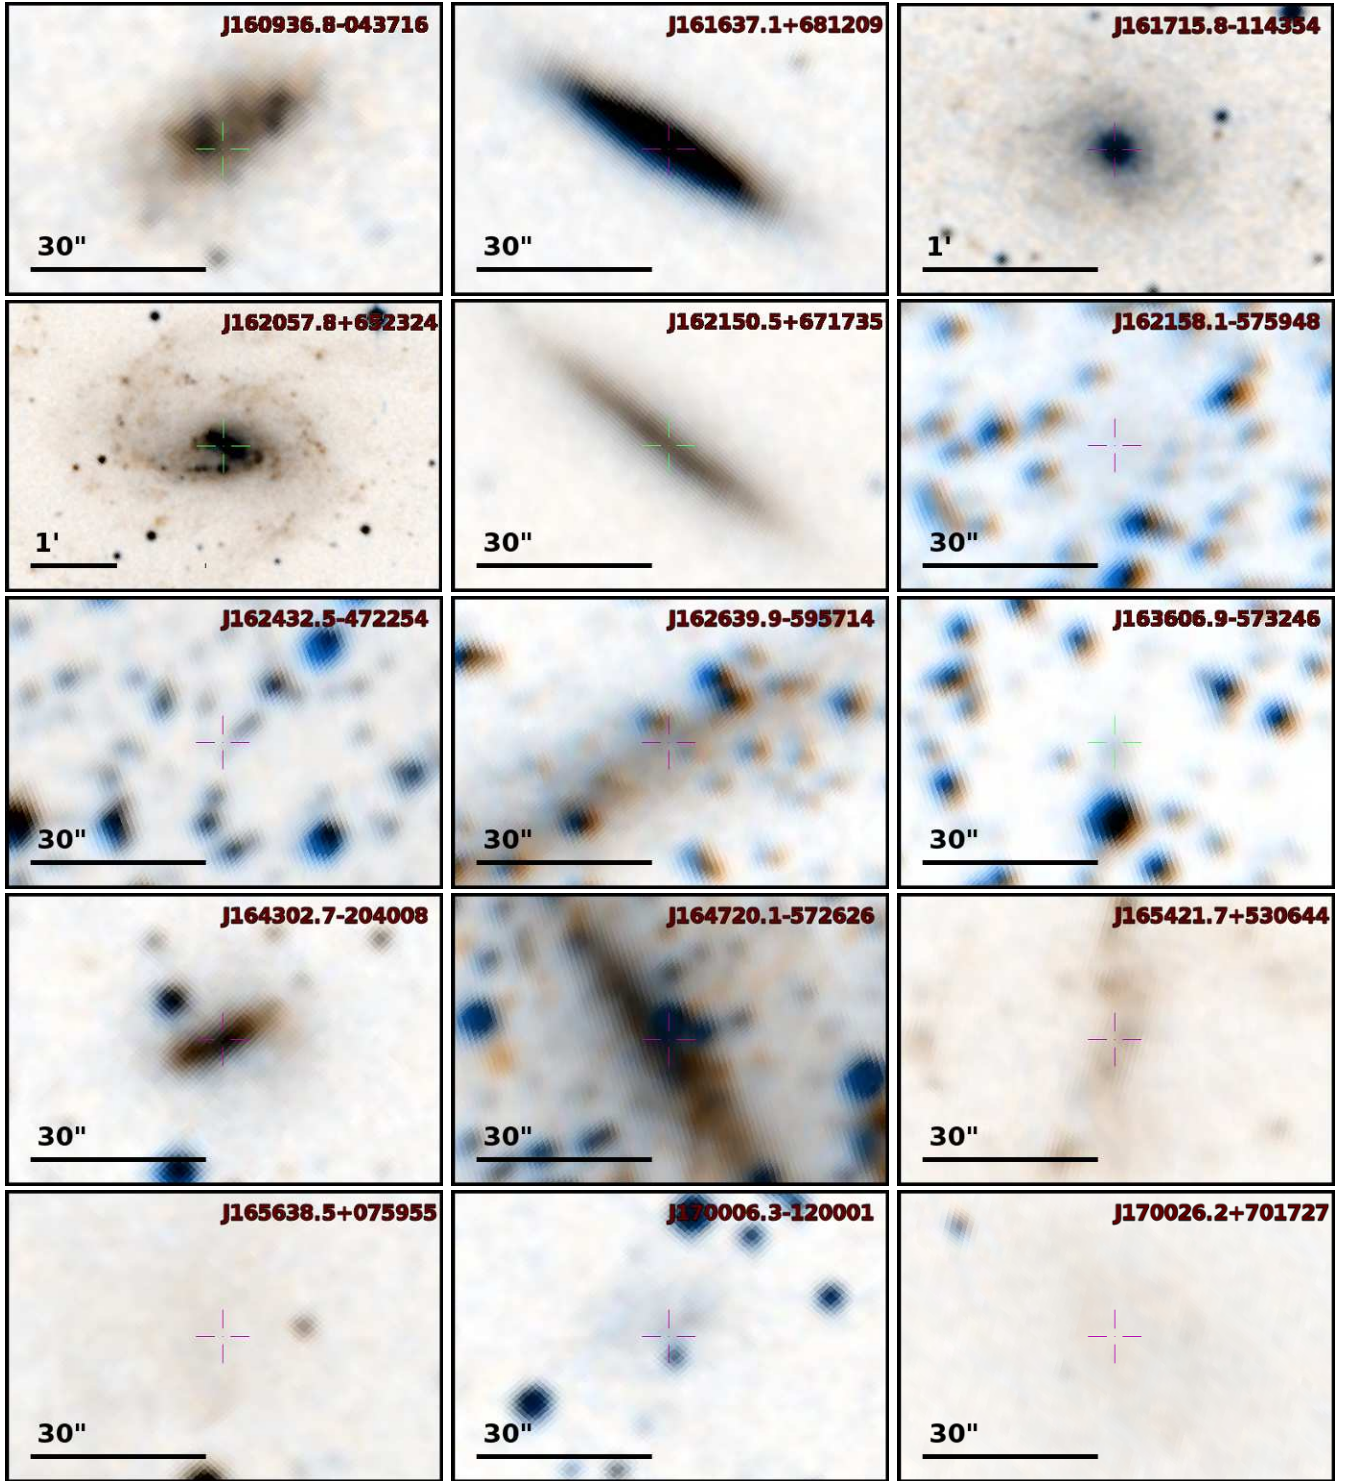

Figure A54. Nearby Void inner galaxies outside the SDSS footprint.

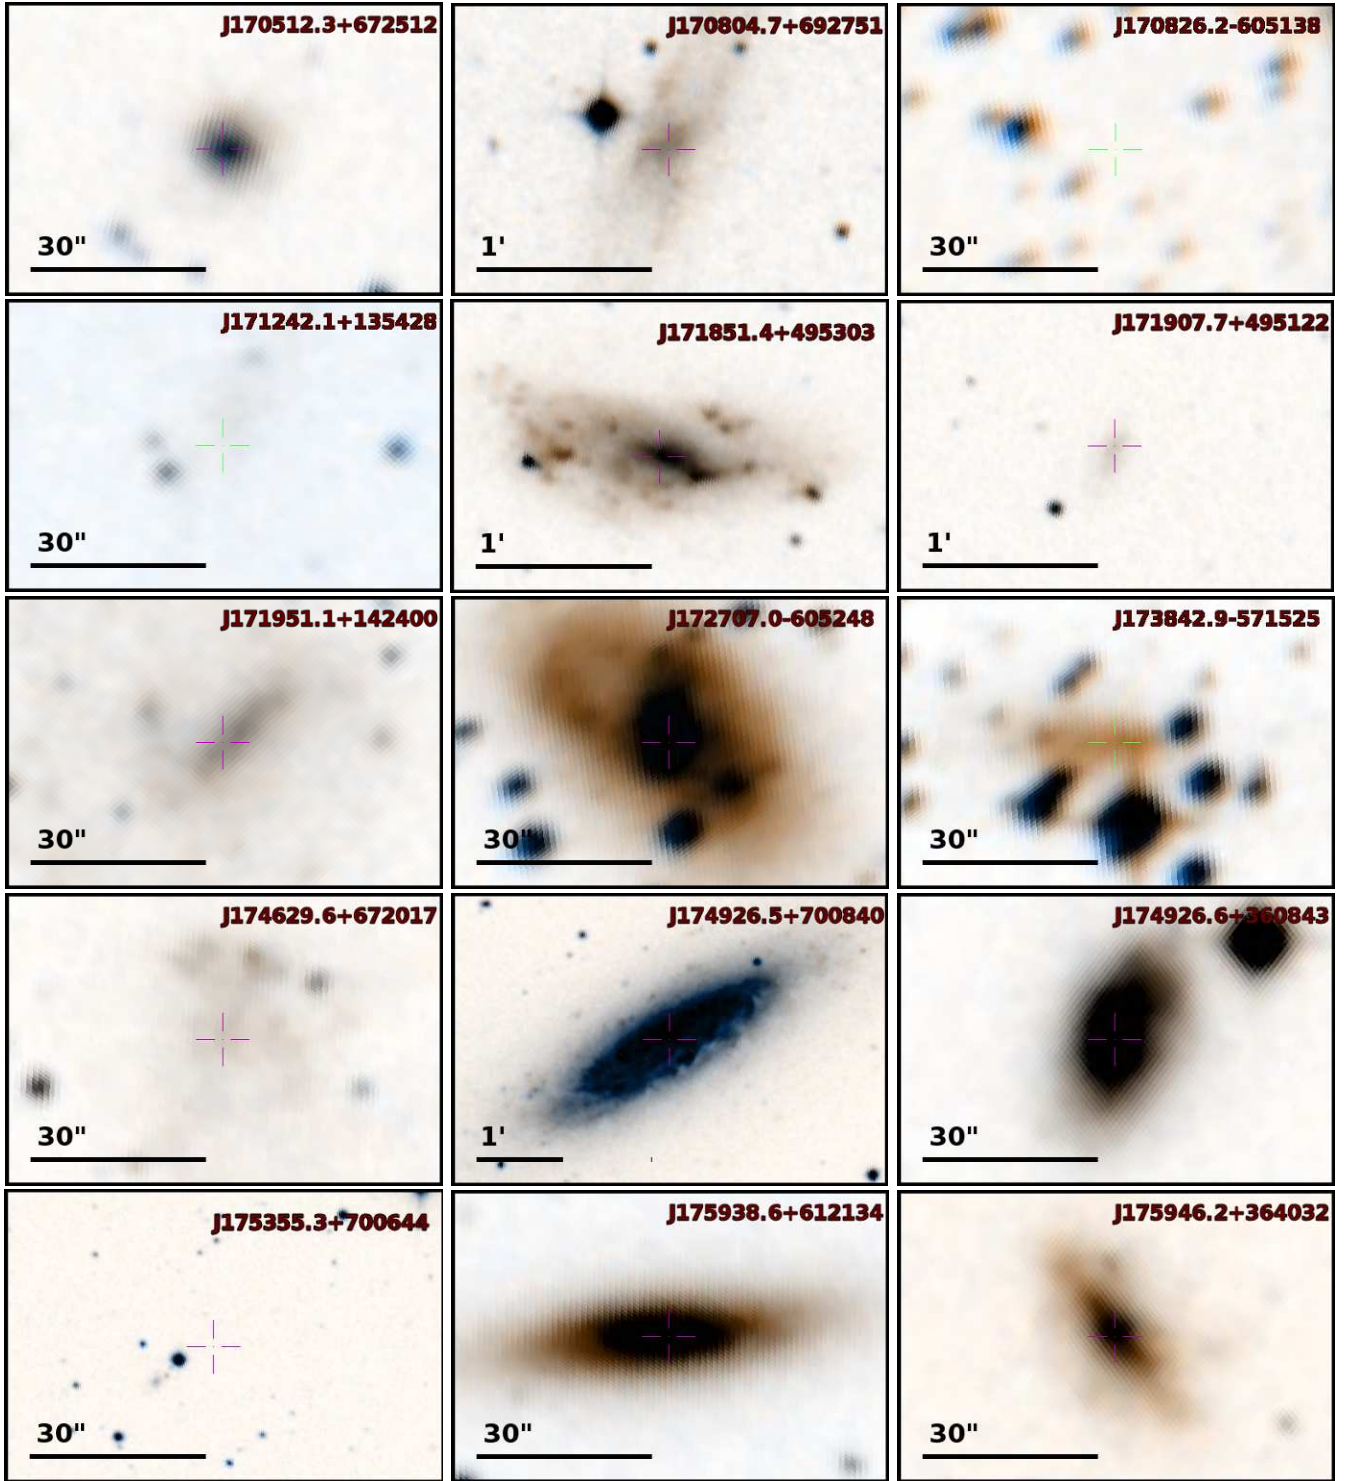

Figure A55. Nearby Void inner galaxies outside the SDSS footprint.



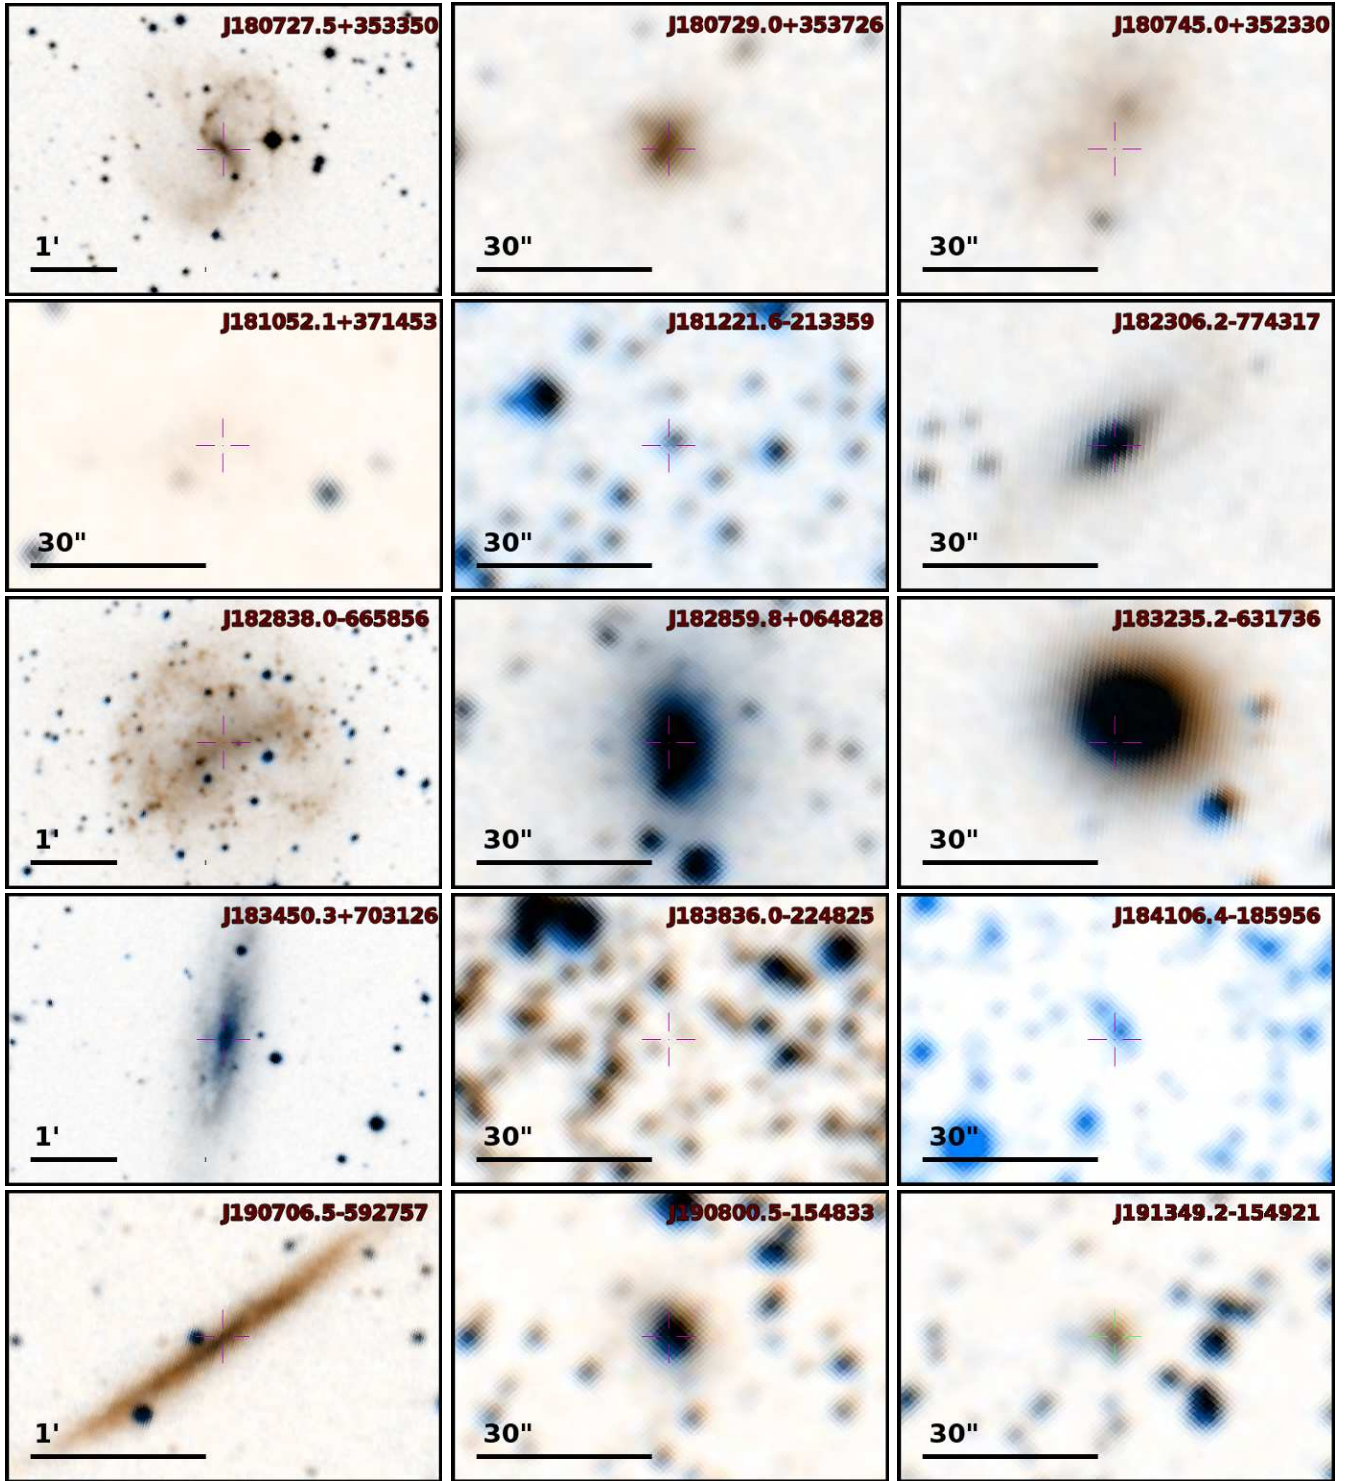

Figure A56. Nearby Void inner galaxies outside the SDSS footprint.

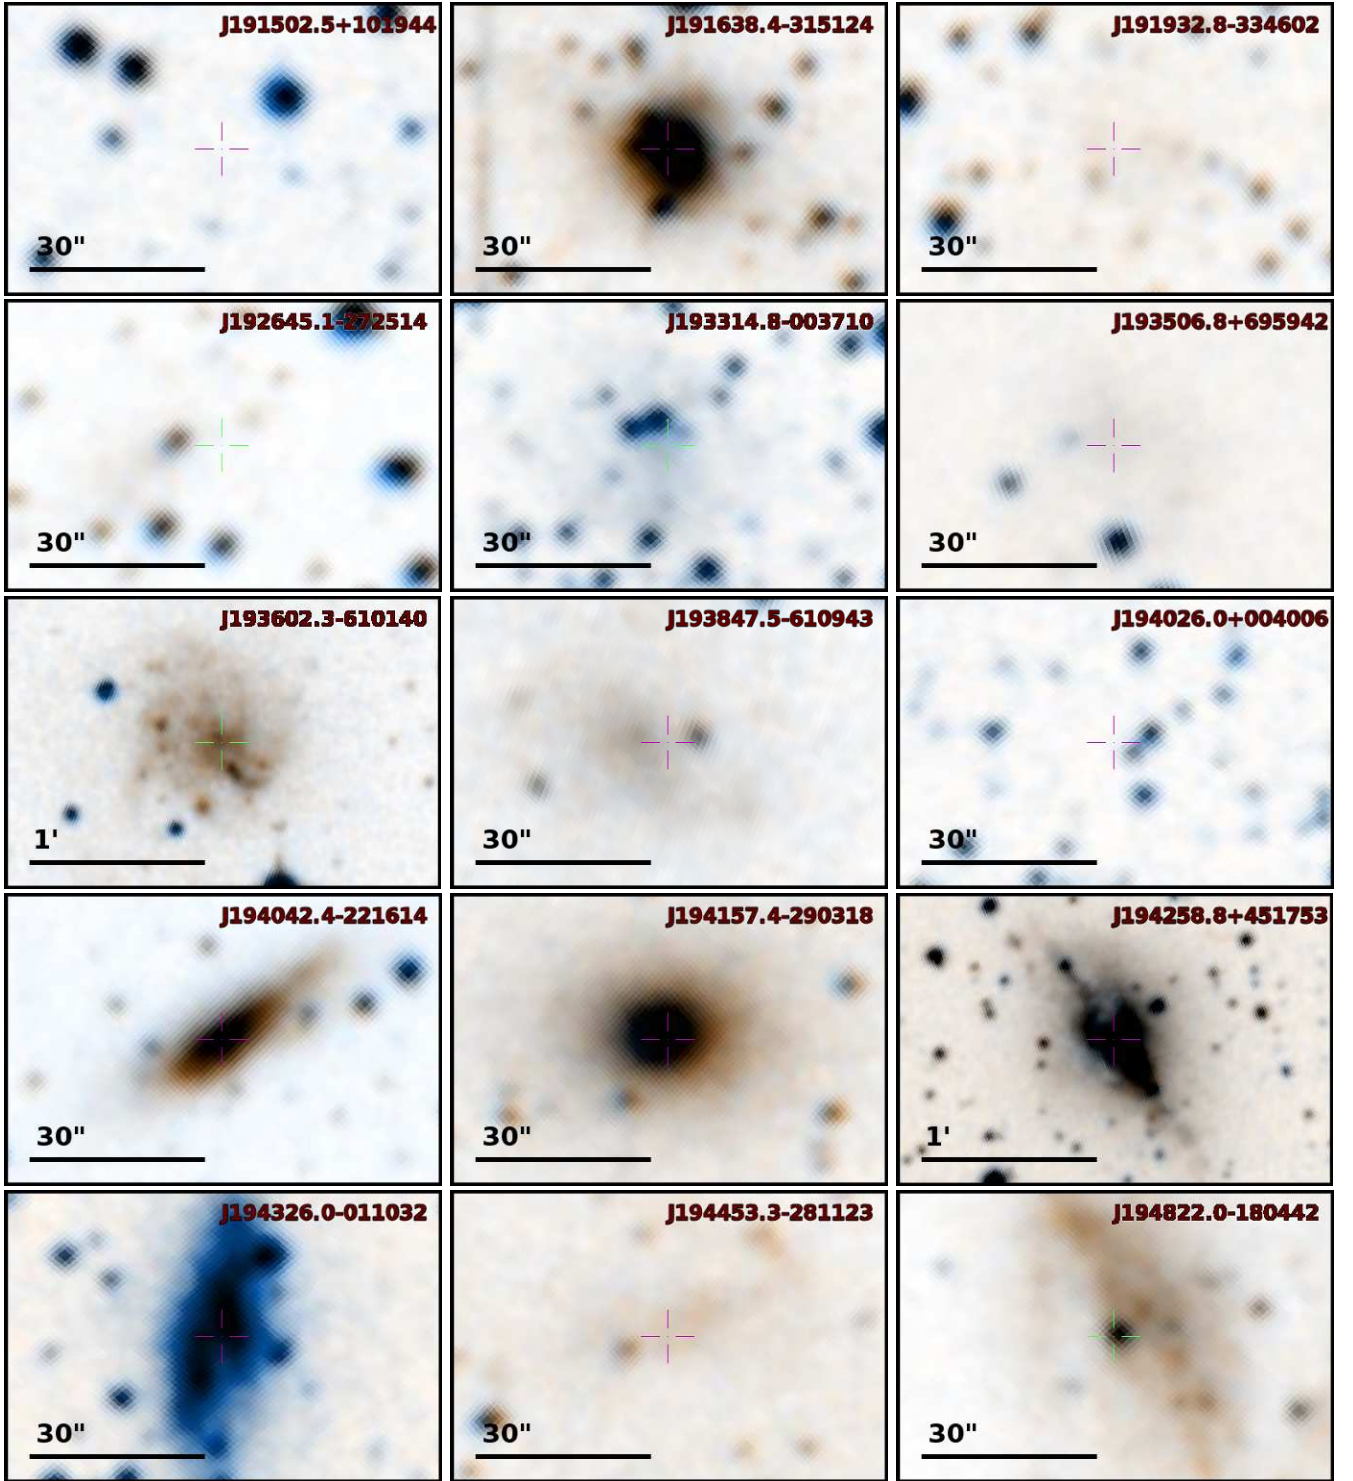

Figure A57. Nearby Void inner galaxies outside the SDSS footprint.



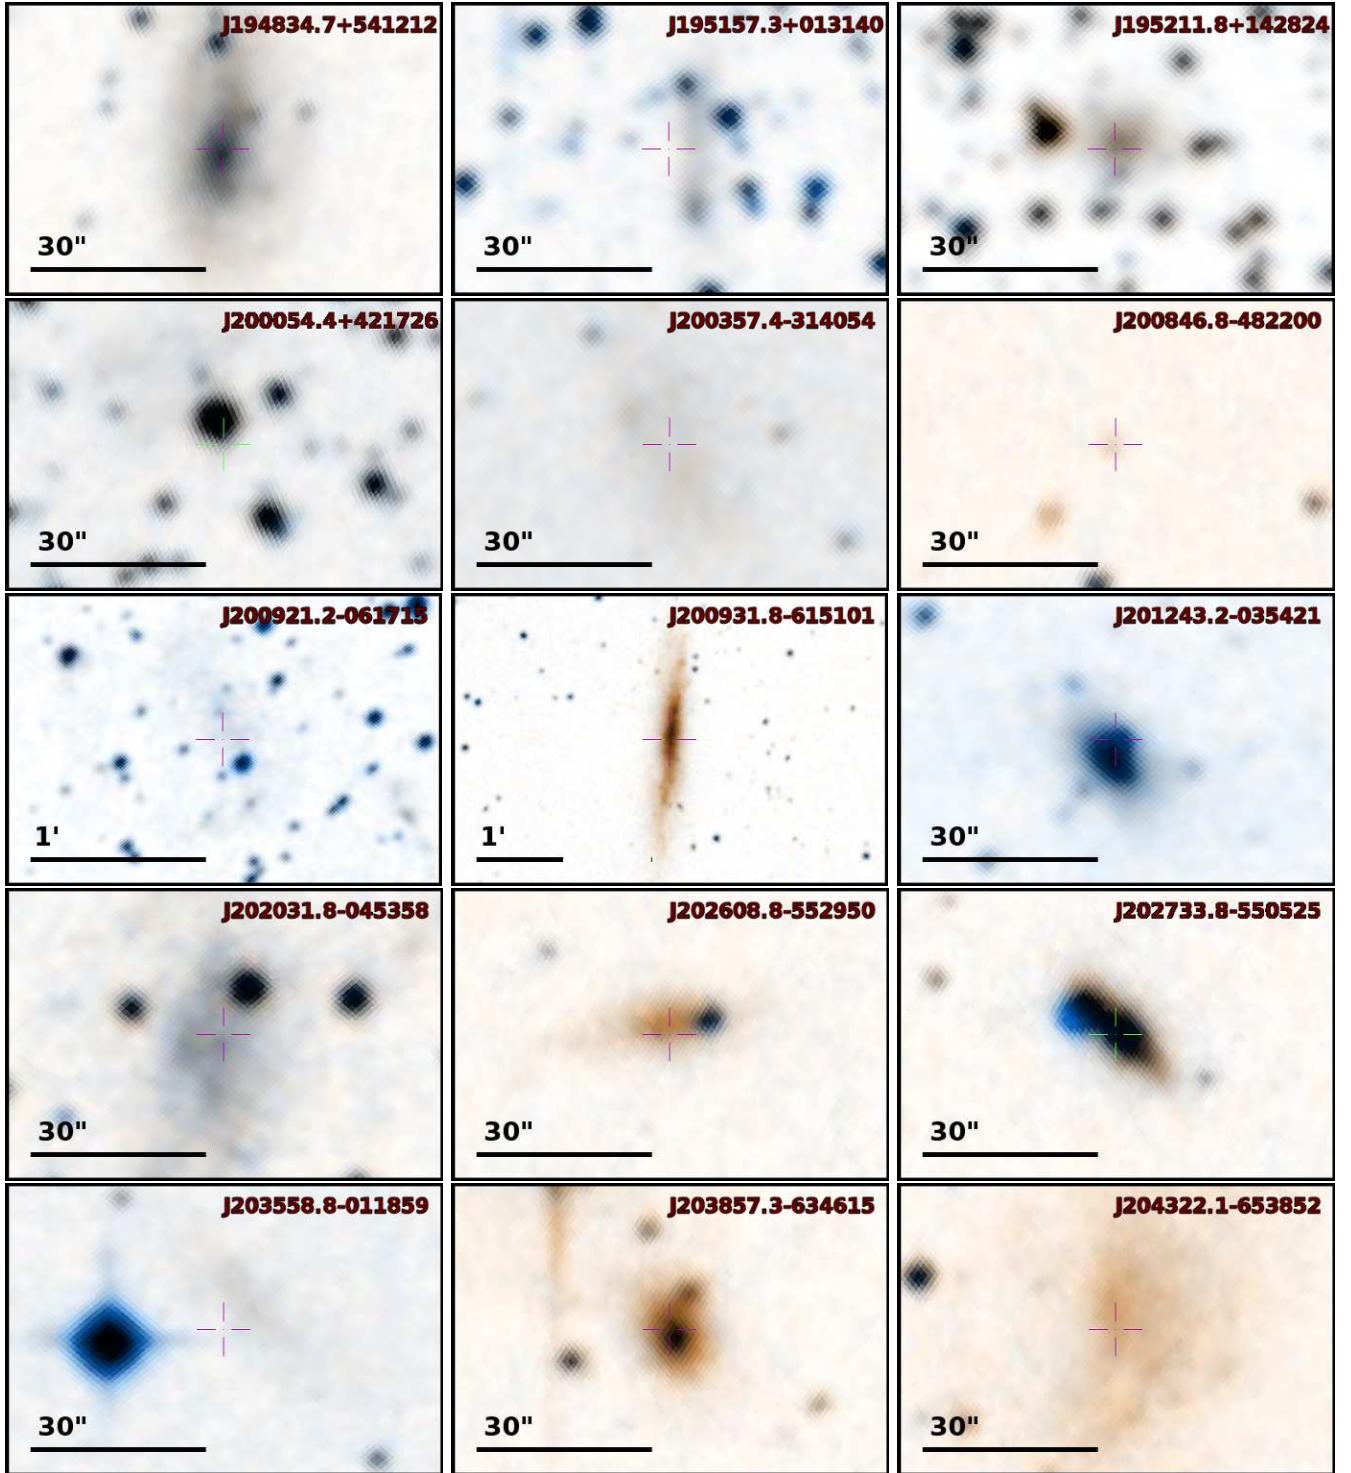

Figure A58. Nearby Void inner galaxies outside the SDSS footprint.



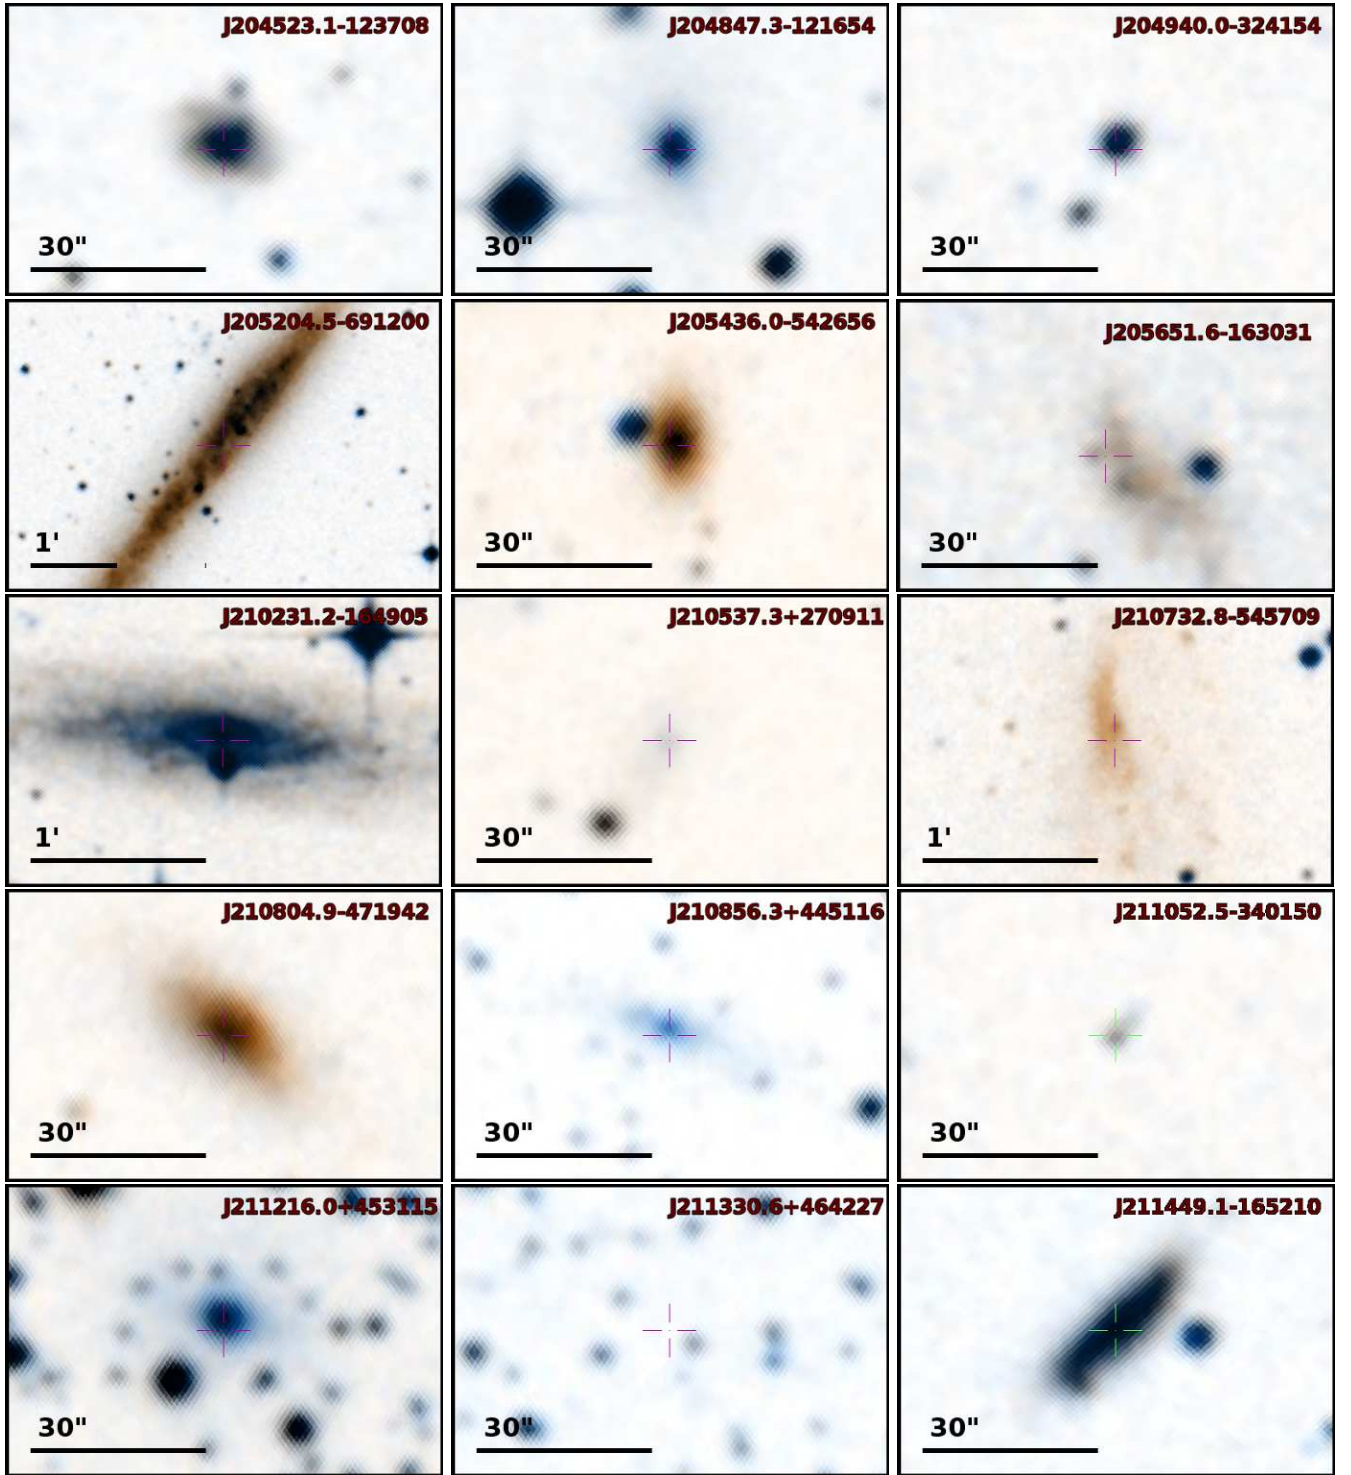

Figure A59. Nearby Void inner galaxies outside the SDSS footprint.

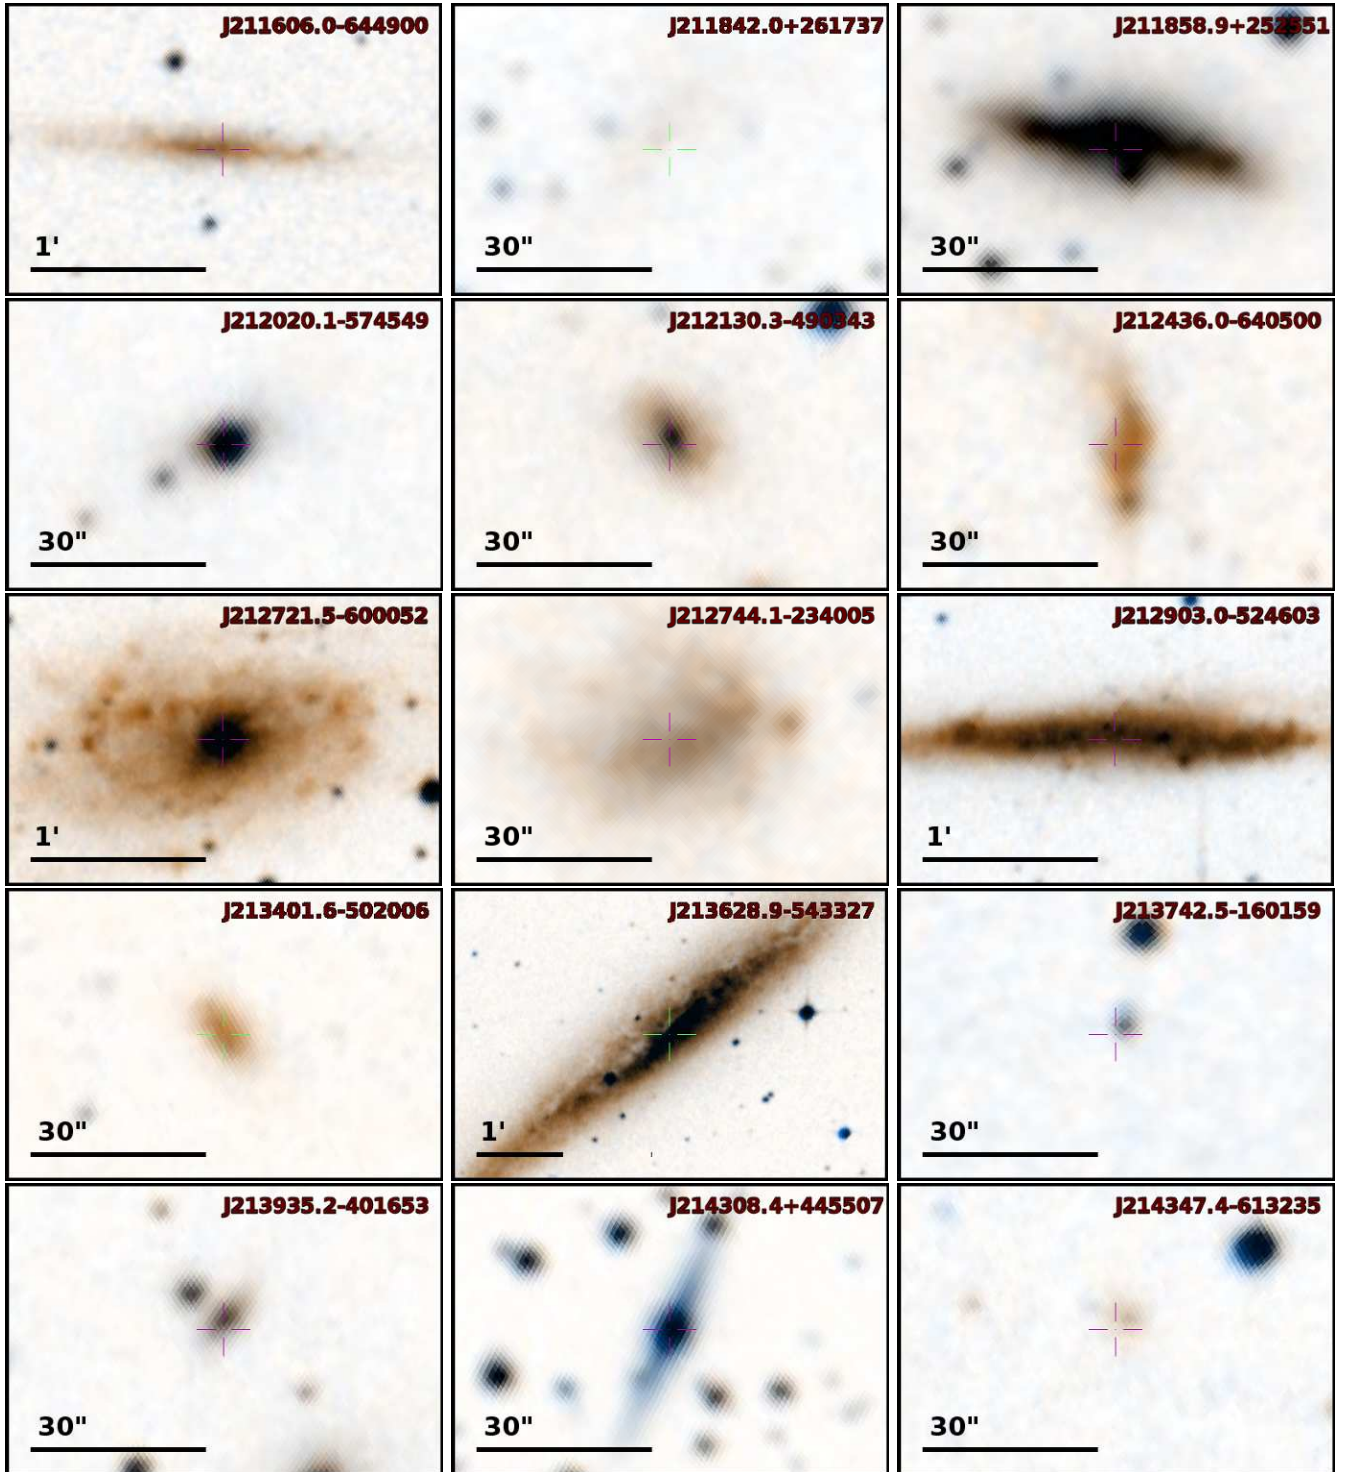

Figure A60. Nearby Void inner galaxies outside the SDSS footprint.

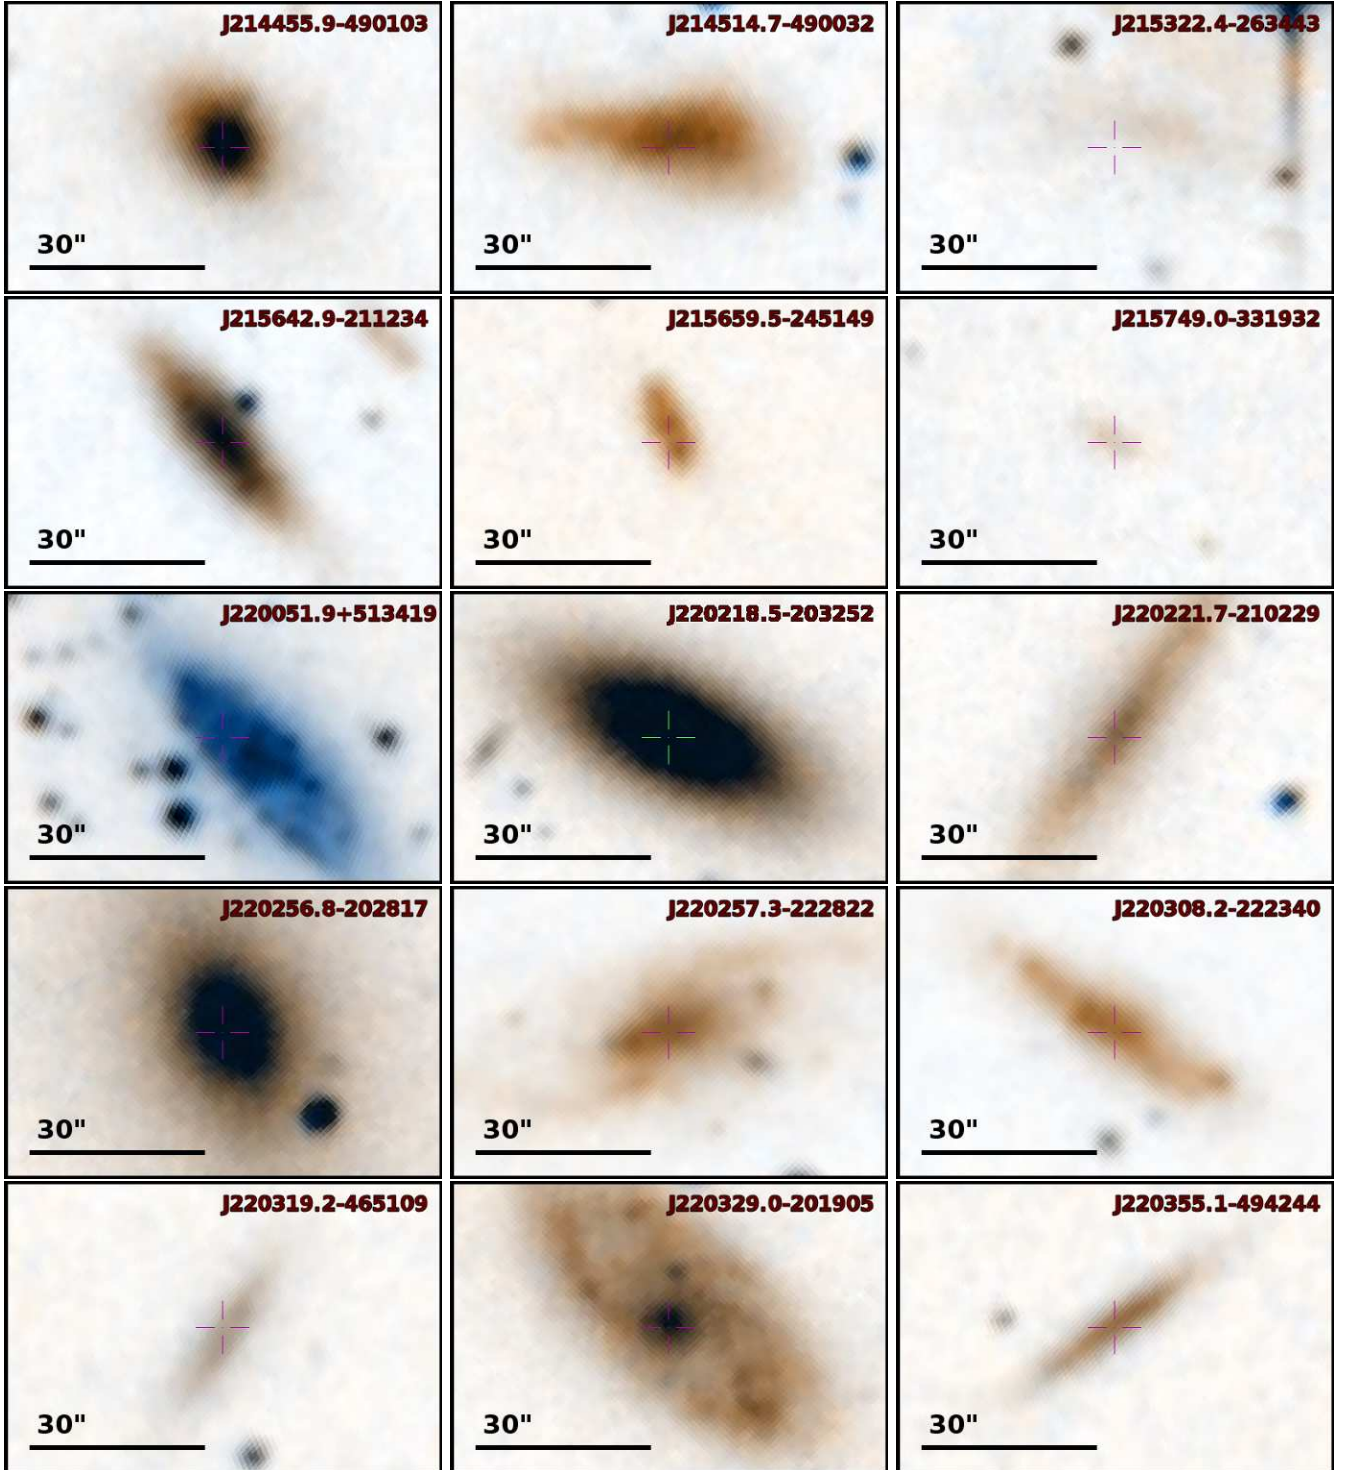

Figure A61. Nearby Void inner galaxies outside the SDSS footprint.



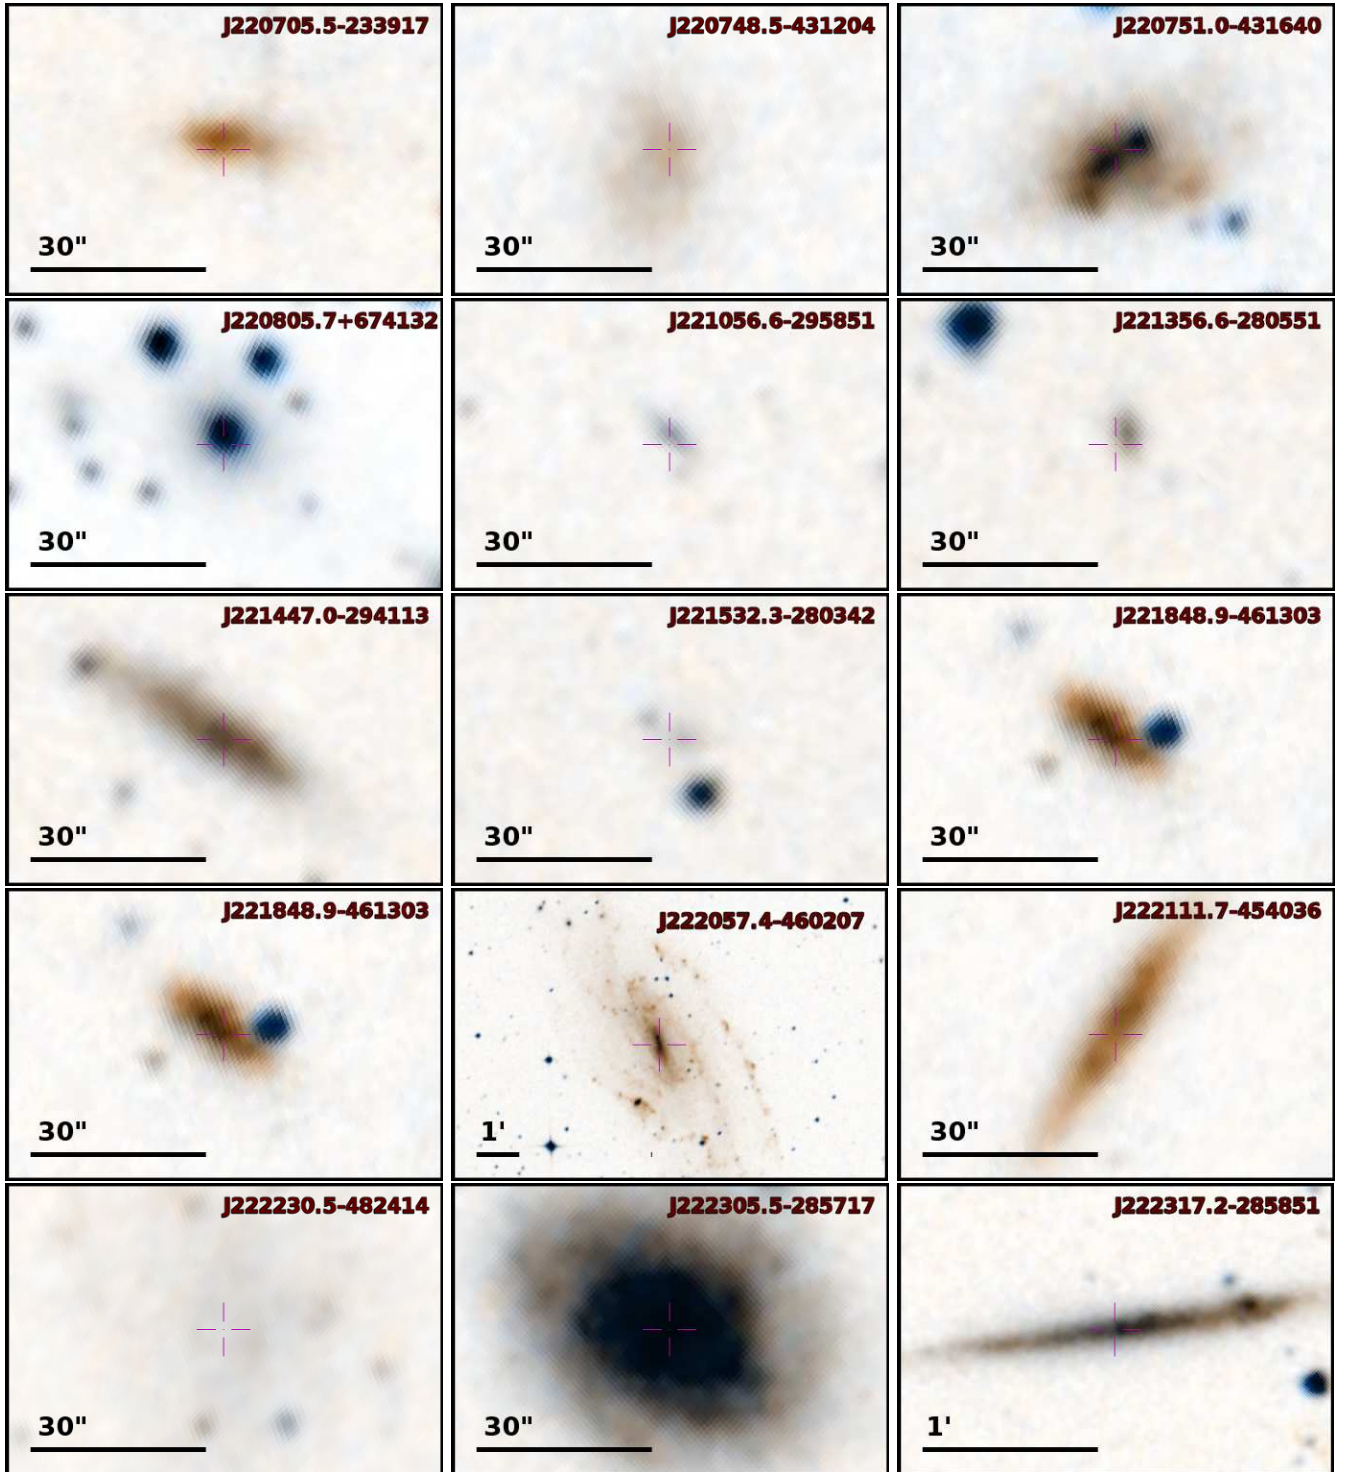

Figure A62. Nearby Void inner galaxies outside the SDSS footprint.



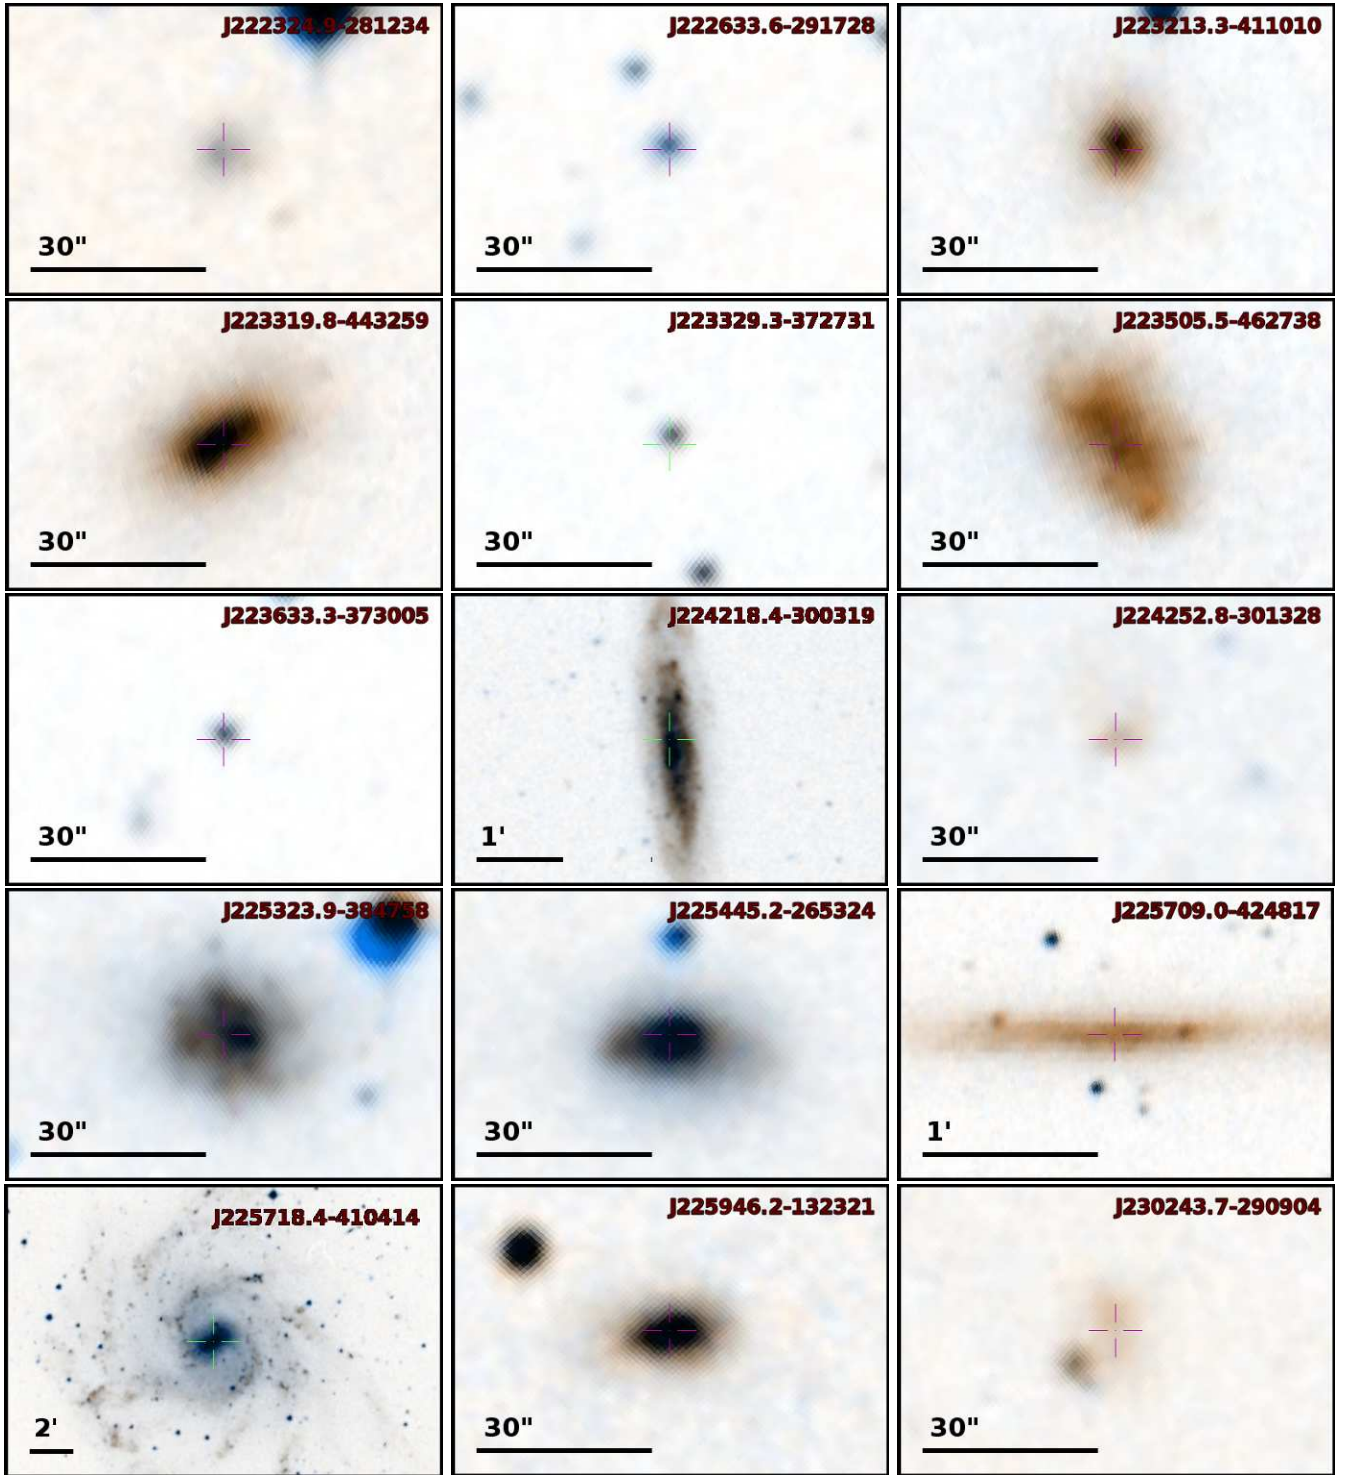

Figure A63. Nearby Void inner galaxies outside the SDSS footprint.

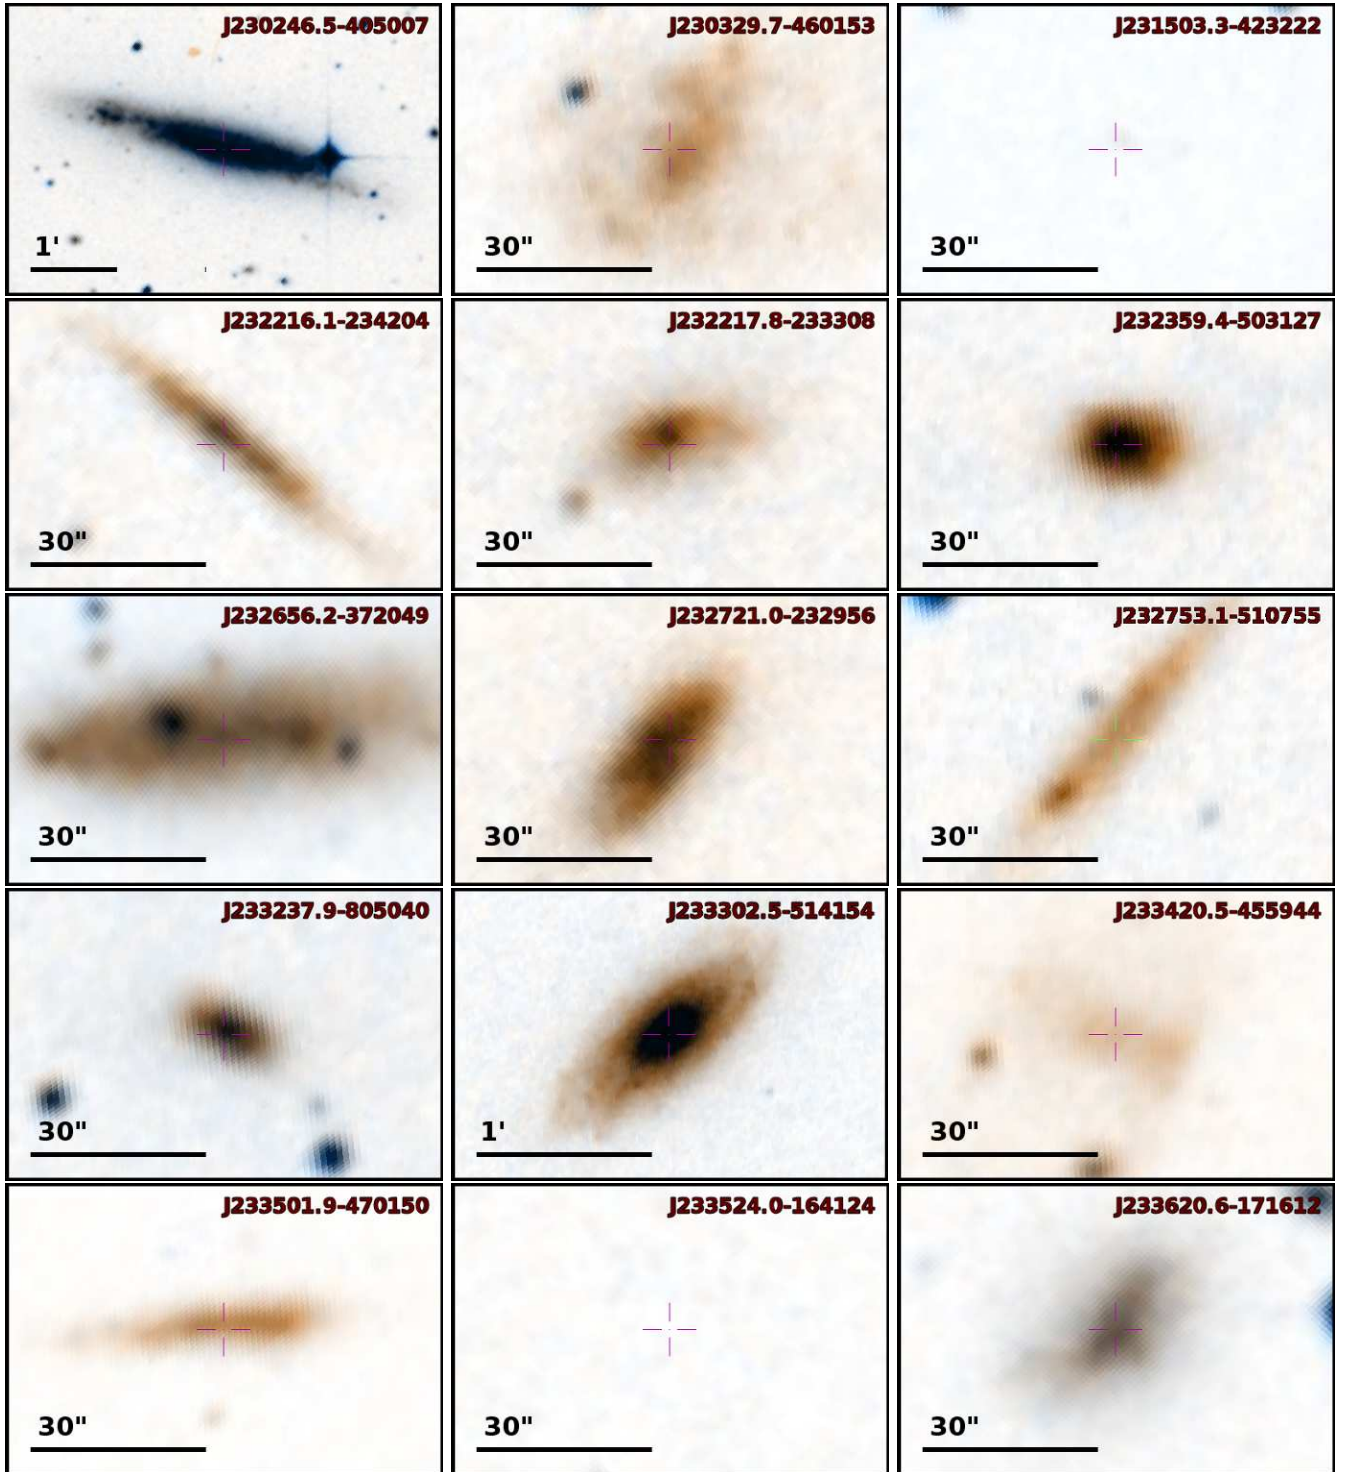

Figure A64. Nearby Void inner galaxies outside the SDSS footprint.

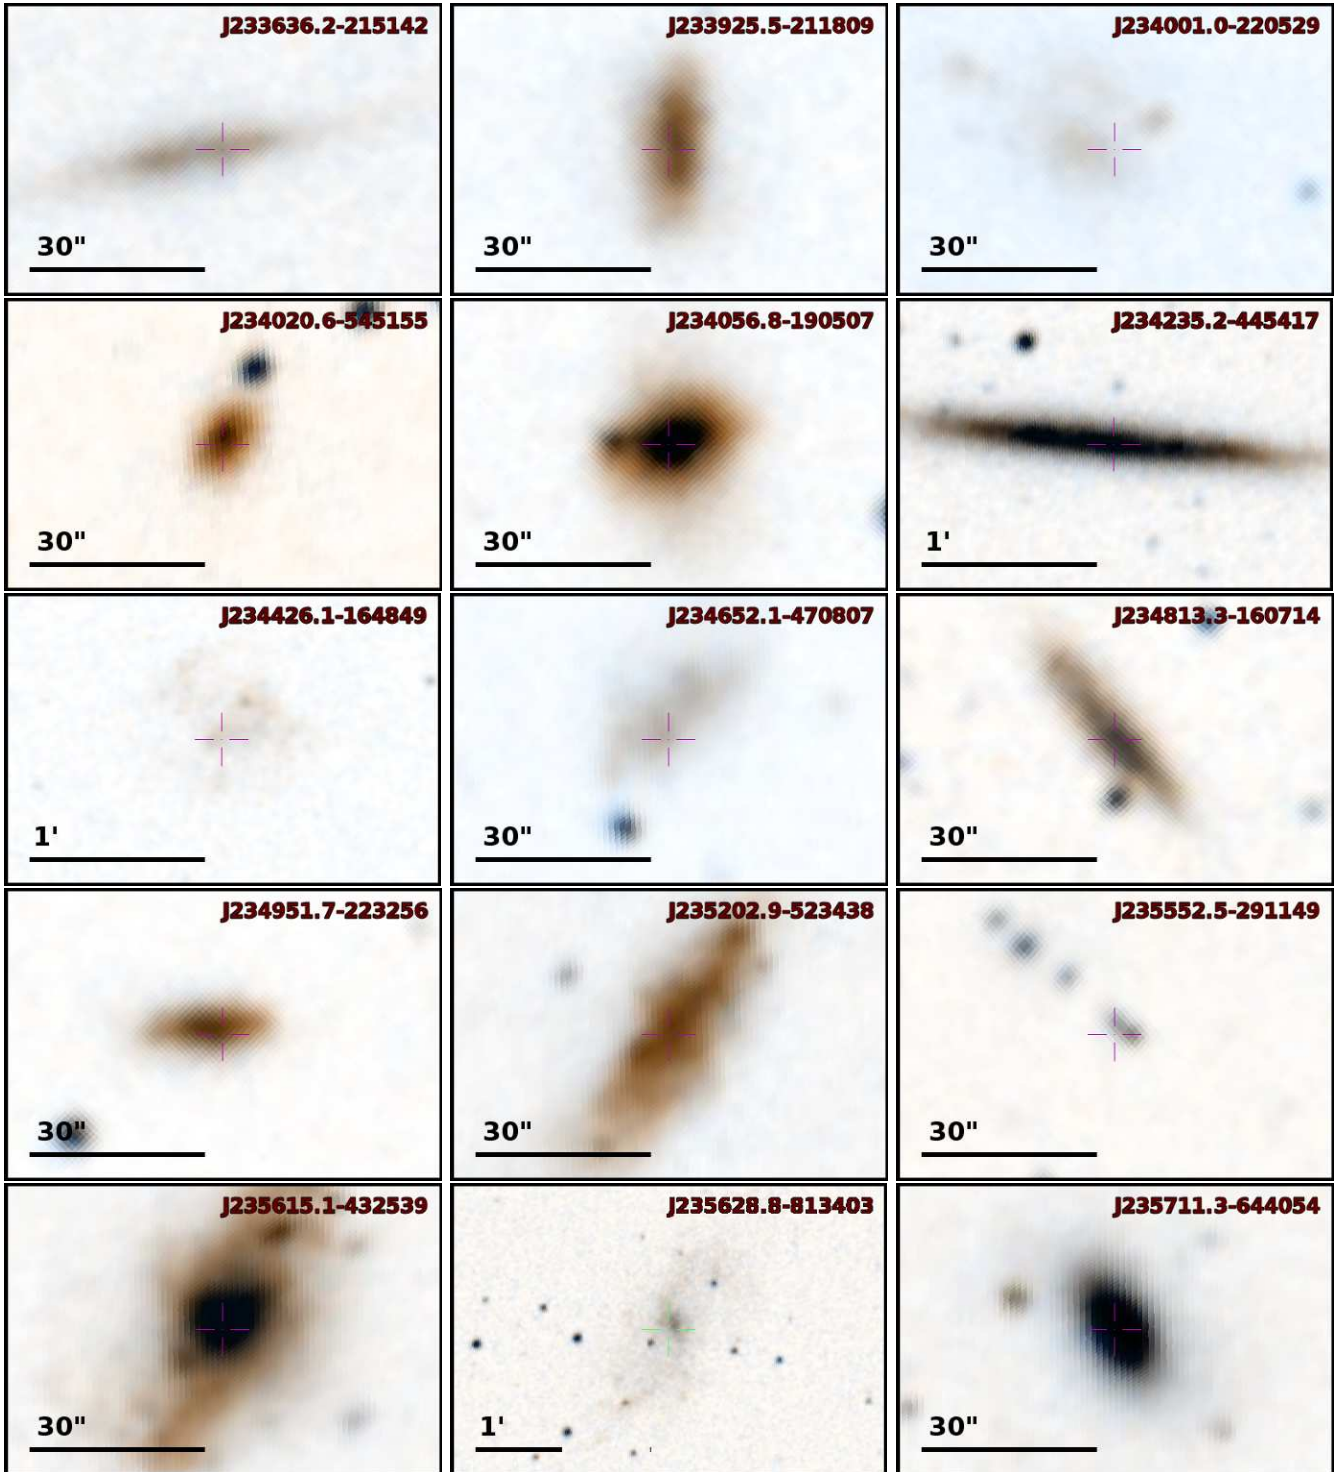

Figure A65. Nearby Void inner galaxies outside the SDSS footprint.



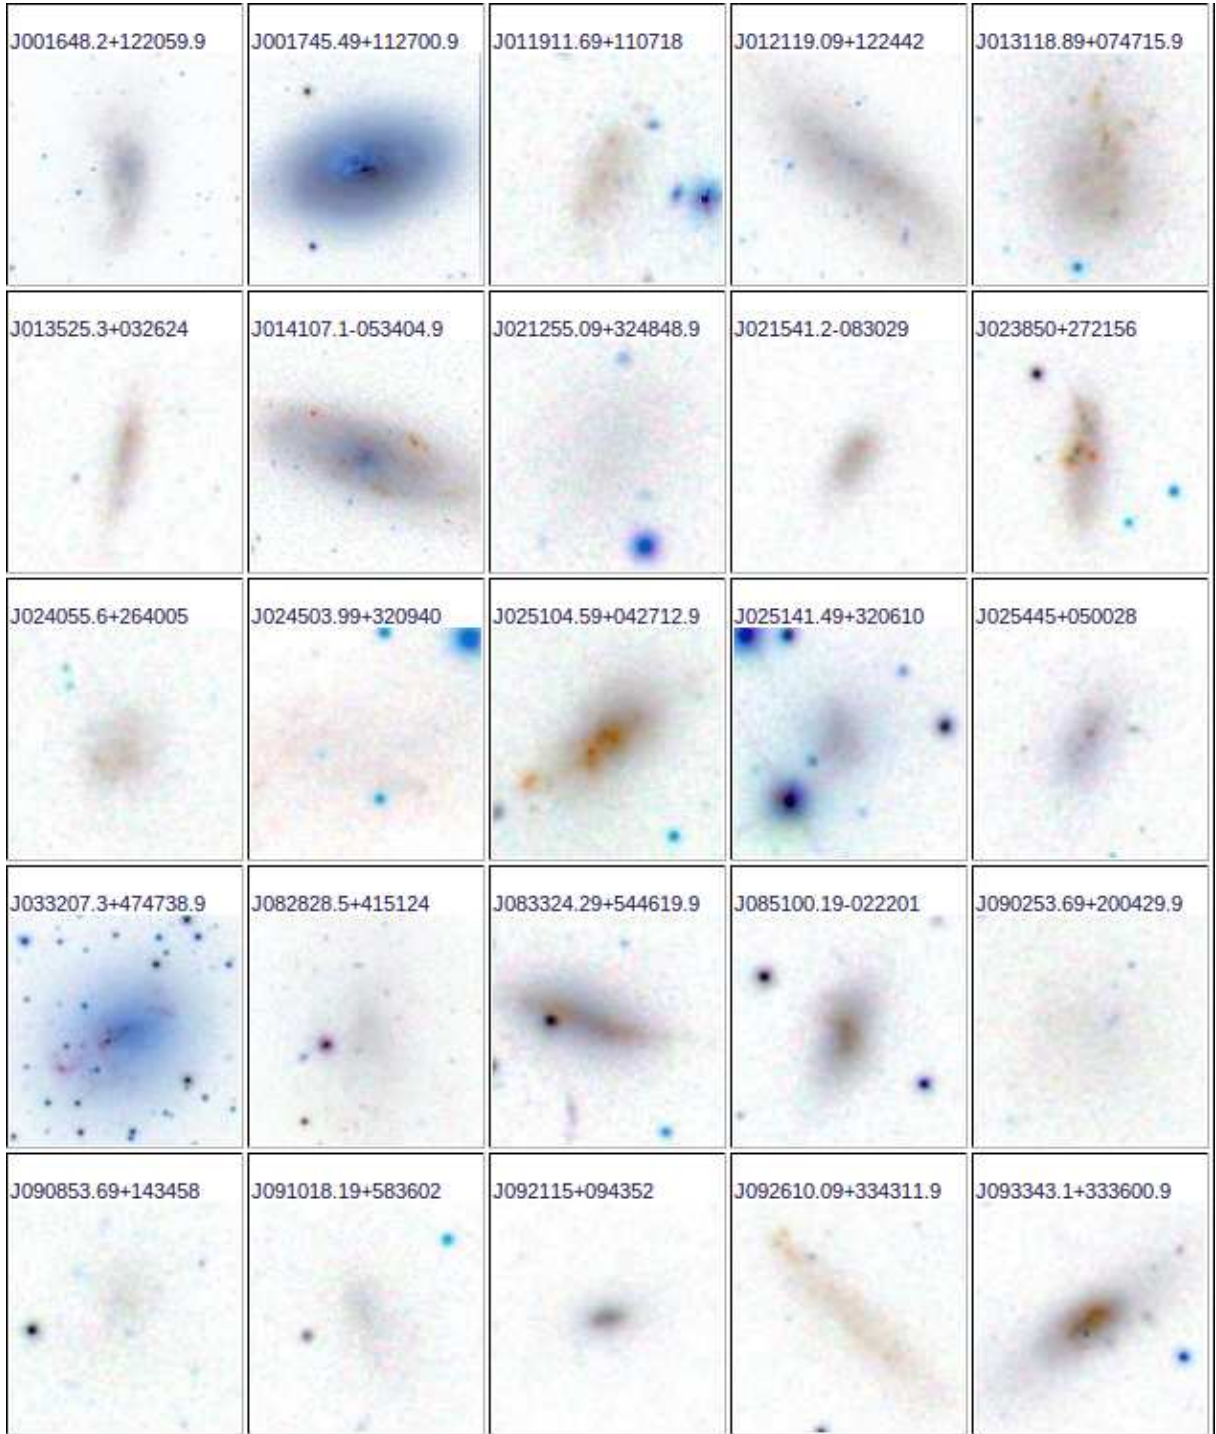

**Figure A66.** Mosaics of the first 25 'outer' nearby void galaxies prepared from the SDSS colour images. The side of the chart is 50".



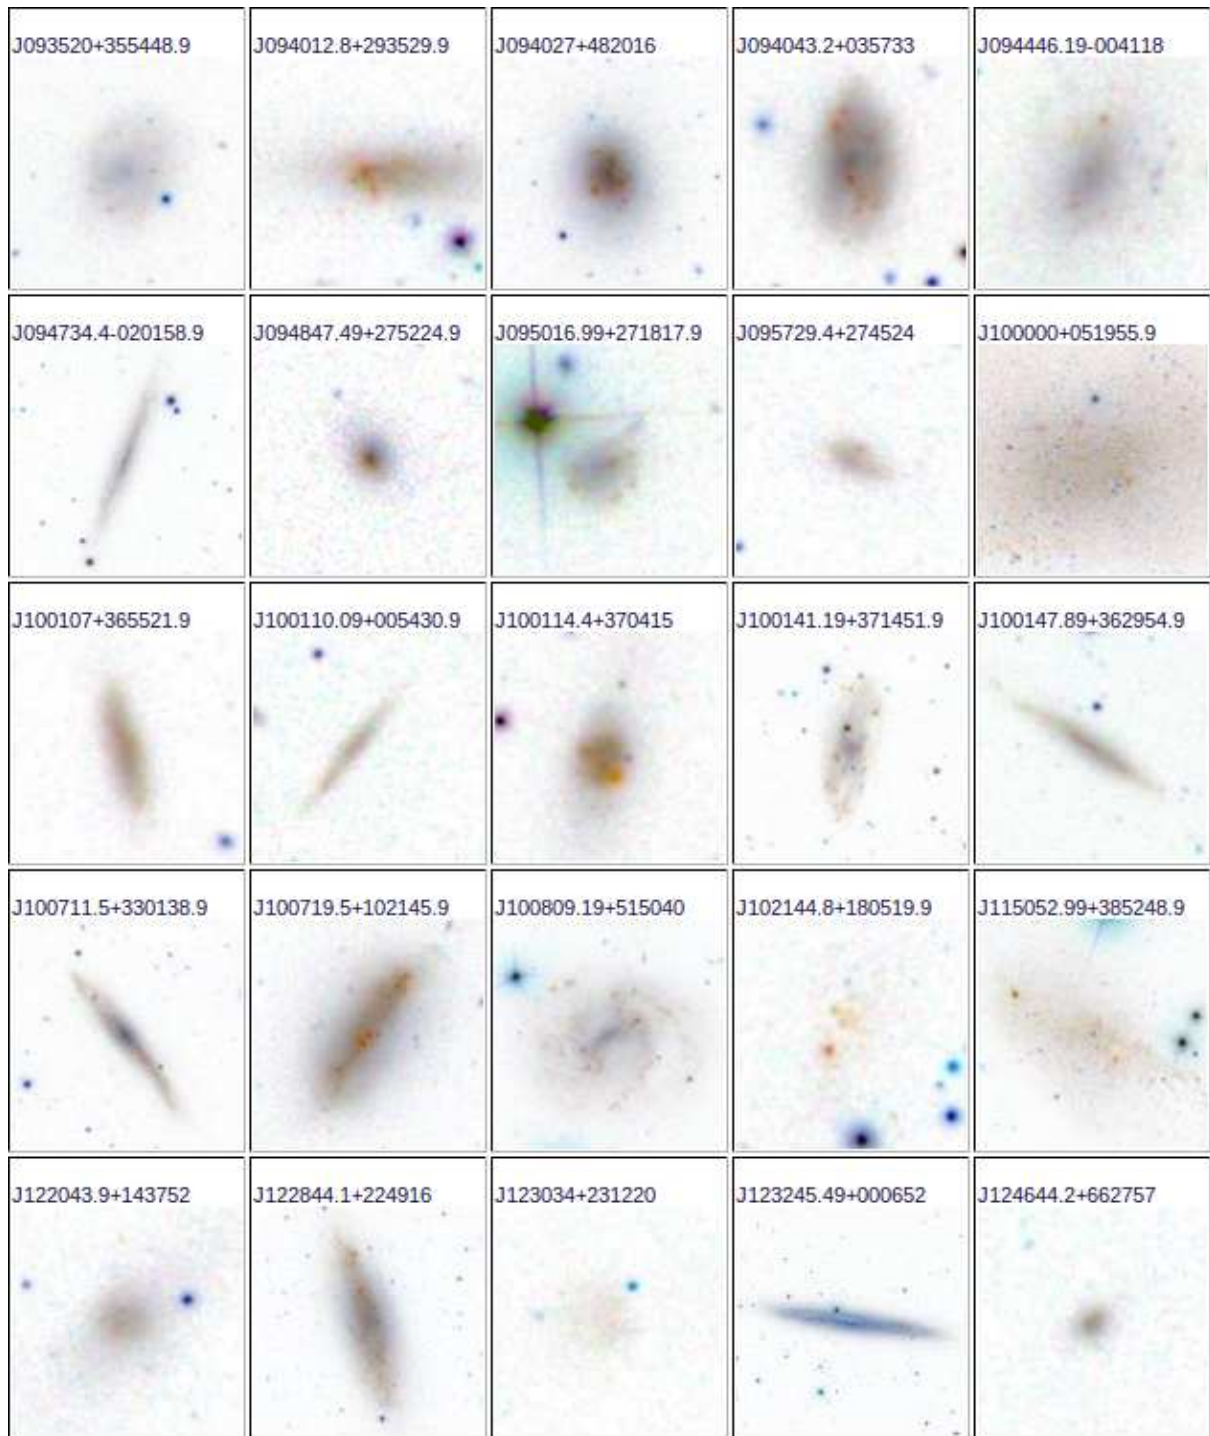

**Figure A67.** Mosaics of the next 25 'outer' nearby void galaxies prepared from the SDSS colour images. The side of the chart is  $50''$ .

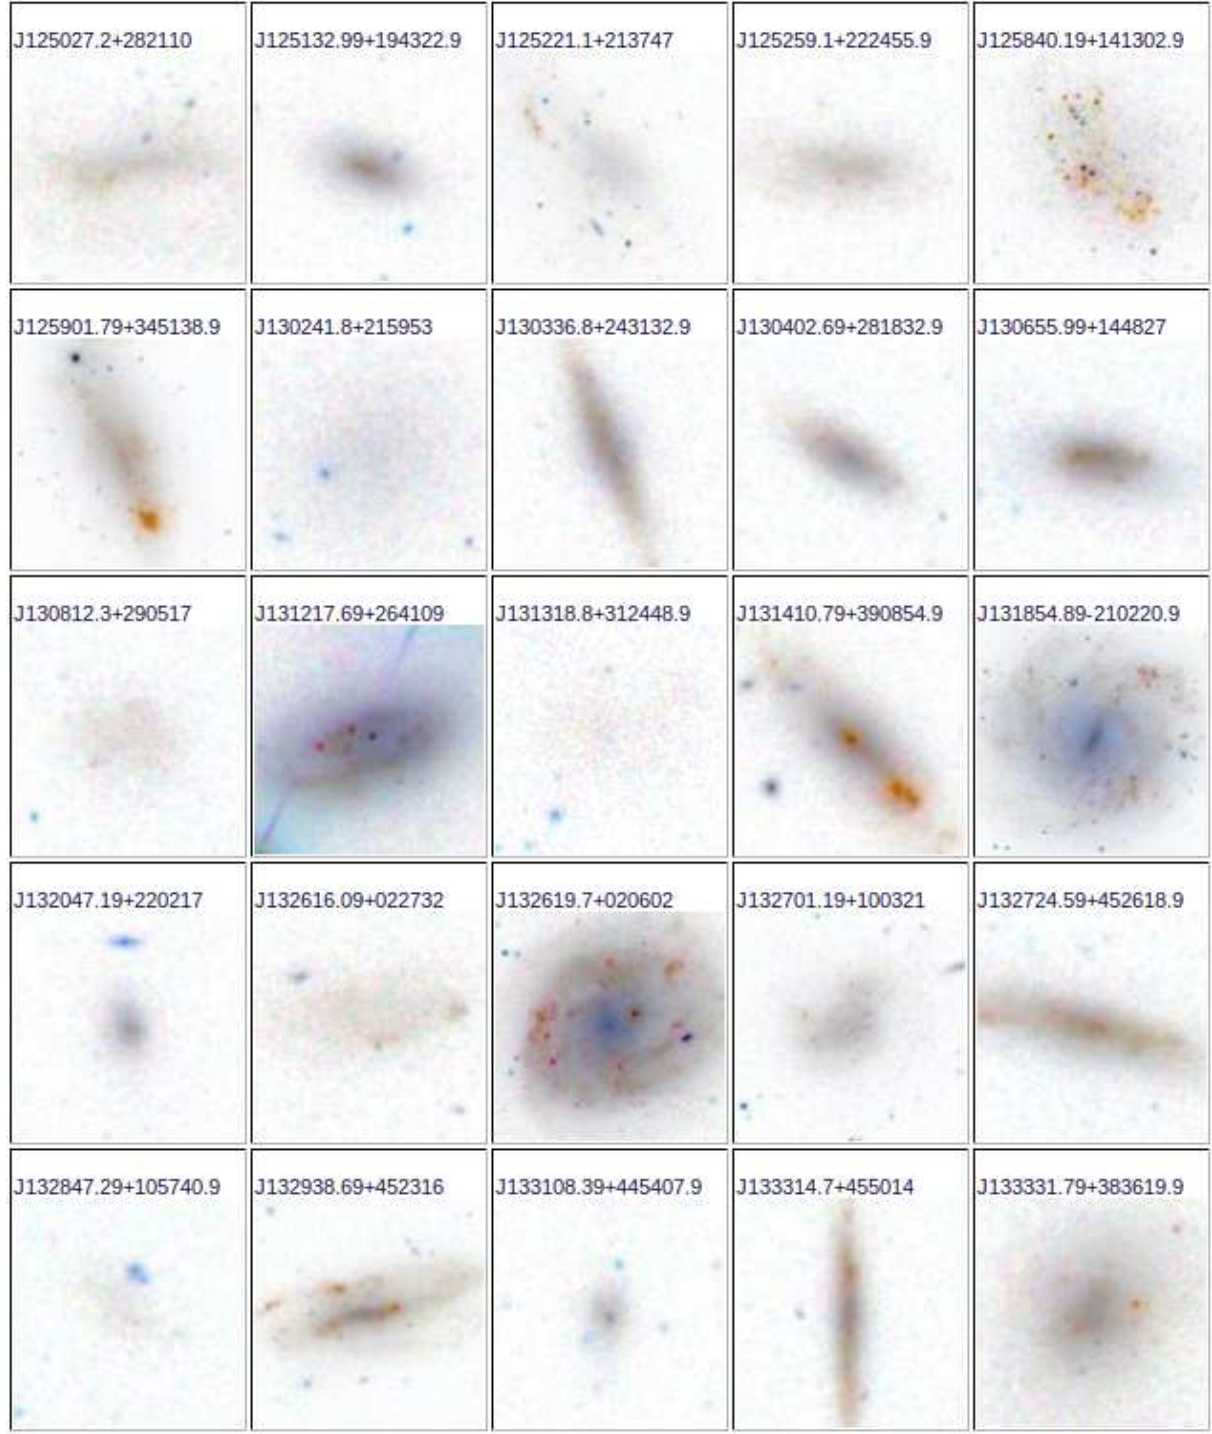

**Figure A68.** Mosaics of the next 25 'outer' nearby void galaxies prepared from the SDSS colour images. The side of the chart is 50".

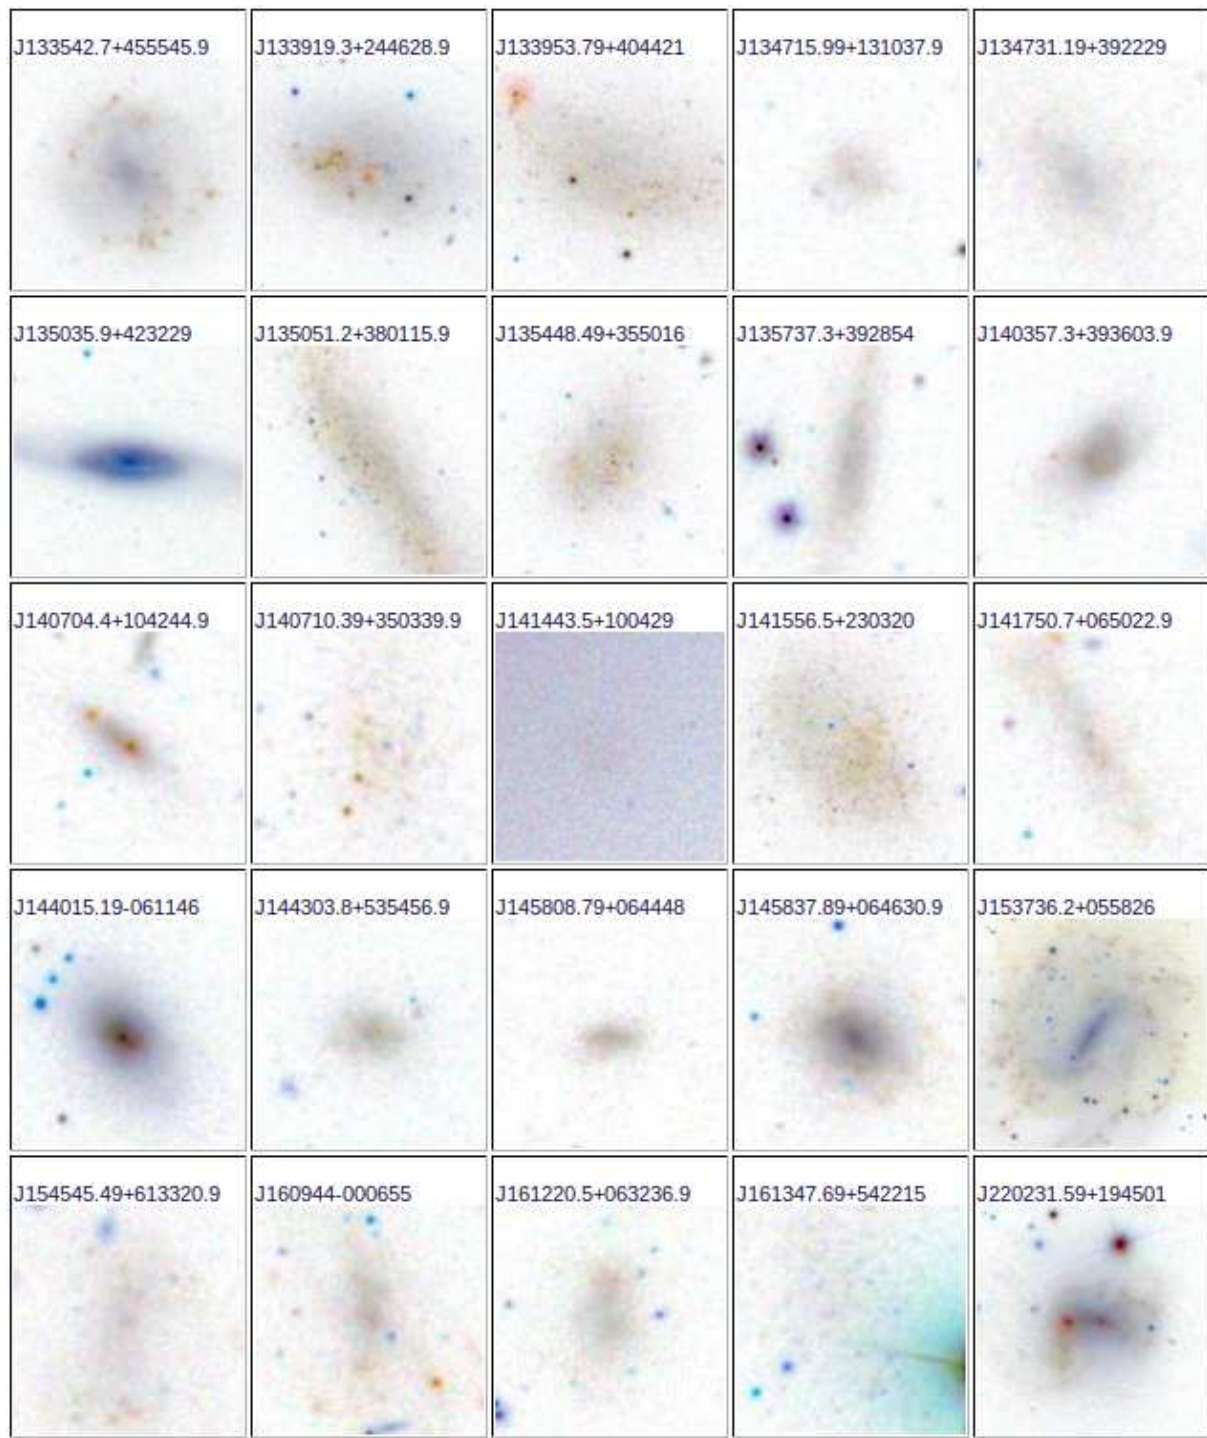

**Figure A69.** Mosaics of the next 25 'outer' nearby void galaxies prepared from the SDSS colour images. The side of the chart is 50".

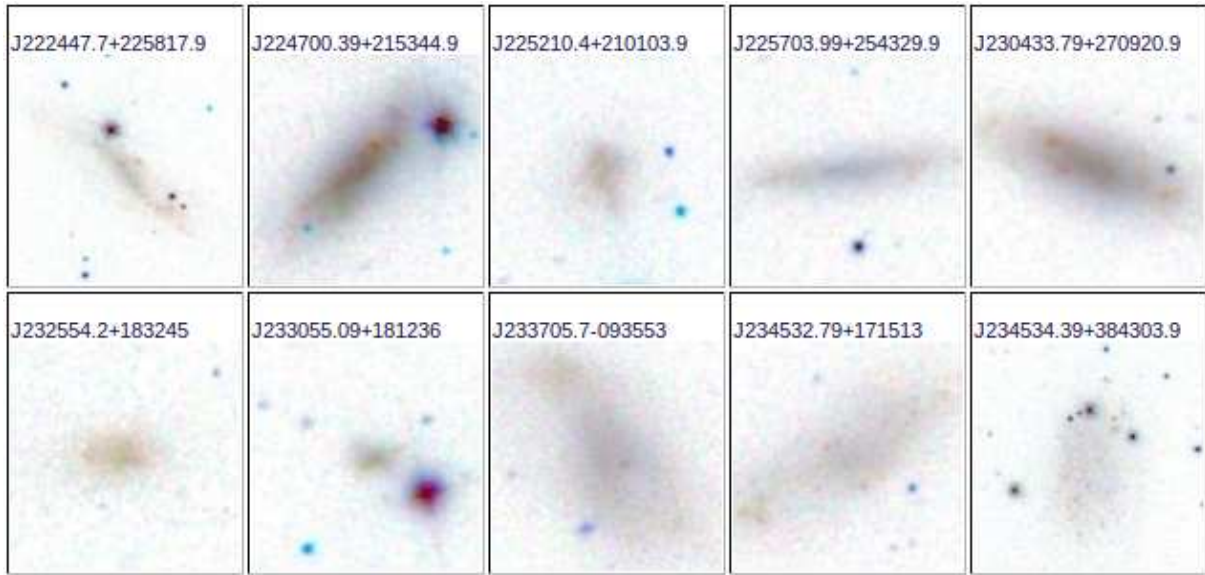

**Figure A70.** Mosaics of the lastt 13 'outer' nearby void galaxies prepared from the SDSS colour images. The side of the chart is 50".



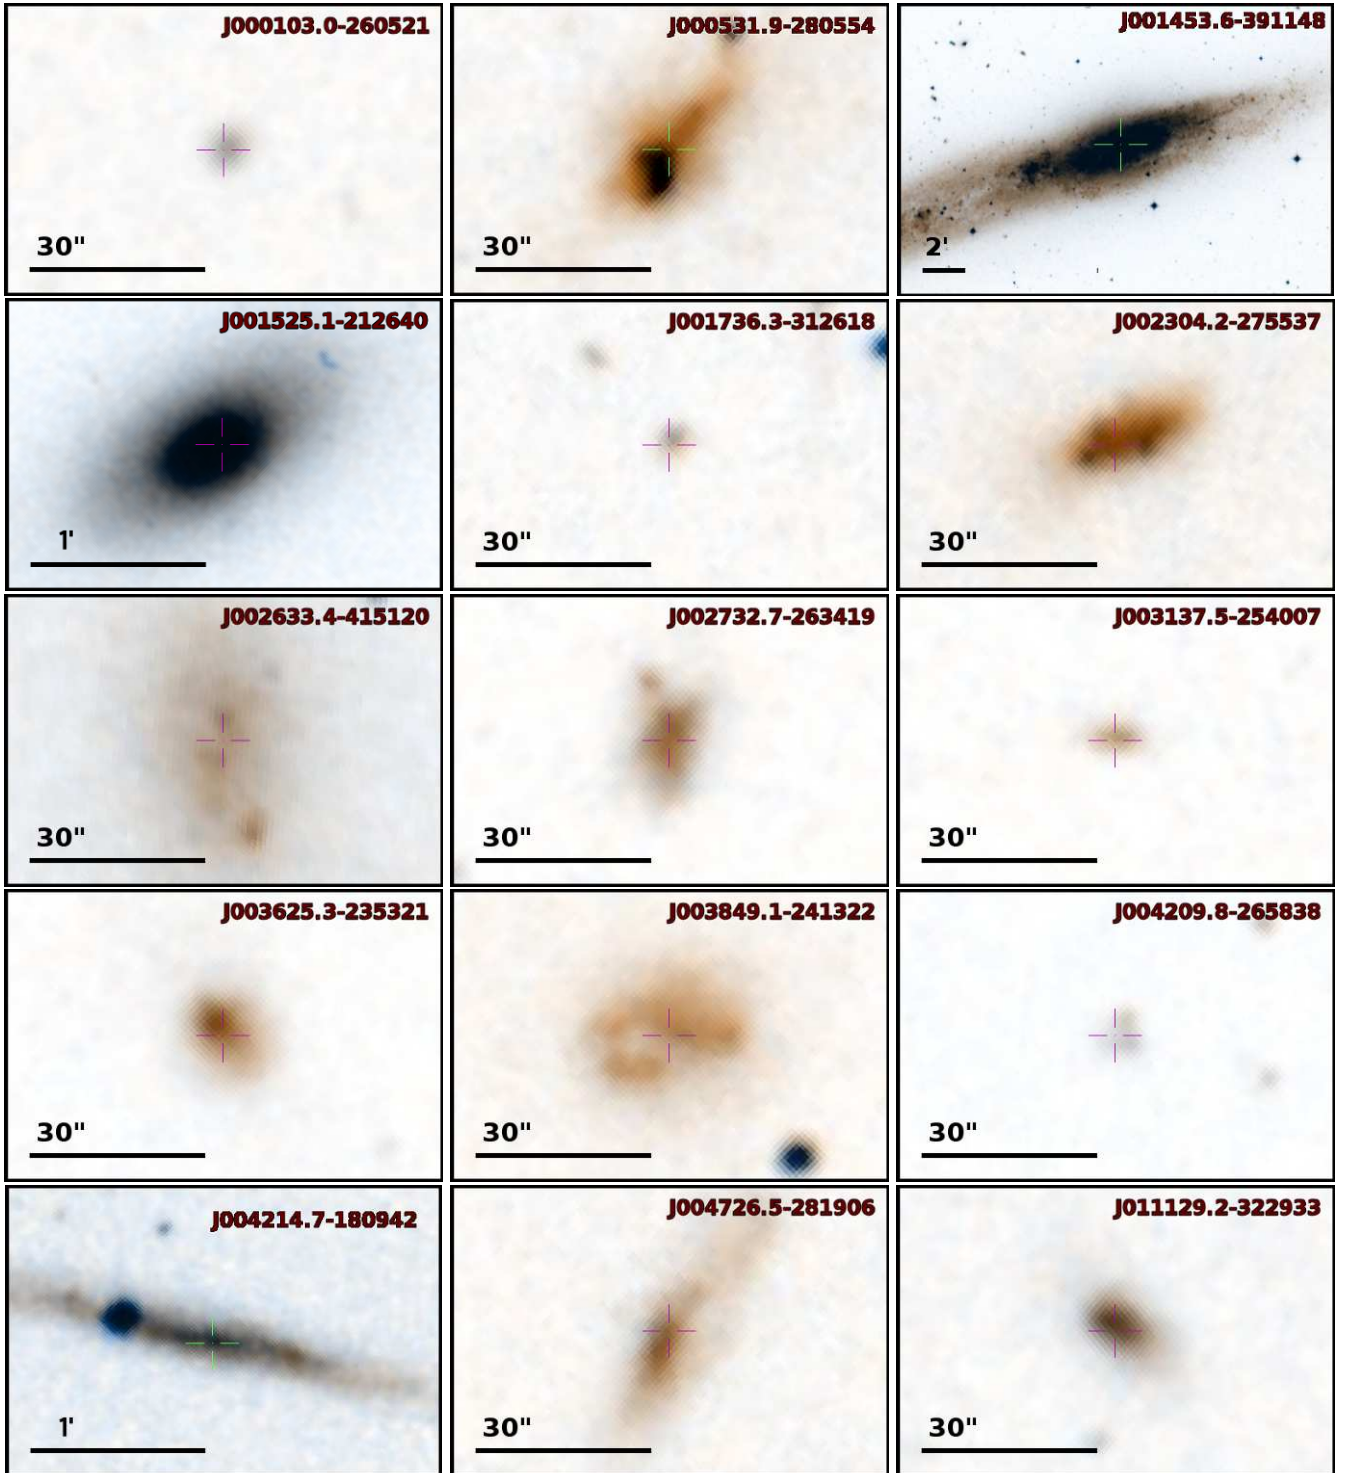

Figure A71. Nearby Void outer galaxies outside the SDSS footprint.

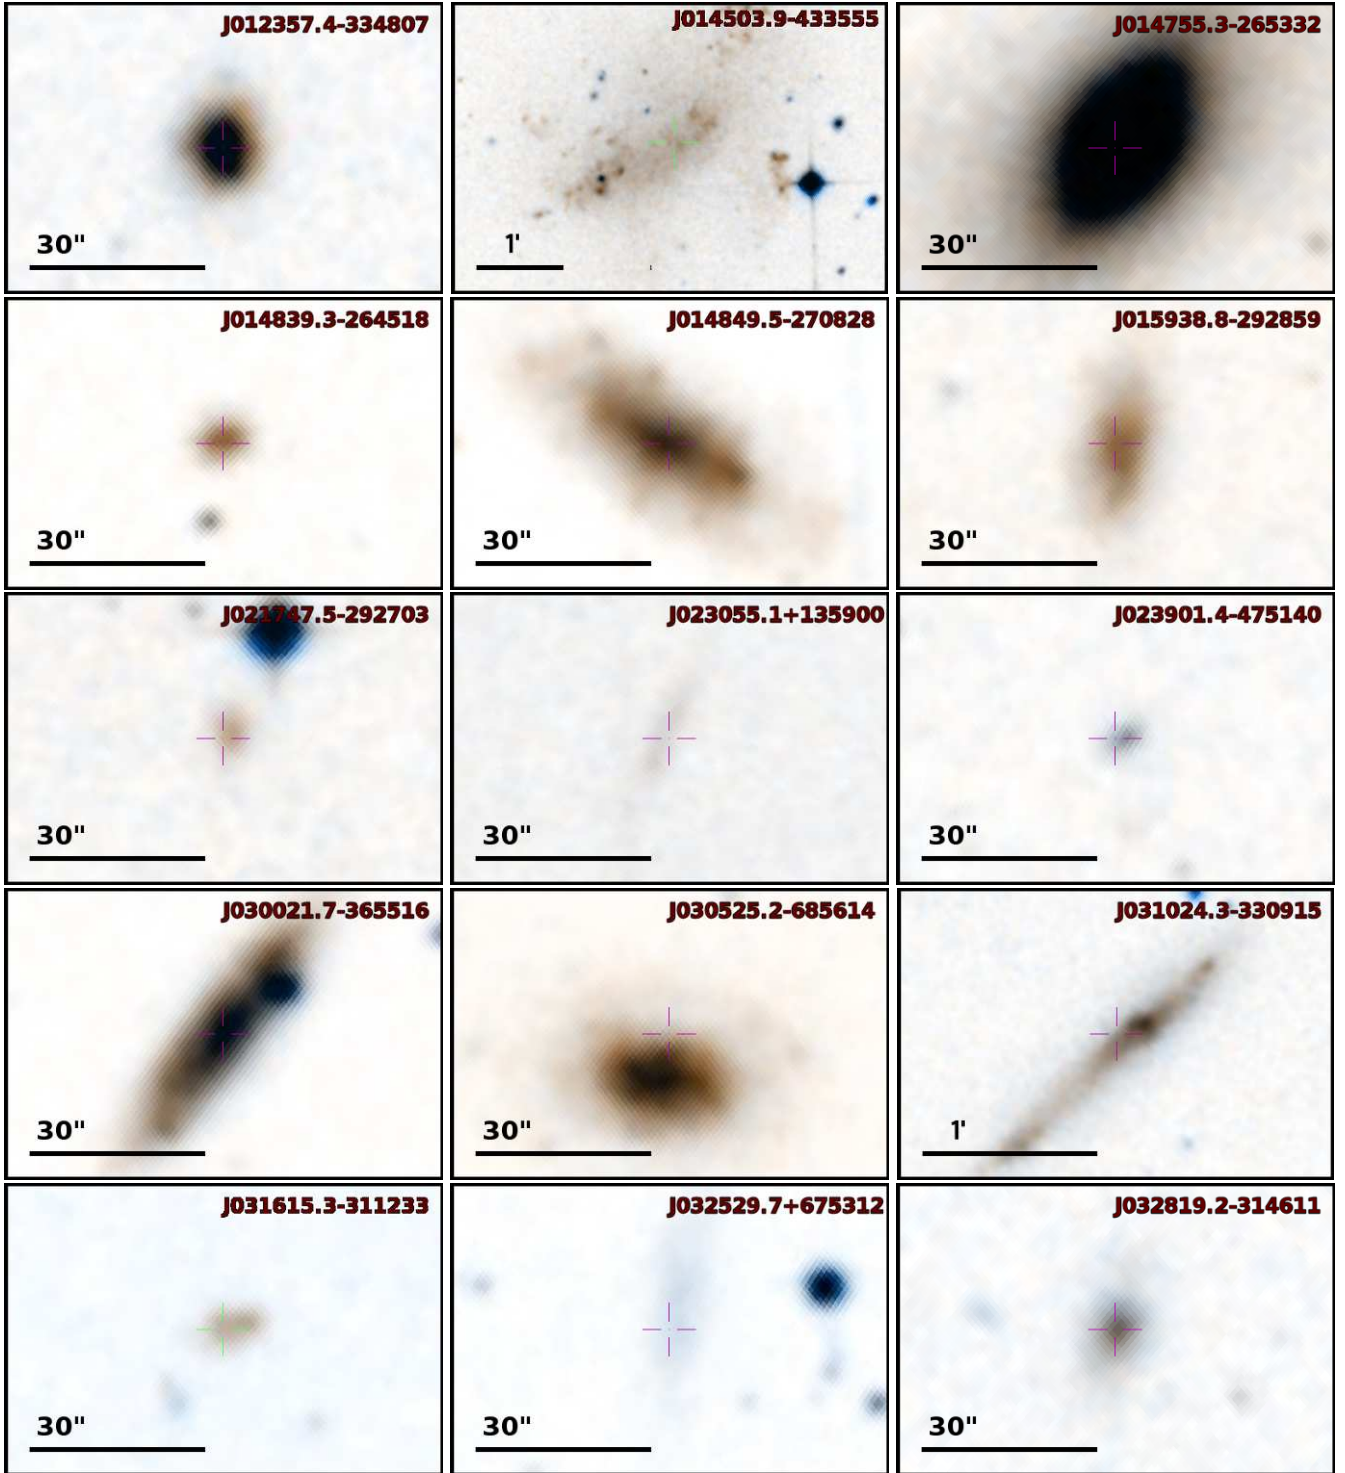

Figure A72. Nearby Void outer galaxies outside the SDSS footprint.

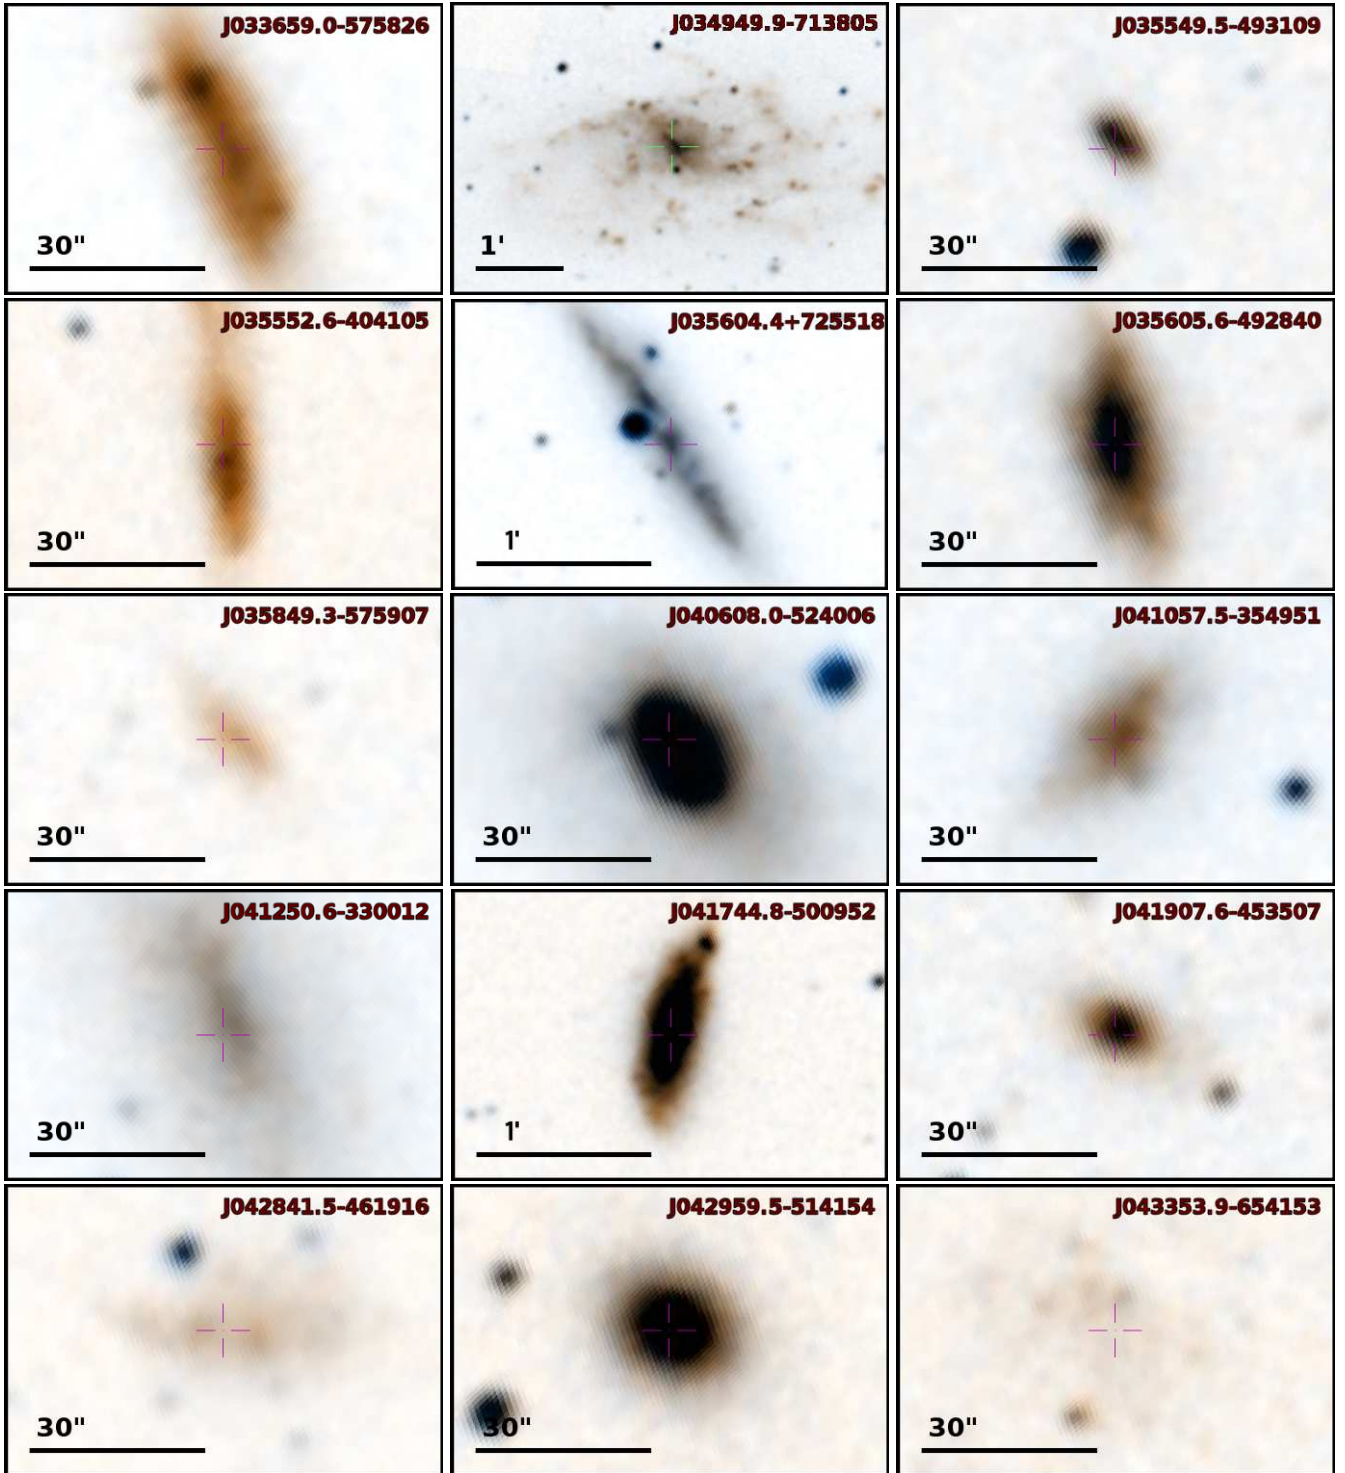

Figure A73. Nearby Void outer galaxies outside the SDSS footprint.



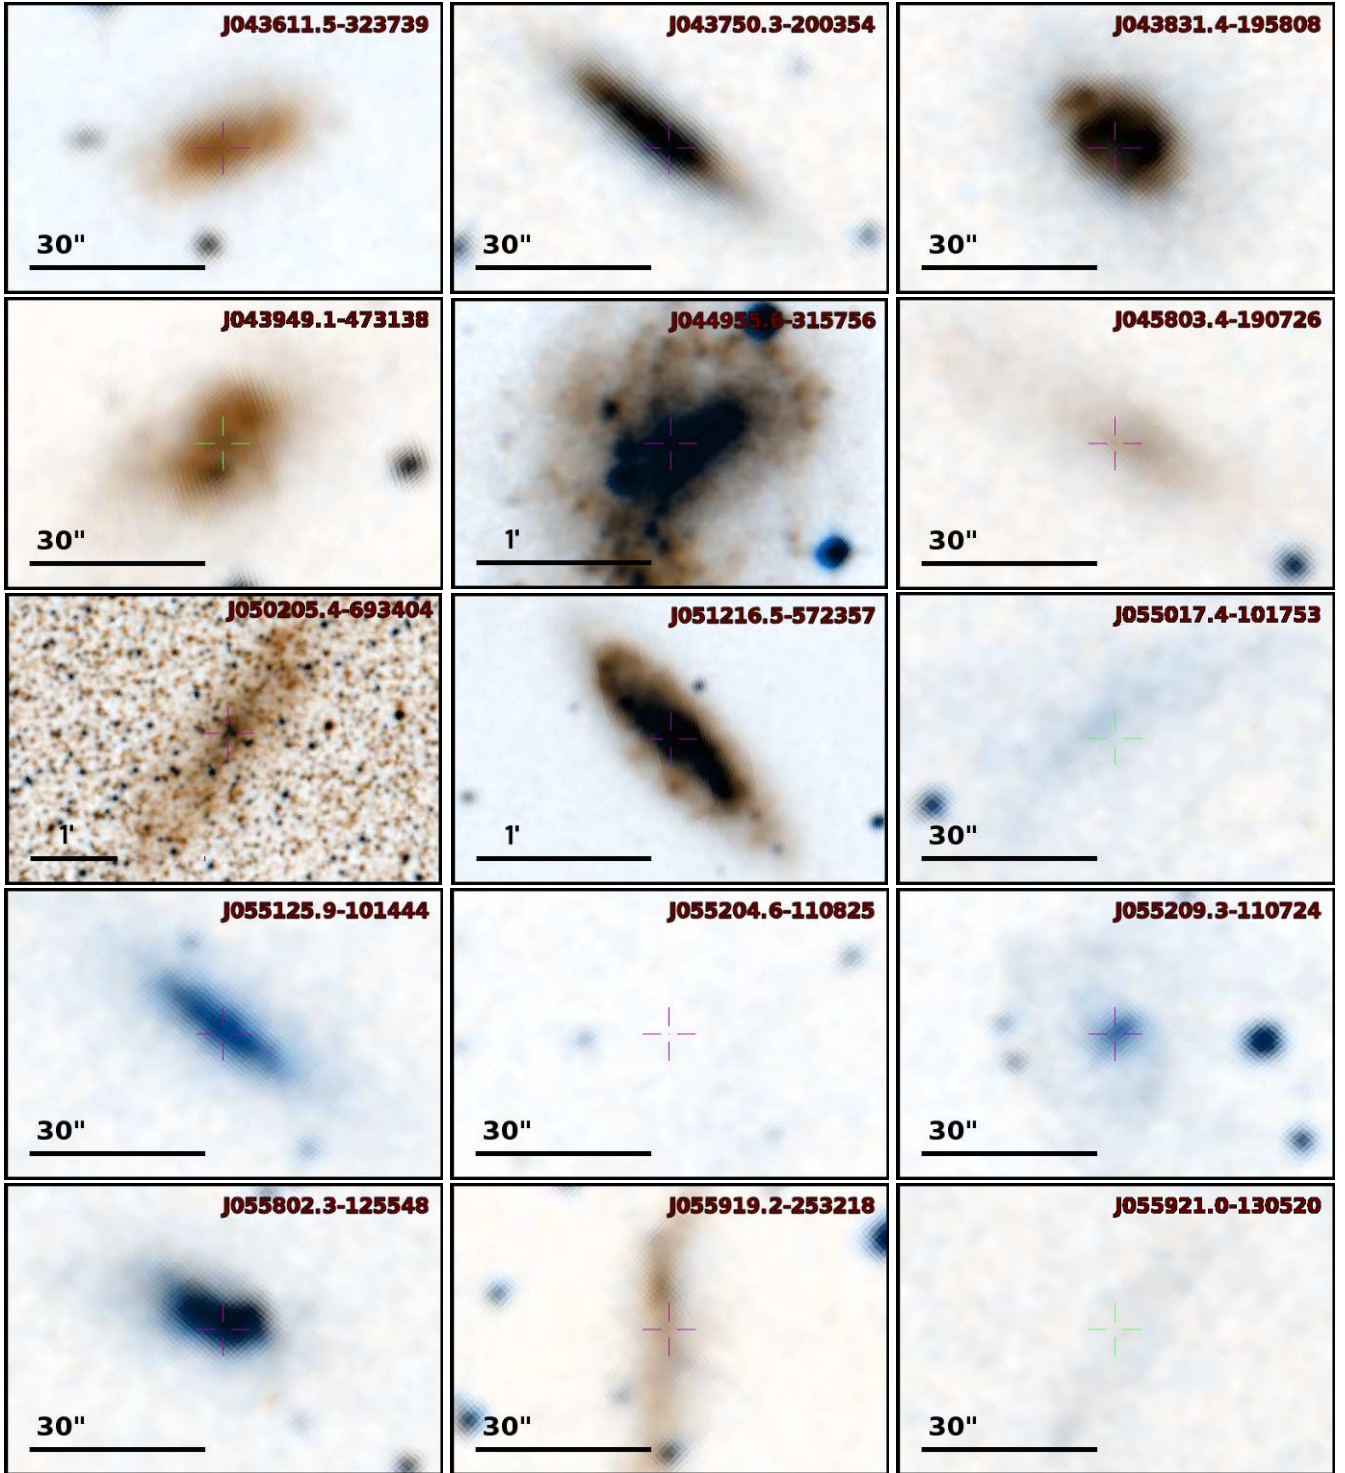

Figure A74. Nearby Void outer galaxies outside the SDSS footprint.



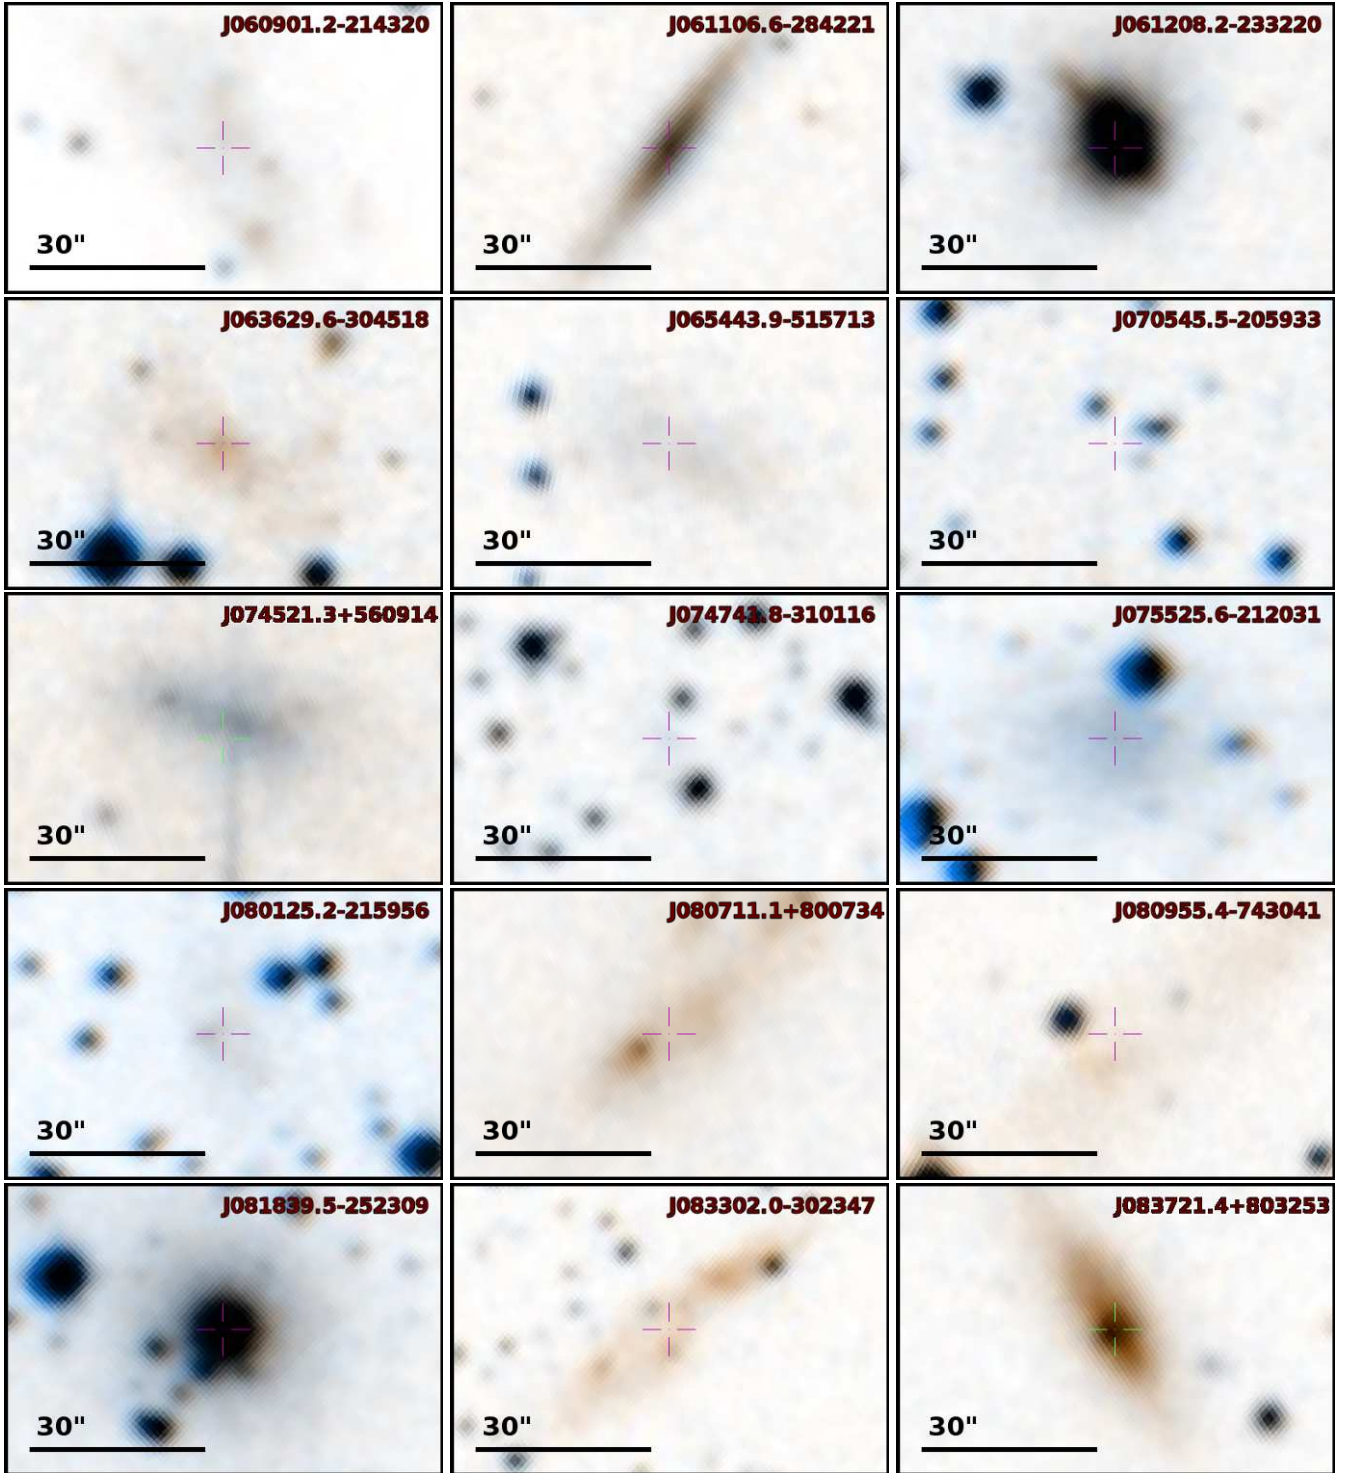

Figure A75. Nearby Void outer galaxies outside the SDSS footprint.

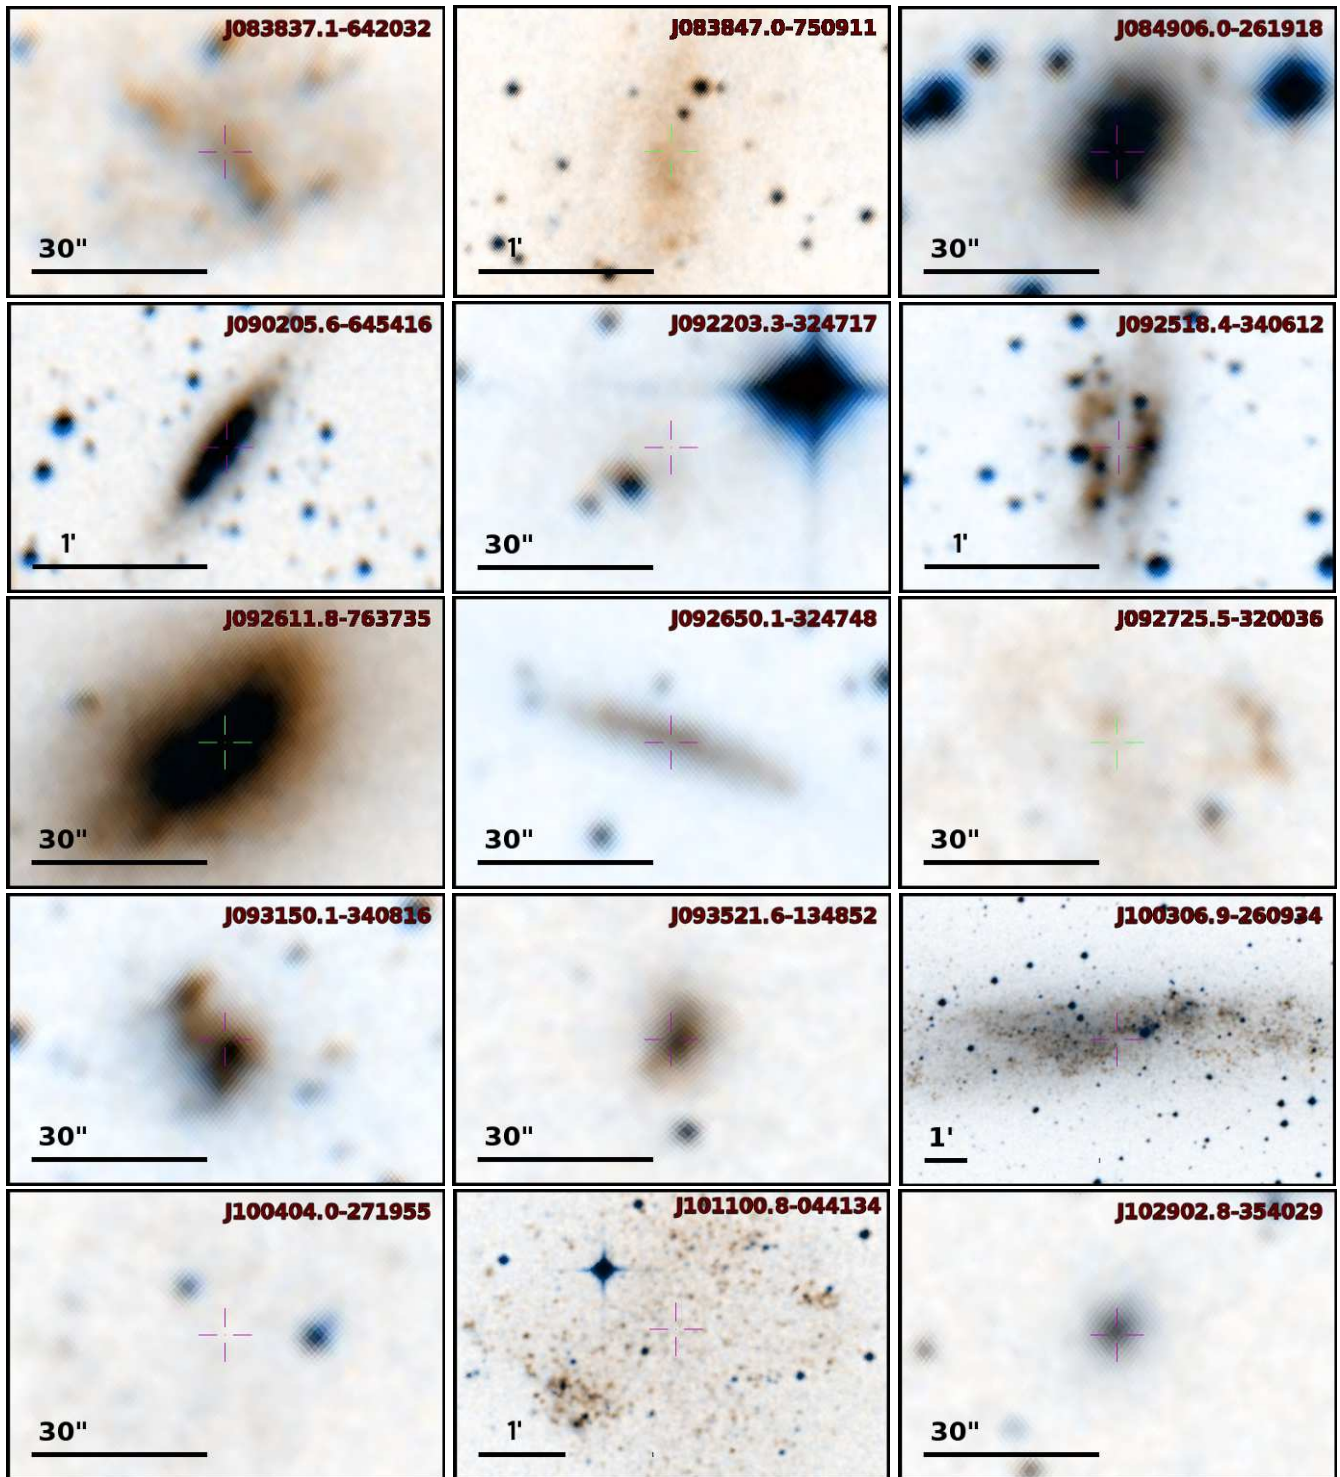

Figure A76. Nearby Void outer galaxies outside the SDSS footprint.



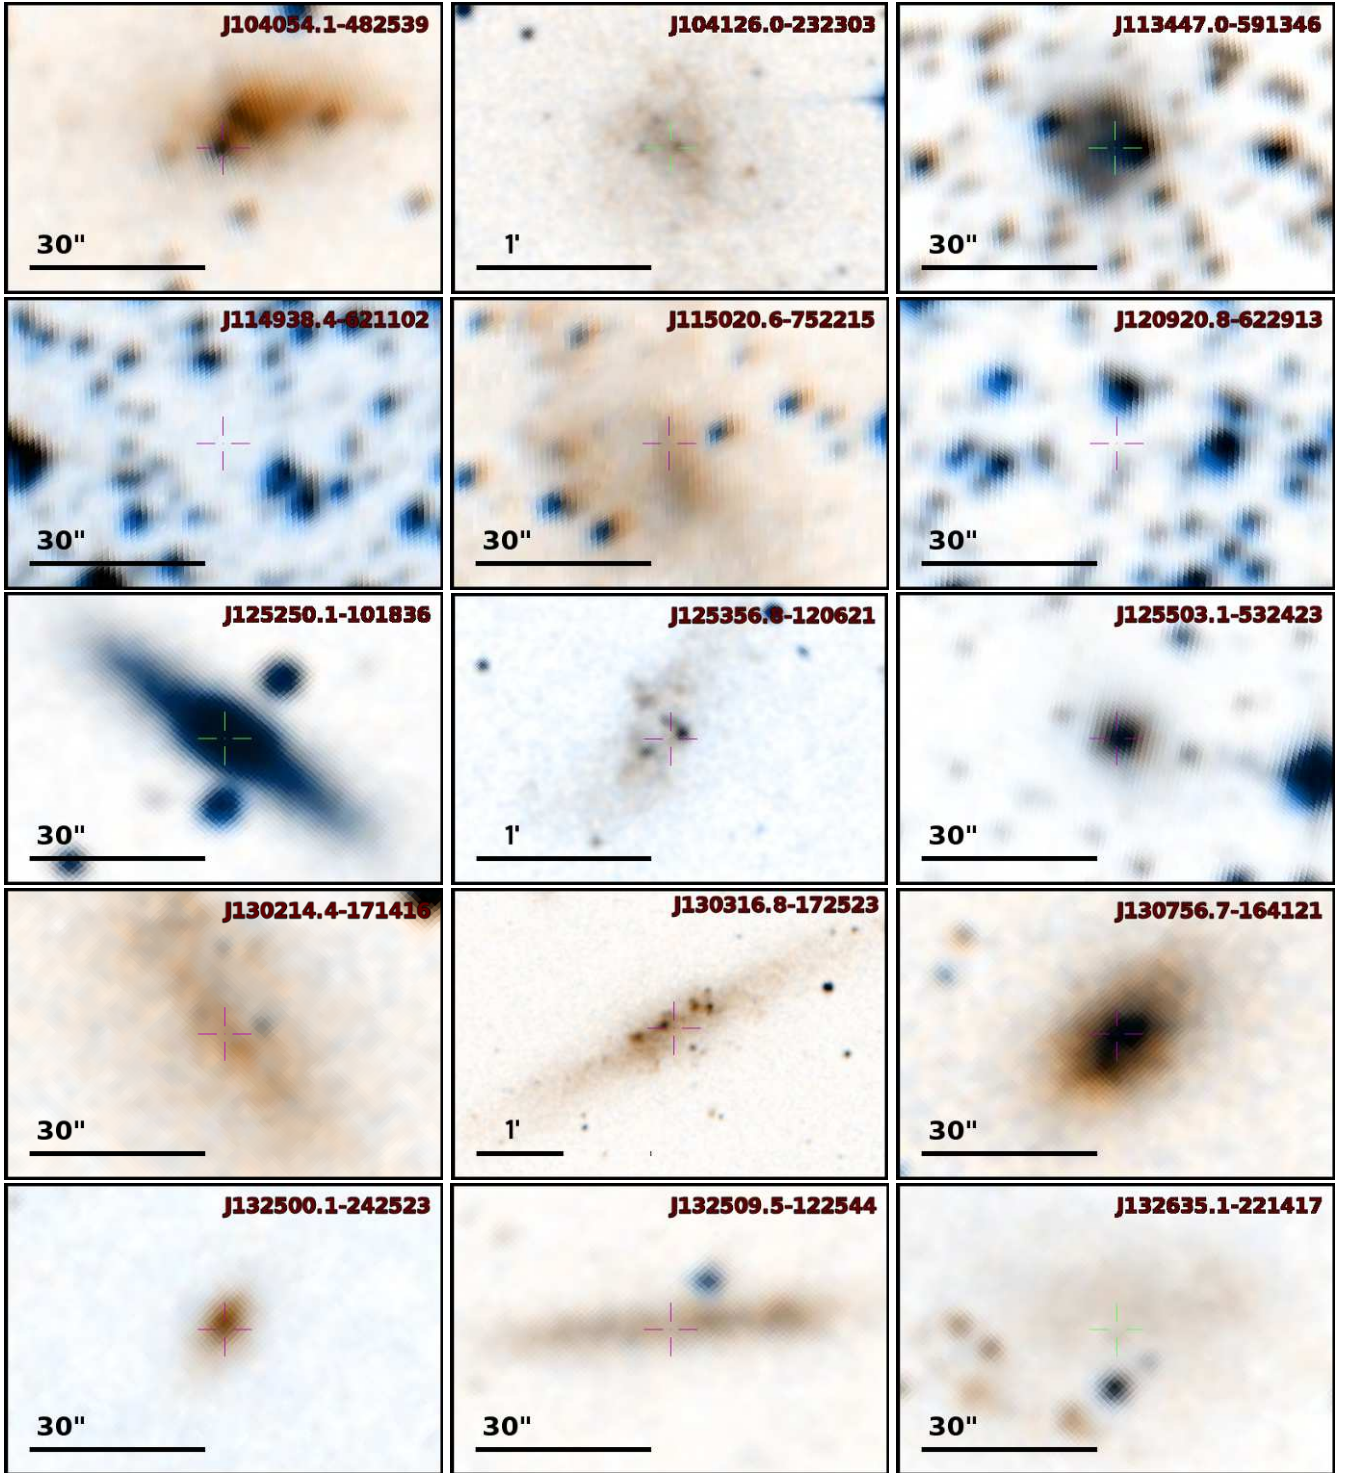

Figure A77. Nearby Void outer galaxies outside the SDSS footprint.

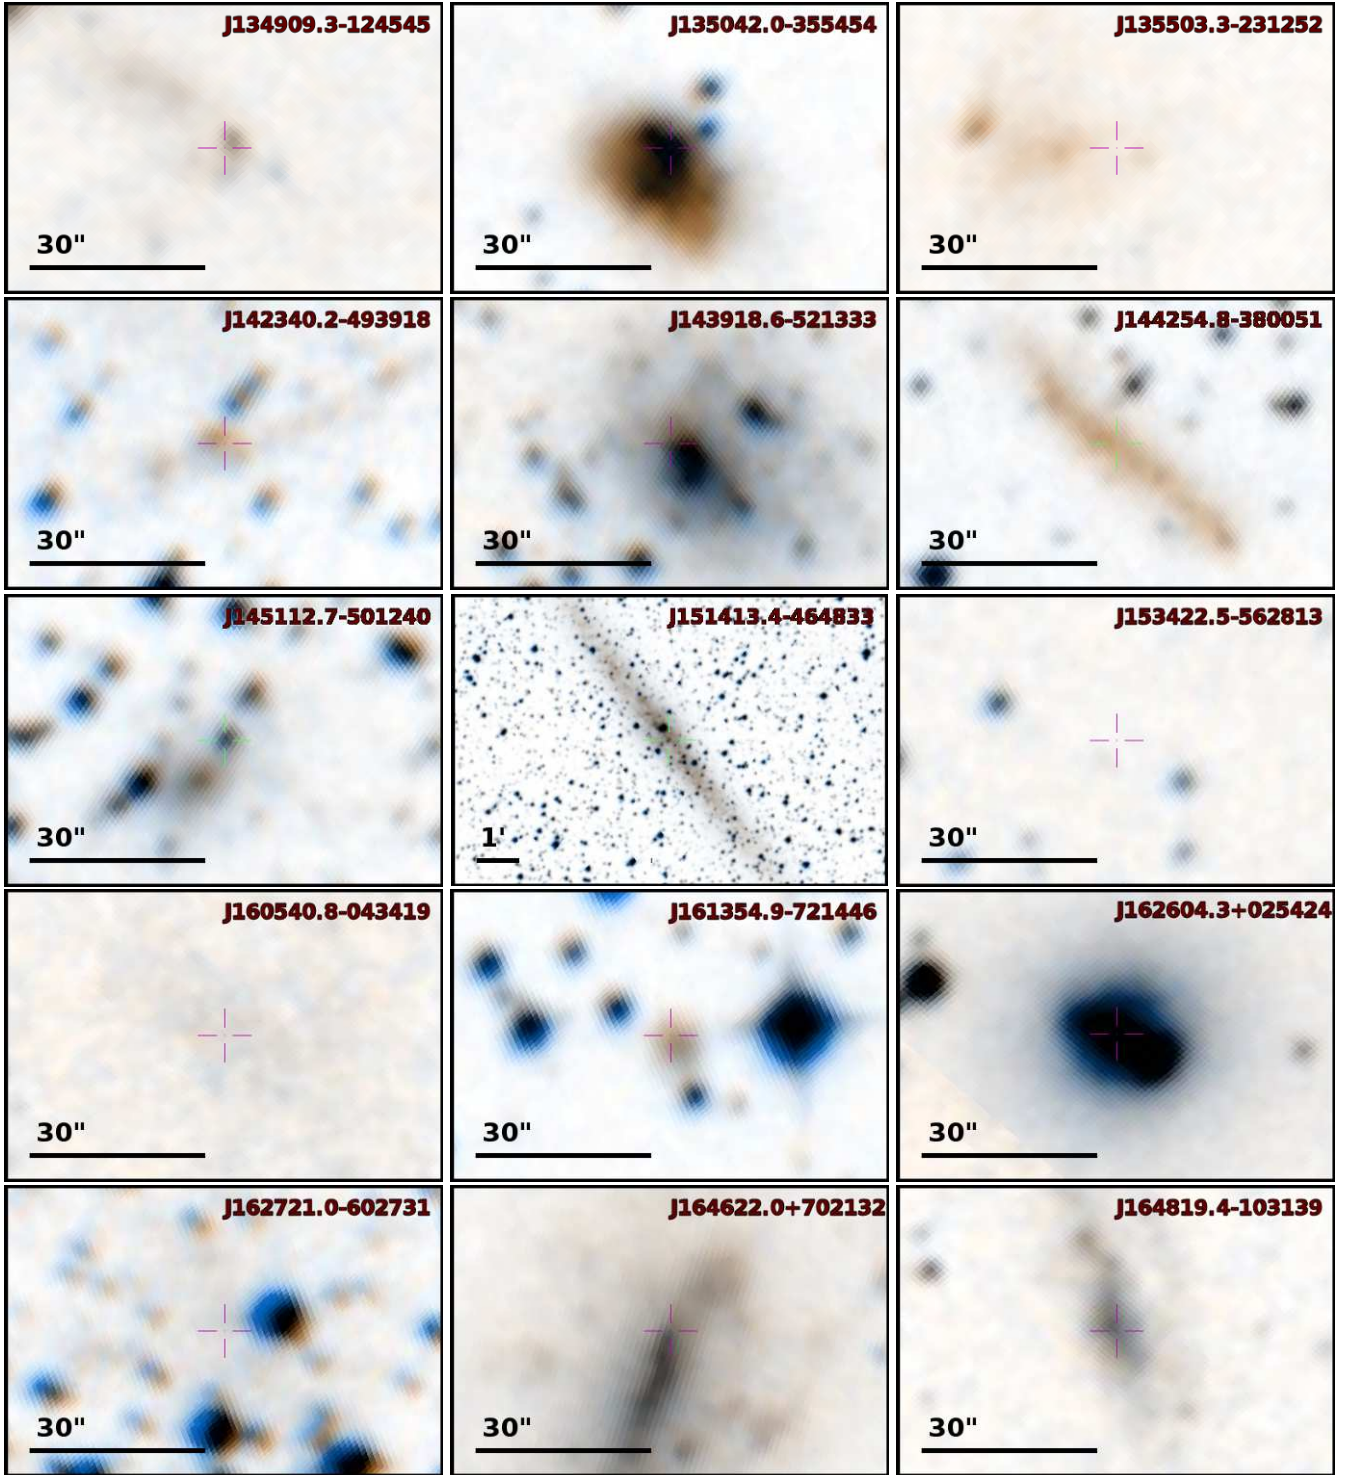

Figure A78. Nearby Void outer galaxies outside the SDSS footprint.



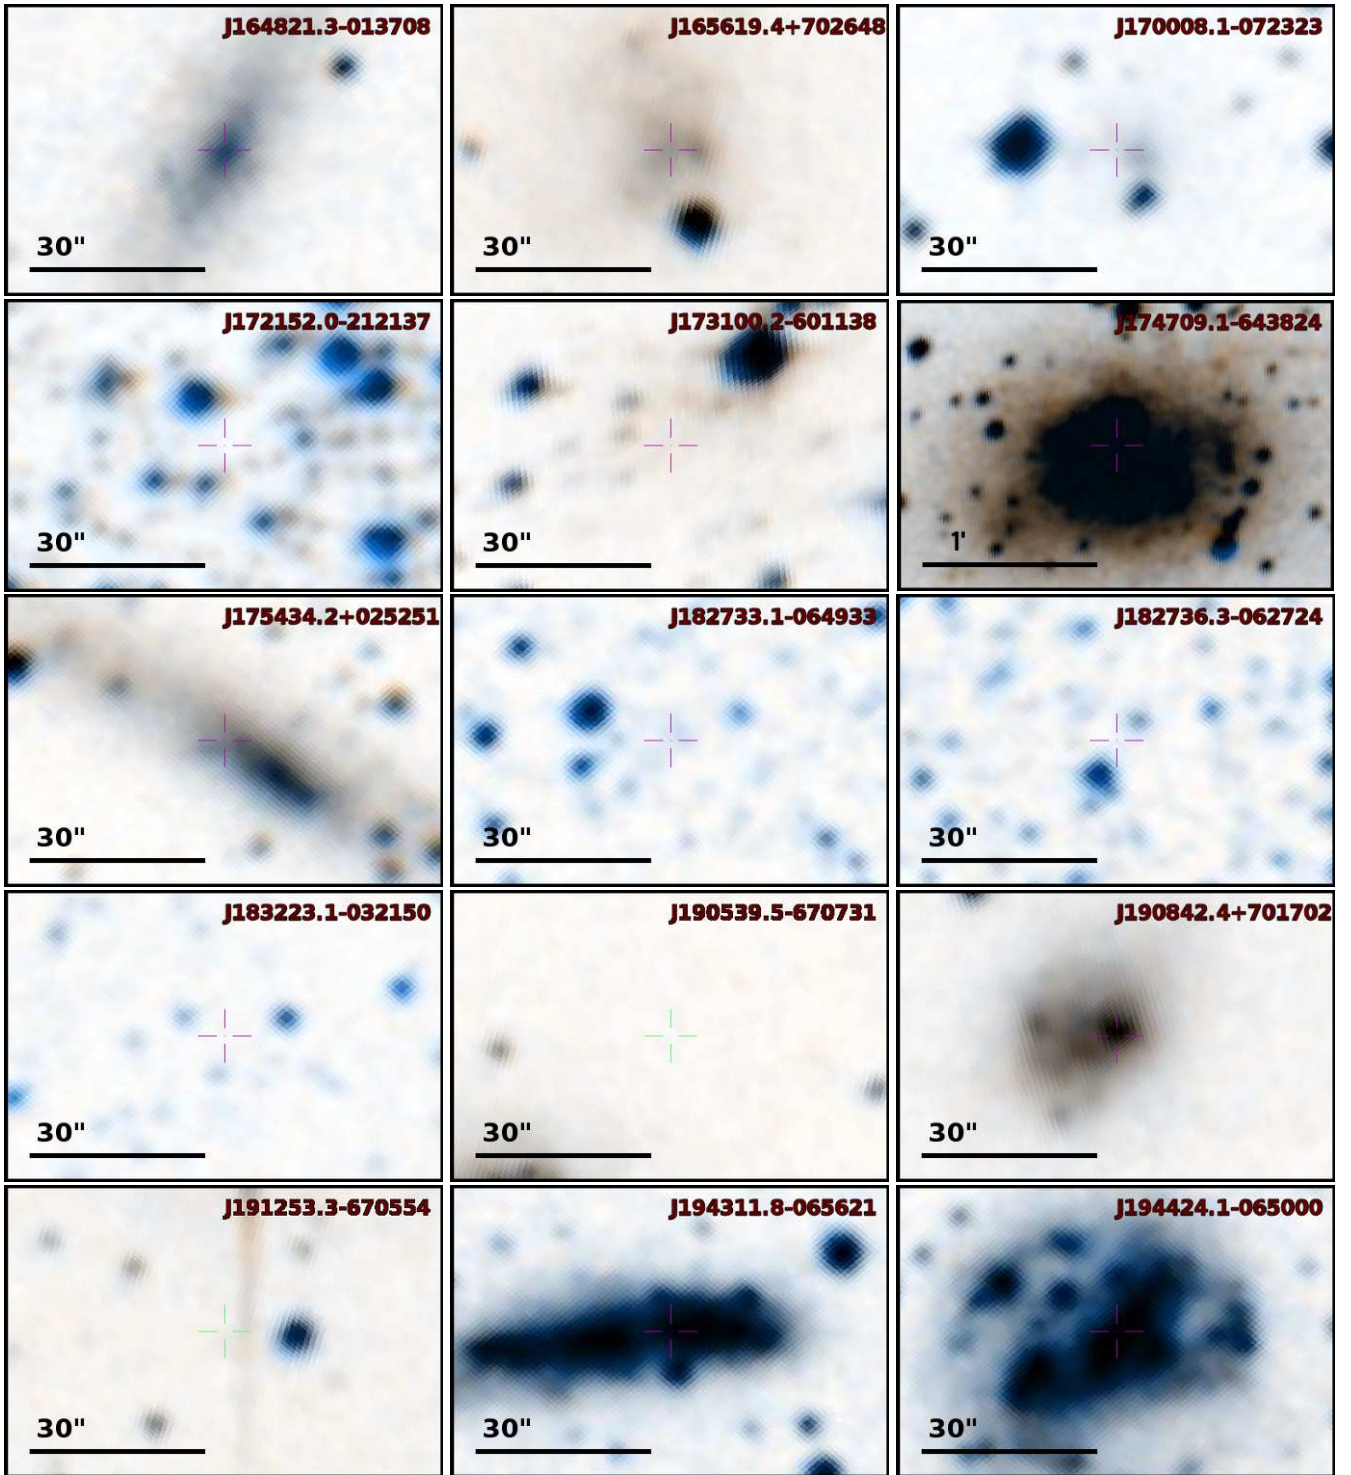

Figure A79. Nearby Void outer galaxies outside the SDSS footprint.

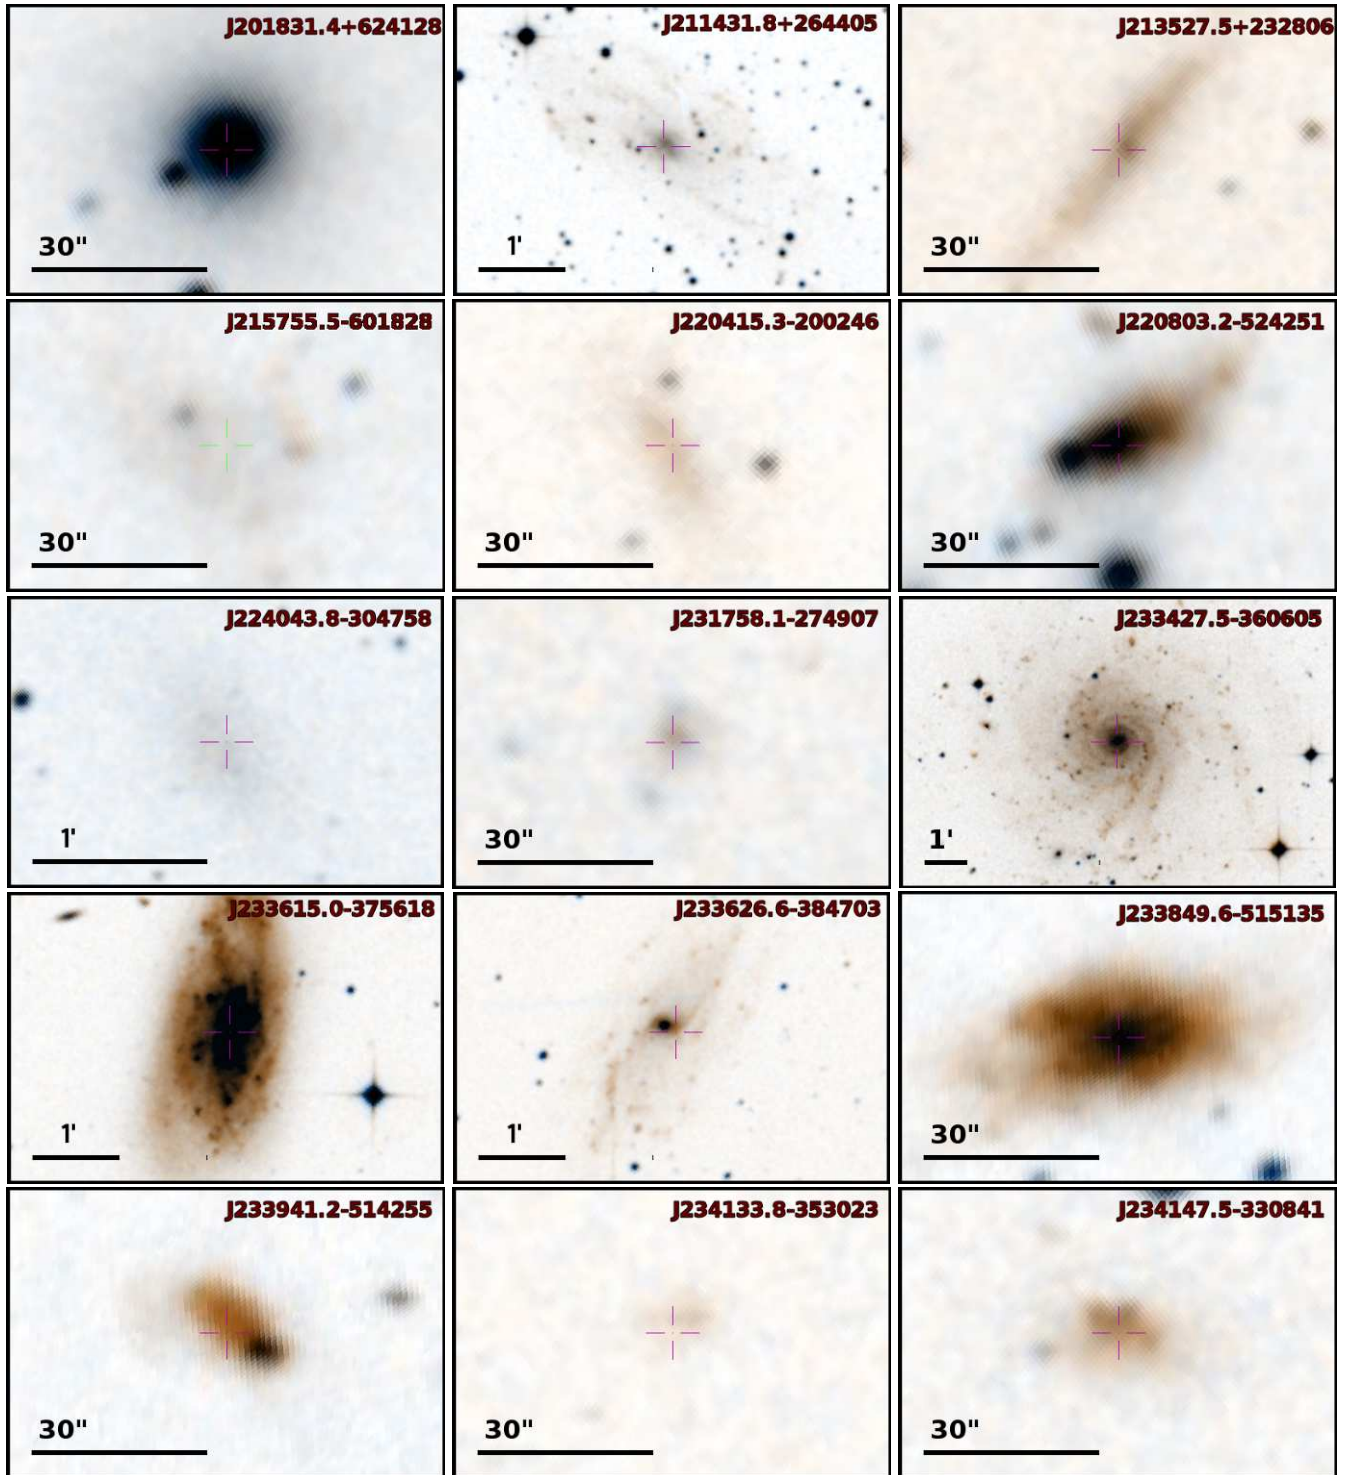

Figure A80. Nearby Void outer galaxies outside the SDSS footprint.

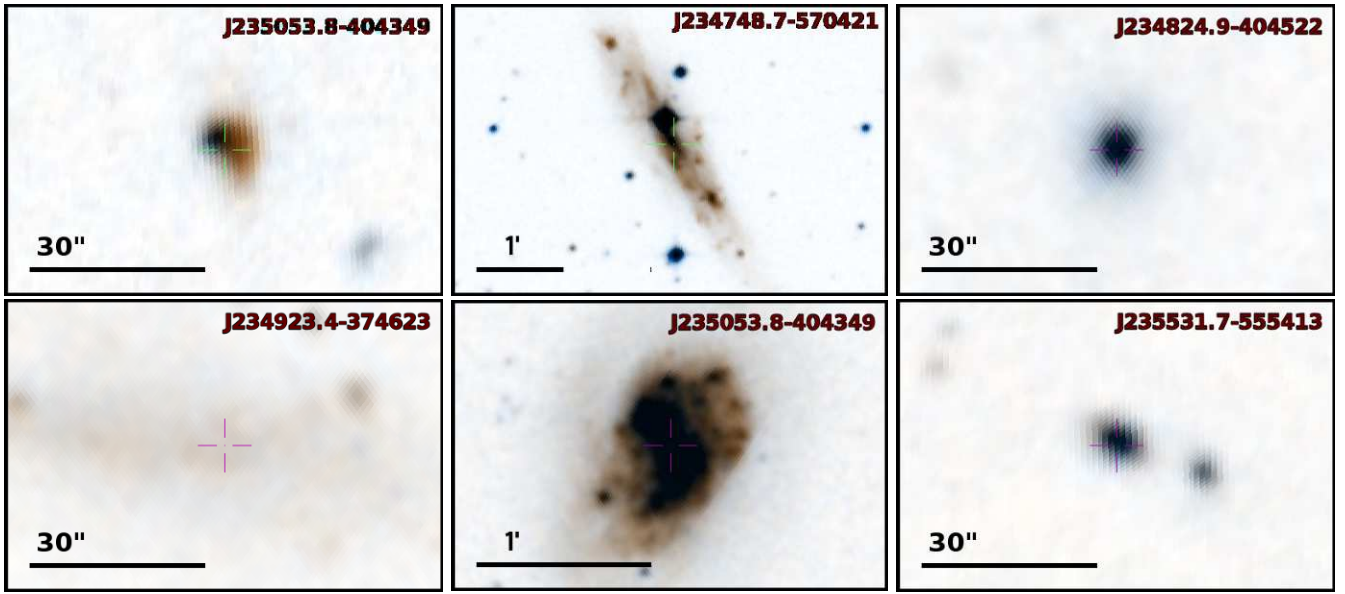

Figure A81. Nearby Void outer galaxies outside the SDSS footprint.
